# Supplementary material for: Neural Networks with Physics-Informed Architectures and Constraints for Dynamical Systems Modeling
Source: arXiv:2109.06407 source file (2022-12-12)
Supplement: Supplementary file 1 [file constraint_loss_data.tex]

\definecolor{color0}{rgb}{1,0,1}

\path [fill=color0, fill opacity=0.4, semithick]
(axis cs:0,8.41387367248535)
--(axis cs:0,7.63184022903442)
--(axis cs:100,7.63175487518311)
--(axis cs:200,7.61650228500366)
--(axis cs:300,0.0006866455078125)
--(axis cs:400,0.000645446765702218)
--(axis cs:500,0.000576019287109375)
--(axis cs:600,0.000528717064298689)
--(axis cs:700,0.000510406505782157)
--(axis cs:800,0.000514984130859375)
--(axis cs:900,0.0408084243535995)
--(axis cs:1000,0.0459358505904675)
--(axis cs:1100,0.160048678517342)
--(axis cs:1200,0.201066821813583)
--(axis cs:1300,0.473329156637192)
--(axis cs:1400,0.406928241252899)
--(axis cs:1500,0.51608282327652)
--(axis cs:1600,0.690039813518524)
--(axis cs:1700,0.666200697422028)
--(axis cs:1800,1.13009893894196)
--(axis cs:1900,1.4127676486969)
--(axis cs:2000,1.67491173744202)
--(axis cs:2100,1.91194152832031)
--(axis cs:2200,2.33479690551758)
--(axis cs:2300,2.6640031337738)
--(axis cs:2400,2.73953890800476)
--(axis cs:2500,2.79550743103027)
--(axis cs:2600,3.30379939079285)
--(axis cs:2700,3.47955751419067)
--(axis cs:2800,3.56284022331238)
--(axis cs:2900,3.95066022872925)
--(axis cs:3000,4.05537939071655)
--(axis cs:3100,3.70586371421814)
--(axis cs:3200,4.09778451919556)
--(axis cs:3300,4.16625499725342)
--(axis cs:3400,4.67464876174927)
--(axis cs:3500,4.82595825195312)
--(axis cs:3600,5.86706829071045)
--(axis cs:3700,6.20315456390381)
--(axis cs:3800,6.64736318588257)
--(axis cs:3900,6.87308120727539)
--(axis cs:4000,6.55149078369141)
--(axis cs:4100,6.26373434066772)
--(axis cs:4200,5.97647094726562)
--(axis cs:4300,5.79604244232178)
--(axis cs:4400,6.80171871185303)
--(axis cs:4500,7.44239521026611)
--(axis cs:4600,8.22664833068848)
--(axis cs:4700,8.28733825683594)
--(axis cs:4800,7.99957466125488)
--(axis cs:4900,7.83669900894165)
--(axis cs:5000,7.97837972640991)
--(axis cs:5100,7.4248194694519)
--(axis cs:5200,7.04610109329224)
--(axis cs:5300,7.18055152893066)
--(axis cs:5400,8.01148128509521)
--(axis cs:5500,8.35300922393799)
--(axis cs:5600,7.4183931350708)
--(axis cs:5700,7.456298828125)
--(axis cs:5800,8.8077392578125)
--(axis cs:5900,8.00116539001465)
--(axis cs:6000,7.66686296463013)
--(axis cs:6100,7.48223161697388)
--(axis cs:6200,7.62960767745972)
--(axis cs:6300,6.42214202880859)
--(axis cs:6400,5.85565423965454)
--(axis cs:6500,5.71112155914307)
--(axis cs:6600,5.8490743637085)
--(axis cs:6700,6.07038021087646)
--(axis cs:6800,6.13049983978271)
--(axis cs:6900,6.20547103881836)
--(axis cs:7000,5.73598527908325)
--(axis cs:7100,6.1784291267395)
--(axis cs:7200,5.76655864715576)
--(axis cs:7300,5.90010356903076)
--(axis cs:7400,5.92307138442993)
--(axis cs:7500,5.97251605987549)
--(axis cs:7600,4.95956611633301)
--(axis cs:7700,4.96305322647095)
--(axis cs:7800,4.73349046707153)
--(axis cs:7900,5.86385869979858)
--(axis cs:8000,5.85897731781006)
--(axis cs:8100,6.18974018096924)
--(axis cs:8200,5.71666812896729)
--(axis cs:8300,5.46551179885864)
--(axis cs:8400,4.82412910461426)
--(axis cs:8500,4.61865043640137)
--(axis cs:8600,4.79533672332764)
--(axis cs:8700,4.90513324737549)
--(axis cs:8800,5.10430908203125)
--(axis cs:8900,5.26723718643188)
--(axis cs:9000,5.21361875534058)
--(axis cs:9100,4.95327186584473)
--(axis cs:9200,4.9489164352417)
--(axis cs:9300,4.62161874771118)
--(axis cs:9400,3.87828803062439)
--(axis cs:9500,4.17340421676636)
--(axis cs:9600,3.99137926101685)
--(axis cs:9700,4.10009765625)
--(axis cs:9800,4.01424741744995)
--(axis cs:9900,3.7936224937439)
--(axis cs:10000,4.1210618019104)
--(axis cs:10100,4.42196035385132)
--(axis cs:10200,4.72764158248901)
--(axis cs:10300,4.63932991027832)
--(axis cs:10400,4.51777362823486)
--(axis cs:10500,4.26390647888184)
--(axis cs:10600,4.31695890426636)
--(axis cs:10700,4.24930906295776)
--(axis cs:10800,4.24373769760132)
--(axis cs:10900,4.32976007461548)
--(axis cs:11000,4.87548589706421)
--(axis cs:11100,4.59371328353882)
--(axis cs:11200,4.25072431564331)
--(axis cs:11300,4.12395048141479)
--(axis cs:11400,3.90697336196899)
--(axis cs:11500,3.55652904510498)
--(axis cs:11600,3.91560053825378)
--(axis cs:11700,3.84647226333618)
--(axis cs:11800,3.97954058647156)
--(axis cs:11900,4.12263059616089)
--(axis cs:12000,4.18025684356689)
--(axis cs:12100,4.27630233764648)
--(axis cs:12200,4.00827074050903)
--(axis cs:12300,3.52186250686646)
--(axis cs:12400,3.44220876693726)
--(axis cs:12500,3.59850907325745)
--(axis cs:12600,3.50187873840332)
--(axis cs:12700,3.61796474456787)
--(axis cs:12800,3.6900646686554)
--(axis cs:12900,3.57481336593628)
--(axis cs:13000,3.41230940818787)
--(axis cs:13100,3.52352380752563)
--(axis cs:13200,4.04837656021118)
--(axis cs:13300,3.84902262687683)
--(axis cs:13400,3.81728410720825)
--(axis cs:13500,3.46647214889526)
--(axis cs:13600,3.44792485237122)
--(axis cs:13700,3.38343596458435)
--(axis cs:13800,3.56418061256409)
--(axis cs:13900,3.58167886734009)
--(axis cs:14000,3.65338897705078)
--(axis cs:14100,3.59256720542908)
--(axis cs:14200,3.38715076446533)
--(axis cs:14300,3.14019060134888)
--(axis cs:14400,3.08116674423218)
--(axis cs:14500,3.36102485656738)
--(axis cs:14600,3.17252254486084)
--(axis cs:14700,2.88228535652161)
--(axis cs:14800,2.9154691696167)
--(axis cs:14900,2.92670202255249)
--(axis cs:15000,2.82349634170532)
--(axis cs:15100,3.15548276901245)
--(axis cs:15200,3.28294801712036)
--(axis cs:15300,3.16390371322632)
--(axis cs:15400,3.13470935821533)
--(axis cs:15500,3.0826473236084)
--(axis cs:15600,3.03697514533997)
--(axis cs:15700,2.75079202651978)
--(axis cs:15800,2.67040848731995)
--(axis cs:15900,2.87613081932068)
--(axis cs:16000,3.01404690742493)
--(axis cs:16100,3.03815579414368)
--(axis cs:16200,3.16276431083679)
--(axis cs:16300,3.22609996795654)
--(axis cs:16400,2.90699791908264)
--(axis cs:16500,2.80696487426758)
--(axis cs:16600,2.83980226516724)
--(axis cs:16700,2.82849931716919)
--(axis cs:16800,2.76139259338379)
--(axis cs:16900,2.87691450119019)
--(axis cs:17000,2.67355394363403)
--(axis cs:17100,2.77340364456177)
--(axis cs:17200,2.83211040496826)
--(axis cs:17300,2.79898285865784)
--(axis cs:17400,2.65877461433411)
--(axis cs:17500,2.75625777244568)
--(axis cs:17600,2.57911920547485)
--(axis cs:17700,2.55428004264832)
--(axis cs:17800,2.57290077209473)
--(axis cs:17900,2.61156129837036)
--(axis cs:18000,2.8154182434082)
--(axis cs:18100,2.75100207328796)
--(axis cs:18200,2.75727820396423)
--(axis cs:18300,2.80413389205933)
--(axis cs:18400,2.81148767471313)
--(axis cs:18500,2.67538070678711)
--(axis cs:18600,2.71283292770386)
--(axis cs:18700,2.70105624198914)
--(axis cs:18800,2.73266577720642)
--(axis cs:18900,2.84857606887817)
--(axis cs:19000,2.97241306304932)
--(axis cs:19100,2.93081259727478)
--(axis cs:19200,2.88247776031494)
--(axis cs:19300,2.7573082447052)
--(axis cs:19400,2.60763835906982)
--(axis cs:19500,2.39734172821045)
--(axis cs:19600,2.92694473266602)
--(axis cs:19700,3.15997314453125)
--(axis cs:19800,3.29364013671875)
--(axis cs:19900,3.36518096923828)
--(axis cs:20000,3.314208984375)
--(axis cs:20100,2.80626392364502)
--(axis cs:20200,2.81702423095703)
--(axis cs:20300,2.69749307632446)
--(axis cs:20400,2.66385507583618)
--(axis cs:20500,2.58675527572632)
--(axis cs:20600,2.58428955078125)
--(axis cs:20700,2.6683349609375)
--(axis cs:20800,2.76310396194458)
--(axis cs:20900,2.61253666877747)
--(axis cs:21000,2.41082763671875)
--(axis cs:21100,2.66192102432251)
--(axis cs:21200,2.50179696083069)
--(axis cs:21300,2.41188097000122)
--(axis cs:21400,2.60182976722717)
--(axis cs:21500,2.59817314147949)
--(axis cs:21600,2.50177264213562)
--(axis cs:21700,2.51591777801514)
--(axis cs:21800,2.39096879959106)
--(axis cs:21900,2.56327128410339)
--(axis cs:22000,2.82365465164185)
--(axis cs:22100,2.74634003639221)
--(axis cs:22200,2.62802648544312)
--(axis cs:22300,2.70856642723083)
--(axis cs:22400,2.43293166160583)
--(axis cs:22500,2.2135009765625)
--(axis cs:22600,2.2135009765625)
--(axis cs:22700,2.2135009765625)
--(axis cs:22800,2.13381338119507)
--(axis cs:22900,2.2135009765625)
--(axis cs:23000,2.24750375747681)
--(axis cs:23100,2.2135009765625)
--(axis cs:23200,2.31971621513367)
--(axis cs:23300,2.36542558670044)
--(axis cs:23400,2.36827898025513)
--(axis cs:23500,2.39692306518555)
--(axis cs:23600,2.39892315864563)
--(axis cs:23700,2.39850544929504)
--(axis cs:23800,2.35869312286377)
--(axis cs:23900,2.37741088867188)
--(axis cs:24000,2.29563474655151)
--(axis cs:24100,2.36462664604187)
--(axis cs:24200,2.36767339706421)
--(axis cs:24300,2.36420607566833)
--(axis cs:24400,2.28696727752686)
--(axis cs:24500,2.33148527145386)
--(axis cs:24600,2.28137564659119)
--(axis cs:24700,2.2135009765625)
--(axis cs:24800,2.2268373966217)
--(axis cs:24900,2.32068347930908)
--(axis cs:25000,2.33114004135132)
--(axis cs:25100,2.24976658821106)
--(axis cs:25200,2.24396705627441)
--(axis cs:25300,2.27048325538635)
--(axis cs:25400,2.2135009765625)
--(axis cs:25500,2.23799514770508)
--(axis cs:25600,2.28055095672607)
--(axis cs:25700,2.34997367858887)
--(axis cs:25800,2.27198553085327)
--(axis cs:25900,2.34653210639954)
--(axis cs:26000,2.24043440818787)
--(axis cs:26100,2.29117441177368)
--(axis cs:26200,2.21348881721497)
--(axis cs:26300,2.21348881721497)
--(axis cs:26400,2.23614454269409)
--(axis cs:26500,2.30545949935913)
--(axis cs:26600,2.21348881721497)
--(axis cs:26700,2.35226941108704)
--(axis cs:26800,2.35150980949402)
--(axis cs:26900,2.2135009765625)
--(axis cs:27000,2.2135009765625)
--(axis cs:27100,2.2135009765625)
--(axis cs:27200,1.72744524478912)
--(axis cs:27300,1.82268071174622)
--(axis cs:27400,1.77955937385559)
--(axis cs:27500,1.87575685977936)
--(axis cs:27600,2.01076650619507)
--(axis cs:27700,2.2135009765625)
--(axis cs:27800,2.2135009765625)
--(axis cs:27900,2.23010492324829)
--(axis cs:28000,2.2135009765625)
--(axis cs:28100,2.2135009765625)
--(axis cs:28200,2.2135009765625)
--(axis cs:28300,2.2135009765625)
--(axis cs:28400,2.2135009765625)
--(axis cs:28500,2.2135009765625)
--(axis cs:28600,2.2135009765625)
--(axis cs:28700,2.2135009765625)
--(axis cs:28800,2.20939946174622)
--(axis cs:28900,2.08012700080872)
--(axis cs:29000,2.2135009765625)
--(axis cs:29100,2.2135009765625)
--(axis cs:29200,2.04013681411743)
--(axis cs:29300,2.2135009765625)
--(axis cs:29400,2.2135009765625)
--(axis cs:29500,2.20463871955872)
--(axis cs:29600,2.2135009765625)
--(axis cs:29700,2.30518078804016)
--(axis cs:29800,2.29588079452515)
--(axis cs:29900,2.23435521125793)
--(axis cs:30000,2.25114941596985)
--(axis cs:30100,2.28232741355896)
--(axis cs:30200,2.2135009765625)
--(axis cs:30300,2.2135009765625)
--(axis cs:30400,2.2135009765625)
--(axis cs:30500,2.22461986541748)
--(axis cs:30600,1.97709965705872)
--(axis cs:30700,2.19704580307007)
--(axis cs:30800,2.2135009765625)
--(axis cs:30900,2.16652822494507)
--(axis cs:31000,2.02177739143372)
--(axis cs:31100,2.12392568588257)
--(axis cs:31200,1.91191411018372)
--(axis cs:31300,2.10488271713257)
--(axis cs:31300,3.09048056602478)
--(axis cs:31300,3.09048056602478)
--(axis cs:31200,3.08254861831665)
--(axis cs:31100,3.09177398681641)
--(axis cs:31000,3.08596873283386)
--(axis cs:30900,3.09504318237305)
--(axis cs:30800,3.10142159461975)
--(axis cs:30700,3.0977189540863)
--(axis cs:30600,3.08425092697144)
--(axis cs:30500,3.14928960800171)
--(axis cs:30400,3.13775086402893)
--(axis cs:30300,3.11360430717468)
--(axis cs:30200,3.13546466827393)
--(axis cs:30100,3.18508791923523)
--(axis cs:30000,3.16388964653015)
--(axis cs:29900,3.1543333530426)
--(axis cs:29800,3.1960301399231)
--(axis cs:29700,3.20427584648132)
--(axis cs:29600,3.13989329338074)
--(axis cs:29500,3.09842967987061)
--(axis cs:29400,3.13490581512451)
--(axis cs:29300,3.10174989700317)
--(axis cs:29200,3.08681344985962)
--(axis cs:29100,3.10332918167114)
--(axis cs:29000,3.12042331695557)
--(axis cs:28900,3.08894801139832)
--(axis cs:28800,3.09888458251953)
--(axis cs:28700,3.14004182815552)
--(axis cs:28600,3.13656449317932)
--(axis cs:28500,3.13244724273682)
--(axis cs:28400,3.11653661727905)
--(axis cs:28300,3.14014625549316)
--(axis cs:28200,3.14000749588013)
--(axis cs:28100,3.1314709186554)
--(axis cs:28000,3.11426401138306)
--(axis cs:27900,3.15208911895752)
--(axis cs:27800,3.1072518825531)
--(axis cs:27700,3.10129165649414)
--(axis cs:27600,3.0855016708374)
--(axis cs:27500,3.08198595046997)
--(axis cs:27400,3.08178496360779)
--(axis cs:27300,3.08161497116089)
--(axis cs:27200,3.08284139633179)
--(axis cs:27100,3.10924100875854)
--(axis cs:27000,3.10985040664673)
--(axis cs:26900,3.13947892189026)
--(axis cs:26800,3.25757193565369)
--(axis cs:26700,3.2586681842804)
--(axis cs:26600,3.14334487915039)
--(axis cs:26500,3.20454216003418)
--(axis cs:26400,3.15530252456665)
--(axis cs:26300,3.1313271522522)
--(axis cs:26200,3.11738157272339)
--(axis cs:26100,3.19209384918213)
--(axis cs:26000,3.1576611995697)
--(axis cs:25900,3.25060343742371)
--(axis cs:25800,3.17749404907227)
--(axis cs:25700,3.25538110733032)
--(axis cs:25600,3.18373966217041)
--(axis cs:25500,3.15630865097046)
--(axis cs:25400,3.13173198699951)
--(axis cs:25300,3.17644047737122)
--(axis cs:25200,3.1596622467041)
--(axis cs:25100,3.1630585193634)
--(axis cs:25000,3.23119735717773)
--(axis cs:24900,3.21958303451538)
--(axis cs:24800,3.15040898323059)
--(axis cs:24700,3.13064455986023)
--(axis cs:24600,3.18436312675476)
--(axis cs:24500,3.23160076141357)
--(axis cs:24400,3.1887001991272)
--(axis cs:24300,3.27720046043396)
--(axis cs:24200,3.28309154510498)
--(axis cs:24100,3.27790236473083)
--(axis cs:24000,3.19582033157349)
--(axis cs:23900,3.30108833312988)
--(axis cs:23800,3.26832485198975)
--(axis cs:23700,3.314208984375)
--(axis cs:23600,3.314208984375)
--(axis cs:23500,3.314208984375)
--(axis cs:23400,3.28414630889893)
--(axis cs:23300,3.2792444229126)
--(axis cs:23200,3.21856474876404)
--(axis cs:23100,3.14069366455078)
--(axis cs:23000,3.16171646118164)
--(axis cs:22900,3.10882186889648)
--(axis cs:22800,3.09248566627502)
--(axis cs:22700,3.11488080024719)
--(axis cs:22600,3.12983751296997)
--(axis cs:22500,3.14250731468201)
--(axis cs:22400,3.18675446510315)
--(axis cs:22300,3.314208984375)
--(axis cs:22200,3.26563358306885)
--(axis cs:22100,3.25318837165833)
--(axis cs:22000,3.314208984375)
--(axis cs:21900,3.314208984375)
--(axis cs:21800,3.28464984893799)
--(axis cs:21700,3.42427968978882)
--(axis cs:21600,3.41652822494507)
--(axis cs:21500,3.39010000228882)
--(axis cs:21400,3.314208984375)
--(axis cs:21300,3.314208984375)
--(axis cs:21200,3.21886563301086)
--(axis cs:21100,3.26416921615601)
--(axis cs:21000,3.14879584312439)
--(axis cs:20900,3.20102143287659)
--(axis cs:20800,3.24071264266968)
--(axis cs:20700,3.20414972305298)
--(axis cs:20600,3.17280292510986)
--(axis cs:20500,3.18395662307739)
--(axis cs:20400,3.21115779876709)
--(axis cs:20300,3.27118396759033)
--(axis cs:20200,3.28809499740601)
--(axis cs:20100,3.31080961227417)
--(axis cs:20000,3.82589387893677)
--(axis cs:19900,3.87583494186401)
--(axis cs:19800,3.94293165206909)
--(axis cs:19700,4.06288003921509)
--(axis cs:19600,4.14494657516479)
--(axis cs:19500,3.79407262802124)
--(axis cs:19400,3.39671635627747)
--(axis cs:19300,3.314208984375)
--(axis cs:19200,3.314208984375)
--(axis cs:19100,3.33260488510132)
--(axis cs:19000,3.314208984375)
--(axis cs:18900,3.314208984375)
--(axis cs:18800,3.49779057502747)
--(axis cs:18700,3.47506093978882)
--(axis cs:18600,3.2810230255127)
--(axis cs:18500,3.23034048080444)
--(axis cs:18400,3.28388977050781)
--(axis cs:18300,3.28841972351074)
--(axis cs:18200,3.26759171485901)
--(axis cs:18100,3.30141520500183)
--(axis cs:18000,3.76045227050781)
--(axis cs:17900,3.74915647506714)
--(axis cs:17800,3.94078779220581)
--(axis cs:17700,3.97451186180115)
--(axis cs:17600,4.2712550163269)
--(axis cs:17500,3.86858773231506)
--(axis cs:17400,4.0525369644165)
--(axis cs:17300,4.10319852828979)
--(axis cs:17200,4.04108285903931)
--(axis cs:17100,3.77439880371094)
--(axis cs:17000,3.87755298614502)
--(axis cs:16900,3.74327564239502)
--(axis cs:16800,3.50828862190247)
--(axis cs:16700,3.92070341110229)
--(axis cs:16600,4.08161735534668)
--(axis cs:16500,4.04100036621094)
--(axis cs:16400,4.09148788452148)
--(axis cs:16300,3.87878322601318)
--(axis cs:16200,3.41092562675476)
--(axis cs:16100,3.23454594612122)
--(axis cs:16000,3.18770289421082)
--(axis cs:15900,3.10547709465027)
--(axis cs:15800,3.26482939720154)
--(axis cs:15700,3.26515007019043)
--(axis cs:15600,3.52773809432983)
--(axis cs:15500,3.52309799194336)
--(axis cs:15400,3.25101613998413)
--(axis cs:15300,3.34386563301086)
--(axis cs:15200,3.38904094696045)
--(axis cs:15100,3.55247592926025)
--(axis cs:15000,3.73790502548218)
--(axis cs:14900,4.18122482299805)
--(axis cs:14800,4.18799829483032)
--(axis cs:14700,4.01092004776001)
--(axis cs:14600,3.79857110977173)
--(axis cs:14500,3.51630258560181)
--(axis cs:14400,3.58951425552368)
--(axis cs:14300,3.8664665222168)
--(axis cs:14200,3.87329816818237)
--(axis cs:14100,3.73712038993835)
--(axis cs:14000,3.98779296875)
--(axis cs:13900,3.77278900146484)
--(axis cs:13800,3.57837319374084)
--(axis cs:13700,3.70303797721863)
--(axis cs:13600,4.10337448120117)
--(axis cs:13500,4.2605619430542)
--(axis cs:13400,4.31583738327026)
--(axis cs:13300,4.14130973815918)
--(axis cs:13200,4.17723369598389)
--(axis cs:13100,4.20536613464355)
--(axis cs:13000,4.16358661651611)
--(axis cs:12900,4.27867746353149)
--(axis cs:12800,4.34906005859375)
--(axis cs:12700,4.29407978057861)
--(axis cs:12600,4.61332225799561)
--(axis cs:12500,4.34491491317749)
--(axis cs:12400,4.58044767379761)
--(axis cs:12300,4.60934686660767)
--(axis cs:12200,4.61270761489868)
--(axis cs:12100,4.84897470474243)
--(axis cs:12000,5.19589900970459)
--(axis cs:11900,5.25280904769897)
--(axis cs:11800,5.12901210784912)
--(axis cs:11700,4.72062253952026)
--(axis cs:11600,4.10224914550781)
--(axis cs:11500,4.45362663269043)
--(axis cs:11400,4.50425004959106)
--(axis cs:11300,4.97426748275757)
--(axis cs:11200,5.25754308700562)
--(axis cs:11100,5.32016897201538)
--(axis cs:11000,5.45561742782593)
--(axis cs:10900,5.31862878799438)
--(axis cs:10800,5.73125314712524)
--(axis cs:10700,5.41918897628784)
--(axis cs:10600,5.30516004562378)
--(axis cs:10500,5.78970623016357)
--(axis cs:10400,5.549072265625)
--(axis cs:10300,5.19104862213135)
--(axis cs:10200,4.89783048629761)
--(axis cs:10100,5.01844549179077)
--(axis cs:10000,4.59472513198853)
--(axis cs:9900,4.82262182235718)
--(axis cs:9800,4.39368915557861)
--(axis cs:9700,4.33928680419922)
--(axis cs:9600,4.84047365188599)
--(axis cs:9500,4.48266649246216)
--(axis cs:9400,4.56843280792236)
--(axis cs:9300,4.77938652038574)
--(axis cs:9200,5.27684926986694)
--(axis cs:9100,5.19427394866943)
--(axis cs:9000,5.87347459793091)
--(axis cs:8900,6.28353261947632)
--(axis cs:8800,6.26194334030151)
--(axis cs:8700,6.47100353240967)
--(axis cs:8600,6.05547714233398)
--(axis cs:8500,6.39884281158447)
--(axis cs:8400,7.01039218902588)
--(axis cs:8300,7.22368478775024)
--(axis cs:8200,7.04433441162109)
--(axis cs:8100,7.83882284164429)
--(axis cs:8000,7.11802768707275)
--(axis cs:7900,6.52932739257812)
--(axis cs:7800,6.72937250137329)
--(axis cs:7700,6.78148698806763)
--(axis cs:7600,6.71542930603027)
--(axis cs:7500,6.76961517333984)
--(axis cs:7400,6.68923854827881)
--(axis cs:7300,6.94512557983398)
--(axis cs:7200,7.01997518539429)
--(axis cs:7100,6.62769556045532)
--(axis cs:7000,7.03955507278442)
--(axis cs:6900,6.6445779800415)
--(axis cs:6800,6.55258798599243)
--(axis cs:6700,6.53139877319336)
--(axis cs:6600,6.84446811676025)
--(axis cs:6500,6.78482055664062)
--(axis cs:6400,7.48538637161255)
--(axis cs:6300,7.81506061553955)
--(axis cs:6200,8.23427772521973)
--(axis cs:6100,8.15260791778564)
--(axis cs:6000,8.27439594268799)
--(axis cs:5900,8.78911972045898)
--(axis cs:5800,9.48759841918945)
--(axis cs:5700,9.54146194458008)
--(axis cs:5600,9.99423503875732)
--(axis cs:5500,9.70250797271729)
--(axis cs:5400,9.257248878479)
--(axis cs:5300,7.88515615463257)
--(axis cs:5200,9.0504846572876)
--(axis cs:5100,8.72604370117188)
--(axis cs:5000,8.58375263214111)
--(axis cs:4900,9.84212112426758)
--(axis cs:4800,10.8238315582275)
--(axis cs:4700,10.2401218414307)
--(axis cs:4600,10.0807847976685)
--(axis cs:4500,8.62196063995361)
--(axis cs:4400,8.96025657653809)
--(axis cs:4300,9.75087928771973)
--(axis cs:4200,8.8569278717041)
--(axis cs:4100,8.68159484863281)
--(axis cs:4000,9.64551734924316)
--(axis cs:3900,7.8516731262207)
--(axis cs:3800,7.34218692779541)
--(axis cs:3700,7.57635974884033)
--(axis cs:3600,8.10210037231445)
--(axis cs:3500,7.04123401641846)
--(axis cs:3400,6.58416604995728)
--(axis cs:3300,6.11940479278564)
--(axis cs:3200,4.95528507232666)
--(axis cs:3100,3.88849282264709)
--(axis cs:3000,4.70580434799194)
--(axis cs:2900,4.95373296737671)
--(axis cs:2800,4.2487587928772)
--(axis cs:2700,4.43647003173828)
--(axis cs:2600,4.61850214004517)
--(axis cs:2500,4.12643051147461)
--(axis cs:2400,3.53213047981262)
--(axis cs:2300,3.38777780532837)
--(axis cs:2200,3.15801095962524)
--(axis cs:2100,2.46476554870605)
--(axis cs:2000,2.34285092353821)
--(axis cs:1900,1.62428593635559)
--(axis cs:1800,1.25765812397003)
--(axis cs:1700,1.38605165481567)
--(axis cs:1600,1.219083070755)
--(axis cs:1500,1.09288311004639)
--(axis cs:1400,0.769291818141937)
--(axis cs:1300,0.79917311668396)
--(axis cs:1200,0.57192051410675)
--(axis cs:1100,0.390252649784088)
--(axis cs:1000,0.118704959750175)
--(axis cs:900,0.0854143053293228)
--(axis cs:800,0.0143444538116455)
--(axis cs:700,0.016373835504055)
--(axis cs:600,0.0186504330486059)
--(axis cs:500,0.0213629752397537)
--(axis cs:400,0.0237089712172747)
--(axis cs:300,0.0260407999157906)
--(axis cs:200,8.40727806091309)
--(axis cs:100,8.419264793396)
--(axis cs:0,8.41387367248535)
--cycle;

\path [fill=white!50.1960784313725!black, fill opacity=0.4, semithick]
(axis cs:0,0.0306430757045746)
--(axis cs:0,0.0231263339519501)
--(axis cs:100,0.0231263302266598)
--(axis cs:200,0.00338825769722462)
--(axis cs:300,0)
--(axis cs:400,0)
--(axis cs:500,0)
--(axis cs:600,0)
--(axis cs:700,0)
--(axis cs:800,0)
--(axis cs:900,0)
--(axis cs:1000,0)
--(axis cs:1100,0)
--(axis cs:1200,0)
--(axis cs:1300,0)
--(axis cs:1400,0)
--(axis cs:1500,0)
--(axis cs:1600,0)
--(axis cs:1700,1.56588976096828e-06)
--(axis cs:1800,3.1724571272207e-06)
--(axis cs:1900,3.1724571272207e-06)
--(axis cs:2000,0.000112820358481258)
--(axis cs:2100,8.82067834027112e-05)
--(axis cs:2200,7.22300610505044e-05)
--(axis cs:2300,1.94787971850019e-05)
--(axis cs:2400,8.87958449311554e-05)
--(axis cs:2500,0.000182356248842552)
--(axis cs:2600,0.000306989531964064)
--(axis cs:2700,0.000302503525745124)
--(axis cs:2800,1.30459666252136e-05)
--(axis cs:2900,5.82337361265672e-06)
--(axis cs:3000,5.8144332797383e-06)
--(axis cs:3100,5.82039365326636e-06)
--(axis cs:3200,2.0828843844356e-05)
--(axis cs:3300,2.64212485490134e-05)
--(axis cs:3400,9.18805599212646e-05)
--(axis cs:3500,0.000110789958853275)
--(axis cs:3600,4.8908590542851e-05)
--(axis cs:3700,0.00094863201957196)
--(axis cs:3800,0.001009761239402)
--(axis cs:3900,0.00104896200355142)
--(axis cs:4000,0.0024506589397788)
--(axis cs:4100,0.00314658577553928)
--(axis cs:4200,0.00347458105534315)
--(axis cs:4300,0.00319546647369862)
--(axis cs:4400,0.00316424574702978)
--(axis cs:4500,0.00714557524770498)
--(axis cs:4600,0.0119987698271871)
--(axis cs:4700,0.0118821710348129)
--(axis cs:4800,0.0131911281496286)
--(axis cs:4900,0.0133456820622087)
--(axis cs:5000,0.00327818980440497)
--(axis cs:5100,0.00317096407525241)
--(axis cs:5200,0.00236369064077735)
--(axis cs:5300,0.00223620235919952)
--(axis cs:5400,0.00132255558855832)
--(axis cs:5500,0.00246542389504611)
--(axis cs:5600,0.00219684233888984)
--(axis cs:5700,0.00213754782453179)
--(axis cs:5800,0.00194246170576662)
--(axis cs:5900,0.00271777180023491)
--(axis cs:6000,0.0035963177215308)
--(axis cs:6100,0.00313019147142768)
--(axis cs:6200,0.00308444094844162)
--(axis cs:6300,0.00359275727532804)
--(axis cs:6400,0.00157132698222995)
--(axis cs:6500,0.00141265976708382)
--(axis cs:6600,0.00134988618083298)
--(axis cs:6700,0.00121315126307309)
--(axis cs:6800,0.000655686832033098)
--(axis cs:6900,0.000920151243917644)
--(axis cs:7000,0.00143891246989369)
--(axis cs:7100,0.00151478894986212)
--(axis cs:7200,0.000719074159860611)
--(axis cs:7300,0.000892358482815325)
--(axis cs:7400,0.000644936983007938)
--(axis cs:7500,0.000911350653041154)
--(axis cs:7600,0.00115555943921208)
--(axis cs:7700,0.00121102214325219)
--(axis cs:7800,0.000859034073073417)
--(axis cs:7900,0.000390279281418771)
--(axis cs:8000,0.000365513551514596)
--(axis cs:8100,0.000537019979674369)
--(axis cs:8200,0.00053558946819976)
--(axis cs:8300,0.000778625137172639)
--(axis cs:8400,0.000749355531297624)
--(axis cs:8500,0.000982785248197615)
--(axis cs:8600,0.000862872577272356)
--(axis cs:8700,0.0010582268005237)
--(axis cs:8800,0.00137609243392944)
--(axis cs:8900,0.00177283282391727)
--(axis cs:9000,0.00162828562315553)
--(axis cs:9100,0.00159947900101542)
--(axis cs:9200,0.0015117364237085)
--(axis cs:9300,0.00127026706468314)
--(axis cs:9400,0.00101182307116687)
--(axis cs:9500,0.000744598684832454)
--(axis cs:9600,0.000785844633355737)
--(axis cs:9700,0.00117454468272626)
--(axis cs:9800,0.00135883805342019)
--(axis cs:9900,0.00137715239543468)
--(axis cs:10000,0.00114104757085443)
--(axis cs:10100,0.00118723465129733)
--(axis cs:10200,0.000624072563368827)
--(axis cs:10300,0.000584291410632432)
--(axis cs:10400,0.000676490366458893)
--(axis cs:10500,0.000428461207775399)
--(axis cs:10600,0.000492548220790923)
--(axis cs:10700,0.000626984518021345)
--(axis cs:10800,0.000534101389348507)
--(axis cs:10900,0.000474438042147085)
--(axis cs:11000,0.000811497797258198)
--(axis cs:11100,0.000749161234125495)
--(axis cs:11200,0.000624201842583716)
--(axis cs:11300,0.000784655567258596)
--(axis cs:11400,0.00103067851159722)
--(axis cs:11500,0.000682958227116615)
--(axis cs:11600,0.000660856545437127)
--(axis cs:11700,0.000593145727179945)
--(axis cs:11800,0.000511708436533809)
--(axis cs:11900,0.000276580336503685)
--(axis cs:12000,0.000406174804084003)
--(axis cs:12100,0.000514661893248558)
--(axis cs:12200,0.00186668639071286)
--(axis cs:12300,0.00206595659255981)
--(axis cs:12400,0.00165327789727598)
--(axis cs:12500,0.00199082773178816)
--(axis cs:12600,0.000628334295470268)
--(axis cs:12700,0.000941379112191498)
--(axis cs:12800,0.000940232130233198)
--(axis cs:12900,0.000790353398770094)
--(axis cs:13000,0.000453878659754992)
--(axis cs:13100,0.000493492814712226)
--(axis cs:13200,0.000401360273826867)
--(axis cs:13300,0.000313533295411617)
--(axis cs:13400,0.000267301395069808)
--(axis cs:13500,0.000303760141832754)
--(axis cs:13600,0.000240279536228627)
--(axis cs:13700,0.000322145235259086)
--(axis cs:13800,0.000351387250702828)
--(axis cs:13900,0.00041383015923202)
--(axis cs:14000,0.000455067143775523)
--(axis cs:14100,0.000467108708107844)
--(axis cs:14200,0.00050036096945405)
--(axis cs:14300,0.000778978108428419)
--(axis cs:14400,0.000757545232772827)
--(axis cs:14500,0.00068353780079633)
--(axis cs:14600,0.000523941591382027)
--(axis cs:14700,0.000588183291256428)
--(axis cs:14800,0.000549827178474516)
--(axis cs:14900,0.000472489977255464)
--(axis cs:15000,0.000554842583369464)
--(axis cs:15100,0.000717753544449806)
--(axis cs:15200,0.000561713124625385)
--(axis cs:15300,0.000371574104065076)
--(axis cs:15400,0.000343527499353513)
--(axis cs:15500,0.000393365626223385)
--(axis cs:15600,0.000342470419127494)
--(axis cs:15700,0.000349378591636196)
--(axis cs:15800,0.000234466788242571)
--(axis cs:15900,0.000353199255187064)
--(axis cs:16000,0.000216448301216587)
--(axis cs:16100,0.000228673685342073)
--(axis cs:16200,0.00043259741505608)
--(axis cs:16300,0.000683778547681868)
--(axis cs:16400,0.000549513089936227)
--(axis cs:16500,0.000457665300928056)
--(axis cs:16600,0.000638294208329171)
--(axis cs:16700,0.000621211540419608)
--(axis cs:16800,0.000504835217725486)
--(axis cs:16900,0.000512643018737435)
--(axis cs:17000,0.000468643673229963)
--(axis cs:17100,0.000401222700020298)
--(axis cs:17200,0.000566810369491577)
--(axis cs:17300,0.000435558147728443)
--(axis cs:17400,0.000510714598931372)
--(axis cs:17500,0.000539803295396268)
--(axis cs:17600,0.000478164030937478)
--(axis cs:17700,0.000323976622894406)
--(axis cs:17800,0.000367301050573587)
--(axis cs:17900,0.000446119112893939)
--(axis cs:18000,0.000352954433765262)
--(axis cs:18100,0.000381519610527903)
--(axis cs:18200,0.000446636695414782)
--(axis cs:18300,0.000484651332953945)
--(axis cs:18400,0.000417876231949776)
--(axis cs:18500,0.00042082933941856)
--(axis cs:18600,0.000271457422059029)
--(axis cs:18700,0.000233244893024676)
--(axis cs:18800,0.000262262299656868)
--(axis cs:18900,0.000411093875300139)
--(axis cs:19000,0.000394359783967957)
--(axis cs:19100,0.000331103801727295)
--(axis cs:19200,0.000337026314809918)
--(axis cs:19300,0.000283943169051781)
--(axis cs:19400,0.000171279913047329)
--(axis cs:19500,0.000237482279771939)
--(axis cs:19600,0.000282644061371684)
--(axis cs:19700,0.000309860508423299)
--(axis cs:19800,0.000291567121166736)
--(axis cs:19900,0.00019612887990661)
--(axis cs:20000,0.000228047501877882)
--(axis cs:20100,0.000378301367163658)
--(axis cs:20200,0.000356118194758892)
--(axis cs:20300,0.000432317901868373)
--(axis cs:20400,0.000396716583054513)
--(axis cs:20500,0.000451327534392476)
--(axis cs:20600,0.000298274244414642)
--(axis cs:20700,0.000231344951316714)
--(axis cs:20800,0.000247871328610927)
--(axis cs:20900,0.000193465384654701)
--(axis cs:21000,6.74217299092561e-05)
--(axis cs:21100,6.26023393124342e-05)
--(axis cs:21200,7.37353402655572e-05)
--(axis cs:21300,4.29153442382812e-06)
--(axis cs:21400,3.18690144922584e-05)
--(axis cs:21500,2.20899819396436e-05)
--(axis cs:21600,6.35610776953399e-05)
--(axis cs:21700,6.05004897806793e-05)
--(axis cs:21800,6.2726714531891e-05)
--(axis cs:21900,4.80856106150895e-05)
--(axis cs:22000,4.03893645852804e-05)
--(axis cs:22100,5.40213659405708e-05)
--(axis cs:22200,3.16277437377721e-05)
--(axis cs:22300,4.29153442382812e-06)
--(axis cs:22400,2.03393865376711e-05)
--(axis cs:22500,2.50051671173424e-05)
--(axis cs:22600,2.29529978241771e-05)
--(axis cs:22700,4.06062754336745e-05)
--(axis cs:22800,6.46154949208722e-05)
--(axis cs:22900,6.3784042140469e-05)
--(axis cs:23000,6.14208547631279e-05)
--(axis cs:23100,6.27589906798676e-05)
--(axis cs:23200,5.7519762776792e-05)
--(axis cs:23300,5.82901848247275e-05)
--(axis cs:23400,3.69577828678302e-05)
--(axis cs:23500,5.90596318943426e-05)
--(axis cs:23600,5.4344956879504e-05)
--(axis cs:23700,5.70487172808498e-05)
--(axis cs:23800,6.39140635030344e-05)
--(axis cs:23900,6.57892669551075e-05)
--(axis cs:24000,6.60006335237995e-05)
--(axis cs:24100,6.56504707876593e-05)
--(axis cs:24200,4.88411460537463e-05)
--(axis cs:24300,5.59390755370259e-05)
--(axis cs:24400,5.84973458899185e-05)
--(axis cs:24500,6.44797692075372e-05)
--(axis cs:24600,6.45109103061259e-05)
--(axis cs:24700,6.00662606302649e-05)
--(axis cs:24800,5.37101295776665e-05)
--(axis cs:24900,5.28728123754263e-05)
--(axis cs:25000,3.83493024855852e-05)
--(axis cs:25100,3.77686519641429e-05)
--(axis cs:25200,6.54003233648837e-05)
--(axis cs:25300,6.13825977779925e-05)
--(axis cs:25400,6.58081698929891e-05)
--(axis cs:25500,6.40425714664161e-05)
--(axis cs:25600,5.96754543948919e-05)
--(axis cs:25700,2.87913135252893e-05)
--(axis cs:25800,3.07034933939576e-05)
--(axis cs:25900,4.68004436697811e-05)
--(axis cs:26000,4.47649508714676e-05)
--(axis cs:26100,6.34065072517842e-05)
--(axis cs:26200,3.69256958947517e-05)
--(axis cs:26300,4.22230150434189e-05)
--(axis cs:26400,6.12229196121916e-05)
--(axis cs:26500,5.34377322765067e-05)
--(axis cs:26600,5.34143036929891e-05)
--(axis cs:26700,5.8580408222042e-05)
--(axis cs:26800,5.83185610594228e-05)
--(axis cs:26900,5.95040619373322e-05)
--(axis cs:27000,5.37692540092394e-05)
--(axis cs:27100,6.27976696705446e-05)
--(axis cs:27200,5.95026358496398e-05)
--(axis cs:27300,6.60377991152927e-05)
--(axis cs:27400,5.81265630898997e-05)
--(axis cs:27500,5.6546414270997e-05)
--(axis cs:27600,5.22584887221456e-05)
--(axis cs:27700,4.96001448482275e-05)
--(axis cs:27800,5.27006632182747e-05)
--(axis cs:27900,4.78716683574021e-05)
--(axis cs:28000,6.60478690406308e-05)
--(axis cs:28100,6.54564355500042e-05)
--(axis cs:28200,6.42421509837732e-05)
--(axis cs:28300,5.70849952055141e-05)
--(axis cs:28400,5.53303543711081e-05)
--(axis cs:28500,5.1965267630294e-05)
--(axis cs:28600,5.83600922254845e-05)
--(axis cs:28700,5.06074575241655e-05)
--(axis cs:28800,4.90575330331922e-05)
--(axis cs:28900,4.96456050314009e-05)
--(axis cs:29000,5.04830095451325e-05)
--(axis cs:29100,5.76744641875848e-05)
--(axis cs:29200,3.72101931134239e-05)
--(axis cs:29300,2.01639923034236e-05)
--(axis cs:29400,3.06696892948821e-05)
--(axis cs:29500,5.35946746822447e-05)
--(axis cs:29600,5.55465085199103e-05)
--(axis cs:29700,6.03445369051769e-05)
--(axis cs:29800,6.60401565255597e-05)
--(axis cs:29900,6.60672376397997e-05)
--(axis cs:30000,6.49206194793805e-05)
--(axis cs:30100,6.46524858893827e-05)
--(axis cs:30200,6.20311184320599e-05)
--(axis cs:30300,6.26942201051861e-05)
--(axis cs:30400,6.15386379649863e-05)
--(axis cs:30500,6.23490050202236e-05)
--(axis cs:30600,6.4222447690554e-05)
--(axis cs:30700,6.5939748310484e-05)
--(axis cs:30800,6.56483753118664e-05)
--(axis cs:30900,5.91143179917708e-05)
--(axis cs:31000,6.08108821325004e-05)
--(axis cs:31100,6.08914560871199e-05)
--(axis cs:31200,5.79154147999361e-05)
--(axis cs:31300,4.2945561290253e-05)
--(axis cs:31400,5.77535975025967e-05)
--(axis cs:31500,5.99377817707136e-05)
--(axis cs:31600,6.12288422416896e-05)
--(axis cs:31700,5.06207725265995e-05)
--(axis cs:31800,5.03953342558816e-05)
--(axis cs:31900,6.24826934654266e-05)
--(axis cs:32000,6.33380404906347e-05)
--(axis cs:32100,6.19651400484145e-05)
--(axis cs:32200,6.27229019301012e-05)
--(axis cs:32300,6.49468856863678e-05)
--(axis cs:32400,5.11507387273014e-05)
--(axis cs:32500,4.60196679341607e-05)
--(axis cs:32600,6.56460324535146e-05)
--(axis cs:32700,6.56132906442508e-05)
--(axis cs:32700,0.000429808569606394)
--(axis cs:32700,0.000429808569606394)
--(axis cs:32600,0.000428798317443579)
--(axis cs:32500,0.000289741234155372)
--(axis cs:32400,0.000296622514724731)
--(axis cs:32300,0.00034842491731979)
--(axis cs:32200,0.000311851501464844)
--(axis cs:32100,0.000302934640785679)
--(axis cs:32000,0.000320005405228585)
--(axis cs:31900,0.000308907037833706)
--(axis cs:31800,0.000296622514724731)
--(axis cs:31700,0.000296622514724731)
--(axis cs:31600,0.000296622514724731)
--(axis cs:31500,0.000296622514724731)
--(axis cs:31400,0.000296622514724731)
--(axis cs:31300,0.000284581969026476)
--(axis cs:31200,0.000296622514724731)
--(axis cs:31100,0.000296622514724731)
--(axis cs:31000,0.000296622514724731)
--(axis cs:30900,0.000296622514724731)
--(axis cs:30800,0.000369119632523507)
--(axis cs:30700,0.000384235376259312)
--(axis cs:30600,0.00045935669913888)
--(axis cs:30500,0.000486422970425338)
--(axis cs:30400,0.000496460183057934)
--(axis cs:30300,0.000481913419207558)
--(axis cs:30200,0.000490444363094866)
--(axis cs:30100,0.000342011451721191)
--(axis cs:30000,0.000347816938301548)
--(axis cs:29900,0.000401794910430908)
--(axis cs:29800,0.000394451606553048)
--(axis cs:29700,0.000296622514724731)
--(axis cs:29600,0.000296622514724731)
--(axis cs:29500,0.000296622514724731)
--(axis cs:29400,0.000269360200036317)
--(axis cs:29300,0.00026055402122438)
--(axis cs:29200,0.000276592385489494)
--(axis cs:29100,0.000296622514724731)
--(axis cs:29000,0.00060199317522347)
--(axis cs:28900,0.000608878443017602)
--(axis cs:28800,0.000613662705291063)
--(axis cs:28700,0.00060096278320998)
--(axis cs:28600,0.000531070225406438)
--(axis cs:28500,0.000296622514724731)
--(axis cs:28400,0.000296622514724731)
--(axis cs:28300,0.000296622514724731)
--(axis cs:28200,0.000334215175826102)
--(axis cs:28100,0.000362265098374337)
--(axis cs:28000,0.000395798677345738)
--(axis cs:27900,0.000623193220235407)
--(axis cs:27800,0.0005832928000018)
--(axis cs:27700,0.000609249749686569)
--(axis cs:27600,0.000587080779951066)
--(axis cs:27500,0.00054873077897355)
--(axis cs:27400,0.000296622514724731)
--(axis cs:27300,0.000394082075217739)
--(axis cs:27200,0.000296622514724731)
--(axis cs:27100,0.000312793243210763)
--(axis cs:27000,0.000296622514724731)
--(axis cs:26900,0.000296622514724731)
--(axis cs:26800,0.000296622514724731)
--(axis cs:26700,0.000296622514724731)
--(axis cs:26600,0.000296622514724731)
--(axis cs:26500,0.000296622514724731)
--(axis cs:26400,0.000296622514724731)
--(axis cs:26300,0.000283468660200015)
--(axis cs:26200,0.000276241102255881)
--(axis cs:26100,0.000472029991215095)
--(axis cs:26000,0.000647519191261381)
--(axis cs:25900,0.00063167919870466)
--(axis cs:25800,0.000750041857827455)
--(axis cs:25700,0.000763342482969165)
--(axis cs:25600,0.000517452484928071)
--(axis cs:25500,0.000330781942466274)
--(axis cs:25400,0.000423160498030484)
--(axis cs:25300,0.000296723854262382)
--(axis cs:25200,0.000360488891601562)
--(axis cs:25100,0.000699751428328454)
--(axis cs:25000,0.000695522932801396)
--(axis cs:24900,0.00058180937776342)
--(axis cs:24800,0.000574518868234009)
--(axis cs:24700,0.000513239065185189)
--(axis cs:24600,0.000454363413155079)
--(axis cs:24500,0.000454919063486159)
--(axis cs:24400,0.000529685232322663)
--(axis cs:24300,0.000554416445083916)
--(axis cs:24200,0.000615412835031748)
--(axis cs:24100,0.000369203102309257)
--(axis cs:24000,0.000389480584999546)
--(axis cs:23900,0.000375318515580148)
--(axis cs:23800,0.000328671943861991)
--(axis cs:23700,0.000296622514724731)
--(axis cs:23600,0.000296622514724731)
--(axis cs:23500,0.000296622514724731)
--(axis cs:23400,0.000276280508842319)
--(axis cs:23300,0.000296622514724731)
--(axis cs:23200,0.000296622514724731)
--(axis cs:23100,0.000312304502585903)
--(axis cs:23000,0.000297117221634835)
--(axis cs:22900,0.000326609617331997)
--(axis cs:22800,0.000341260427376255)
--(axis cs:22700,0.000678921118378639)
--(axis cs:22600,0.000803314382210374)
--(axis cs:22500,0.000789365149103105)
--(axis cs:22400,0.000820940418634564)
--(axis cs:22300,0.00108089949935675)
--(axis cs:22200,0.000743570388294756)
--(axis cs:22100,0.0005717757740058)
--(axis cs:22000,0.000680528813973069)
--(axis cs:21900,0.000621485174633563)
--(axis cs:21800,0.000311899173539132)
--(axis cs:21700,0.000296622514724731)
--(axis cs:21600,0.000360614067176357)
--(axis cs:21500,0.000295634556096047)
--(axis cs:21400,0.00038749334635213)
--(axis cs:21300,0.000431094085797668)
--(axis cs:21200,0.000564546906389296)
--(axis cs:21100,0.000764197495300323)
--(axis cs:21000,0.00084747385699302)
--(axis cs:20900,0.000939193763770163)
--(axis cs:20800,0.00085969822248444)
--(axis cs:20700,0.000763381132856011)
--(axis cs:20600,0.000505784526467323)
--(axis cs:20500,0.000552331213839352)
--(axis cs:20400,0.000587330316193402)
--(axis cs:20300,0.000609409820754081)
--(axis cs:20200,0.00058870913926512)
--(axis cs:20100,0.000691056251525879)
--(axis cs:20000,0.000680454424582422)
--(axis cs:19900,0.000585872097872198)
--(axis cs:19800,0.000657883239910007)
--(axis cs:19700,0.000681118399370462)
--(axis cs:19600,0.000626231369096786)
--(axis cs:19500,0.00055654050083831)
--(axis cs:19400,0.000800590612925589)
--(axis cs:19300,0.00083296443335712)
--(axis cs:19200,0.00098073307890445)
--(axis cs:19100,0.00107223936356604)
--(axis cs:19000,0.00111384829506278)
--(axis cs:18900,0.000817757856566459)
--(axis cs:18800,0.00056940910872072)
--(axis cs:18700,0.000532862497493625)
--(axis cs:18600,0.000586670299526304)
--(axis cs:18500,0.000433194625657052)
--(axis cs:18400,0.00109824188984931)
--(axis cs:18300,0.00133301073219627)
--(axis cs:18200,0.00139070826116949)
--(axis cs:18100,0.00125109124928713)
--(axis cs:18000,0.00129413651302457)
--(axis cs:17900,0.00144243822433054)
--(axis cs:17800,0.00143080821726471)
--(axis cs:17700,0.00127321726176888)
--(axis cs:17600,0.00129726529121399)
--(axis cs:17500,0.00138112728018314)
--(axis cs:17400,0.000745803117752075)
--(axis cs:17300,0.000646996486466378)
--(axis cs:17200,0.000789068173617125)
--(axis cs:17100,0.000868092523887753)
--(axis cs:17000,0.00080181349767372)
--(axis cs:16900,0.000768876052461565)
--(axis cs:16800,0.000770672399085015)
--(axis cs:16700,0.000682532670907676)
--(axis cs:16600,0.000894022348802537)
--(axis cs:16500,0.000839029671624303)
--(axis cs:16400,0.000665177183691412)
--(axis cs:16300,0.00100823643151671)
--(axis cs:16200,0.00103776156902313)
--(axis cs:16100,0.0011181925656274)
--(axis cs:16000,0.00206673704087734)
--(axis cs:15900,0.00188990391325206)
--(axis cs:15800,0.00145033316221088)
--(axis cs:15700,0.00137086154427379)
--(axis cs:15600,0.00147497223224491)
--(axis cs:15500,0.000702688354067504)
--(axis cs:15400,0.00086618063505739)
--(axis cs:15300,0.00109796668402851)
--(axis cs:15200,0.00104960205499083)
--(axis cs:15100,0.000806992873549461)
--(axis cs:15000,0.000869799812790006)
--(axis cs:14900,0.000799063825979829)
--(axis cs:14800,0.00118718715384603)
--(axis cs:14700,0.00101103784982115)
--(axis cs:14600,0.0011989347403869)
--(axis cs:14500,0.00120780104771256)
--(axis cs:14400,0.00131765019614249)
--(axis cs:14300,0.001236826996319)
--(axis cs:14200,0.00134775647893548)
--(axis cs:14100,0.00122826592996716)
--(axis cs:14000,0.000950384128373116)
--(axis cs:13900,0.000829899334348738)
--(axis cs:13800,0.000449379731435329)
--(axis cs:13700,0.000478802161524072)
--(axis cs:13600,0.000404360587708652)
--(axis cs:13500,0.000473129737656564)
--(axis cs:13400,0.000607198453508317)
--(axis cs:13300,0.000439059745986015)
--(axis cs:13200,0.000806813884992152)
--(axis cs:13100,0.00105686776805669)
--(axis cs:13000,0.00129044719506055)
--(axis cs:12900,0.00176306581124663)
--(axis cs:12800,0.00174810038879514)
--(axis cs:12700,0.00156978366430849)
--(axis cs:12600,0.00291052460670471)
--(axis cs:12500,0.00472676288336515)
--(axis cs:12400,0.00468807620927691)
--(axis cs:12300,0.00466108880937099)
--(axis cs:12200,0.00496246619150043)
--(axis cs:12100,0.00497586792334914)
--(axis cs:12000,0.0012787461746484)
--(axis cs:11900,0.00130064610857517)
--(axis cs:11800,0.000835507526062429)
--(axis cs:11700,0.00111468625254929)
--(axis cs:11600,0.000798213470261544)
--(axis cs:11500,0.00133719807490706)
--(axis cs:11400,0.00163503887597471)
--(axis cs:11300,0.0016118228668347)
--(axis cs:11200,0.0012613475555554)
--(axis cs:11100,0.00156088452786207)
--(axis cs:11000,0.00144863489549607)
--(axis cs:10900,0.000958719872869551)
--(axis cs:10800,0.00117983424570411)
--(axis cs:10700,0.00127160223200917)
--(axis cs:10600,0.00116684508975595)
--(axis cs:10500,0.000901373918168247)
--(axis cs:10400,0.000774584710597992)
--(axis cs:10300,0.00105199520476162)
--(axis cs:10200,0.00169135432224721)
--(axis cs:10100,0.00166051986161619)
--(axis cs:10000,0.00183544750325382)
--(axis cs:9900,0.00182968482840806)
--(axis cs:9800,0.00323178456164896)
--(axis cs:9700,0.00322102359496057)
--(axis cs:9600,0.00299980537965894)
--(axis cs:9500,0.00388824776746333)
--(axis cs:9400,0.00332495500333607)
--(axis cs:9300,0.00262635061517358)
--(axis cs:9200,0.00260999612510204)
--(axis cs:9100,0.0026292959228158)
--(axis cs:9000,0.00181044987402856)
--(axis cs:8900,0.00223683612421155)
--(axis cs:8800,0.00345804309472442)
--(axis cs:8700,0.00346140749752522)
--(axis cs:8600,0.00394976418465376)
--(axis cs:8500,0.00425735302269459)
--(axis cs:8400,0.00412781909108162)
--(axis cs:8300,0.00237380480393767)
--(axis cs:8200,0.00297504896298051)
--(axis cs:8100,0.00323183601722121)
--(axis cs:8000,0.00382241583429277)
--(axis cs:7900,0.00399987027049065)
--(axis cs:7800,0.00358116440474987)
--(axis cs:7700,0.0030046715401113)
--(axis cs:7600,0.00225143833085895)
--(axis cs:7500,0.00173270329833031)
--(axis cs:7400,0.0023513447958976)
--(axis cs:7300,0.00242571299895644)
--(axis cs:7200,0.00177385029383004)
--(axis cs:7100,0.00217148056253791)
--(axis cs:7000,0.00331671955063939)
--(axis cs:6900,0.00347181688994169)
--(axis cs:6800,0.00314376223832369)
--(axis cs:6700,0.00362760503776371)
--(axis cs:6600,0.00294733070768416)
--(axis cs:6500,0.00199420447461307)
--(axis cs:6400,0.00280755572021008)
--(axis cs:6300,0.005852778442204)
--(axis cs:6200,0.00725432299077511)
--(axis cs:6100,0.00679267989471555)
--(axis cs:6000,0.00780160585418344)
--(axis cs:5900,0.00955414958298206)
--(axis cs:5800,0.00543675059452653)
--(axis cs:5700,0.009016796015203)
--(axis cs:5600,0.0114225083962083)
--(axis cs:5500,0.0104024764150381)
--(axis cs:5400,0.00875507108867168)
--(axis cs:5300,0.00929964333772659)
--(axis cs:5200,0.00533171836286783)
--(axis cs:5100,0.00453941896557808)
--(axis cs:5000,0.0112622445449233)
--(axis cs:4900,0.0158562194555998)
--(axis cs:4800,0.0153893530368805)
--(axis cs:4700,0.0152548868209124)
--(axis cs:4600,0.0144877852872014)
--(axis cs:4500,0.0147397397086024)
--(axis cs:4400,0.00623001763597131)
--(axis cs:4300,0.00558767002075911)
--(axis cs:4200,0.0054984213784337)
--(axis cs:4100,0.00849147327244282)
--(axis cs:4000,0.00481600174680352)
--(axis cs:3900,0.00465850066393614)
--(axis cs:3800,0.00459417654201388)
--(axis cs:3700,0.00407146476209164)
--(axis cs:3600,0.000885947374626994)
--(axis cs:3500,0.00062057888135314)
--(axis cs:3400,0.000565089634619653)
--(axis cs:3300,0.000492898107040673)
--(axis cs:3200,0.000619693193584681)
--(axis cs:3100,0.000653818831779063)
--(axis cs:3000,0.000663258484564722)
--(axis cs:2900,0.000705189071595669)
--(axis cs:2800,0.0012213122099638)
--(axis cs:2700,0.00110361468978226)
--(axis cs:2600,0.00081557035446167)
--(axis cs:2500,0.000816366053186357)
--(axis cs:2400,0.00174612016417086)
--(axis cs:2300,0.00163894076831639)
--(axis cs:2200,0.00119736674241722)
--(axis cs:2100,0.0011970242485404)
--(axis cs:2000,0.00121557246893644)
--(axis cs:1900,0.000473798660095781)
--(axis cs:1800,0.000473849358968437)
--(axis cs:1700,5.85056550335139e-05)
--(axis cs:1600,5.32619742443785e-05)
--(axis cs:1500,3.74135709080292e-07)
--(axis cs:1400,3.74135709080292e-07)
--(axis cs:1300,0)
--(axis cs:1200,0)
--(axis cs:1100,0)
--(axis cs:1000,0)
--(axis cs:900,0)
--(axis cs:800,0)
--(axis cs:700,0)
--(axis cs:600,0)
--(axis cs:500,0)
--(axis cs:400,0)
--(axis cs:300,0)
--(axis cs:200,0.00881713815033436)
--(axis cs:100,0.0306430608034134)
--(axis cs:0,0.0306430757045746)
--cycle;

\addplot [ultra thick, color0]
table {%
0 8.02285671234131
200 8.01188850402832
300 0.0127649931237102
400 0.0116200773045421
500 0.010469563305378
600 0.00921935867518187
700 0.00822855811566114
800 0.00728759728372097
900 0.0631113722920418
1000 0.0823204144835472
1100 0.271043390035629
1200 0.386493742465973
1300 0.611946046352386
1400 0.572146594524384
1500 0.804482996463776
1600 0.954561531543732
1700 1.02612626552582
1800 1.1938784122467
1900 1.52497792243958
2000 2.00888156890869
2100 2.16211676597595
2200 2.74640417098999
2300 3.08615374565125
2400 3.15682768821716
2500 3.46096873283386
2600 3.97202110290527
2700 3.99569797515869
2800 3.90579962730408
2900 4.45219659805298
3000 4.38059186935425
3100 3.79717826843262
3200 4.46060276031494
3300 5.16678476333618
3400 5.62940692901611
3500 5.83866834640503
3600 6.95056390762329
3700 6.98970651626587
3800 6.95466709136963
3900 7.36237764358521
4000 8.09850406646729
4100 7.6254768371582
4200 7.51403903961182
4300 7.78181838989258
4400 7.91416215896606
4500 8.00523662567139
4600 9.00368595123291
4700 9.23652172088623
4800 9.4207935333252
5000 8.30564594268799
5100 8.07543182373047
5200 8.0482931137085
5300 7.57342767715454
5400 8.63436508178711
5500 8.94951248168945
5600 8.6783561706543
5700 8.45694828033447
5800 9.12291812896729
5900 8.3579626083374
6000 7.97651195526123
6100 7.81741952896118
6200 7.94464015960693
6300 7.11860179901123
6400 6.6705207824707
6500 6.29312562942505
6600 6.34677076339722
6700 6.30088996887207
6900 6.42502450942993
7000 6.38777112960815
7100 6.4030613899231
7200 6.291907787323
7300 6.36771774291992
7400 6.27017068862915
7500 6.34333992004395
7600 5.8374981880188
7700 5.87226963043213
7800 5.73143148422241
7900 6.20656204223633
8000 6.48850297927856
8100 6.95723485946655
8200 6.38050222396851
8300 6.3445987701416
8500 5.50874757766724
8600 5.3769588470459
8700 5.57762718200684
8800 5.6437463760376
8900 5.81199550628662
9000 5.54354763031006
9100 5.0737738609314
9200 5.1360878944397
9300 4.69922399520874
9400 4.24691152572632
9600 4.41592741012573
9700 4.21882104873657
9800 4.22069501876831
9900 4.3081226348877
10000 4.35789346694946
10100 4.68083906173706
10200 4.81273698806763
10400 5.03342294692993
10500 5.02680635452271
10600 4.81105947494507
10700 4.8342490196228
10800 4.90513467788696
10900 4.82419490814209
11000 5.16555070877075
11100 4.93984079360962
11300 4.57365751266479
11400 4.20561122894287
11500 4.00507783889771
11600 4.00209188461304
11800 4.55427646636963
11900 4.68771934509277
12000 4.68807744979858
12100 4.59658622741699
12200 4.34490537643433
12300 4.06560468673706
12400 4.01132822036743
12500 3.97171258926392
12600 4.0576000213623
12700 3.978187084198
12800 4.0494065284729
13000 3.81913685798645
13100 3.86444520950317
13200 4.10762071609497
13300 3.99516606330872
13400 4.06655979156494
13500 3.86351728439331
13600 3.73480677604675
13700 3.54323697090149
13800 3.57127714157104
13900 3.67723369598389
14000 3.83620977401733
14100 3.66484355926514
14200 3.63022398948669
14400 3.37823867797852
14500 3.43866372108459
14600 3.48554658889771
14700 3.44660234451294
14800 3.55173397064209
14900 3.55396342277527
15000 3.28070092201233
15100 3.35397934913635
15200 3.33599424362183
15300 3.25266146659851
15400 3.19286227226257
15500 3.3028724193573
15600 3.24873089790344
15700 3.00797080993652
15800 2.96761918067932
15900 2.99080348014832
16000 3.10087513923645
16100 3.14485287666321
16200 3.2868447303772
16300 3.55244183540344
16400 3.49924349784851
16500 3.42398285865784
16600 3.46071028709412
16700 3.37460112571716
16800 3.16508436203003
16900 3.3100950717926
17000 3.27555322647095
17100 3.27390098571777
17200 3.43659639358521
17300 3.45109057426453
17400 3.35565519332886
17500 3.31242275238037
17600 3.42518711090088
17700 3.26439547538757
17800 3.25684428215027
17900 3.18035864830017
18000 3.28793478012085
18100 3.0262086391449
18200 3.0124351978302
18300 3.04627728462219
18400 3.04768896102905
18500 2.95286083221436
18600 2.99692821502686
18700 3.10954618453979
18800 3.13004970550537
18900 3.11223936080933
19000 3.1609411239624
19100 3.16083979606628
19200 3.0992431640625
19300 3.05238389968872
19400 3.04624032974243
19500 3.09570693969727
19600 3.53594541549683
19700 3.57744526863098
19800 3.5685715675354
19900 3.62050771713257
20000 3.55332827568054
20100 3.05853652954102
20200 3.0525598526001
20300 2.98433804512024
20400 2.93479442596436
20500 2.86130833625793
20600 2.83131527900696
20700 2.92368102073669
20800 3.00190854072571
20900 2.90149736404419
21000 2.7432541847229
21100 2.96304559707642
21200 2.86033153533936
21300 2.88781356811523
21400 2.99364852905273
21500 3.04029512405396
21600 3.00837063789368
21700 3.01662135124207
21800 2.83780884742737
22000 3.09070611000061
22100 2.99976444244385
22200 2.94683027267456
22300 3.03568124771118
22400 2.80984306335449
22500 2.67645668983459
22600 2.65469980239868
22700 2.62380743026733
22800 2.55384135246277
22900 2.60882973670959
23000 2.7046103477478
23100 2.67352700233459
23200 2.76914072036743
23300 2.82233452796936
23400 2.82621216773987
23500 2.87126493453979
23700 2.87418627738953
23800 2.81350898742676
23900 2.83924961090088
24000 2.74572801589966
24100 2.82126402854919
24300 2.82070350646973
24400 2.73783349990845
24500 2.78154277801514
24600 2.73286890983582
24700 2.65618515014648
24800 2.68862295150757
24900 2.77013278007507
25000 2.78116869926453
25100 2.70641279220581
25200 2.70181441307068
25300 2.72346186637878
25400 2.65816259384155
25600 2.73214507102966
25700 2.80267786979675
25800 2.72473978996277
25900 2.79856824874878
26000 2.69904732704163
26100 2.74163413047791
26200 2.6294960975647
26300 2.65742564201355
26400 2.69572377204895
26500 2.75500106811523
26600 2.67778754234314
26700 2.80546879768372
26800 2.80454087257385
26900 2.67153382301331
27000 2.61150717735291
27100 2.60992836952209
27200 2.40514326095581
27300 2.45013070106506
27400 2.43067240715027
27600 2.51282548904419
27700 2.58704447746277
27800 2.60462236404419
27900 2.69109725952148
28000 2.62236309051514
28100 2.65769052505493
28200 2.67240357398987
28300 2.67263174057007
28400 2.62760424613953
28500 2.65944838523865
28700 2.67246079444885
28800 2.57903671264648
28900 2.53594589233398
29000 2.63609981536865
29100 2.59337568283081
29200 2.52261543273926
29400 2.66378593444824
29500 2.57744932174683
29600 2.67221665382385
29700 2.75472807884216
29800 2.7459557056427
29900 2.69434404373169
30000 2.70751976966858
30100 2.73370766639709
30200 2.66475415229797
30300 2.62080097198486
30400 2.66865205764771
30500 2.68695497512817
30600 2.50160312652588
30700 2.57491850852966
30800 2.58745908737183
30900 2.56474614143372
31000 2.51649570465088
31100 2.55054521560669
31200 2.4798743724823
31300 2.54419755935669
};
\addplot [ultra thick, white!40.2745098039216!black]
table {%
0 0.0268847029656172
100 0.0268846955150366
200 0.00610269932076335
nan nan
1400 1.54972013888255e-07
1500 1.54972013888255e-07
1600 2.21977625187719e-05
1700 3.00357660307782e-05
1800 0.000203554300242104
1900 0.000203399366000667
2000 0.000664196559228003
2100 0.000642615545075387
2200 0.000634798547253013
2300 0.000700054515618831
2400 0.000917457917239517
2500 0.000513201928697526
2600 0.000565209134947509
2700 0.000703059020452201
2800 0.00055936211720109
2900 0.00034209992736578
3000 0.000331256742356345
3100 0.000301200110698119
3200 0.000287021131953225
3300 0.000236117368331179
3400 0.000298633269267157
3500 0.000365684478310868
3600 0.000466565281385556
3700 0.00251004821620882
3800 0.00280196871608496
3900 0.00285373139195144
4000 0.00382519024424255
4100 0.00581903010606766
4200 0.00465607549995184
4300 0.0045601730234921
4400 0.00482929963618517
4500 0.011493188329041
4600 0.0131754269823432
4700 0.0135685270652175
4800 0.0142262782901525
4900 0.0146009512245655
5000 0.00723568117246032
5100 0.00383315328508615
5200 0.00382903730496764
5300 0.00532755767926574
5400 0.00469263503327966
5500 0.00575459841638803
5600 0.00620127096772194
5700 0.00502439634874463
5800 0.00367808970622718
5900 0.00613596057519317
6000 0.00552066043019295
6100 0.00489796372130513
6200 0.00516938045620918
6300 0.0047227693721652
6400 0.00218944088555872
6500 0.00170903571415693
6600 0.00214860774576664
6700 0.00233749183826149
6800 0.00177851272746921
6900 0.00219598459079862
7000 0.00237781601026654
7100 0.00186251744162291
7200 0.00124646199401468
7300 0.00165903591550887
7400 0.00149814074393362
7500 0.00132202717941254
7600 0.00170349888503551
7700 0.0021078463178128
7900 0.00202075252309442
8000 0.00201718253083527
8100 0.00179734430275857
8200 0.00167857413180172
8300 0.00157621479593217
8400 0.00239862804301083
8500 0.00246334099210799
8700 0.00217081094160676
8800 0.0023390231654048
8900 0.00198206841014326
9000 0.00171642517670989
9100 0.00211438746191561
9200 0.00206086575053632
9300 0.00194830901455134
9400 0.00216838950291276
9500 0.00231642299331725
9600 0.00189282547216862
9700 0.00219778390601277
9800 0.00229531084187329
9900 0.00160341849550605
10000 0.00148849666584283
10100 0.00145295029506087
10200 0.00114528916310519
10300 0.000818143365904689
10400 0.000725537480320781
10500 0.000664917461108416
10600 0.000829696655273438
10700 0.000949293549638242
10800 0.000856967933941633
10900 0.000716579204890877
11000 0.00113006634637713
11100 0.00115502288099378
11200 0.000955913681536913
11300 0.00125864939764142
11400 0.00138044147752225
11600 0.00074049411341548
11700 0.000853915873449296
11800 0.000673608097713441
11900 0.000788612989708781
12000 0.000905076507478952
12100 0.00274526537396014
12200 0.00323062739335001
12300 0.00324807642027736
12400 0.00311931385658681
12500 0.00335879577323794
12600 0.00171405216678977
12700 0.00125861004926264
12800 0.00134416634682566
12900 0.00127670983783901
13000 0.000872162752784789
13100 0.000775180116761476
13200 0.00060408707940951
13300 0.000380297453375533
13400 0.000452913896879181
13500 0.000389941415050998
13600 0.0003223201201763
13700 0.000395236536860466
13800 0.000399585493141785
13900 0.000625393760856241
14100 0.000847687479108572
14300 0.00100790231954306
14400 0.00101918180007488
14500 0.000945669191423804
14600 0.000861438049469143
14700 0.000820328656118363
14800 0.00086850713705644
14900 0.000635776785202324
15000 0.000712321256287396
15200 0.000814586703199893
15300 0.000734770263079554
15400 0.000612974225077778
15500 0.000548026990145445
15600 0.00087379600154236
15700 0.000787369324825704
15800 0.000753086933400482
15900 0.00102836079895496
16000 0.00105289230123162
16100 0.000673433183692396
16200 0.000735179404728115
16300 0.000837415456771851
16400 0.000598740472923964
16500 0.00064834754448384
16600 0.000758272595703602
16700 0.000647765526082367
16800 0.000637753983028233
16900 0.000647423847112805
17000 0.000635228701867163
17100 0.000601404870394617
17200 0.000677939329762012
17300 0.00054673757404089
17400 0.000643368461169302
17500 0.000960465404205024
17600 0.000914510223083198
17700 0.000798596767708659
17800 0.000899054750334471
17900 0.000944278901442885
18000 0.000823545444291085
18100 0.000816305284388363
18200 0.000918672594707459
18300 0.000894757220521569
18400 0.00074328196933493
18500 0.000427554012276232
18600 0.000425680365879089
18700 0.000381495628971606
18800 0.000422847253503278
18900 0.000618425896391273
19000 0.000754104228690267
19100 0.000691882858518511
19200 0.000658879755064845
19300 0.000558453903067857
19400 0.000483610201627016
19500 0.000410616339650005
19600 0.000454437627922744
19700 0.000495489570312202
19800 0.000474725296953693
19900 0.00039100056164898
20000 0.000454251043265685
20100 0.000539151893462986
20200 0.000491074693854898
20300 0.000533568905666471
20400 0.000482579052913934
20500 0.000501829315908253
20600 0.000402029399992898
20700 0.000497362925671041
20800 0.000553784717340022
20900 0.00056632945779711
21000 0.000457447749795392
21100 0.000413399975514039
21200 0.000319141137879342
21300 0.000213207793422043
21400 0.000209681165870279
21500 0.00015886225446593
21600 0.000217026521568187
21700 0.000196351655176841
21800 0.000204271083930507
21900 0.00033478534896858
22000 0.000360459031071514
22100 0.000312898540869355
22200 0.000387599051464349
22300 0.00053043570369482
22400 0.000420639873482287
22500 0.000407185201765969
22600 0.000413133617257699
22700 0.000359763740561903
22800 0.000214058178244159
22900 0.000209174482733943
23000 0.000199343805434182
23100 0.000204406140255742
23200 0.000188332793186419
23300 0.000190216320334002
23400 0.000156619178596884
23500 0.000192214982234873
23600 0.00018151402764488
23700 0.000187232115422376
23800 0.000209861973416992
23900 0.000225410884013399
24000 0.000230131539865397
24100 0.000223372422624379
24200 0.000332126946887001
24300 0.000305177731206641
24400 0.000294091354589909
24500 0.000259699387243018
24600 0.000259437190834433
24700 0.000286652648355812
24800 0.000314114469802007
24900 0.000317341124173254
25000 0.00036693611764349
25100 0.000368760025594383
25200 0.000220467671169899
25300 0.000199212634470314
25400 0.000244484341237694
25500 0.00021056535479147
25700 0.000396066898247227
25800 0.000390372588299215
25900 0.000339239835739136
26000 0.000346142100170255
26100 0.000267718191025779
26200 0.000156583424541168
26300 0.000162845870363526
26400 0.000198672234546393
26500 0.000179781505721621
26600 0.000179737791768275
26700 0.000190955397556536
26800 0.000190287857549265
26900 0.00019343095482327
27000 0.000180405360879377
27100 0.00020456915081013
27200 0.000193427025806159
27300 0.000231665311730467
27400 0.000189806989510544
27500 0.000302638625726104
27600 0.000319669634336606
27700 0.000329424918163568
27800 0.000317996658850461
27900 0.000335532356984913
28000 0.000232237565796822
28100 0.000221059715840966
28200 0.000211709731956944
28300 0.000187315599760041
28400 0.00018349286983721
28500 0.000177127119968645
28600 0.00029471522429958
28700 0.000325785193126649
28800 0.000331360060954466
29000 0.000326237990520895
29100 0.000188702368177474
29200 0.000156901282025501
29300 0.000140358970384113
29400 0.000150014966493472
29500 0.000180075556272641
29600 0.000183941883733496
29700 0.000195874818018638
29800 0.000231788581004366
29900 0.000234236285905354
30000 0.000216243613976985
30100 0.000214308514841832
30200 0.000276237726211548
30300 0.000272303877864033
30400 0.000278999475995079
30500 0.000274385965894908
30600 0.000261789537034929
30700 0.000228383141802624
30800 0.000223344584810548
30900 0.000192362043890171
31000 0.000197325163753703
31100 0.000197583474800922
31200 0.000189286496606655
31300 0.000163763790624216
31400 0.000188893071026541
31500 0.000194666790775955
31600 0.00019869209791068
31700 0.000174850240000524
31800 0.000174480694113299
31900 0.00020327368110884
32000 0.000206973098102026
32100 0.000201282848138362
32200 0.000204255164135247
32300 0.000216446351259947
32400 0.000175732391653582
32500 0.000167880454682745
32600 0.000247222167672589
32700 0.00024771096650511
};
