# Supplementary material for: Neural Networks with Physics-Informed Architectures and Constraints for Dynamical Systems Modeling
Source: arXiv:2109.06407 source file (2022-12-12)
Supplement: Supplementary file 3 [file train_test_loss_data.tex]

\definecolor{color0}{rgb}{1,0,1}

\path [fill=red, fill opacity=0.4, ultra thick]
(axis cs:0,0.0544604100286961)
--(axis cs:0,0.0544556342065334)
--(axis cs:100,0.054262787103653)
--(axis cs:200,0.0538671836256981)
--(axis cs:300,0.053299356251955)
--(axis cs:400,0.0524099729955196)
--(axis cs:500,0.0512915588915348)
--(axis cs:600,0.0498612597584724)
--(axis cs:700,0.048358503729105)
--(axis cs:800,0.0468810349702835)
--(axis cs:900,0.0455310307443142)
--(axis cs:1000,0.0442750826478004)
--(axis cs:1100,0.0432932898402214)
--(axis cs:1200,0.0424183383584023)
--(axis cs:1300,0.0415273271501064)
--(axis cs:1400,0.0406446345150471)
--(axis cs:1500,0.0398341491818428)
--(axis cs:1600,0.0391616970300674)
--(axis cs:1700,0.0385490283370018)
--(axis cs:1800,0.0380383096635342)
--(axis cs:1900,0.0376506596803665)
--(axis cs:2000,0.0372785739600658)
--(axis cs:2100,0.0367969311773777)
--(axis cs:2200,0.0362707525491714)
--(axis cs:2300,0.0357639789581299)
--(axis cs:2400,0.0351036749780178)
--(axis cs:2500,0.0343529209494591)
--(axis cs:2600,0.0336244218051434)
--(axis cs:2700,0.0329313911497593)
--(axis cs:2800,0.0321676023304462)
--(axis cs:2900,0.0315744169056416)
--(axis cs:3000,0.0310739763081074)
--(axis cs:3100,0.0305582359433174)
--(axis cs:3200,0.0300906151533127)
--(axis cs:3300,0.0296397153288126)
--(axis cs:3400,0.0291373878717422)
--(axis cs:3500,0.0286697149276733)
--(axis cs:3600,0.0282844062894583)
--(axis cs:3700,0.0278869438916445)
--(axis cs:3800,0.0275154709815979)
--(axis cs:3900,0.0271617714315653)
--(axis cs:4000,0.0268238559365273)
--(axis cs:4100,0.0264994949102402)
--(axis cs:4200,0.0262080077081919)
--(axis cs:4300,0.0259157679975033)
--(axis cs:4400,0.0256689712405205)
--(axis cs:4500,0.025422491133213)
--(axis cs:4600,0.0251766443252563)
--(axis cs:4700,0.0248826667666435)
--(axis cs:4800,0.0246551185846329)
--(axis cs:4900,0.0243975836783648)
--(axis cs:5000,0.02416424266994)
--(axis cs:5100,0.0239365864545107)
--(axis cs:5200,0.0237438529729843)
--(axis cs:5300,0.0235683433711529)
--(axis cs:5400,0.0233610551804304)
--(axis cs:5500,0.0231598597019911)
--(axis cs:5600,0.023010179400444)
--(axis cs:5700,0.0228530038148165)
--(axis cs:5800,0.0226530227810144)
--(axis cs:5900,0.0224942173808813)
--(axis cs:6000,0.0224036760628223)
--(axis cs:6100,0.022212190553546)
--(axis cs:6200,0.0220252610743046)
--(axis cs:6300,0.0218626577407122)
--(axis cs:6400,0.0217299945652485)
--(axis cs:6500,0.0215557813644409)
--(axis cs:6600,0.0214070416986942)
--(axis cs:6700,0.0212934091687202)
--(axis cs:6800,0.0211514942348003)
--(axis cs:6900,0.0209446866065264)
--(axis cs:7000,0.0208285804837942)
--(axis cs:7100,0.0207280609756708)
--(axis cs:7200,0.0205901581794024)
--(axis cs:7300,0.0204629115760326)
--(axis cs:7400,0.0203637108206749)
--(axis cs:7500,0.0202481839805841)
--(axis cs:7600,0.0201098583638668)
--(axis cs:7700,0.0200173370540142)
--(axis cs:7800,0.0199753753840923)
--(axis cs:7900,0.0198731906712055)
--(axis cs:8000,0.0197667293250561)
--(axis cs:8100,0.019667761400342)
--(axis cs:8200,0.0195592604577541)
--(axis cs:8300,0.0194630138576031)
--(axis cs:8400,0.0193438455462456)
--(axis cs:8500,0.0192207656800747)
--(axis cs:8600,0.019170131534338)
--(axis cs:8700,0.0191291328519583)
--(axis cs:8800,0.0189835410565138)
--(axis cs:8900,0.0188969131559134)
--(axis cs:9000,0.01880769059062)
--(axis cs:9100,0.0187026020139456)
--(axis cs:9200,0.0185937248170376)
--(axis cs:9300,0.0185507107526064)
--(axis cs:9400,0.0184898860752583)
--(axis cs:9500,0.0184556003659964)
--(axis cs:9600,0.0183398947119713)
--(axis cs:9700,0.0182806253433228)
--(axis cs:9800,0.0181940011680126)
--(axis cs:9900,0.0180638488382101)
--(axis cs:10000,0.0179491955786943)
--(axis cs:10100,0.017841188237071)
--(axis cs:10200,0.0176926981657743)
--(axis cs:10300,0.0175967868417501)
--(axis cs:10400,0.0175317618995905)
--(axis cs:10500,0.0174021758139133)
--(axis cs:10600,0.0173880644142628)
--(axis cs:10700,0.0173646006733179)
--(axis cs:10800,0.0172961968928576)
--(axis cs:10900,0.0171888209879398)
--(axis cs:11000,0.0171309262514114)
--(axis cs:11100,0.0169935300946236)
--(axis cs:11200,0.0169182326644659)
--(axis cs:11300,0.0168725401163101)
--(axis cs:11400,0.016796637326479)
--(axis cs:11500,0.016751479357481)
--(axis cs:11600,0.0166537445038557)
--(axis cs:11700,0.0165449250489473)
--(axis cs:11800,0.0164618492126465)
--(axis cs:11900,0.0164309032261372)
--(axis cs:12000,0.0163197480142117)
--(axis cs:12100,0.0162341054528952)
--(axis cs:12200,0.0161963142454624)
--(axis cs:12300,0.01618174277246)
--(axis cs:12400,0.0160710904747248)
--(axis cs:12500,0.0160338543355465)
--(axis cs:12600,0.0159660317003727)
--(axis cs:12700,0.015897274017334)
--(axis cs:12800,0.0158267971128225)
--(axis cs:12900,0.0158129688352346)
--(axis cs:13000,0.0157561786472797)
--(axis cs:13100,0.0156633742153645)
--(axis cs:13200,0.0156288873404264)
--(axis cs:13300,0.0155679890885949)
--(axis cs:13400,0.015466975979507)
--(axis cs:13500,0.0153632434085011)
--(axis cs:13600,0.0152401765808463)
--(axis cs:13700,0.0151568911969662)
--(axis cs:13800,0.0151304304599762)
--(axis cs:13900,0.0151357362046838)
--(axis cs:14000,0.0151082603260875)
--(axis cs:14100,0.0150860194116831)
--(axis cs:14200,0.0150018809363246)
--(axis cs:14300,0.0149315511807799)
--(axis cs:14400,0.0148943904787302)
--(axis cs:14500,0.0148011669516563)
--(axis cs:14600,0.0147597370669246)
--(axis cs:14700,0.0147587619721889)
--(axis cs:14800,0.0147669324651361)
--(axis cs:14900,0.0146925253793597)
--(axis cs:15000,0.0146520137786865)
--(axis cs:15100,0.0145990373566747)
--(axis cs:15200,0.0145597932860255)
--(axis cs:15300,0.0145007641986012)
--(axis cs:15400,0.0144540788605809)
--(axis cs:15500,0.0144067155197263)
--(axis cs:15600,0.0143493665382266)
--(axis cs:15700,0.0142554761841893)
--(axis cs:15800,0.0142619730904698)
--(axis cs:15900,0.0142113519832492)
--(axis cs:16000,0.0141738196834922)
--(axis cs:16100,0.0141389593482018)
--(axis cs:16200,0.0141159929335117)
--(axis cs:16300,0.0140097886323929)
--(axis cs:16400,0.0140025140717626)
--(axis cs:16500,0.0139666171744466)
--(axis cs:16600,0.0139559656381607)
--(axis cs:16700,0.0138910617679358)
--(axis cs:16800,0.0138474320992827)
--(axis cs:16900,0.0137956654652953)
--(axis cs:17000,0.0137717258185148)
--(axis cs:17100,0.0136962793767452)
--(axis cs:17200,0.01372582744807)
--(axis cs:17300,0.0136330248787999)
--(axis cs:17400,0.0135961640626192)
--(axis cs:17500,0.0135835250839591)
--(axis cs:17600,0.0135486600920558)
--(axis cs:17700,0.0134784579277039)
--(axis cs:17800,0.0135223409160972)
--(axis cs:17900,0.0134405894204974)
--(axis cs:18000,0.0133964847773314)
--(axis cs:18100,0.0133821414783597)
--(axis cs:18200,0.0133144287392497)
--(axis cs:18300,0.0132715748623013)
--(axis cs:18400,0.01326759532094)
--(axis cs:18500,0.013171287253499)
--(axis cs:18600,0.0131280375644565)
--(axis cs:18700,0.0131670320406556)
--(axis cs:18800,0.0131124742329121)
--(axis cs:18900,0.0130656994879246)
--(axis cs:19000,0.0130478031933308)
--(axis cs:19100,0.0129994284361601)
--(axis cs:19200,0.0129510853439569)
--(axis cs:19300,0.0129520930349827)
--(axis cs:19400,0.0129182981327176)
--(axis cs:19500,0.012884110212326)
--(axis cs:19600,0.0128494678065181)
--(axis cs:19700,0.0128425601869822)
--(axis cs:19800,0.0128195835277438)
--(axis cs:19900,0.0128211388364434)
--(axis cs:20000,0.0127958301454782)
--(axis cs:20100,0.0128185274079442)
--(axis cs:20200,0.0127081871032715)
--(axis cs:20300,0.0126992203295231)
--(axis cs:20400,0.0126626091077924)
--(axis cs:20500,0.0126040503382683)
--(axis cs:20600,0.0125713516026735)
--(axis cs:20700,0.0125728696584702)
--(axis cs:20800,0.0125019447878003)
--(axis cs:20900,0.0124830706045032)
--(axis cs:21000,0.0124933244660497)
--(axis cs:21100,0.0124383922666311)
--(axis cs:21200,0.01238146238029)
--(axis cs:21300,0.0123946191743016)
--(axis cs:21400,0.0123699186369777)
--(axis cs:21500,0.0122704524546862)
--(axis cs:21600,0.0122605636715889)
--(axis cs:21700,0.0122461812570691)
--(axis cs:21800,0.0122376251965761)
--(axis cs:21900,0.0122387958690524)
--(axis cs:22000,0.0122581394389272)
--(axis cs:22100,0.0122813833877444)
--(axis cs:22200,0.0121810473501682)
--(axis cs:22300,0.0121277393773198)
--(axis cs:22400,0.012080860324204)
--(axis cs:22500,0.0120696211233735)
--(axis cs:22600,0.0119963428005576)
--(axis cs:22700,0.0120304087176919)
--(axis cs:22800,0.0120290163904428)
--(axis cs:22900,0.0119633991271257)
--(axis cs:23000,0.0119415419176221)
--(axis cs:23100,0.0119390795007348)
--(axis cs:23200,0.0119160618633032)
--(axis cs:23300,0.0119337383657694)
--(axis cs:23400,0.0119722811505198)
--(axis cs:23500,0.0119769787415862)
--(axis cs:23600,0.0119992168620229)
--(axis cs:23700,0.0119779221713543)
--(axis cs:23800,0.0119130099192262)
--(axis cs:23900,0.0118473377078772)
--(axis cs:24000,0.0118102850392461)
--(axis cs:24100,0.0118188504129648)
--(axis cs:24200,0.011789171025157)
--(axis cs:24300,0.0117522710934281)
--(axis cs:24400,0.011734020896256)
--(axis cs:24500,0.0117339137941599)
--(axis cs:24600,0.0116416933014989)
--(axis cs:24700,0.0116728991270065)
--(axis cs:24800,0.0116539001464844)
--(axis cs:24900,0.0116408346220851)
--(axis cs:25000,0.011630249209702)
--(axis cs:25100,0.0115809440612793)
--(axis cs:25200,0.0115015031769872)
--(axis cs:25300,0.0115537643432617)
--(axis cs:25400,0.0115228649228811)
--(axis cs:25500,0.0115791317075491)
--(axis cs:25600,0.0116032604128122)
--(axis cs:25700,0.0115549089387059)
--(axis cs:25800,0.0115009304136038)
--(axis cs:25900,0.0115269664674997)
--(axis cs:26000,0.0115234274417162)
--(axis cs:26100,0.0115083549171686)
--(axis cs:26100,0.0119591541588306)
--(axis cs:26100,0.0119591541588306)
--(axis cs:26000,0.0119519662111998)
--(axis cs:25900,0.0119433784857392)
--(axis cs:25800,0.011936510913074)
--(axis cs:25700,0.0119388094171882)
--(axis cs:25600,0.0119435833767056)
--(axis cs:25500,0.01193852070719)
--(axis cs:25400,0.0119404662400484)
--(axis cs:25300,0.0119446646422148)
--(axis cs:25200,0.0119415652006865)
--(axis cs:25100,0.0119485789909959)
--(axis cs:25000,0.0119504695758224)
--(axis cs:24900,0.0119587359949946)
--(axis cs:24800,0.0119654517620802)
--(axis cs:24700,0.0119749177247286)
--(axis cs:24600,0.0119625115767121)
--(axis cs:24500,0.0119722979143262)
--(axis cs:24400,0.0119829708710313)
--(axis cs:24300,0.0119849359616637)
--(axis cs:24200,0.0119915865361691)
--(axis cs:24100,0.012009721249342)
--(axis cs:24000,0.0120248794555664)
--(axis cs:23900,0.0120248794555664)
--(axis cs:23800,0.0120350839570165)
--(axis cs:23700,0.0120603926479816)
--(axis cs:23600,0.0120548652485013)
--(axis cs:23500,0.0120907733216882)
--(axis cs:23400,0.0121250152587891)
--(axis cs:23300,0.0121221542358398)
--(axis cs:23200,0.0121251102536917)
--(axis cs:23100,0.0121641159057617)
--(axis cs:23000,0.0121542932465672)
--(axis cs:22900,0.0121618267148733)
--(axis cs:22800,0.0122117958962917)
--(axis cs:22700,0.0122381234541535)
--(axis cs:22600,0.0122654503211379)
--(axis cs:22500,0.0123108746483922)
--(axis cs:22400,0.0123540451750159)
--(axis cs:22300,0.012373742647469)
--(axis cs:22200,0.0124011989682913)
--(axis cs:22100,0.0123969120904803)
--(axis cs:22000,0.0123847965151072)
--(axis cs:21900,0.0123737333342433)
--(axis cs:21800,0.0123680112883449)
--(axis cs:21700,0.012409414164722)
--(axis cs:21600,0.0124173481017351)
--(axis cs:21500,0.0124794915318489)
--(axis cs:21400,0.0125247500836849)
--(axis cs:21300,0.0125572141259909)
--(axis cs:21200,0.0125944409519434)
--(axis cs:21100,0.0126098366454244)
--(axis cs:21000,0.0126252938061953)
--(axis cs:20900,0.0126391900703311)
--(axis cs:20800,0.0126958461478353)
--(axis cs:20700,0.0126935001462698)
--(axis cs:20600,0.0127169769257307)
--(axis cs:20500,0.0127220153808594)
--(axis cs:20400,0.0127724651247263)
--(axis cs:20300,0.0127746928483248)
--(axis cs:20200,0.012856213375926)
--(axis cs:20100,0.0128957824781537)
--(axis cs:20000,0.0129368286579847)
--(axis cs:19900,0.0129301669076085)
--(axis cs:19800,0.0129576679319143)
--(axis cs:19700,0.0129804350435734)
--(axis cs:19600,0.013002417050302)
--(axis cs:19500,0.0130496025085449)
--(axis cs:19400,0.0130996704101562)
--(axis cs:19300,0.0131112094968557)
--(axis cs:19200,0.0131596568971872)
--(axis cs:19100,0.0131754353642464)
--(axis cs:19000,0.0131762679666281)
--(axis cs:18900,0.0131357405334711)
--(axis cs:18800,0.0132158044725657)
--(axis cs:18700,0.0132748605683446)
--(axis cs:18600,0.0133171081542969)
--(axis cs:18500,0.0133959772065282)
--(axis cs:18400,0.0135154724121094)
--(axis cs:18300,0.0135165210813284)
--(axis cs:18200,0.0135496230795979)
--(axis cs:18100,0.0135834449902177)
--(axis cs:18000,0.013546722009778)
--(axis cs:17900,0.013551140204072)
--(axis cs:17800,0.0135754263028502)
--(axis cs:17700,0.0136132687330246)
--(axis cs:17600,0.013629131950438)
--(axis cs:17500,0.0137187084183097)
--(axis cs:17400,0.0137523543089628)
--(axis cs:17300,0.0138086322695017)
--(axis cs:17200,0.0138773918151855)
--(axis cs:17100,0.013890934176743)
--(axis cs:17000,0.0139442440122366)
--(axis cs:16900,0.0139674190431833)
--(axis cs:16800,0.0139827728271484)
--(axis cs:16700,0.013984203338623)
--(axis cs:16600,0.0140440072864294)
--(axis cs:16500,0.0141013832762837)
--(axis cs:16400,0.0140979969874024)
--(axis cs:16300,0.0140926409512758)
--(axis cs:16200,0.0141599653288722)
--(axis cs:16100,0.0141788106411695)
--(axis cs:16000,0.0142360096797347)
--(axis cs:15900,0.0142741044983268)
--(axis cs:15800,0.0143489548936486)
--(axis cs:15700,0.0143393436446786)
--(axis cs:15600,0.0144090326502919)
--(axis cs:15500,0.0144206034019589)
--(axis cs:15400,0.0144716138020158)
--(axis cs:15300,0.0145261259749532)
--(axis cs:15200,0.0146220847964287)
--(axis cs:15100,0.0146814035251737)
--(axis cs:15000,0.0147329801693559)
--(axis cs:14900,0.0147829754278064)
--(axis cs:14800,0.0147873079404235)
--(axis cs:14700,0.014823580160737)
--(axis cs:14600,0.0148650435730815)
--(axis cs:14500,0.0148841384798288)
--(axis cs:14400,0.0149312755092978)
--(axis cs:14300,0.0149893751367927)
--(axis cs:14200,0.0150564378127456)
--(axis cs:14100,0.0151063445955515)
--(axis cs:14000,0.0151844741776586)
--(axis cs:13900,0.0151990409940481)
--(axis cs:13800,0.0152580263093114)
--(axis cs:13700,0.0153612140566111)
--(axis cs:13600,0.0154139995574951)
--(axis cs:13500,0.0154553409665823)
--(axis cs:13400,0.0155464736744761)
--(axis cs:13300,0.0156712662428617)
--(axis cs:13200,0.0157166477292776)
--(axis cs:13100,0.0157855004072189)
--(axis cs:13000,0.015837674960494)
--(axis cs:12900,0.0159115381538868)
--(axis cs:12800,0.0159089341759682)
--(axis cs:12700,0.0159742049872875)
--(axis cs:12600,0.0160312168300152)
--(axis cs:12500,0.0161022655665874)
--(axis cs:12400,0.0161391254514456)
--(axis cs:12300,0.0162517540156841)
--(axis cs:12200,0.0163264274597168)
--(axis cs:12100,0.0163723398000002)
--(axis cs:12000,0.0163866430521011)
--(axis cs:11900,0.0164893697947264)
--(axis cs:11800,0.0165151376277208)
--(axis cs:11700,0.0165887419134378)
--(axis cs:11600,0.0167105849832296)
--(axis cs:11500,0.0167687721550465)
--(axis cs:11400,0.0168108567595482)
--(axis cs:11300,0.0169003717601299)
--(axis cs:11200,0.017009686678648)
--(axis cs:11100,0.0170697756111622)
--(axis cs:11000,0.0171493533998728)
--(axis cs:10900,0.0172552578151226)
--(axis cs:10800,0.0173345487564802)
--(axis cs:10700,0.0174223240464926)
--(axis cs:10600,0.017500139772892)
--(axis cs:10500,0.0175880901515484)
--(axis cs:10400,0.0176221840083599)
--(axis cs:10300,0.017712926492095)
--(axis cs:10200,0.0178159978240728)
--(axis cs:10100,0.0178976263850927)
--(axis cs:10000,0.0179755203425884)
--(axis cs:9900,0.0181197952479124)
--(axis cs:9800,0.0182127691805363)
--(axis cs:9700,0.0182967185974121)
--(axis cs:9600,0.0184009186923504)
--(axis cs:9500,0.0184660032391548)
--(axis cs:9400,0.0185186844319105)
--(axis cs:9300,0.0185909271240234)
--(axis cs:9200,0.0186445564031601)
--(axis cs:9100,0.0187652036547661)
--(axis cs:9000,0.0188222415745258)
--(axis cs:8900,0.0189501885324717)
--(axis cs:8800,0.0190504547208548)
--(axis cs:8700,0.019168246537447)
--(axis cs:8600,0.0192687511444092)
--(axis cs:8500,0.0194073058664799)
--(axis cs:8400,0.0194907188415527)
--(axis cs:8300,0.0195724964141846)
--(axis cs:8200,0.0196840241551399)
--(axis cs:8100,0.0198117177933455)
--(axis cs:8000,0.0199092403054237)
--(axis cs:7900,0.0200229231268167)
--(axis cs:7800,0.0201691929250956)
--(axis cs:7700,0.0202890820801258)
--(axis cs:7600,0.0203902721405029)
--(axis cs:7500,0.0205122027546167)
--(axis cs:7400,0.0206296630203724)
--(axis cs:7300,0.0207211002707481)
--(axis cs:7200,0.0208144392818213)
--(axis cs:7100,0.0209157187491655)
--(axis cs:7000,0.021091153845191)
--(axis cs:6900,0.021198557689786)
--(axis cs:6800,0.0213660709559917)
--(axis cs:6700,0.0215334333479404)
--(axis cs:6600,0.0217078104615211)
--(axis cs:6500,0.0218086428940296)
--(axis cs:6400,0.022011237218976)
--(axis cs:6300,0.02210951782763)
--(axis cs:6200,0.0222347341477871)
--(axis cs:6100,0.0223589893430471)
--(axis cs:6000,0.0225149635225534)
--(axis cs:5900,0.0226863902062178)
--(axis cs:5800,0.0228119697421789)
--(axis cs:5700,0.0228954497724771)
--(axis cs:5600,0.0230821706354618)
--(axis cs:5500,0.0232521779835224)
--(axis cs:5400,0.0234648454934359)
--(axis cs:5300,0.0236899703741074)
--(axis cs:5200,0.0239703170955181)
--(axis cs:5100,0.0241235736757517)
--(axis cs:5000,0.0243731029331684)
--(axis cs:4900,0.0246245861053467)
--(axis cs:4800,0.0248805526643991)
--(axis cs:4700,0.0251049045473337)
--(axis cs:4600,0.0253956317901611)
--(axis cs:4500,0.025603998452425)
--(axis cs:4400,0.0258862152695656)
--(axis cs:4300,0.0261315330862999)
--(axis cs:4200,0.0264453180134296)
--(axis cs:4100,0.026761507615447)
--(axis cs:4000,0.0271197073161602)
--(axis cs:3900,0.0274217370897532)
--(axis cs:3800,0.0277978181838989)
--(axis cs:3700,0.0281137228012085)
--(axis cs:3600,0.0284902099519968)
--(axis cs:3500,0.0289130918681622)
--(axis cs:3400,0.0293532349169254)
--(axis cs:3300,0.029787415638566)
--(axis cs:3200,0.0302085392177105)
--(axis cs:3100,0.0307397656142712)
--(axis cs:3000,0.0312823168933392)
--(axis cs:2900,0.0318399704992771)
--(axis cs:2800,0.0324261635541916)
--(axis cs:2700,0.0331516452133656)
--(axis cs:2600,0.0338584668934345)
--(axis cs:2500,0.0346151106059551)
--(axis cs:2400,0.0353444591164589)
--(axis cs:2300,0.0359557159245014)
--(axis cs:2200,0.0365590080618858)
--(axis cs:2100,0.0370881333947182)
--(axis cs:2000,0.0374819412827492)
--(axis cs:1900,0.0378921739757061)
--(axis cs:1800,0.0383850336074829)
--(axis cs:1700,0.0389180555939674)
--(axis cs:1600,0.0394937992095947)
--(axis cs:1500,0.0401790514588356)
--(axis cs:1400,0.0409828312695026)
--(axis cs:1300,0.0418524779379368)
--(axis cs:1200,0.0427315831184387)
--(axis cs:1100,0.0436275228857994)
--(axis cs:1000,0.044728197157383)
--(axis cs:900,0.0459869876503944)
--(axis cs:800,0.0473590902984142)
--(axis cs:700,0.0488145910203457)
--(axis cs:600,0.0502175539731979)
--(axis cs:500,0.0514817722141743)
--(axis cs:400,0.0525183789432049)
--(axis cs:300,0.0533152855932713)
--(axis cs:200,0.0538861751556396)
--(axis cs:100,0.054278127849102)
--(axis cs:0,0.0544604100286961)
--cycle;

\path [fill=blue, fill opacity=0.4, ultra thick]
(axis cs:0,0.0544335320591927)
--(axis cs:0,0.054432176053524)
--(axis cs:100,0.0542495846748352)
--(axis cs:200,0.0538603290915489)
--(axis cs:300,0.0532742850482464)
--(axis cs:400,0.0523951910436153)
--(axis cs:500,0.0512865595519543)
--(axis cs:600,0.0498741120100021)
--(axis cs:700,0.0483564101159573)
--(axis cs:800,0.0468932762742043)
--(axis cs:900,0.0455633401870728)
--(axis cs:1000,0.0443078018724918)
--(axis cs:1100,0.0432846322655678)
--(axis cs:1200,0.0424345768988132)
--(axis cs:1300,0.0415556877851486)
--(axis cs:1400,0.0406647920608521)
--(axis cs:1500,0.0398291163146496)
--(axis cs:1600,0.0391828306019306)
--(axis cs:1700,0.0385722517967224)
--(axis cs:1800,0.0380669757723808)
--(axis cs:1900,0.0376584194600582)
--(axis cs:2000,0.0372646190226078)
--(axis cs:2100,0.0367649793624878)
--(axis cs:2200,0.0362177900969982)
--(axis cs:2300,0.0356799587607384)
--(axis cs:2400,0.0350086912512779)
--(axis cs:2500,0.034287117421627)
--(axis cs:2600,0.0335360057651997)
--(axis cs:2700,0.0328628718852997)
--(axis cs:2800,0.0321836248040199)
--(axis cs:2900,0.0316130146384239)
--(axis cs:3000,0.0310813430696726)
--(axis cs:3100,0.0305554866790771)
--(axis cs:3200,0.0300310850143433)
--(axis cs:3300,0.0295623950660229)
--(axis cs:3400,0.0290660616010427)
--(axis cs:3500,0.0286244861781597)
--(axis cs:3600,0.0282619949430227)
--(axis cs:3700,0.0279204603284597)
--(axis cs:3800,0.0275640245527029)
--(axis cs:3900,0.0272417049854994)
--(axis cs:4000,0.0269234739243984)
--(axis cs:4100,0.0266087632626295)
--(axis cs:4200,0.0262746028602123)
--(axis cs:4300,0.0259784460067749)
--(axis cs:4400,0.0256840698421001)
--(axis cs:4500,0.025422353297472)
--(axis cs:4600,0.0251768156886101)
--(axis cs:4700,0.0248997993767262)
--(axis cs:4800,0.0246410723775625)
--(axis cs:4900,0.0244234297424555)
--(axis cs:5000,0.0241819582879543)
--(axis cs:5100,0.023911451920867)
--(axis cs:5200,0.023717975243926)
--(axis cs:5300,0.0235067047178745)
--(axis cs:5400,0.0233240239322186)
--(axis cs:5500,0.0231068357825279)
--(axis cs:5600,0.0229784715920687)
--(axis cs:5700,0.0227612499147654)
--(axis cs:5800,0.0225841049104929)
--(axis cs:5900,0.0224048607051373)
--(axis cs:6000,0.022297715768218)
--(axis cs:6100,0.022106122225523)
--(axis cs:6200,0.0219367016106844)
--(axis cs:6300,0.0217886604368687)
--(axis cs:6400,0.0216727647930384)
--(axis cs:6500,0.0214779749512672)
--(axis cs:6600,0.0213423296809196)
--(axis cs:6700,0.0212131068110466)
--(axis cs:6800,0.021058265119791)
--(axis cs:6900,0.0209077894687653)
--(axis cs:7000,0.0208116676658392)
--(axis cs:7100,0.0206428822129965)
--(axis cs:7200,0.0205142125487328)
--(axis cs:7300,0.0203821882605553)
--(axis cs:7400,0.0202583931386471)
--(axis cs:7500,0.0200969353318214)
--(axis cs:7600,0.0200254842638969)
--(axis cs:7700,0.0199416987597942)
--(axis cs:7800,0.0198725201189518)
--(axis cs:7900,0.0197923127561808)
--(axis cs:8000,0.019678020849824)
--(axis cs:8100,0.0195372961461544)
--(axis cs:8200,0.0194431748241186)
--(axis cs:8300,0.0193353183567524)
--(axis cs:8400,0.0192584041506052)
--(axis cs:8500,0.019168758764863)
--(axis cs:8600,0.0191126521676779)
--(axis cs:8700,0.0189914871007204)
--(axis cs:8800,0.0188591480255127)
--(axis cs:8900,0.0187256205826998)
--(axis cs:9000,0.0186511036008596)
--(axis cs:9100,0.0185457225888968)
--(axis cs:9200,0.0184227023273706)
--(axis cs:9300,0.0183546524494886)
--(axis cs:9400,0.0182809066027403)
--(axis cs:9500,0.0182144083082676)
--(axis cs:9600,0.0181195940822363)
--(axis cs:9700,0.0180124081671238)
--(axis cs:9800,0.0179086569696665)
--(axis cs:9900,0.017798975110054)
--(axis cs:10000,0.0176953189074993)
--(axis cs:10100,0.0176235102117062)
--(axis cs:10200,0.0175520293414593)
--(axis cs:10300,0.0174635890871286)
--(axis cs:10400,0.0173541065305471)
--(axis cs:10500,0.0172543525695801)
--(axis cs:10600,0.0171952247619629)
--(axis cs:10700,0.0171174947172403)
--(axis cs:10800,0.0170639995485544)
--(axis cs:10900,0.0169872753322124)
--(axis cs:11000,0.0168898832052946)
--(axis cs:11100,0.0167966745793819)
--(axis cs:11200,0.0167413782328367)
--(axis cs:11300,0.0166730396449566)
--(axis cs:11400,0.0166212692856789)
--(axis cs:11500,0.0165572986006737)
--(axis cs:11600,0.0164825115352869)
--(axis cs:11700,0.0163666065782309)
--(axis cs:11800,0.0163099095225334)
--(axis cs:11900,0.0162454601377249)
--(axis cs:12000,0.0161346904933453)
--(axis cs:12100,0.0160410888493061)
--(axis cs:12200,0.0159886367619038)
--(axis cs:12300,0.0158777721226215)
--(axis cs:12400,0.0158244129270315)
--(axis cs:12500,0.015808392316103)
--(axis cs:12600,0.0157580859959126)
--(axis cs:12700,0.0156753528863192)
--(axis cs:12800,0.0156015632674098)
--(axis cs:12900,0.0155363623052835)
--(axis cs:13000,0.0154847735539079)
--(axis cs:13100,0.0154057005420327)
--(axis cs:13200,0.0153419924899936)
--(axis cs:13300,0.0153291122987866)
--(axis cs:13400,0.0152128096669912)
--(axis cs:13500,0.0151236429810524)
--(axis cs:13600,0.015059688128531)
--(axis cs:13700,0.0150268282741308)
--(axis cs:13800,0.014957713894546)
--(axis cs:13900,0.0148977460339665)
--(axis cs:14000,0.01487170252949)
--(axis cs:14100,0.0147934667766094)
--(axis cs:14200,0.0147208524867892)
--(axis cs:14300,0.0146452272310853)
--(axis cs:14400,0.0145756239071488)
--(axis cs:14500,0.014508455991745)
--(axis cs:14600,0.0144579643383622)
--(axis cs:14700,0.014405052177608)
--(axis cs:14800,0.0143630979582667)
--(axis cs:14900,0.0143644157797098)
--(axis cs:15000,0.0142960594967008)
--(axis cs:15100,0.0142386313527822)
--(axis cs:15200,0.0141917616128922)
--(axis cs:15300,0.0141233718022704)
--(axis cs:15400,0.0140844332054257)
--(axis cs:15500,0.014009271748364)
--(axis cs:15600,0.0139885367825627)
--(axis cs:15700,0.0139292981475592)
--(axis cs:15800,0.0139255244284868)
--(axis cs:15900,0.0138300377875566)
--(axis cs:16000,0.0137888630852103)
--(axis cs:16100,0.0137423677369952)
--(axis cs:16200,0.013752356171608)
--(axis cs:16300,0.0137053225189447)
--(axis cs:16400,0.0137010253965855)
--(axis cs:16500,0.0137208076193929)
--(axis cs:16600,0.0136511018499732)
--(axis cs:16700,0.0135561199858785)
--(axis cs:16800,0.0135262375697494)
--(axis cs:16900,0.0134382331743836)
--(axis cs:17000,0.0134098026901484)
--(axis cs:17100,0.0133632188662887)
--(axis cs:17200,0.0133196245878935)
--(axis cs:17300,0.0133143421262503)
--(axis cs:17400,0.0132740456610918)
--(axis cs:17500,0.0132473865523934)
--(axis cs:17600,0.0132341384887695)
--(axis cs:17700,0.0131863597780466)
--(axis cs:17800,0.0131292343139648)
--(axis cs:17900,0.0130986217409372)
--(axis cs:18000,0.0130372466519475)
--(axis cs:18100,0.0130224227905273)
--(axis cs:18200,0.0129850385710597)
--(axis cs:18300,0.0129268644377589)
--(axis cs:18400,0.0128796249628067)
--(axis cs:18500,0.0128180403262377)
--(axis cs:18600,0.0128370337188244)
--(axis cs:18700,0.0128092914819717)
--(axis cs:18800,0.0127866473048925)
--(axis cs:18900,0.0127832889556885)
--(axis cs:19000,0.0127441491931677)
--(axis cs:19100,0.0127102853730321)
--(axis cs:19200,0.0126736154779792)
--(axis cs:19300,0.0125960726290941)
--(axis cs:19400,0.0125647252425551)
--(axis cs:19500,0.0125095723196864)
--(axis cs:19600,0.0124355554580688)
--(axis cs:19700,0.0124140903353691)
--(axis cs:19800,0.0124387741088867)
--(axis cs:19900,0.0124377254396677)
--(axis cs:20000,0.0124164577573538)
--(axis cs:20100,0.0124020669609308)
--(axis cs:20200,0.0123092858120799)
--(axis cs:20300,0.0122746285051107)
--(axis cs:20400,0.012230608612299)
--(axis cs:20500,0.012207574211061)
--(axis cs:20600,0.0122112045064569)
--(axis cs:20700,0.0121787525713444)
--(axis cs:20800,0.012142944149673)
--(axis cs:20900,0.0121135106310248)
--(axis cs:21000,0.0120790479704738)
--(axis cs:21100,0.0120518682524562)
--(axis cs:21200,0.0120136570185423)
--(axis cs:21300,0.0119550349190831)
--(axis cs:21400,0.0119206691160798)
--(axis cs:21500,0.0119044575840235)
--(axis cs:21600,0.0118471728637815)
--(axis cs:21700,0.0118621876463294)
--(axis cs:21800,0.0118607524782419)
--(axis cs:21900,0.0118111614137888)
--(axis cs:22000,0.0117671964690089)
--(axis cs:22100,0.0117557924240828)
--(axis cs:22200,0.0117327310144901)
--(axis cs:22300,0.0116840796545148)
--(axis cs:22400,0.0116962529718876)
--(axis cs:22500,0.0116653814911842)
--(axis cs:22600,0.0116074196994305)
--(axis cs:22700,0.0116332052275538)
--(axis cs:22800,0.0115885734558105)
--(axis cs:22900,0.0115231517702341)
--(axis cs:23000,0.0115125775337219)
--(axis cs:23100,0.0115283606573939)
--(axis cs:23200,0.0114797987043858)
--(axis cs:23300,0.0114748952910304)
--(axis cs:23400,0.0114502180367708)
--(axis cs:23500,0.011414622887969)
--(axis cs:23600,0.0113980295136571)
--(axis cs:23700,0.0113910268992186)
--(axis cs:23800,0.0113622667267919)
--(axis cs:23900,0.011357975192368)
--(axis cs:24000,0.0113400230184197)
--(axis cs:24100,0.0113336816430092)
--(axis cs:24200,0.0112646101042628)
--(axis cs:24300,0.0112400809302926)
--(axis cs:24400,0.0112124439328909)
--(axis cs:24500,0.0111760143190622)
--(axis cs:24600,0.0111130774021149)
--(axis cs:24700,0.0110944975167513)
--(axis cs:24800,0.0110788950696588)
--(axis cs:24900,0.0110671268776059)
--(axis cs:25000,0.0110290525481105)
--(axis cs:25100,0.011013412848115)
--(axis cs:25200,0.0109880920499563)
--(axis cs:25300,0.010956522077322)
--(axis cs:25400,0.0109062027186155)
--(axis cs:25500,0.0109069822356105)
--(axis cs:25600,0.0108440211042762)
--(axis cs:25700,0.0108280181884766)
--(axis cs:25800,0.0108275879174471)
--(axis cs:25900,0.0108341220766306)
--(axis cs:26000,0.0108281131833792)
--(axis cs:26100,0.0108047481626272)
--(axis cs:26200,0.0108080413192511)
--(axis cs:26300,0.0107443304732442)
--(axis cs:26400,0.0107106622308493)
--(axis cs:26500,0.0106398211792111)
--(axis cs:26600,0.0106361387297511)
--(axis cs:26700,0.0105820652097464)
--(axis cs:26800,0.0105976108461618)
--(axis cs:26900,0.0105530740693212)
--(axis cs:27000,0.0106028560549021)
--(axis cs:27100,0.01062788721174)
--(axis cs:27200,0.0106025440618396)
--(axis cs:27300,0.0106082381680608)
--(axis cs:27400,0.0105803441256285)
--(axis cs:27500,0.0105407144874334)
--(axis cs:27600,0.0104920500889421)
--(axis cs:27700,0.0105308536440134)
--(axis cs:27800,0.010491942986846)
--(axis cs:27900,0.0104450732469559)
--(axis cs:28000,0.0104446904733777)
--(axis cs:28100,0.0104502430185676)
--(axis cs:28200,0.0104138376191258)
--(axis cs:28300,0.0103866392746568)
--(axis cs:28400,0.0103658782318234)
--(axis cs:28500,0.0103333117440343)
--(axis cs:28600,0.0102964034304023)
--(axis cs:28700,0.0102840242907405)
--(axis cs:28800,0.0102773820981383)
--(axis cs:28900,0.0102506531402469)
--(axis cs:29000,0.0102233570069075)
--(axis cs:29100,0.0102275386452675)
--(axis cs:29200,0.0102102616801858)
--(axis cs:29300,0.0102035067975521)
--(axis cs:29400,0.0101978303864598)
--(axis cs:29500,0.0102004054933786)
--(axis cs:29600,0.0101241115480661)
--(axis cs:29700,0.0101123806089163)
--(axis cs:29800,0.0100692752748728)
--(axis cs:29900,0.0100580947473645)
--(axis cs:30000,0.00999717693775892)
--(axis cs:30100,0.0100271226838231)
--(axis cs:30200,0.0100125409662724)
--(axis cs:30300,0.00998885650187731)
--(axis cs:30400,0.0099664218723774)
--(axis cs:30500,0.00996250100433826)
--(axis cs:30600,0.00992115773260593)
--(axis cs:30700,0.00990260019898415)
--(axis cs:30800,0.00987290777266026)
--(axis cs:30900,0.00985742546617985)
--(axis cs:31000,0.00986372958868742)
--(axis cs:31100,0.00986238848417997)
--(axis cs:31200,0.00987695250660181)
--(axis cs:31300,0.00990858115255833)
--(axis cs:31400,0.00989713333547115)
--(axis cs:31500,0.00988187827169895)
--(axis cs:31600,0.00985479354858398)
--(axis cs:31700,0.00983131490647793)
--(axis cs:31800,0.0098100658506155)
--(axis cs:31900,0.00980119686573744)
--(axis cs:32000,0.0098111480474472)
--(axis cs:32100,0.00981569290161133)
--(axis cs:32200,0.00981852784752846)
--(axis cs:32300,0.00978679116815329)
--(axis cs:32400,0.00975015573203564)
--(axis cs:32500,0.009734439663589)
--(axis cs:32600,0.00969409942626953)
--(axis cs:32700,0.009674072265625)
--(axis cs:32800,0.00960033945739269)
--(axis cs:32900,0.00961164012551308)
--(axis cs:33000,0.00957019906491041)
--(axis cs:33100,0.0095888739451766)
--(axis cs:33200,0.00958347320556641)
--(axis cs:33300,0.00957717932760715)
--(axis cs:33400,0.0095664020627737)
--(axis cs:33500,0.00954713858664036)
--(axis cs:33600,0.0095362663269043)
--(axis cs:33700,0.00953149795532227)
--(axis cs:33800,0.0095067024230957)
--(axis cs:33900,0.00947237014770508)
--(axis cs:34000,0.00947550870478153)
--(axis cs:34100,0.00946750678122044)
--(axis cs:34200,0.00943441409617662)
--(axis cs:34300,0.0094276424497366)
--(axis cs:34400,0.00939884223043919)
--(axis cs:34500,0.00938577670603991)
--(axis cs:34600,0.00939655303955078)
--(axis cs:34700,0.00938138924539089)
--(axis cs:34800,0.00937452353537083)
--(axis cs:34900,0.00935935974121094)
--(axis cs:35000,0.0093864444643259)
--(axis cs:35100,0.0093670841306448)
--(axis cs:35200,0.00936946831643581)
--(axis cs:35300,0.00936307944357395)
--(axis cs:35400,0.00935020484030247)
--(axis cs:35500,0.00930281262844801)
--(axis cs:35600,0.0093226432800293)
--(axis cs:35700,0.00929911714047194)
--(axis cs:35800,0.00930395163595676)
--(axis cs:35900,0.00928819738328457)
--(axis cs:36000,0.00925733521580696)
--(axis cs:36100,0.00925680436193943)
--(axis cs:36200,0.00926316436380148)
--(axis cs:36300,0.00921400170773268)
--(axis cs:36400,0.00921938940882683)
--(axis cs:36500,0.00924787390977144)
--(axis cs:36600,0.00920475646853447)
--(axis cs:36700,0.0091787064447999)
--(axis cs:36800,0.00921904947608709)
--(axis cs:36900,0.00919449981302023)
--(axis cs:37000,0.00914567429572344)
--(axis cs:37100,0.00913190841674805)
--(axis cs:37200,0.00915038865059614)
--(axis cs:37300,0.00911509525030851)
--(axis cs:37400,0.00910098385065794)
--(axis cs:37500,0.00910989940166473)
--(axis cs:37600,0.00913388933986425)
--(axis cs:37700,0.00909369345754385)
--(axis cs:37800,0.00910383928567171)
--(axis cs:37900,0.0091019831597805)
--(axis cs:38000,0.00908968411386013)
--(axis cs:38100,0.00904272776097059)
--(axis cs:38200,0.00901900418102741)
--(axis cs:38300,0.00901689566671848)
--(axis cs:38400,0.00899532716721296)
--(axis cs:38500,0.00898173451423645)
--(axis cs:38600,0.00900714099407196)
--(axis cs:38700,0.00908674672245979)
--(axis cs:38800,0.00906237680464983)
--(axis cs:38900,0.00905407965183258)
--(axis cs:39000,0.00903932470828295)
--(axis cs:39100,0.00901929475367069)
--(axis cs:39200,0.00893999356776476)
--(axis cs:39300,0.00893727131187916)
--(axis cs:39400,0.0089572612196207)
--(axis cs:39500,0.00893682986497879)
--(axis cs:39600,0.00891405995935202)
--(axis cs:39700,0.00891833938658237)
--(axis cs:39800,0.00891280639916658)
--(axis cs:39900,0.00888894032686949)
--(axis cs:40000,0.00889360066503286)
--(axis cs:40100,0.00888642575591803)
--(axis cs:40200,0.00887435674667358)
--(axis cs:40300,0.00884527992457151)
--(axis cs:40400,0.00882230885326862)
--(axis cs:40500,0.0088125579059124)
--(axis cs:40600,0.00879974383860826)
--(axis cs:40700,0.00878274161368608)
--(axis cs:40800,0.00874852947890759)
--(axis cs:40900,0.00875944271683693)
--(axis cs:41000,0.00874897837638855)
--(axis cs:41100,0.00875204335898161)
--(axis cs:41200,0.00873498991131783)
--(axis cs:41300,0.00874389242380857)
--(axis cs:41400,0.00873820669949055)
--(axis cs:41500,0.00874119997024536)
--(axis cs:41600,0.00873902998864651)
--(axis cs:41700,0.00873311888426542)
--(axis cs:41800,0.00873902998864651)
--(axis cs:41900,0.00871986616402864)
--(axis cs:42000,0.00870660506188869)
--(axis cs:42100,0.00867892988026142)
--(axis cs:42200,0.008676677942276)
--(axis cs:42300,0.0086832819506526)
--(axis cs:42400,0.00870413146913052)
--(axis cs:42500,0.00868688337504864)
--(axis cs:42600,0.00868965871632099)
--(axis cs:42700,0.00867720320820808)
--(axis cs:42800,0.00864903908222914)
--(axis cs:42900,0.00860601384192705)
--(axis cs:43000,0.00859019998461008)
--(axis cs:43100,0.00861037988215685)
--(axis cs:43200,0.00862129125744104)
--(axis cs:43300,0.00861293915659189)
--(axis cs:43400,0.00863310135900974)
--(axis cs:43500,0.00862407591193914)
--(axis cs:43600,0.0085749039426446)
--(axis cs:43700,0.00853749923408031)
--(axis cs:43800,0.00850390363484621)
--(axis cs:43900,0.0084768533706665)
--(axis cs:44000,0.00848947465419769)
--(axis cs:44100,0.00849755853414536)
--(axis cs:44200,0.00852383859455585)
--(axis cs:44300,0.00856842193752527)
--(axis cs:44400,0.00856337137520313)
--(axis cs:44500,0.00858696084469557)
--(axis cs:44600,0.00858033075928688)
--(axis cs:44700,0.00856744311749935)
--(axis cs:44800,0.00852421671152115)
--(axis cs:44900,0.00850964430719614)
--(axis cs:44900,0.00981760025024414)
--(axis cs:44900,0.00981760025024414)
--(axis cs:44800,0.00981760025024414)
--(axis cs:44700,0.00981760025024414)
--(axis cs:44600,0.00981760025024414)
--(axis cs:44500,0.00981760025024414)
--(axis cs:44400,0.00981760025024414)
--(axis cs:44300,0.00981760025024414)
--(axis cs:44200,0.00981760025024414)
--(axis cs:44100,0.00981760025024414)
--(axis cs:44000,0.00981760025024414)
--(axis cs:43900,0.00981760025024414)
--(axis cs:43800,0.00981760025024414)
--(axis cs:43700,0.00981760025024414)
--(axis cs:43600,0.00981760025024414)
--(axis cs:43500,0.00981760025024414)
--(axis cs:43400,0.00981700047850609)
--(axis cs:43300,0.00981760025024414)
--(axis cs:43200,0.00981760025024414)
--(axis cs:43100,0.00981760025024414)
--(axis cs:43000,0.00981760025024414)
--(axis cs:42900,0.00981760025024414)
--(axis cs:42800,0.00981454085558653)
--(axis cs:42700,0.00981021858751774)
--(axis cs:42600,0.00980831682682037)
--(axis cs:42500,0.00980873964726925)
--(axis cs:42400,0.00980611518025398)
--(axis cs:42300,0.00980929005891085)
--(axis cs:42200,0.00981029868125916)
--(axis cs:42100,0.00980995409190655)
--(axis cs:42000,0.00980573892593384)
--(axis cs:41900,0.00980373192578554)
--(axis cs:41800,0.00980084389448166)
--(axis cs:41700,0.00980173330754042)
--(axis cs:41600,0.00980084389448166)
--(axis cs:41500,0.00980051793158054)
--(axis cs:41400,0.00980096682906151)
--(axis cs:41300,0.00980011280626059)
--(axis cs:41200,0.00980145111680031)
--(axis cs:41100,0.00979889277368784)
--(axis cs:41000,0.00979935191571712)
--(axis cs:40900,0.00979778729379177)
--(axis cs:40800,0.0097994189709425)
--(axis cs:40700,0.00979432556778193)
--(axis cs:40600,0.00979181844741106)
--(axis cs:40500,0.00978993996977806)
--(axis cs:40400,0.0097885187715292)
--(axis cs:40300,0.00978519301861525)
--(axis cs:40200,0.00978103838860989)
--(axis cs:40100,0.00977933313697577)
--(axis cs:40000,0.00977832544595003)
--(axis cs:39900,0.00977897923439741)
--(axis cs:39800,0.00977565068751574)
--(axis cs:39700,0.00977488607168198)
--(axis cs:39600,0.00977547746151686)
--(axis cs:39500,0.00977235287427902)
--(axis cs:39400,0.00976959615945816)
--(axis cs:39300,0.00977229326963425)
--(axis cs:39200,0.00977192353457212)
--(axis cs:39100,0.00976154021918774)
--(axis cs:39000,0.00975905824452639)
--(axis cs:38900,0.00975727289915085)
--(axis cs:38800,0.00975628662854433)
--(axis cs:38700,0.00975347124040127)
--(axis cs:38600,0.00976307690143585)
--(axis cs:38500,0.00976635701954365)
--(axis cs:38400,0.00976459216326475)
--(axis cs:38300,0.00976184196770191)
--(axis cs:38200,0.00976157747209072)
--(axis cs:38100,0.00975864287465811)
--(axis cs:38000,0.0097531396895647)
--(axis cs:37900,0.00975177623331547)
--(axis cs:37800,0.00975157413631678)
--(axis cs:37700,0.00975269172340631)
--(axis cs:37600,0.00974841695278883)
--(axis cs:37500,0.00975091755390167)
--(axis cs:37400,0.0097518851980567)
--(axis cs:37300,0.00975036341696978)
--(axis cs:37200,0.00974679458886385)
--(axis cs:37100,0.00974861718714237)
--(axis cs:37000,0.00974724907428026)
--(axis cs:36900,0.0097429296001792)
--(axis cs:36800,0.00974114146083593)
--(axis cs:36700,0.00974422600120306)
--(axis cs:36600,0.00974214635789394)
--(axis cs:36500,0.00973946321755648)
--(axis cs:36400,0.00974111817777157)
--(axis cs:36300,0.00974148418754339)
--(axis cs:36200,0.00973879639059305)
--(axis cs:36100,0.00973905250430107)
--(axis cs:36000,0.00973903015255928)
--(axis cs:35900,0.00973811373114586)
--(axis cs:35800,0.00973799359053373)
--(axis cs:35700,0.00973800290375948)
--(axis cs:35600,0.00973809510469437)
--(axis cs:35500,0.00973799359053373)
--(axis cs:35400,0.00973860640078783)
--(axis cs:35300,0.00973900593817234)
--(axis cs:35200,0.00973924621939659)
--(axis cs:35100,0.00973915308713913)
--(axis cs:35000,0.00974002201110125)
--(axis cs:34900,0.00973888020962477)
--(axis cs:34800,0.00973945483565331)
--(axis cs:34700,0.00973976869136095)
--(axis cs:34600,0.00974058546125889)
--(axis cs:34500,0.00973998662084341)
--(axis cs:34400,0.00974072329699993)
--(axis cs:34300,0.00974283181130886)
--(axis cs:34200,0.0097479997202754)
--(axis cs:34100,0.0097534628584981)
--(axis cs:34000,0.00976626947522163)
--(axis cs:33900,0.00976164545863867)
--(axis cs:33800,0.00976221822202206)
--(axis cs:33700,0.00976445339620113)
--(axis cs:33600,0.00976430624723434)
--(axis cs:33500,0.00977353285998106)
--(axis cs:33400,0.00977737735956907)
--(axis cs:33300,0.00977974198758602)
--(axis cs:33200,0.00977542996406555)
--(axis cs:33100,0.00978298578411341)
--(axis cs:33000,0.00978099834173918)
--(axis cs:32900,0.00978724099695683)
--(axis cs:32800,0.00978576205670834)
--(axis cs:32700,0.00978967826813459)
--(axis cs:32600,0.00979689229279757)
--(axis cs:32500,0.00980173423886299)
--(axis cs:32400,0.00980805233120918)
--(axis cs:32300,0.00981394853442907)
--(axis cs:32200,0.00982570089399815)
--(axis cs:32100,0.00983877014368773)
--(axis cs:32000,0.00983702205121517)
--(axis cs:31900,0.00985331833362579)
--(axis cs:31800,0.00988580379635096)
--(axis cs:31700,0.0099287535995245)
--(axis cs:31600,0.00991843268275261)
--(axis cs:31500,0.00996512826532125)
--(axis cs:31400,0.00995264388620853)
--(axis cs:31300,0.00996849779039621)
--(axis cs:31200,0.009929527528584)
--(axis cs:31100,0.00993061345070601)
--(axis cs:31000,0.00988692883402109)
--(axis cs:30900,0.0099186897277832)
--(axis cs:30800,0.00994133017957211)
--(axis cs:30700,0.00996723212301731)
--(axis cs:30600,0.00999963656067848)
--(axis cs:30500,0.0100844949483871)
--(axis cs:30400,0.0100713726133108)
--(axis cs:30300,0.0100850341841578)
--(axis cs:30200,0.0100639341399074)
--(axis cs:30100,0.0101233161985874)
--(axis cs:30000,0.0100917937234044)
--(axis cs:29900,0.0101124988868833)
--(axis cs:29800,0.0101455114781857)
--(axis cs:29700,0.0101354792714119)
--(axis cs:29600,0.0101544018834829)
--(axis cs:29500,0.0102128060534596)
--(axis cs:29400,0.0102396458387375)
--(axis cs:29300,0.0102354511618614)
--(axis cs:29200,0.0102814668789506)
--(axis cs:29100,0.0102936252951622)
--(axis cs:29000,0.010263666510582)
--(axis cs:28900,0.0102819548919797)
--(axis cs:28800,0.0103355403989553)
--(axis cs:28700,0.010355013422668)
--(axis cs:28600,0.0104009350761771)
--(axis cs:28500,0.0104560265317559)
--(axis cs:28400,0.0104374885559082)
--(axis cs:28300,0.0104182744398713)
--(axis cs:28200,0.0104532698169351)
--(axis cs:28100,0.0104832882061601)
--(axis cs:28000,0.0104785915464163)
--(axis cs:27900,0.0105533748865128)
--(axis cs:27800,0.0105800963938236)
--(axis cs:27700,0.0106152836233377)
--(axis cs:27600,0.0106422612443566)
--(axis cs:27500,0.0107002258300781)
--(axis cs:27400,0.0107155852019787)
--(axis cs:27300,0.0107455253601074)
--(axis cs:27200,0.0107453344389796)
--(axis cs:27100,0.0107482140883803)
--(axis cs:27000,0.0107669522985816)
--(axis cs:26900,0.010798410512507)
--(axis cs:26800,0.0107461269944906)
--(axis cs:26700,0.0107617303729057)
--(axis cs:26600,0.0107875196263194)
--(axis cs:26500,0.0108062783256173)
--(axis cs:26400,0.01082525216043)
--(axis cs:26300,0.0108385263010859)
--(axis cs:26200,0.010894107632339)
--(axis cs:26100,0.0109390905126929)
--(axis cs:26000,0.0109749333932996)
--(axis cs:25900,0.0109571469947696)
--(axis cs:25800,0.0109552219510078)
--(axis cs:25700,0.0109237283468246)
--(axis cs:25600,0.0109124695882201)
--(axis cs:25500,0.0109326867386699)
--(axis cs:25400,0.010975981131196)
--(axis cs:25300,0.0110233183950186)
--(axis cs:25200,0.0110782776027918)
--(axis cs:25100,0.0111314402893186)
--(axis cs:25000,0.0111259380355477)
--(axis cs:24900,0.0111210821196437)
--(axis cs:24800,0.0111306188628078)
--(axis cs:24700,0.0111324712634087)
--(axis cs:24600,0.0111339837312698)
--(axis cs:24500,0.0111861554905772)
--(axis cs:24400,0.0112485243007541)
--(axis cs:24300,0.0112746423110366)
--(axis cs:24200,0.0113095743581653)
--(axis cs:24100,0.0113524440675974)
--(axis cs:24000,0.0113473823294044)
--(axis cs:23900,0.0113813653588295)
--(axis cs:23800,0.0114620383828878)
--(axis cs:23700,0.0114919431507587)
--(axis cs:23600,0.0115079907700419)
--(axis cs:23500,0.0115275271236897)
--(axis cs:23400,0.0115677919238806)
--(axis cs:23300,0.0115403588861227)
--(axis cs:23200,0.0115270856767893)
--(axis cs:23100,0.0115502355620265)
--(axis cs:23000,0.0115682603791356)
--(axis cs:22900,0.0115883247926831)
--(axis cs:22800,0.0116338850930333)
--(axis cs:22700,0.0116669228300452)
--(axis cs:22600,0.0116993905976415)
--(axis cs:22500,0.011736324056983)
--(axis cs:22400,0.0117433462291956)
--(axis cs:22300,0.0117527963593602)
--(axis cs:22200,0.0117894168943167)
--(axis cs:22100,0.0118451043963432)
--(axis cs:22000,0.0118656335398555)
--(axis cs:21900,0.011854974552989)
--(axis cs:21800,0.011913432739675)
--(axis cs:21700,0.01194451097399)
--(axis cs:21600,0.011992777697742)
--(axis cs:21500,0.0120187178254128)
--(axis cs:21400,0.0121123054996133)
--(axis cs:21300,0.012103752233088)
--(axis cs:21200,0.0120978355407715)
--(axis cs:21100,0.0120992418378592)
--(axis cs:21000,0.0121458228677511)
--(axis cs:20900,0.0121409082785249)
--(axis cs:20800,0.0121867768466473)
--(axis cs:20700,0.0122829936444759)
--(axis cs:20600,0.0122548015788198)
--(axis cs:20500,0.0122761065140367)
--(axis cs:20400,0.0123125072568655)
--(axis cs:20300,0.0123425479978323)
--(axis cs:20200,0.0123398872092366)
--(axis cs:20100,0.0124297142028809)
--(axis cs:20000,0.0124724106863141)
--(axis cs:19900,0.0124943275004625)
--(axis cs:19800,0.0125038232654333)
--(axis cs:19700,0.0125264618545771)
--(axis cs:19600,0.0125227924436331)
--(axis cs:19500,0.0125947585329413)
--(axis cs:19400,0.0126494700089097)
--(axis cs:19300,0.0127182956784964)
--(axis cs:19200,0.0127710346132517)
--(axis cs:19100,0.0128004103899002)
--(axis cs:19000,0.0128087922930717)
--(axis cs:18900,0.0128120575100183)
--(axis cs:18800,0.01285320520401)
--(axis cs:18700,0.01288185082376)
--(axis cs:18600,0.0129249505698681)
--(axis cs:18500,0.0129923932254314)
--(axis cs:18400,0.0130294803529978)
--(axis cs:18300,0.0130600640550256)
--(axis cs:18200,0.0130613837391138)
--(axis cs:18100,0.0131297605112195)
--(axis cs:18000,0.0131539581343532)
--(axis cs:17900,0.0131791587918997)
--(axis cs:17800,0.0132534941658378)
--(axis cs:17700,0.0133034186437726)
--(axis cs:17600,0.0133366109803319)
--(axis cs:17500,0.0133627345785499)
--(axis cs:17400,0.0133653841912746)
--(axis cs:17300,0.0134083516895771)
--(axis cs:17200,0.013502337038517)
--(axis cs:17100,0.0134558184072375)
--(axis cs:17000,0.0135493315756321)
--(axis cs:16900,0.0136361690238118)
--(axis cs:16800,0.0136342803016305)
--(axis cs:16700,0.0136768454685807)
--(axis cs:16600,0.0137632852420211)
--(axis cs:16500,0.0137732746079564)
--(axis cs:16400,0.0138300899416208)
--(axis cs:16300,0.0138827264308929)
--(axis cs:16200,0.0139306541532278)
--(axis cs:16100,0.0139421466737986)
--(axis cs:16000,0.0139581207185984)
--(axis cs:15900,0.0139944553375244)
--(axis cs:15800,0.0140493391081691)
--(axis cs:15700,0.0140560511499643)
--(axis cs:15600,0.0141534069553018)
--(axis cs:15500,0.0142648192122579)
--(axis cs:15400,0.0142949419096112)
--(axis cs:15300,0.014360242523253)
--(axis cs:15200,0.0144058167934418)
--(axis cs:15100,0.0144036412239075)
--(axis cs:15000,0.0144205363467336)
--(axis cs:14900,0.0144539996981621)
--(axis cs:14800,0.0144898723810911)
--(axis cs:14700,0.0145029770210385)
--(axis cs:14600,0.0145877758041024)
--(axis cs:14500,0.0146119892597198)
--(axis cs:14400,0.014730310998857)
--(axis cs:14300,0.0148157123476267)
--(axis cs:14200,0.0148933883756399)
--(axis cs:14100,0.0149639127776027)
--(axis cs:14000,0.0150173390284181)
--(axis cs:13900,0.0150119299069047)
--(axis cs:13800,0.0150462435558438)
--(axis cs:13700,0.0151396095752716)
--(axis cs:13600,0.015181771479547)
--(axis cs:13500,0.0152234509587288)
--(axis cs:13400,0.0153436157852411)
--(axis cs:13300,0.0154324052855372)
--(axis cs:13200,0.0154607770964503)
--(axis cs:13100,0.0155480857938528)
--(axis cs:13000,0.0156178520992398)
--(axis cs:12900,0.0156608354300261)
--(axis cs:12800,0.0156801957637072)
--(axis cs:12700,0.0157846454530954)
--(axis cs:12600,0.0158737972378731)
--(axis cs:12500,0.0159679260104895)
--(axis cs:12400,0.0160554368048906)
--(axis cs:12300,0.0161532387137413)
--(axis cs:12200,0.0161912459880114)
--(axis cs:12100,0.0162125881761312)
--(axis cs:12000,0.0162795092910528)
--(axis cs:11900,0.0163390878587961)
--(axis cs:11800,0.0164129436016083)
--(axis cs:11700,0.0164711978286505)
--(axis cs:11600,0.016582490876317)
--(axis cs:11500,0.0166755206882954)
--(axis cs:11400,0.0167262069880962)
--(axis cs:11300,0.0167422741651535)
--(axis cs:11200,0.0168737974017859)
--(axis cs:11100,0.0169166661798954)
--(axis cs:11000,0.016962630674243)
--(axis cs:10900,0.0170543827116489)
--(axis cs:10800,0.0171628128737211)
--(axis cs:10700,0.0172284189611673)
--(axis cs:10600,0.0173048358410597)
--(axis cs:10500,0.0174034386873245)
--(axis cs:10400,0.0174682922661304)
--(axis cs:10300,0.017548430711031)
--(axis cs:10200,0.0176105983555317)
--(axis cs:10100,0.0177533254027367)
--(axis cs:10000,0.0178423877805471)
--(axis cs:9900,0.0179459564387798)
--(axis cs:9800,0.0180930253118277)
--(axis cs:9700,0.0181863345205784)
--(axis cs:9600,0.0182542745023966)
--(axis cs:9500,0.0183899328112602)
--(axis cs:9400,0.0184973832219839)
--(axis cs:9300,0.0185294654220343)
--(axis cs:9200,0.0186066273599863)
--(axis cs:9100,0.0187499988824129)
--(axis cs:9000,0.0188134498894215)
--(axis cs:8900,0.0189013760536909)
--(axis cs:8800,0.0189830996096134)
--(axis cs:8700,0.0191060844808817)
--(axis cs:8600,0.0191610809415579)
--(axis cs:8500,0.0192514453083277)
--(axis cs:8400,0.0193099640309811)
--(axis cs:8300,0.0194547735154629)
--(axis cs:8200,0.0195495467633009)
--(axis cs:8100,0.0196616724133492)
--(axis cs:8000,0.0197633597999811)
--(axis cs:7900,0.0198562163859606)
--(axis cs:7800,0.0199846141040325)
--(axis cs:7700,0.0200949162244797)
--(axis cs:7600,0.0201998911798)
--(axis cs:7500,0.0203391071408987)
--(axis cs:7400,0.0204577445983887)
--(axis cs:7300,0.020592775195837)
--(axis cs:7200,0.02069091796875)
--(axis cs:7100,0.0207929126918316)
--(axis cs:7000,0.020945405587554)
--(axis cs:6900,0.0211072918027639)
--(axis cs:6800,0.0212579146027565)
--(axis cs:6700,0.0214105136692524)
--(axis cs:6600,0.0215893276035786)
--(axis cs:6500,0.0217418186366558)
--(axis cs:6400,0.02189726755023)
--(axis cs:6300,0.0220845192670822)
--(axis cs:6200,0.0222288463264704)
--(axis cs:6100,0.0224009975790977)
--(axis cs:6000,0.0225120577961206)
--(axis cs:5900,0.0227011889219284)
--(axis cs:5800,0.0228366442024708)
--(axis cs:5700,0.0229272488504648)
--(axis cs:5600,0.0230689588934183)
--(axis cs:5500,0.0232525579631329)
--(axis cs:5400,0.0234100855886936)
--(axis cs:5300,0.0236716121435165)
--(axis cs:5200,0.0239564217627048)
--(axis cs:5100,0.0241363178938627)
--(axis cs:5000,0.0244102627038956)
--(axis cs:4900,0.0246717222034931)
--(axis cs:4800,0.0248761884868145)
--(axis cs:4700,0.0251153223216534)
--(axis cs:4600,0.025427620857954)
--(axis cs:4500,0.0256318561732769)
--(axis cs:4400,0.0259376652538776)
--(axis cs:4300,0.0261977445334196)
--(axis cs:4200,0.026547908782959)
--(axis cs:4100,0.0268498193472624)
--(axis cs:4000,0.0272371061146259)
--(axis cs:3900,0.0275289546698332)
--(axis cs:3800,0.0279086977243423)
--(axis cs:3700,0.0282009057700634)
--(axis cs:3600,0.0285837352275848)
--(axis cs:3500,0.0289764702320099)
--(axis cs:3400,0.0294577870517969)
--(axis cs:3300,0.0298750400543213)
--(axis cs:3200,0.0303155612200499)
--(axis cs:3100,0.0307642351835966)
--(axis cs:3000,0.0312351882457733)
--(axis cs:2900,0.031732052564621)
--(axis cs:2800,0.0323612876236439)
--(axis cs:2700,0.0331559777259827)
--(axis cs:2600,0.033890638500452)
--(axis cs:2500,0.0346561186015606)
--(axis cs:2400,0.0353867933154106)
--(axis cs:2300,0.0359896793961525)
--(axis cs:2200,0.0364970974624157)
--(axis cs:2100,0.0370430052280426)
--(axis cs:2000,0.0374748520553112)
--(axis cs:1900,0.0378871001303196)
--(axis cs:1800,0.0384030789136887)
--(axis cs:1700,0.0389373302459717)
--(axis cs:1600,0.0395270250737667)
--(axis cs:1500,0.0402104370296001)
--(axis cs:1400,0.0409765765070915)
--(axis cs:1300,0.0417912527918816)
--(axis cs:1200,0.0426510572433472)
--(axis cs:1100,0.0435818210244179)
--(axis cs:1000,0.0446990989148617)
--(axis cs:900,0.0459758415818214)
--(axis cs:800,0.0473586320877075)
--(axis cs:700,0.0488137416541576)
--(axis cs:600,0.0502007082104683)
--(axis cs:500,0.0514562092721462)
--(axis cs:400,0.0525052286684513)
--(axis cs:300,0.0533110685646534)
--(axis cs:200,0.0538739748299122)
--(axis cs:100,0.0542582049965858)
--(axis cs:0,0.0544335320591927)
--cycle;

\path [fill=green!50.1960784313725!black, fill opacity=0.4, ultra thick]
(axis cs:0,0.0637036859989166)
--(axis cs:0,0.0636349767446518)
--(axis cs:100,0.0615603215992451)
--(axis cs:200,0.0590961202979088)
--(axis cs:300,0.0565544627606869)
--(axis cs:400,0.0542185232043266)
--(axis cs:500,0.0527046918869019)
--(axis cs:600,0.052056085318327)
--(axis cs:700,0.0517884381115437)
--(axis cs:800,0.0516378432512283)
--(axis cs:900,0.051479309797287)
--(axis cs:1000,0.051042702049017)
--(axis cs:1100,0.0501771159470081)
--(axis cs:1200,0.0489348508417606)
--(axis cs:1300,0.0474495440721512)
--(axis cs:1400,0.0455842725932598)
--(axis cs:1500,0.0437570475041866)
--(axis cs:1600,0.0418655760586262)
--(axis cs:1700,0.0397585742175579)
--(axis cs:1800,0.0369190648198128)
--(axis cs:1900,0.033805537968874)
--(axis cs:2000,0.030795119702816)
--(axis cs:2100,0.0282053463160992)
--(axis cs:2200,0.0261255018413067)
--(axis cs:2300,0.0245132707059383)
--(axis cs:2400,0.0232763905078173)
--(axis cs:2500,0.0221428163349628)
--(axis cs:2600,0.0210395399481058)
--(axis cs:2700,0.0200916286557913)
--(axis cs:2800,0.0192982442677021)
--(axis cs:2900,0.0186894182115793)
--(axis cs:3000,0.018135953694582)
--(axis cs:3100,0.0176824033260345)
--(axis cs:3200,0.017232982441783)
--(axis cs:3300,0.0168337393552065)
--(axis cs:3400,0.0164223331958055)
--(axis cs:3500,0.0160551816225052)
--(axis cs:3600,0.015727449208498)
--(axis cs:3700,0.0153868198394775)
--(axis cs:3800,0.0150002241134644)
--(axis cs:3900,0.0146481990814209)
--(axis cs:4000,0.0142989158630371)
--(axis cs:4100,0.0139313936233521)
--(axis cs:4200,0.0136183062568307)
--(axis cs:4300,0.0133459279313684)
--(axis cs:4400,0.0131141152232885)
--(axis cs:4500,0.0129212141036987)
--(axis cs:4600,0.0127708734944463)
--(axis cs:4700,0.0126023534685373)
--(axis cs:4800,0.0124559877440333)
--(axis cs:4900,0.0122753251343966)
--(axis cs:5000,0.0121081974357367)
--(axis cs:5100,0.011993714608252)
--(axis cs:5200,0.0118730310350657)
--(axis cs:5300,0.0117479087784886)
--(axis cs:5400,0.0116108180955052)
--(axis cs:5500,0.0114802848547697)
--(axis cs:5600,0.0113481674343348)
--(axis cs:5700,0.0112878559157252)
--(axis cs:5800,0.0111934188753366)
--(axis cs:5900,0.0111123975366354)
--(axis cs:6000,0.0110433055087924)
--(axis cs:6100,0.0109653947874904)
--(axis cs:6200,0.0108279697597027)
--(axis cs:6300,0.0107330400496721)
--(axis cs:6400,0.0106290513649583)
--(axis cs:6500,0.0105752069503069)
--(axis cs:6600,0.0104993423447013)
--(axis cs:6700,0.0103827137500048)
--(axis cs:6800,0.0103110717609525)
--(axis cs:6900,0.0102437743917108)
--(axis cs:7000,0.0101909032091498)
--(axis cs:7100,0.0101536978036165)
--(axis cs:7200,0.0100868744775653)
--(axis cs:7300,0.0100052990019321)
--(axis cs:7400,0.00998483877629042)
--(axis cs:7500,0.0099245086312294)
--(axis cs:7600,0.00982762966305017)
--(axis cs:7700,0.00982656609266996)
--(axis cs:7800,0.00977120362222195)
--(axis cs:7900,0.00968469679355621)
--(axis cs:8000,0.00964463874697685)
--(axis cs:8100,0.00961857009679079)
--(axis cs:8200,0.0095398910343647)
--(axis cs:8300,0.00952783972024918)
--(axis cs:8400,0.0094585120677948)
--(axis cs:8500,0.00942463893443346)
--(axis cs:8600,0.00938692130148411)
--(axis cs:8700,0.00931196194142103)
--(axis cs:8800,0.00928010977804661)
--(axis cs:8900,0.00923133175820112)
--(axis cs:9000,0.00919395219534636)
--(axis cs:9100,0.00914883613586426)
--(axis cs:9200,0.00909476261585951)
--(axis cs:9300,0.00905415881425142)
--(axis cs:9400,0.00900821667164564)
--(axis cs:9500,0.00897607766091824)
--(axis cs:9600,0.00891470909118652)
--(axis cs:9700,0.00887002982199192)
--(axis cs:9800,0.00882124807685614)
--(axis cs:9900,0.00877401046454906)
--(axis cs:10000,0.00874427333474159)
--(axis cs:10100,0.00871048588305712)
--(axis cs:10200,0.00866400729864836)
--(axis cs:10300,0.00862484890967607)
--(axis cs:10400,0.00858969707041979)
--(axis cs:10500,0.00855994131416082)
--(axis cs:10600,0.00851969514042139)
--(axis cs:10700,0.00850529689341784)
--(axis cs:10800,0.00846571940928698)
--(axis cs:10900,0.00847913883626461)
--(axis cs:11000,0.00841078720986843)
--(axis cs:11100,0.00840597786009312)
--(axis cs:11200,0.00838897936046124)
--(axis cs:11300,0.00835347175598145)
--(axis cs:11400,0.00828185118734837)
--(axis cs:11500,0.00827784556895494)
--(axis cs:11600,0.0082249641418457)
--(axis cs:11700,0.00817920360714197)
--(axis cs:11800,0.00819506403058767)
--(axis cs:11900,0.00818183459341526)
--(axis cs:12000,0.00817676912993193)
--(axis cs:12100,0.00812316592782736)
--(axis cs:12200,0.00811531767249107)
--(axis cs:12300,0.00805472396314144)
--(axis cs:12400,0.00801105424761772)
--(axis cs:12500,0.00797216966748238)
--(axis cs:12600,0.00797000527381897)
--(axis cs:12700,0.00795022211968899)
--(axis cs:12800,0.00794303510338068)
--(axis cs:12900,0.00794792175292969)
--(axis cs:13000,0.00792036391794682)
--(axis cs:13100,0.00788555666804314)
--(axis cs:13200,0.00785708427429199)
--(axis cs:13300,0.00781445484608412)
--(axis cs:13400,0.00776035943999887)
--(axis cs:13500,0.00774708157405257)
--(axis cs:13600,0.00775386998429894)
--(axis cs:13700,0.0077319392003119)
--(axis cs:13800,0.00771483406424522)
--(axis cs:13900,0.00768750580027699)
--(axis cs:14000,0.00769880134612322)
--(axis cs:14100,0.00765533465892076)
--(axis cs:14200,0.00760951219126582)
--(axis cs:14300,0.00758652854710817)
--(axis cs:14400,0.00756483059376478)
--(axis cs:14500,0.00749981077387929)
--(axis cs:14600,0.00749107683077455)
--(axis cs:14700,0.00751647725701332)
--(axis cs:14800,0.0074959802441299)
--(axis cs:14900,0.00748709868639708)
--(axis cs:15000,0.00748205184936523)
--(axis cs:15100,0.00743943825364113)
--(axis cs:15200,0.00739577645435929)
--(axis cs:15300,0.00737026613205671)
--(axis cs:15400,0.00732450466603041)
--(axis cs:15500,0.00732960691675544)
--(axis cs:15600,0.00734138488769531)
--(axis cs:15700,0.00732079707086086)
--(axis cs:15800,0.00730999745428562)
--(axis cs:15900,0.00729026785120368)
--(axis cs:16000,0.00725416000932455)
--(axis cs:16100,0.00720404461026192)
--(axis cs:16200,0.00717591494321823)
--(axis cs:16300,0.00715883914381266)
--(axis cs:16400,0.00721436971798539)
--(axis cs:16500,0.00719568924978375)
--(axis cs:16600,0.00719826994463801)
--(axis cs:16700,0.00718113174661994)
--(axis cs:16800,0.0071498267352581)
--(axis cs:16900,0.00709204701706767)
--(axis cs:17000,0.00711231352761388)
--(axis cs:17100,0.00710775004699826)
--(axis cs:17200,0.00712878024205565)
--(axis cs:17300,0.0071251867339015)
--(axis cs:17400,0.00711927423253655)
--(axis cs:17500,0.0071036284789443)
--(axis cs:17600,0.00706869876012206)
--(axis cs:17700,0.00706928502768278)
--(axis cs:17800,0.00703867571428418)
--(axis cs:17900,0.00702173914760351)
--(axis cs:18000,0.00699694408103824)
--(axis cs:18100,0.00699098501354456)
--(axis cs:18200,0.00695144524797797)
--(axis cs:18300,0.00691674137488008)
--(axis cs:18400,0.00689218798652291)
--(axis cs:18500,0.00688536372035742)
--(axis cs:18600,0.00688301911577582)
--(axis cs:18700,0.00689382385462523)
--(axis cs:18800,0.00690444838255644)
--(axis cs:18900,0.00690837763249874)
--(axis cs:19000,0.00689779920503497)
--(axis cs:19100,0.00688023492693901)
--(axis cs:19200,0.00687850220128894)
--(axis cs:19300,0.00687556760385633)
--(axis cs:19400,0.00686239078640938)
--(axis cs:19500,0.00684259226545691)
--(axis cs:19600,0.00682610226795077)
--(axis cs:19700,0.00682611484080553)
--(axis cs:19800,0.00678225141018629)
--(axis cs:19900,0.00678906450048089)
--(axis cs:20000,0.00676918029785156)
--(axis cs:20100,0.00673599867150187)
--(axis cs:20200,0.00670981407165527)
--(axis cs:20300,0.00672059040516615)
--(axis cs:20400,0.00669183721765876)
--(axis cs:20500,0.00669727334752679)
--(axis cs:20600,0.00670366268604994)
--(axis cs:20700,0.00664744386449456)
--(axis cs:20800,0.00663218507543206)
--(axis cs:20900,0.00660948734730482)
--(axis cs:21000,0.00661106128245592)
--(axis cs:21100,0.00661759357899427)
--(axis cs:21200,0.00663557043299079)
--(axis cs:21300,0.00658988952636719)
--(axis cs:21400,0.00658845901489258)
--(axis cs:21500,0.00655603408813477)
--(axis cs:21600,0.00654501933604479)
--(axis cs:21700,0.00655541429296136)
--(axis cs:21800,0.00655937194824219)
--(axis cs:21900,0.00655121821910143)
--(axis cs:22000,0.00654945382848382)
--(axis cs:22100,0.00650849333032966)
--(axis cs:22200,0.00648646336048841)
--(axis cs:22300,0.00649633398279548)
--(axis cs:22400,0.00645995140075684)
--(axis cs:22500,0.00646467227488756)
--(axis cs:22600,0.00647244462743402)
--(axis cs:22700,0.00646667461842299)
--(axis cs:22800,0.0064691542647779)
--(axis cs:22900,0.0064558507874608)
--(axis cs:23000,0.00646581640467048)
--(axis cs:23100,0.00642790785059333)
--(axis cs:23200,0.00640363711863756)
--(axis cs:23300,0.00639920216053724)
--(axis cs:23400,0.00635423650965095)
--(axis cs:23500,0.00636143703013659)
--(axis cs:23600,0.00638828286901116)
--(axis cs:23700,0.00638351449742913)
--(axis cs:23800,0.00635166186839342)
--(axis cs:23900,0.00634322175756097)
--(axis cs:24000,0.00631790142506361)
--(axis cs:24100,0.00630531320348382)
--(axis cs:24200,0.00628027925267816)
--(axis cs:24300,0.00627965945750475)
--(axis cs:24400,0.00627865782007575)
--(axis cs:24500,0.00632481556385756)
--(axis cs:24600,0.0063331127166748)
--(axis cs:24700,0.00630888948217034)
--(axis cs:24800,0.00628075608983636)
--(axis cs:24900,0.00627627363428473)
--(axis cs:25000,0.00624547014012933)
--(axis cs:25100,0.00621428480371833)
--(axis cs:25200,0.00622339267283678)
--(axis cs:25300,0.00621962547302246)
--(axis cs:25400,0.00617651920765638)
--(axis cs:25500,0.00613861065357924)
--(axis cs:25600,0.00611248007044196)
--(axis cs:25700,0.00609655398875475)
--(axis cs:25800,0.00611190777271986)
--(axis cs:25900,0.00613398570567369)
--(axis cs:26000,0.00615301122888923)
--(axis cs:26100,0.00614552479237318)
--(axis cs:26200,0.00616130838170648)
--(axis cs:26300,0.00610504159703851)
--(axis cs:26400,0.00611205119639635)
--(axis cs:26500,0.00609974842518568)
--(axis cs:26600,0.00612187385559082)
--(axis cs:26700,0.00609207153320312)
--(axis cs:26800,0.00610895175486803)
--(axis cs:26900,0.00609846133738756)
--(axis cs:27000,0.00608248729258776)
--(axis cs:27100,0.00608263025060296)
--(axis cs:27200,0.00608439464122057)
--(axis cs:27300,0.00606460589915514)
--(axis cs:27400,0.00604515057057142)
--(axis cs:27500,0.006012630648911)
--(axis cs:27600,0.00597839336842299)
--(axis cs:27700,0.0060126781463623)
--(axis cs:27800,0.00600185384973884)
--(axis cs:27900,0.00604710588231683)
--(axis cs:28000,0.00606708507984877)
--(axis cs:28100,0.00607876759022474)
--(axis cs:28200,0.00605406751856208)
--(axis cs:28300,0.00600781431421638)
--(axis cs:28400,0.00597372045740485)
--(axis cs:28500,0.00596423167735338)
--(axis cs:28600,0.00589852314442396)
--(axis cs:28700,0.00586962699890137)
--(axis cs:28800,0.00586962699890137)
--(axis cs:28900,0.00586962699890137)
--(axis cs:29000,0.00586962699890137)
--(axis cs:29100,0.00586962699890137)
--(axis cs:29200,0.00586962699890137)
--(axis cs:29300,0.00586962699890137)
--(axis cs:29400,0.00586962699890137)
--(axis cs:29500,0.00586962699890137)
--(axis cs:29600,0.00586962699890137)
--(axis cs:29700,0.00586962699890137)
--(axis cs:29800,0.00586962699890137)
--(axis cs:29900,0.00586962699890137)
--(axis cs:30000,0.00586962699890137)
--(axis cs:30100,0.00586962699890137)
--(axis cs:30200,0.00586962699890137)
--(axis cs:30300,0.00586962699890137)
--(axis cs:30400,0.00586962699890137)
--(axis cs:30400,0.00680618034675717)
--(axis cs:30400,0.00680618034675717)
--(axis cs:30300,0.00680519454181194)
--(axis cs:30200,0.00680339336395264)
--(axis cs:30100,0.00680307345464826)
--(axis cs:30000,0.00680376728996634)
--(axis cs:29900,0.00680395774543285)
--(axis cs:29800,0.00680351629853249)
--(axis cs:29700,0.00680292770266533)
--(axis cs:29600,0.00680841039866209)
--(axis cs:29500,0.00681035313755274)
--(axis cs:29400,0.00681691337376833)
--(axis cs:29300,0.0068219481036067)
--(axis cs:29200,0.00682665267959237)
--(axis cs:29100,0.00681893434375525)
--(axis cs:29000,0.00681679742410779)
--(axis cs:28900,0.00681161321699619)
--(axis cs:28800,0.00680893380194902)
--(axis cs:28700,0.00680827163159847)
--(axis cs:28600,0.00681248959153891)
--(axis cs:28500,0.00682251621037722)
--(axis cs:28400,0.00682880030944943)
--(axis cs:28300,0.00683867791667581)
--(axis cs:28200,0.00684615503996611)
--(axis cs:28100,0.00684823608025908)
--(axis cs:28000,0.00684164231643081)
--(axis cs:27900,0.00684214988723397)
--(axis cs:27800,0.0068357321433723)
--(axis cs:27700,0.00683506531640887)
--(axis cs:27600,0.00683228950947523)
--(axis cs:27500,0.00683529209345579)
--(axis cs:27400,0.00683677289634943)
--(axis cs:27300,0.00683995150029659)
--(axis cs:27200,0.00684288609772921)
--(axis cs:27100,0.00684427656233311)
--(axis cs:27000,0.00684519670903683)
--(axis cs:26900,0.00684589613229036)
--(axis cs:26800,0.00685000419616699)
--(axis cs:26700,0.00684454757720232)
--(axis cs:26600,0.00685066170990467)
--(axis cs:26500,0.00684921769425273)
--(axis cs:26400,0.00685421517118812)
--(axis cs:26300,0.00685153249651194)
--(axis cs:26200,0.0068633034825325)
--(axis cs:26100,0.00686630746349692)
--(axis cs:26000,0.0068733086809516)
--(axis cs:25900,0.00687126070261002)
--(axis cs:25800,0.00687388377264142)
--(axis cs:25700,0.0068721417337656)
--(axis cs:25600,0.00686814589425921)
--(axis cs:25500,0.00687062228098512)
--(axis cs:25400,0.00687291892245412)
--(axis cs:25300,0.00687442906200886)
--(axis cs:25200,0.00687346374616027)
--(axis cs:25100,0.00687964493408799)
--(axis cs:25000,0.00687833409756422)
--(axis cs:24900,0.00688449759036303)
--(axis cs:24800,0.00688654230907559)
--(axis cs:24700,0.00688771065324545)
--(axis cs:24600,0.00689282454550266)
--(axis cs:24500,0.00689405994489789)
--(axis cs:24400,0.00688763614743948)
--(axis cs:24300,0.00689318217337132)
--(axis cs:24200,0.00689812377095222)
--(axis cs:24100,0.00689811166375875)
--(axis cs:24000,0.00690383743494749)
--(axis cs:23900,0.0069077811203897)
--(axis cs:23800,0.00690534897148609)
--(axis cs:23700,0.00690628448501229)
--(axis cs:23600,0.00690426724031568)
--(axis cs:23500,0.00690383417531848)
--(axis cs:23400,0.00690954877063632)
--(axis cs:23300,0.00691248569637537)
--(axis cs:23200,0.00691372016444802)
--(axis cs:23100,0.00691669154912233)
--(axis cs:23000,0.00691855559125543)
--(axis cs:22900,0.00692102592438459)
--(axis cs:22800,0.00691938027739525)
--(axis cs:22700,0.00692318379878998)
--(axis cs:22600,0.00692597264423966)
--(axis cs:22500,0.00692754238843918)
--(axis cs:22400,0.00693544512614608)
--(axis cs:22300,0.00693489564582705)
--(axis cs:22200,0.00693235686048865)
--(axis cs:22100,0.00693506561219692)
--(axis cs:22000,0.00693991128355265)
--(axis cs:21900,0.00693983305245638)
--(axis cs:21800,0.00694178696721792)
--(axis cs:21700,0.00694312667474151)
--(axis cs:21600,0.00694181537255645)
--(axis cs:21500,0.00694055063650012)
--(axis cs:21400,0.00694113364443183)
--(axis cs:21300,0.0069435597397387)
--(axis cs:21200,0.00695066805928946)
--(axis cs:21100,0.00694889528676867)
--(axis cs:21000,0.0069519761018455)
--(axis cs:20900,0.00695595610886812)
--(axis cs:20800,0.00695722689852118)
--(axis cs:20700,0.0069634816609323)
--(axis cs:20600,0.00696854898706079)
--(axis cs:20500,0.00696797296404839)
--(axis cs:20400,0.00696876691654325)
--(axis cs:20300,0.00697500770911574)
--(axis cs:20200,0.00697367358952761)
--(axis cs:20100,0.00698158936575055)
--(axis cs:20000,0.00698174675926566)
--(axis cs:19900,0.00698623666539788)
--(axis cs:19800,0.00699233449995518)
--(axis cs:19700,0.00698935240507126)
--(axis cs:19600,0.00700141256675124)
--(axis cs:19500,0.00700892368331552)
--(axis cs:19400,0.00702034216374159)
--(axis cs:19300,0.0070073870010674)
--(axis cs:19200,0.00702235056087375)
--(axis cs:19100,0.00700930040329695)
--(axis cs:19000,0.0070216809399426)
--(axis cs:18900,0.00702619552612305)
--(axis cs:18800,0.00705757131800056)
--(axis cs:18700,0.00709705520421267)
--(axis cs:18600,0.00710719218477607)
--(axis cs:18500,0.00711969379335642)
--(axis cs:18400,0.00709490897133946)
--(axis cs:18300,0.00706820469349623)
--(axis cs:18200,0.00702619552612305)
--(axis cs:18100,0.00703792553395033)
--(axis cs:18000,0.00702776899561286)
--(axis cs:17900,0.00704736728221178)
--(axis cs:17800,0.00708571774885058)
--(axis cs:17700,0.00709848385304213)
--(axis cs:17600,0.00713456375524402)
--(axis cs:17500,0.00714769959449768)
--(axis cs:17400,0.00715639442205429)
--(axis cs:17300,0.00713947787880898)
--(axis cs:17200,0.00715031614527106)
--(axis cs:17100,0.00715222349390388)
--(axis cs:17000,0.00717884534969926)
--(axis cs:16900,0.00722551345825195)
--(axis cs:16800,0.00726496055722237)
--(axis cs:16700,0.007254000287503)
--(axis cs:16600,0.0072748507373035)
--(axis cs:16500,0.00731732649728656)
--(axis cs:16400,0.00730074429884553)
--(axis cs:16300,0.00733062066137791)
--(axis cs:16200,0.00735750887542963)
--(axis cs:16100,0.00734021980315447)
--(axis cs:16000,0.00733294477686286)
--(axis cs:15900,0.00735705671831965)
--(axis cs:15800,0.00733642559498549)
--(axis cs:15700,0.00735532958060503)
--(axis cs:15600,0.00736895576119423)
--(axis cs:15500,0.00739146396517754)
--(axis cs:15400,0.00744504481554031)
--(axis cs:15300,0.00748283043503761)
--(axis cs:15200,0.00747804576531053)
--(axis cs:15100,0.00753200892359018)
--(axis cs:15000,0.00751964747905731)
--(axis cs:14900,0.00752363912761211)
--(axis cs:14800,0.00752763403579593)
--(axis cs:14700,0.00754294404760003)
--(axis cs:14600,0.00756636029109359)
--(axis cs:14500,0.00759110460057855)
--(axis cs:14400,0.0076126460917294)
--(axis cs:14300,0.00764517672359943)
--(axis cs:14200,0.00766068836674094)
--(axis cs:14100,0.00768190901726484)
--(axis cs:14000,0.00771438889205456)
--(axis cs:13900,0.00772396707907319)
--(axis cs:13800,0.00780001655220985)
--(axis cs:13700,0.0077975750900805)
--(axis cs:13600,0.00783543009310961)
--(axis cs:13500,0.00790242943912745)
--(axis cs:13400,0.00794703885912895)
--(axis cs:13300,0.00789913721382618)
--(axis cs:13200,0.00796949397772551)
--(axis cs:13100,0.00797528587281704)
--(axis cs:13000,0.00796883553266525)
--(axis cs:12900,0.00801739562302828)
--(axis cs:12800,0.00802528951317072)
--(axis cs:12700,0.00807026773691177)
--(axis cs:12600,0.00809737108647823)
--(axis cs:12500,0.008087158203125)
--(axis cs:12400,0.00811796169728041)
--(axis cs:12300,0.0081805232912302)
--(axis cs:12200,0.00819945335388184)
--(axis cs:12100,0.00821065902709961)
--(axis cs:12000,0.00824675522744656)
--(axis cs:11900,0.00827126484364271)
--(axis cs:11800,0.0082700913771987)
--(axis cs:11700,0.00830178428441286)
--(axis cs:11600,0.00839497987180948)
--(axis cs:11500,0.00842467602342367)
--(axis cs:11400,0.00842657312750816)
--(axis cs:11300,0.0084508340805769)
--(axis cs:11200,0.00846203416585922)
--(axis cs:11100,0.00843081437051296)
--(axis cs:11000,0.00846766401082277)
--(axis cs:10900,0.00852099433541298)
--(axis cs:10800,0.00857131276279688)
--(axis cs:10700,0.00859530735760927)
--(axis cs:10600,0.00863382127135992)
--(axis cs:10500,0.00861503463238478)
--(axis cs:10400,0.00863938964903355)
--(axis cs:10300,0.00867146532982588)
--(axis cs:10200,0.0087111433967948)
--(axis cs:10100,0.00876222644001245)
--(axis cs:10000,0.0088041303679347)
--(axis cs:9900,0.00884761847555637)
--(axis cs:9800,0.00888233166188002)
--(axis cs:9700,0.00894193816930056)
--(axis cs:9600,0.00897412747144699)
--(axis cs:9500,0.00902276486158371)
--(axis cs:9400,0.00908310990780592)
--(axis cs:9300,0.00910678971558809)
--(axis cs:9200,0.00914421118795872)
--(axis cs:9100,0.00917877350002527)
--(axis cs:9000,0.0092154499143362)
--(axis cs:8900,0.00926203746348619)
--(axis cs:8800,0.00934122782200575)
--(axis cs:8700,0.00940224342048168)
--(axis cs:8600,0.00942602753639221)
--(axis cs:8500,0.0095024798065424)
--(axis cs:8400,0.00956587679684162)
--(axis cs:8300,0.00961537379771471)
--(axis cs:8200,0.0096556656062603)
--(axis cs:8100,0.00970613956451416)
--(axis cs:8000,0.00981700979173183)
--(axis cs:7900,0.00987306423485279)
--(axis cs:7800,0.0098628206178546)
--(axis cs:7700,0.00992436241358519)
--(axis cs:7600,0.00999546144157648)
--(axis cs:7500,0.0100149633362889)
--(axis cs:7400,0.0101019144058228)
--(axis cs:7300,0.0101523157209158)
--(axis cs:7200,0.0101942485198379)
--(axis cs:7100,0.010236781090498)
--(axis cs:7000,0.0102639170363545)
--(axis cs:6900,0.0103161102160811)
--(axis cs:6800,0.0104055153205991)
--(axis cs:6700,0.0104808509349823)
--(axis cs:6600,0.0105427661910653)
--(axis cs:6500,0.0106602907180786)
--(axis cs:6400,0.0107465982437134)
--(axis cs:6300,0.0108617544174194)
--(axis cs:6200,0.0109682800248265)
--(axis cs:6100,0.0109872091561556)
--(axis cs:6000,0.0110870404168963)
--(axis cs:5900,0.0112245623022318)
--(axis cs:5800,0.0113101406022906)
--(axis cs:5700,0.0114040626212955)
--(axis cs:5600,0.011522326618433)
--(axis cs:5500,0.0116109661757946)
--(axis cs:5400,0.0116998655721545)
--(axis cs:5300,0.011818116530776)
--(axis cs:5200,0.0119392452761531)
--(axis cs:5100,0.0121285384520888)
--(axis cs:5000,0.0122660491615534)
--(axis cs:4900,0.0124231390655041)
--(axis cs:4800,0.0125930495560169)
--(axis cs:4700,0.0127431964501739)
--(axis cs:4600,0.0128848413005471)
--(axis cs:4500,0.0130982156842947)
--(axis cs:4400,0.0132982013747096)
--(axis cs:4300,0.0135007658973336)
--(axis cs:4200,0.0137696610763669)
--(axis cs:4100,0.0140824858099222)
--(axis cs:4000,0.0144160836935043)
--(axis cs:3900,0.0147873442620039)
--(axis cs:3800,0.0151412114500999)
--(axis cs:3700,0.0155271738767624)
--(axis cs:3600,0.0158979017287493)
--(axis cs:3500,0.0163123495876789)
--(axis cs:3400,0.0166979525238276)
--(axis cs:3300,0.0170717183500528)
--(axis cs:3200,0.0174731034785509)
--(axis cs:3100,0.0178576372563839)
--(axis cs:3000,0.0182927809655666)
--(axis cs:2900,0.0188154391944408)
--(axis cs:2800,0.0194802042096853)
--(axis cs:2700,0.0203478150069714)
--(axis cs:2600,0.0214035753160715)
--(axis cs:2500,0.0224937796592712)
--(axis cs:2400,0.0235886592417955)
--(axis cs:2300,0.0249193906784058)
--(axis cs:2200,0.0267025306820869)
--(axis cs:2100,0.0289442576467991)
--(axis cs:2000,0.031578965485096)
--(axis cs:1900,0.0345292389392853)
--(axis cs:1800,0.0373213961720467)
--(axis cs:1700,0.0399247892200947)
--(axis cs:1600,0.0421821065247059)
--(axis cs:1500,0.0441334955394268)
--(axis cs:1400,0.0460115931928158)
--(axis cs:1300,0.0477711781859398)
--(axis cs:1200,0.0492039807140827)
--(axis cs:1100,0.0503541566431522)
--(axis cs:1000,0.0511730425059795)
--(axis cs:900,0.0515283420681953)
--(axis cs:800,0.0516600236296654)
--(axis cs:700,0.0518020577728748)
--(axis cs:600,0.0520781837403774)
--(axis cs:500,0.0527633503079414)
--(axis cs:400,0.0543137490749359)
--(axis cs:300,0.056662742048502)
--(axis cs:200,0.0592069700360298)
--(axis cs:100,0.0616600550711155)
--(axis cs:0,0.0637036859989166)
--cycle;

\path [fill=color0, fill opacity=0.4, ultra thick]
(axis cs:0,0.0487950257956982)
--(axis cs:0,0.048629354685545)
--(axis cs:100,0.0425903834402561)
--(axis cs:200,0.0358326621353626)
--(axis cs:300,0.0322679057717323)
--(axis cs:400,0.0296411383897066)
--(axis cs:500,0.0268500093370676)
--(axis cs:600,0.0239638518542051)
--(axis cs:700,0.0221002344042063)
--(axis cs:800,0.0210253950208426)
--(axis cs:900,0.0199772603809834)
--(axis cs:1000,0.0189599748700857)
--(axis cs:1100,0.0181993190199137)
--(axis cs:1200,0.0174159165471792)
--(axis cs:1300,0.0166514068841934)
--(axis cs:1400,0.0159712340682745)
--(axis cs:1500,0.0153839690610766)
--(axis cs:1600,0.0148046240210533)
--(axis cs:1700,0.014320963062346)
--(axis cs:1800,0.0139094097539783)
--(axis cs:1900,0.0135928550735116)
--(axis cs:2000,0.0132493302226067)
--(axis cs:2100,0.0130304284393787)
--(axis cs:2200,0.0127656832337379)
--(axis cs:2300,0.0126054286956787)
--(axis cs:2400,0.0123540880158544)
--(axis cs:2500,0.0121608413755894)
--(axis cs:2600,0.011988771148026)
--(axis cs:2700,0.0119153903797269)
--(axis cs:2800,0.0117283780127764)
--(axis cs:2900,0.0115924319252372)
--(axis cs:3000,0.0114399464800954)
--(axis cs:3100,0.0113275982439518)
--(axis cs:3200,0.011183762922883)
--(axis cs:3300,0.0110980747267604)
--(axis cs:3400,0.0109866783022881)
--(axis cs:3500,0.0108873844146729)
--(axis cs:3600,0.0107817053794861)
--(axis cs:3700,0.0106692845001817)
--(axis cs:3800,0.0106248613446951)
--(axis cs:3900,0.0105391638353467)
--(axis cs:4000,0.0104595050215721)
--(axis cs:4100,0.0104005625471473)
--(axis cs:4200,0.0103146806359291)
--(axis cs:4300,0.0102438535541296)
--(axis cs:4400,0.010179559700191)
--(axis cs:4500,0.010112164542079)
--(axis cs:4600,0.0100308721885085)
--(axis cs:4700,0.00996671337634325)
--(axis cs:4800,0.00991099141538143)
--(axis cs:4900,0.00983161572366953)
--(axis cs:5000,0.00978424865752459)
--(axis cs:5100,0.00970828905701637)
--(axis cs:5200,0.00964848976582289)
--(axis cs:5300,0.00956210121512413)
--(axis cs:5400,0.00952408835291862)
--(axis cs:5500,0.00950355548411608)
--(axis cs:5600,0.00945037603378296)
--(axis cs:5700,0.00940935779362917)
--(axis cs:5800,0.0093857403844595)
--(axis cs:5900,0.00934929586946964)
--(axis cs:6000,0.00929865427315235)
--(axis cs:6100,0.00925660040229559)
--(axis cs:6200,0.00918538589030504)
--(axis cs:6300,0.00912001170217991)
--(axis cs:6400,0.0090666376054287)
--(axis cs:6500,0.00904356595128775)
--(axis cs:6600,0.00901827123016119)
--(axis cs:6700,0.0089785810559988)
--(axis cs:6800,0.00892381649464369)
--(axis cs:6900,0.00889419391751289)
--(axis cs:7000,0.00887663848698139)
--(axis cs:7100,0.00886866543442011)
--(axis cs:7200,0.00884649716317654)
--(axis cs:7300,0.0088197709992528)
--(axis cs:7400,0.00877709407359362)
--(axis cs:7500,0.00875394325703382)
--(axis cs:7600,0.00869183707982302)
--(axis cs:7700,0.00870625954121351)
--(axis cs:7800,0.00868376810103655)
--(axis cs:7900,0.00864872243255377)
--(axis cs:8000,0.00859700888395309)
--(axis cs:8100,0.00856242142617702)
--(axis cs:8200,0.00850940681993961)
--(axis cs:8300,0.00848625972867012)
--(axis cs:8400,0.00845228787511587)
--(axis cs:8500,0.00843879766762257)
--(axis cs:8600,0.00842626113444567)
--(axis cs:8700,0.00839195679873228)
--(axis cs:8800,0.00836566742509604)
--(axis cs:8900,0.00833487696945667)
--(axis cs:9000,0.00833966769278049)
--(axis cs:9100,0.00828318577259779)
--(axis cs:9200,0.0082489000633359)
--(axis cs:9300,0.00820619240403175)
--(axis cs:9400,0.00819161627441645)
--(axis cs:9500,0.00814506970345974)
--(axis cs:9600,0.00811932049691677)
--(axis cs:9700,0.00811350345611572)
--(axis cs:9800,0.00805970560759306)
--(axis cs:9900,0.00802341289818287)
--(axis cs:10000,0.00800802744925022)
--(axis cs:10100,0.00798420887440443)
--(axis cs:10200,0.00796267949044704)
--(axis cs:10300,0.0079263923689723)
--(axis cs:10400,0.0079063419252634)
--(axis cs:10500,0.0078976396471262)
--(axis cs:10600,0.00789041537791491)
--(axis cs:10700,0.00789506454020739)
--(axis cs:10800,0.00783126801252365)
--(axis cs:10900,0.00783181190490723)
--(axis cs:11000,0.00779289705678821)
--(axis cs:11100,0.00774736423045397)
--(axis cs:11200,0.00773830432444811)
--(axis cs:11300,0.00773878116160631)
--(axis cs:11400,0.00768057256937027)
--(axis cs:11500,0.00766446581110358)
--(axis cs:11600,0.00764429569244385)
--(axis cs:11700,0.00761656742542982)
--(axis cs:11800,0.00758202094584703)
--(axis cs:11900,0.00758399954065681)
--(axis cs:12000,0.00758855324238539)
--(axis cs:12100,0.00756383547559381)
--(axis cs:12200,0.00754580507054925)
--(axis cs:12300,0.00753645459190011)
--(axis cs:12400,0.00748999183997512)
--(axis cs:12500,0.00746054155752063)
--(axis cs:12600,0.00742542650550604)
--(axis cs:12700,0.00741562899202108)
--(axis cs:12800,0.00741031160578132)
--(axis cs:12900,0.0074401618912816)
--(axis cs:13000,0.00741944322362542)
--(axis cs:13100,0.00740952510386705)
--(axis cs:13200,0.00739088049158454)
--(axis cs:13300,0.00735251884907484)
--(axis cs:13400,0.00730678020045161)
--(axis cs:13500,0.00729226740077138)
--(axis cs:13600,0.00727970292791724)
--(axis cs:13700,0.00726479012519121)
--(axis cs:13800,0.00724495621398091)
--(axis cs:13900,0.00724936369806528)
--(axis cs:14000,0.00725152622908354)
--(axis cs:14100,0.00721871387213469)
--(axis cs:14200,0.00717947306111455)
--(axis cs:14300,0.00717320898547769)
--(axis cs:14400,0.0071441913023591)
--(axis cs:14500,0.00710551673546433)
--(axis cs:14600,0.00713607203215361)
--(axis cs:14700,0.00710894074290991)
--(axis cs:14800,0.00711694406345487)
--(axis cs:14900,0.00711003970354795)
--(axis cs:15000,0.00710693653672934)
--(axis cs:15100,0.00706619722768664)
--(axis cs:15200,0.00702973082661629)
--(axis cs:15300,0.00701700802892447)
--(axis cs:15400,0.00700150290504098)
--(axis cs:15500,0.00701642408967018)
--(axis cs:15600,0.00699433730915189)
--(axis cs:15700,0.00697788083925843)
--(axis cs:15800,0.00698116468265653)
--(axis cs:15900,0.00697905430570245)
--(axis cs:16000,0.00693949498236179)
--(axis cs:16100,0.00692489137873054)
--(axis cs:16200,0.00691823940724134)
--(axis cs:16300,0.00688695115968585)
--(axis cs:16400,0.00687217712402344)
--(axis cs:16500,0.00686378497630358)
--(axis cs:16600,0.00686823157593608)
--(axis cs:16700,0.00686463294550776)
--(axis cs:16800,0.00685898680239916)
--(axis cs:16900,0.00687061669304967)
--(axis cs:17000,0.0068803308531642)
--(axis cs:17100,0.00685529690235853)
--(axis cs:17200,0.0068522454239428)
--(axis cs:17300,0.00681436061859131)
--(axis cs:17400,0.00680170068517327)
--(axis cs:17500,0.00678095826879144)
--(axis cs:17600,0.00678722839802504)
--(axis cs:17700,0.00676970463246107)
--(axis cs:17800,0.00677111139521003)
--(axis cs:17900,0.00673153391107917)
--(axis cs:18000,0.00671780109405518)
--(axis cs:18100,0.00668911915272474)
--(axis cs:18200,0.0066691399551928)
--(axis cs:18300,0.00664226990193129)
--(axis cs:18400,0.0066446540877223)
--(axis cs:18500,0.00663094501942396)
--(axis cs:18600,0.0066535472869873)
--(axis cs:18700,0.00663735857233405)
--(axis cs:18800,0.00665199756622314)
--(axis cs:18900,0.0066337650641799)
--(axis cs:19000,0.00662564625963569)
--(axis cs:19100,0.00658912677317858)
--(axis cs:19200,0.00659799575805664)
--(axis cs:19300,0.00657196063548326)
--(axis cs:19400,0.0065452097915113)
--(axis cs:19500,0.0065624238923192)
--(axis cs:19600,0.00655088433995843)
--(axis cs:19700,0.00655388832092285)
--(axis cs:19800,0.00654449453577399)
--(axis cs:19900,0.00655112275853753)
--(axis cs:20000,0.00652060518041253)
--(axis cs:20100,0.00651860237121582)
--(axis cs:20200,0.00651373853906989)
--(axis cs:20300,0.00651788711547852)
--(axis cs:20400,0.00651340465992689)
--(axis cs:20500,0.00646762829273939)
--(axis cs:20600,0.00647521018981934)
--(axis cs:20700,0.00644521694630384)
--(axis cs:20800,0.00643229484558105)
--(axis cs:20900,0.00641841907054186)
--(axis cs:21000,0.00641264906153083)
--(axis cs:21100,0.00638670939952135)
--(axis cs:21200,0.00641841907054186)
--(axis cs:21300,0.00644340505823493)
--(axis cs:21400,0.00646753329783678)
--(axis cs:21500,0.006439876742661)
--(axis cs:21600,0.00643353443592787)
--(axis cs:21700,0.00642824172973633)
--(axis cs:21800,0.00640988349914551)
--(axis cs:21900,0.00638389587402344)
--(axis cs:22000,0.00639939308166504)
--(axis cs:22100,0.00638508796691895)
--(axis cs:22200,0.00637631397694349)
--(axis cs:22300,0.00635781278833747)
--(axis cs:22400,0.00635724049061537)
--(axis cs:22500,0.0063323020003736)
--(axis cs:22600,0.00631151208654046)
--(axis cs:22700,0.00631580362096429)
--(axis cs:22800,0.00631403923034668)
--(axis cs:22900,0.0062711713835597)
--(axis cs:23000,0.00626158714294434)
--(axis cs:23100,0.00626249331980944)
--(axis cs:23200,0.00625009555369616)
--(axis cs:23300,0.0062402724288404)
--(axis cs:23400,0.0062397001311183)
--(axis cs:23500,0.0062244413420558)
--(axis cs:23600,0.00624947529286146)
--(axis cs:23700,0.00626001367345452)
--(axis cs:23800,0.00622797012329102)
--(axis cs:23900,0.00622858991846442)
--(axis cs:24000,0.00624403962865472)
--(axis cs:24100,0.00620822887867689)
--(axis cs:24200,0.00617251405492425)
--(axis cs:24300,0.00617852201685309)
--(axis cs:24400,0.0061799050308764)
--(axis cs:24500,0.0061952592805028)
--(axis cs:24600,0.00617904681712389)
--(axis cs:24700,0.00618939381092787)
--(axis cs:24800,0.00618629436939955)
--(axis cs:24900,0.00619616499170661)
--(axis cs:25000,0.00615673046559095)
--(axis cs:25100,0.00616712588816881)
--(axis cs:25200,0.00614318856969476)
--(axis cs:25300,0.00615339260548353)
--(axis cs:25400,0.00612487085163593)
--(axis cs:25500,0.00612589996308088)
--(axis cs:25600,0.00612058583647013)
--(axis cs:25700,0.00610326603055)
--(axis cs:25800,0.00607524299994111)
--(axis cs:25900,0.00609194999560714)
--(axis cs:26000,0.00609895773231983)
--(axis cs:26100,0.00608359789475799)
--(axis cs:26200,0.00609194999560714)
--(axis cs:26300,0.00609240913763642)
--(axis cs:26400,0.00607309071347117)
--(axis cs:26500,0.00606232881546021)
--(axis cs:26600,0.00606499053537846)
--(axis cs:26700,0.00604886654764414)
--(axis cs:26800,0.00604299595579505)
--(axis cs:26900,0.0060273939743638)
--(axis cs:27000,0.00600355491042137)
--(axis cs:27100,0.00601628236472607)
--(axis cs:27200,0.00603239145129919)
--(axis cs:27300,0.00603869277983904)
--(axis cs:27400,0.00603882735595107)
--(axis cs:27500,0.00603353884071112)
--(axis cs:27600,0.00602705590426922)
--(axis cs:27700,0.00602827221155167)
--(axis cs:27800,0.00602955650538206)
--(axis cs:27900,0.0060479617677629)
--(axis cs:28000,0.00604091212153435)
--(axis cs:28100,0.00601987820118666)
--(axis cs:28200,0.00600133696570992)
--(axis cs:28300,0.00600604387000203)
--(axis cs:28400,0.00597369764000177)
--(axis cs:28500,0.00598981138318777)
--(axis cs:28600,0.00598837155848742)
--(axis cs:28700,0.00599867384880781)
--(axis cs:28800,0.00597992585971951)
--(axis cs:28900,0.00599289406090975)
--(axis cs:29000,0.00596372643485665)
--(axis cs:29100,0.00598411727696657)
--(axis cs:29200,0.00597958220168948)
--(axis cs:29300,0.00595729425549507)
--(axis cs:29400,0.00595050305128098)
--(axis cs:29500,0.00598157569766045)
--(axis cs:29600,0.00594915030524135)
--(axis cs:29700,0.00592750543728471)
--(axis cs:29800,0.00594446295872331)
--(axis cs:29900,0.00591845624148846)
--(axis cs:30000,0.00588985299691558)
--(axis cs:30100,0.00588816264644265)
--(axis cs:30200,0.00587033992633224)
--(axis cs:30300,0.00586241390556097)
--(axis cs:30400,0.00589474523440003)
--(axis cs:30500,0.00589365419000387)
--(axis cs:30600,0.00589284533634782)
--(axis cs:30700,0.00589931523427367)
--(axis cs:30800,0.00588883180171251)
--(axis cs:30900,0.00587429851293564)
--(axis cs:31000,0.00586935039609671)
--(axis cs:31100,0.00586432591080666)
--(axis cs:31200,0.00586871337145567)
--(axis cs:31300,0.00586574152112007)
--(axis cs:31300,0.00685878470540047)
--(axis cs:31300,0.00685878470540047)
--(axis cs:31200,0.00685848388820887)
--(axis cs:31100,0.00685892906039953)
--(axis cs:31000,0.00685841962695122)
--(axis cs:30900,0.0068579213693738)
--(axis cs:30800,0.00685648526996374)
--(axis cs:30700,0.00685547525063157)
--(axis cs:30600,0.00685609551146626)
--(axis cs:30500,0.00685601774603128)
--(axis cs:30400,0.00685591297224164)
--(axis cs:30300,0.0068591246381402)
--(axis cs:30200,0.00685831857845187)
--(axis cs:30100,0.00685654999688268)
--(axis cs:30000,0.00685638515278697)
--(axis cs:29900,0.00685369037091732)
--(axis cs:29800,0.00685139885172248)
--(axis cs:29700,0.00685287499800324)
--(axis cs:29600,0.00685100303962827)
--(axis cs:29500,0.00684842746704817)
--(axis cs:29400,0.00685088988393545)
--(axis cs:29300,0.00685032922774553)
--(axis cs:29200,0.00684857694432139)
--(axis cs:29100,0.00684823840856552)
--(axis cs:29000,0.00684980908408761)
--(axis cs:28900,0.00684759952127934)
--(axis cs:28800,0.0068485508672893)
--(axis cs:28700,0.00684719253331423)
--(axis cs:28600,0.00684792548418045)
--(axis cs:28500,0.00684782117605209)
--(axis cs:28400,0.00684902630746365)
--(axis cs:28300,0.00684668822214007)
--(axis cs:28200,0.00684700766578317)
--(axis cs:28100,0.00684579182416201)
--(axis cs:28000,0.00684456247836351)
--(axis cs:27900,0.00684418855234981)
--(axis cs:27800,0.00684520602226257)
--(axis cs:27700,0.00684528145939112)
--(axis cs:27600,0.00684535410255194)
--(axis cs:27500,0.00684497505426407)
--(axis cs:27400,0.0068446765653789)
--(axis cs:27300,0.00684468448162079)
--(axis cs:27200,0.00684504024684429)
--(axis cs:27100,0.00684601906687021)
--(axis cs:27000,0.00684685632586479)
--(axis cs:26900,0.00684533454477787)
--(axis cs:26800,0.0068444493226707)
--(axis cs:26700,0.00684414245188236)
--(axis cs:26600,0.00684337224811316)
--(axis cs:26500,0.00684349145740271)
--(axis cs:26400,0.00684302998706698)
--(axis cs:26300,0.00684233894571662)
--(axis cs:26200,0.00684235384687781)
--(axis cs:26100,0.00684263044968247)
--(axis cs:26000,0.00684214849025011)
--(axis cs:25900,0.00684235384687781)
--(axis cs:25800,0.00684294337406754)
--(axis cs:25700,0.00684203580021858)
--(axis cs:25600,0.00684169214218855)
--(axis cs:25500,0.00684162322431803)
--(axis cs:25400,0.0068416353315115)
--(axis cs:25300,0.00684154685586691)
--(axis cs:25200,0.00684152776375413)
--(axis cs:25100,0.00684162555262446)
--(axis cs:25000,0.00684155989438295)
--(axis cs:24900,0.00684200879186392)
--(axis cs:24800,0.00684184534475207)
--(axis cs:24700,0.00684189330786467)
--(axis cs:24600,0.00684174662455916)
--(axis cs:24500,0.00684199202805758)
--(axis cs:24400,0.00684175733476877)
--(axis cs:24300,0.00684174057096243)
--(axis cs:24200,0.00684167444705963)
--(axis cs:24100,0.0068422588519752)
--(axis cs:24000,0.00684333546087146)
--(axis cs:23900,0.00684280740097165)
--(axis cs:23800,0.00684278830885887)
--(axis cs:23700,0.00684398785233498)
--(axis cs:23600,0.00684354593977332)
--(axis cs:23500,0.00684268260374665)
--(axis cs:23400,0.00684317760169506)
--(axis cs:23300,0.0068431980907917)
--(axis cs:23200,0.00684356968849897)
--(axis cs:23100,0.00684409961104393)
--(axis cs:23000,0.00684405863285065)
--(axis cs:22900,0.00684451125562191)
--(axis cs:22800,0.00684706494212151)
--(axis cs:22700,0.00684718927368522)
--(axis cs:22600,0.0068468889221549)
--(axis cs:22500,0.0068484335206449)
--(axis cs:22400,0.00685102120041847)
--(axis cs:22300,0.00685156462714076)
--(axis cs:22200,0.00685385940596461)
--(axis cs:22100,0.00685791065916419)
--(axis cs:22000,0.00686048809438944)
--(axis cs:21900,0.00685680378228426)
--(axis cs:21800,0.00686061894521117)
--(axis cs:21700,0.00686425669118762)
--(axis cs:21600,0.00686814822256565)
--(axis cs:21500,0.00687059108167887)
--(axis cs:21400,0.00687263533473015)
--(axis cs:21300,0.00686806859448552)
--(axis cs:21200,0.00686535751447082)
--(axis cs:21100,0.00685850949957967)
--(axis cs:21000,0.00686125038191676)
--(axis cs:20900,0.00686386320739985)
--(axis cs:20800,0.00686691189184785)
--(axis cs:20700,0.00687206024304032)
--(axis cs:20600,0.00687845330685377)
--(axis cs:20500,0.00687720300629735)
--(axis cs:20400,0.00688099442049861)
--(axis cs:20300,0.00688225077465177)
--(axis cs:20200,0.00688097160309553)
--(axis cs:20100,0.00688423356041312)
--(axis cs:20000,0.00688360305503011)
--(axis cs:19900,0.00688777305185795)
--(axis cs:19800,0.00688679981976748)
--(axis cs:19700,0.00688942521810532)
--(axis cs:19600,0.00689151789993048)
--(axis cs:19500,0.00689552025869489)
--(axis cs:19400,0.00689194351434708)
--(axis cs:19300,0.00690188352018595)
--(axis cs:19200,0.00691154366359115)
--(axis cs:19100,0.00690960139036179)
--(axis cs:19000,0.00691692670807242)
--(axis cs:18900,0.00692056957632303)
--(axis cs:18800,0.0069130090996623)
--(axis cs:18700,0.00690589565783739)
--(axis cs:18600,0.00690960418432951)
--(axis cs:18500,0.00690615642815828)
--(axis cs:18400,0.006911251693964)
--(axis cs:18300,0.00691266497597098)
--(axis cs:18200,0.00691762054339051)
--(axis cs:18100,0.00692132348194718)
--(axis cs:18000,0.00692610489204526)
--(axis cs:17900,0.00692688627168536)
--(axis cs:17800,0.00693369749933481)
--(axis cs:17700,0.00693205138668418)
--(axis cs:17600,0.00693516293540597)
--(axis cs:17500,0.00693432847037911)
--(axis cs:17400,0.00693860603496432)
--(axis cs:17300,0.00694237509742379)
--(axis cs:17200,0.00694820517674088)
--(axis cs:17100,0.00694858096539974)
--(axis cs:17000,0.00695458659902215)
--(axis cs:16900,0.0069570573978126)
--(axis cs:16800,0.00695490650832653)
--(axis cs:16700,0.00694778235629201)
--(axis cs:16600,0.00694995326921344)
--(axis cs:16500,0.00694509129971266)
--(axis cs:16400,0.00694220652803779)
--(axis cs:16300,0.00695037143304944)
--(axis cs:16200,0.00695663783699274)
--(axis cs:16100,0.0069870101287961)
--(axis cs:16000,0.00700664054602385)
--(axis cs:15900,0.00703346729278564)
--(axis cs:15800,0.00703204656019807)
--(axis cs:15700,0.00704294303432107)
--(axis cs:15600,0.0070369285531342)
--(axis cs:15500,0.007033821195364)
--(axis cs:15400,0.00705683277919888)
--(axis cs:15300,0.00708681717514992)
--(axis cs:15200,0.00712904939427972)
--(axis cs:15100,0.00713546294718981)
--(axis cs:15000,0.00714412052184343)
--(axis cs:14900,0.0071481941267848)
--(axis cs:14800,0.00716171273961663)
--(axis cs:14700,0.00715939421206713)
--(axis cs:14600,0.00714157614856958)
--(axis cs:14500,0.00719118909910321)
--(axis cs:14400,0.00720639247447252)
--(axis cs:14300,0.00725531578063965)
--(axis cs:14200,0.00726492423564196)
--(axis cs:14100,0.00726276729255915)
--(axis cs:14000,0.00726703740656376)
--(axis cs:13900,0.00729024410247803)
--(axis cs:13800,0.0072992448695004)
--(axis cs:13700,0.00733289727941155)
--(axis cs:13600,0.00736005324870348)
--(axis cs:13500,0.00740097695961595)
--(axis cs:13400,0.00742184510454535)
--(axis cs:13300,0.00747497379779816)
--(axis cs:13200,0.00748876994475722)
--(axis cs:13100,0.00750908674672246)
--(axis cs:13000,0.00752719352021813)
--(axis cs:12900,0.00753316236659884)
--(axis cs:12800,0.00752022257074714)
--(axis cs:12700,0.00753671303391457)
--(axis cs:12600,0.0075503122061491)
--(axis cs:12500,0.00755246868357062)
--(axis cs:12400,0.00757865095511079)
--(axis cs:12300,0.00760956248268485)
--(axis cs:12200,0.0076560340821743)
--(axis cs:12100,0.00769981788471341)
--(axis cs:12000,0.00771000003442168)
--(axis cs:11900,0.00771084753796458)
--(axis cs:11800,0.0077040153555572)
--(axis cs:11700,0.0077028046362102)
--(axis cs:11600,0.0077107478864491)
--(axis cs:11500,0.00776638835668564)
--(axis cs:11400,0.00778775382786989)
--(axis cs:11300,0.00781305134296417)
--(axis cs:11200,0.00781823322176933)
--(axis cs:11100,0.00783918891102076)
--(axis cs:11000,0.0078557226806879)
--(axis cs:10900,0.00793302804231644)
--(axis cs:10800,0.00796305760741234)
--(axis cs:10700,0.00800886563956738)
--(axis cs:10600,0.00803768821060658)
--(axis cs:10500,0.00805125664919615)
--(axis cs:10400,0.00803550519049168)
--(axis cs:10300,0.00806283950805664)
--(axis cs:10200,0.00807841867208481)
--(axis cs:10100,0.00810746848583221)
--(axis cs:10000,0.00810604821890593)
--(axis cs:9900,0.00814112648367882)
--(axis cs:9800,0.00817620288580656)
--(axis cs:9700,0.00818442087620497)
--(axis cs:9600,0.00819882191717625)
--(axis cs:9500,0.00823299121111631)
--(axis cs:9400,0.00825307331979275)
--(axis cs:9300,0.00825977325439453)
--(axis cs:9200,0.00825564842671156)
--(axis cs:9100,0.00830129161477089)
--(axis cs:9000,0.00835177861154079)
--(axis cs:8900,0.00838332064449787)
--(axis cs:8800,0.00840079784393311)
--(axis cs:8700,0.00844440422952175)
--(axis cs:8600,0.00846142135560513)
--(axis cs:8500,0.0084675308316946)
--(axis cs:8400,0.00850044842809439)
--(axis cs:8300,0.00852862559258938)
--(axis cs:8200,0.00855123810470104)
--(axis cs:8100,0.00861977320164442)
--(axis cs:8000,0.00861954689025879)
--(axis cs:7900,0.00867083016782999)
--(axis cs:7800,0.00869068410247564)
--(axis cs:7700,0.00873917900025845)
--(axis cs:7600,0.00876313541084528)
--(axis cs:7500,0.0088068749755621)
--(axis cs:7400,0.00885336101055145)
--(axis cs:7300,0.00890163984149694)
--(axis cs:7200,0.0089099109172821)
--(axis cs:7100,0.00894253794103861)
--(axis cs:7000,0.00897443294525146)
--(axis cs:6900,0.00900376215577126)
--(axis cs:6800,0.00904353521764278)
--(axis cs:6700,0.00908470805734396)
--(axis cs:6600,0.00910090561956167)
--(axis cs:6500,0.00914750061929226)
--(axis cs:6400,0.00919509865343571)
--(axis cs:6300,0.00921312812715769)
--(axis cs:6200,0.00926152523607016)
--(axis cs:6100,0.00927507970482111)
--(axis cs:6000,0.00933827273547649)
--(axis cs:5900,0.00941464304924011)
--(axis cs:5800,0.00947486516088247)
--(axis cs:5700,0.00950172636657953)
--(axis cs:5600,0.00954005774110556)
--(axis cs:5500,0.00959188025444746)
--(axis cs:5400,0.00963639654219151)
--(axis cs:5300,0.00970355793833733)
--(axis cs:5200,0.00977576896548271)
--(axis cs:5100,0.00985685549676418)
--(axis cs:5000,0.00987931620329618)
--(axis cs:4900,0.00993124302476645)
--(axis cs:4800,0.00996583886444569)
--(axis cs:4700,0.0100254779681563)
--(axis cs:4600,0.0100779226049781)
--(axis cs:4500,0.0101523566991091)
--(axis cs:4400,0.0101955411955714)
--(axis cs:4300,0.0102711115032434)
--(axis cs:4200,0.0103566171601415)
--(axis cs:4100,0.0104250544682145)
--(axis cs:4000,0.0105152726173401)
--(axis cs:3900,0.0106360139325261)
--(axis cs:3800,0.010682194493711)
--(axis cs:3700,0.0107612954452634)
--(axis cs:3600,0.0108530335128307)
--(axis cs:3500,0.0109247211366892)
--(axis cs:3400,0.0110286697745323)
--(axis cs:3300,0.0111628901213408)
--(axis cs:3200,0.0113132260739803)
--(axis cs:3100,0.0114332046359777)
--(axis cs:3000,0.0115463379770517)
--(axis cs:2900,0.0116647724062204)
--(axis cs:2800,0.0118211749941111)
--(axis cs:2700,0.0119809145107865)
--(axis cs:2600,0.0121162803843617)
--(axis cs:2500,0.0123082492500544)
--(axis cs:2400,0.0125016439706087)
--(axis cs:2300,0.0126613760367036)
--(axis cs:2200,0.0128647033125162)
--(axis cs:2100,0.0131368450820446)
--(axis cs:2000,0.0134150385856628)
--(axis cs:1900,0.0137205282226205)
--(axis cs:1800,0.0140944411978126)
--(axis cs:1700,0.0145047549158335)
--(axis cs:1600,0.015034407377243)
--(axis cs:1500,0.0155743416398764)
--(axis cs:1400,0.0162540432065725)
--(axis cs:1300,0.01698974147439)
--(axis cs:1200,0.0178048741072416)
--(axis cs:1100,0.0186079870909452)
--(axis cs:1000,0.0194399263709784)
--(axis cs:900,0.0204215664416552)
--(axis cs:800,0.0214774925261736)
--(axis cs:700,0.0224762018769979)
--(axis cs:600,0.0242088567465544)
--(axis cs:500,0.027130639180541)
--(axis cs:400,0.0299398619681597)
--(axis cs:300,0.0326264128088951)
--(axis cs:200,0.0363860614597797)
--(axis cs:100,0.0428013391792774)
--(axis cs:0,0.0487950257956982)
--cycle;

\path [fill=white!40.1960784313725!black, fill opacity=0.4, ultra thick]
(axis cs:0,0.0491982959210873)
--(axis cs:0,0.049132626503706)
--(axis cs:100,0.0430962294340134)
--(axis cs:200,0.0363682098686695)
--(axis cs:300,0.0321813933551311)
--(axis cs:400,0.0294917728751898)
--(axis cs:500,0.0267006009817123)
--(axis cs:600,0.0238281451165676)
--(axis cs:700,0.0221217013895512)
--(axis cs:800,0.0211009476333857)
--(axis cs:900,0.0200391244143248)
--(axis cs:1000,0.0190135780721903)
--(axis cs:1100,0.018229840323329)
--(axis cs:1200,0.0174305085092783)
--(axis cs:1300,0.0165961217135191)
--(axis cs:1400,0.0158965904265642)
--(axis cs:1500,0.01532275788486)
--(axis cs:1600,0.0147445248439908)
--(axis cs:1700,0.0142889143899083)
--(axis cs:1800,0.0139182126149535)
--(axis cs:1900,0.0135842338204384)
--(axis cs:2000,0.0132447788491845)
--(axis cs:2100,0.0130140380933881)
--(axis cs:2200,0.012761645950377)
--(axis cs:2300,0.0125689264386892)
--(axis cs:2400,0.0123534565791488)
--(axis cs:2500,0.0121830115094781)
--(axis cs:2600,0.0120224803686142)
--(axis cs:2700,0.0119075067341328)
--(axis cs:2800,0.0117439897730947)
--(axis cs:2900,0.0116162057965994)
--(axis cs:3000,0.0115119013935328)
--(axis cs:3100,0.0113889779895544)
--(axis cs:3200,0.0112512428313494)
--(axis cs:3300,0.0111356787383556)
--(axis cs:3400,0.0109908860176802)
--(axis cs:3500,0.0108609609305859)
--(axis cs:3600,0.0107248928397894)
--(axis cs:3700,0.0106415031477809)
--(axis cs:3800,0.0105662290006876)
--(axis cs:3900,0.0104771545156837)
--(axis cs:4000,0.0103706466034055)
--(axis cs:4100,0.0103115122765303)
--(axis cs:4200,0.0102346502244473)
--(axis cs:4300,0.010163658298552)
--(axis cs:4400,0.0101066147908568)
--(axis cs:4500,0.0100476108491421)
--(axis cs:4600,0.0100204711779952)
--(axis cs:4700,0.00994156487286091)
--(axis cs:4800,0.00988617539405823)
--(axis cs:4900,0.00979821756482124)
--(axis cs:5000,0.00974726025015116)
--(axis cs:5100,0.00966677814722061)
--(axis cs:5200,0.00961588229984045)
--(axis cs:5300,0.00954455137252808)
--(axis cs:5400,0.00952557288110256)
--(axis cs:5500,0.00947717949748039)
--(axis cs:5600,0.00941329170018435)
--(axis cs:5700,0.00941506028175354)
--(axis cs:5800,0.00939751323312521)
--(axis cs:5900,0.00935683492571115)
--(axis cs:6000,0.00929501000791788)
--(axis cs:6100,0.0092425849288702)
--(axis cs:6200,0.00916855875402689)
--(axis cs:6300,0.00912216678261757)
--(axis cs:6400,0.00907672196626663)
--(axis cs:6500,0.00904580112546682)
--(axis cs:6600,0.00900828558951616)
--(axis cs:6700,0.00897378940135241)
--(axis cs:6800,0.00893955212086439)
--(axis cs:6900,0.0089056259021163)
--(axis cs:7000,0.00889360066503286)
--(axis cs:7100,0.00887115020304918)
--(axis cs:7200,0.00887722987681627)
--(axis cs:7300,0.0088274534791708)
--(axis cs:7400,0.00879304111003876)
--(axis cs:7500,0.00875385571271181)
--(axis cs:7600,0.00868077296763659)
--(axis cs:7700,0.00862491130828857)
--(axis cs:7800,0.00861332379281521)
--(axis cs:7900,0.00858140364289284)
--(axis cs:8000,0.00855625048279762)
--(axis cs:8100,0.00853403843939304)
--(axis cs:8200,0.00848930142819881)
--(axis cs:8300,0.00844331737607718)
--(axis cs:8400,0.00844314135611057)
--(axis cs:8500,0.0084140794351697)
--(axis cs:8600,0.0083959000185132)
--(axis cs:8700,0.00837953109294176)
--(axis cs:8800,0.00834438763558865)
--(axis cs:8900,0.00829768180847168)
--(axis cs:9000,0.0082654133439064)
--(axis cs:9100,0.00823108945041895)
--(axis cs:9200,0.00821364019066095)
--(axis cs:9300,0.00818733032792807)
--(axis cs:9400,0.00816063489764929)
--(axis cs:9500,0.00814556702971458)
--(axis cs:9600,0.00812162738293409)
--(axis cs:9700,0.00807300396263599)
--(axis cs:9800,0.00803261063992977)
--(axis cs:9900,0.0080031817778945)
--(axis cs:10000,0.00800285954028368)
--(axis cs:10100,0.00795783288776875)
--(axis cs:10200,0.00793487299233675)
--(axis cs:10300,0.00790082477033138)
--(axis cs:10400,0.00789136905223131)
--(axis cs:10500,0.00785657204687595)
--(axis cs:10600,0.00784869492053986)
--(axis cs:10700,0.00782443396747112)
--(axis cs:10800,0.00780411204323173)
--(axis cs:10900,0.00778473308309913)
--(axis cs:11000,0.00773728685453534)
--(axis cs:11100,0.00771230226382613)
--(axis cs:11200,0.00772428046911955)
--(axis cs:11300,0.00772189116105437)
--(axis cs:11400,0.00769791612401605)
--(axis cs:11500,0.00767219066619873)
--(axis cs:11600,0.00764191150665283)
--(axis cs:11700,0.00758969783782959)
--(axis cs:11800,0.00757623743265867)
--(axis cs:11900,0.0075700324960053)
--(axis cs:12000,0.00758716836571693)
--(axis cs:12100,0.00757521670311689)
--(axis cs:12200,0.00759265432134271)
--(axis cs:12300,0.00756454421207309)
--(axis cs:12400,0.00751562789082527)
--(axis cs:12500,0.00748812826350331)
--(axis cs:12600,0.00744058145210147)
--(axis cs:12700,0.00742497015744448)
--(axis cs:12800,0.00740518048405647)
--(axis cs:12900,0.00739777088165283)
--(axis cs:13000,0.00736655527725816)
--(axis cs:13100,0.007316704839468)
--(axis cs:13200,0.00730377109721303)
--(axis cs:13300,0.00727003859356046)
--(axis cs:13400,0.00726979784667492)
--(axis cs:13500,0.00727691408246756)
--(axis cs:13600,0.00726385274901986)
--(axis cs:13700,0.00722099281847477)
--(axis cs:13800,0.00720012607052922)
--(axis cs:13900,0.00719556258991361)
--(axis cs:14000,0.00715773878619075)
--(axis cs:14100,0.00712947361171246)
--(axis cs:14200,0.00712584098801017)
--(axis cs:14300,0.0071299490518868)
--(axis cs:14400,0.00711811892688274)
--(axis cs:14500,0.00711890868842602)
--(axis cs:14600,0.00711896410211921)
--(axis cs:14700,0.00708145694807172)
--(axis cs:14800,0.00707411766052246)
--(axis cs:14900,0.00708451261743903)
--(axis cs:15000,0.00708606233820319)
--(axis cs:15100,0.00705220131203532)
--(axis cs:15200,0.00703921308740973)
--(axis cs:15300,0.00701575679704547)
--(axis cs:15400,0.00695932609960437)
--(axis cs:15500,0.00691783800721169)
--(axis cs:15600,0.00693326629698277)
--(axis cs:15700,0.00692059239372611)
--(axis cs:15800,0.00691557954996824)
--(axis cs:15900,0.00692317495122552)
--(axis cs:16000,0.00690956134349108)
--(axis cs:16100,0.00688606919720769)
--(axis cs:16200,0.00686616683378816)
--(axis cs:16300,0.00685786409303546)
--(axis cs:16400,0.00687220832332969)
--(axis cs:16500,0.00688349036499858)
--(axis cs:16600,0.00687645189464092)
--(axis cs:16700,0.0068903504870832)
--(axis cs:16800,0.0068669319152832)
--(axis cs:16900,0.00683695776388049)
--(axis cs:17000,0.00679626455530524)
--(axis cs:17100,0.00679817190393806)
--(axis cs:17200,0.00676906108856201)
--(axis cs:17300,0.00675816554576159)
--(axis cs:17400,0.00675151124596596)
--(axis cs:17500,0.00677290186285973)
--(axis cs:17600,0.00674161966890097)
--(axis cs:17700,0.00672448566183448)
--(axis cs:17800,0.00671280268579721)
--(axis cs:17900,0.00669991970062256)
--(axis cs:18000,0.00664999475702643)
--(axis cs:18100,0.00664889812469482)
--(axis cs:18200,0.0066505060531199)
--(axis cs:18300,0.00661106687039137)
--(axis cs:18400,0.00657129799947143)
--(axis cs:18500,0.00658774701878428)
--(axis cs:18600,0.00659332657232881)
--(axis cs:18700,0.00658155046403408)
--(axis cs:18800,0.0066035334020853)
--(axis cs:18900,0.0066056726500392)
--(axis cs:19000,0.00657343119382858)
--(axis cs:19100,0.00655139796435833)
--(axis cs:19200,0.00654098484665155)
--(axis cs:19300,0.00652728090062737)
--(axis cs:19400,0.00651273969560862)
--(axis cs:19500,0.00650787353515625)
--(axis cs:19600,0.00647808937355876)
--(axis cs:19700,0.00648327590897679)
--(axis cs:19800,0.00644602114334702)
--(axis cs:19900,0.00642811181023717)
--(axis cs:20000,0.00642998749390244)
--(axis cs:20100,0.00641488051041961)
--(axis cs:20200,0.00642308965325356)
--(axis cs:20300,0.00640921574085951)
--(axis cs:20400,0.00640395935624838)
--(axis cs:20500,0.00639859307557344)
--(axis cs:20600,0.006396877579391)
--(axis cs:20700,0.00636670086532831)
--(axis cs:20800,0.00639046309515834)
--(axis cs:20900,0.00638170260936022)
--(axis cs:21000,0.0063633918762207)
--(axis cs:21100,0.00636102957651019)
--(axis cs:21200,0.00633905967697501)
--(axis cs:21300,0.0063130808994174)
--(axis cs:21400,0.00632077641785145)
--(axis cs:21500,0.00631920993328094)
--(axis cs:21600,0.00632180133834481)
--(axis cs:21700,0.00632417760789394)
--(axis cs:21800,0.00631679408252239)
--(axis cs:21900,0.00631573330610991)
--(axis cs:22000,0.00631213188171387)
--(axis cs:22100,0.00629358272999525)
--(axis cs:22200,0.00628466624766588)
--(axis cs:22300,0.00628232955932617)
--(axis cs:22400,0.00626506097614765)
--(axis cs:22500,0.00627197651192546)
--(axis cs:22600,0.00627545453608036)
--(axis cs:22700,0.00626832060515881)
--(axis cs:22800,0.00626265536993742)
--(axis cs:22900,0.00627807900309563)
--(axis cs:23000,0.00626330124214292)
--(axis cs:23100,0.00624522846192122)
--(axis cs:23200,0.00623960606753826)
--(axis cs:23300,0.00624810950830579)
--(axis cs:23400,0.0062272297218442)
--(axis cs:23500,0.00621978519484401)
--(axis cs:23600,0.00622192258015275)
--(axis cs:23700,0.00623825564980507)
--(axis cs:23800,0.00622668955475092)
--(axis cs:23900,0.00622470583766699)
--(axis cs:24000,0.00620948290452361)
--(axis cs:24100,0.00621706293895841)
--(axis cs:24200,0.00620395503938198)
--(axis cs:24300,0.00621651764959097)
--(axis cs:24400,0.00621782569214702)
--(axis cs:24500,0.00621491670608521)
--(axis cs:24600,0.00620065163820982)
--(axis cs:24700,0.006169602740556)
--(axis cs:24800,0.00614321744069457)
--(axis cs:24900,0.00611946452409029)
--(axis cs:25000,0.00611034408211708)
--(axis cs:25100,0.00610245810821652)
--(axis cs:25200,0.00611995439976454)
--(axis cs:25300,0.00611498160287738)
--(axis cs:25400,0.00610325066372752)
--(axis cs:25500,0.0061086849309504)
--(axis cs:25600,0.00609581032767892)
--(axis cs:25700,0.00606576120480895)
--(axis cs:25800,0.00606416864320636)
--(axis cs:25900,0.00608102371916175)
--(axis cs:26000,0.00607087649405003)
--(axis cs:26100,0.00607871497049928)
--(axis cs:26200,0.00610943930223584)
--(axis cs:26300,0.00609516818076372)
--(axis cs:26400,0.00608719093725085)
--(axis cs:26500,0.00609641522169113)
--(axis cs:26600,0.00608465680852532)
--(axis cs:26700,0.0060420511290431)
--(axis cs:26800,0.00604402506724)
--(axis cs:26900,0.0060420511290431)
--(axis cs:27000,0.00605070497840643)
--(axis cs:27100,0.00609509274363518)
--(axis cs:27200,0.00609293766319752)
--(axis cs:27300,0.00608446728438139)
--(axis cs:27400,0.00606318330392241)
--(axis cs:27500,0.00605127448216081)
--(axis cs:27600,0.00602985825389624)
--(axis cs:27700,0.00603320170193911)
--(axis cs:27800,0.00603483524173498)
--(axis cs:27900,0.00605154037475586)
--(axis cs:28000,0.00604087393730879)
--(axis cs:28100,0.0060338475741446)
--(axis cs:28200,0.00601716199889779)
--(axis cs:28300,0.00599558930844069)
--(axis cs:28400,0.00596809014678001)
--(axis cs:28500,0.00595699856057763)
--(axis cs:28600,0.00594380544498563)
--(axis cs:28700,0.00595455849543214)
--(axis cs:28800,0.00596927152946591)
--(axis cs:28900,0.00596709968522191)
--(axis cs:29000,0.00596656557172537)
--(axis cs:29100,0.00594815285876393)
--(axis cs:29200,0.00592686794698238)
--(axis cs:29300,0.00590530410408974)
--(axis cs:29400,0.00591854937374592)
--(axis cs:29500,0.00590434949845076)
--(axis cs:29600,0.00589915690943599)
--(axis cs:29700,0.00590286031365395)
--(axis cs:29800,0.00591499963775277)
--(axis cs:29900,0.00589018315076828)
--(axis cs:30000,0.00589213101193309)
--(axis cs:30100,0.00588105525821447)
--(axis cs:30200,0.00588728068396449)
--(axis cs:30300,0.0058612278662622)
--(axis cs:30400,0.00585675705224276)
--(axis cs:30500,0.00585881993174553)
--(axis cs:30600,0.00584628619253635)
--(axis cs:30700,0.00583822093904018)
--(axis cs:30800,0.00585656613111496)
--(axis cs:30900,0.0058605782687664)
--(axis cs:31000,0.00582373281940818)
--(axis cs:31100,0.00583539251238108)
--(axis cs:31200,0.00583952059969306)
--(axis cs:31300,0.00584150850772858)
--(axis cs:31400,0.00582977291196585)
--(axis cs:31500,0.00582927605137229)
--(axis cs:31600,0.00580247212201357)
--(axis cs:31700,0.00578415207564831)
--(axis cs:31800,0.00577504793182015)
--(axis cs:31900,0.00577998254448175)
--(axis cs:32000,0.00581149710342288)
--(axis cs:32100,0.00581409689038992)
--(axis cs:32200,0.00582621805369854)
--(axis cs:32300,0.00583718903362751)
--(axis cs:32400,0.00581577979028225)
--(axis cs:32500,0.00578591134399176)
--(axis cs:32600,0.00580557016655803)
--(axis cs:32700,0.00578438164666295)
--(axis cs:32700,0.00639748573303223)
--(axis cs:32700,0.00639748573303223)
--(axis cs:32600,0.00639748573303223)
--(axis cs:32500,0.00639748573303223)
--(axis cs:32400,0.00639748573303223)
--(axis cs:32300,0.00639748573303223)
--(axis cs:32200,0.00639748573303223)
--(axis cs:32100,0.00639748573303223)
--(axis cs:32000,0.00639748573303223)
--(axis cs:31900,0.00639748573303223)
--(axis cs:31800,0.00639748573303223)
--(axis cs:31700,0.00639748573303223)
--(axis cs:31600,0.00639748573303223)
--(axis cs:31500,0.00639748573303223)
--(axis cs:31400,0.00639748573303223)
--(axis cs:31300,0.00639748573303223)
--(axis cs:31200,0.00639748573303223)
--(axis cs:31100,0.00639748573303223)
--(axis cs:31000,0.00639748573303223)
--(axis cs:30900,0.00639748573303223)
--(axis cs:30800,0.00639748573303223)
--(axis cs:30700,0.00639748573303223)
--(axis cs:30600,0.00639748573303223)
--(axis cs:30500,0.00639748573303223)
--(axis cs:30400,0.00639748573303223)
--(axis cs:30300,0.00639748573303223)
--(axis cs:30200,0.00639748573303223)
--(axis cs:30100,0.00639748573303223)
--(axis cs:30000,0.00639748573303223)
--(axis cs:29900,0.00639748573303223)
--(axis cs:29800,0.00639748573303223)
--(axis cs:29700,0.00639748573303223)
--(axis cs:29600,0.00639748573303223)
--(axis cs:29500,0.00639748573303223)
--(axis cs:29400,0.00639748573303223)
--(axis cs:29300,0.00639748573303223)
--(axis cs:29200,0.00639748573303223)
--(axis cs:29100,0.00639748573303223)
--(axis cs:29000,0.00639748573303223)
--(axis cs:28900,0.00639748573303223)
--(axis cs:28800,0.00639748573303223)
--(axis cs:28700,0.00639748573303223)
--(axis cs:28600,0.00639748573303223)
--(axis cs:28500,0.00639748573303223)
--(axis cs:28400,0.00639748573303223)
--(axis cs:28300,0.00639748573303223)
--(axis cs:28200,0.00639748573303223)
--(axis cs:28100,0.00639748573303223)
--(axis cs:28000,0.00639748573303223)
--(axis cs:27900,0.00639748573303223)
--(axis cs:27800,0.00639748573303223)
--(axis cs:27700,0.00639748573303223)
--(axis cs:27600,0.00639748573303223)
--(axis cs:27500,0.00639748573303223)
--(axis cs:27400,0.00639748573303223)
--(axis cs:27300,0.00639748573303223)
--(axis cs:27200,0.00639748573303223)
--(axis cs:27100,0.00639748573303223)
--(axis cs:27000,0.00639748573303223)
--(axis cs:26900,0.00639748573303223)
--(axis cs:26800,0.00639748573303223)
--(axis cs:26700,0.00639748573303223)
--(axis cs:26600,0.00639748573303223)
--(axis cs:26500,0.00639748573303223)
--(axis cs:26400,0.00639748573303223)
--(axis cs:26300,0.00639748573303223)
--(axis cs:26200,0.00639748573303223)
--(axis cs:26100,0.00639748573303223)
--(axis cs:26000,0.00639748573303223)
--(axis cs:25900,0.00639748573303223)
--(axis cs:25800,0.00639748573303223)
--(axis cs:25700,0.00639748573303223)
--(axis cs:25600,0.00639748573303223)
--(axis cs:25500,0.00639748573303223)
--(axis cs:25400,0.00639748573303223)
--(axis cs:25300,0.00639748573303223)
--(axis cs:25200,0.00639748573303223)
--(axis cs:25100,0.00639748573303223)
--(axis cs:25000,0.00639748573303223)
--(axis cs:24900,0.00639748573303223)
--(axis cs:24800,0.00639518303796649)
--(axis cs:24700,0.00639124168083072)
--(axis cs:24600,0.00638686306774616)
--(axis cs:24500,0.00638499576598406)
--(axis cs:24400,0.00638463022187352)
--(axis cs:24300,0.00638479460030794)
--(axis cs:24200,0.00638642068952322)
--(axis cs:24100,0.00638472614809871)
--(axis cs:24000,0.00638569379225373)
--(axis cs:23900,0.00638378970324993)
--(axis cs:23800,0.00638355500996113)
--(axis cs:23700,0.00638225674629211)
--(axis cs:23600,0.00638412544503808)
--(axis cs:23500,0.00638438807800412)
--(axis cs:23400,0.00638349168002605)
--(axis cs:23300,0.00638127280399203)
--(axis cs:23200,0.0063821142539382)
--(axis cs:23100,0.00638154614716768)
--(axis cs:23000,0.00638006860390306)
--(axis cs:22900,0.00637946743518114)
--(axis cs:22800,0.00638010911643505)
--(axis cs:22700,0.00637978501617908)
--(axis cs:22600,0.00637951772660017)
--(axis cs:22500,0.00637962622568011)
--(axis cs:22400,0.00637996103614569)
--(axis cs:22300,0.0063794506713748)
--(axis cs:22200,0.00637946417555213)
--(axis cs:22100,0.00637964671477675)
--(axis cs:22000,0.00638356572017074)
--(axis cs:21900,0.00638625491410494)
--(axis cs:21800,0.00638697482645512)
--(axis cs:21700,0.00639523100107908)
--(axis cs:21600,0.00640380615368485)
--(axis cs:21500,0.00640525389462709)
--(axis cs:21400,0.00642377696931362)
--(axis cs:21300,0.00642524287104607)
--(axis cs:21200,0.00642517162486911)
--(axis cs:21100,0.00641706166788936)
--(axis cs:21000,0.00641902908682823)
--(axis cs:20900,0.00642001815140247)
--(axis cs:20800,0.00642223376780748)
--(axis cs:20700,0.00643466040492058)
--(axis cs:20600,0.00643320102244616)
--(axis cs:20500,0.00645334459841251)
--(axis cs:20400,0.00646562222391367)
--(axis cs:20300,0.00647897645831108)
--(axis cs:20200,0.00648374855518341)
--(axis cs:20100,0.00651555042713881)
--(axis cs:20000,0.00648298254236579)
--(axis cs:19900,0.0065013887360692)
--(axis cs:19800,0.00649347295984626)
--(axis cs:19700,0.00651768920943141)
--(axis cs:19600,0.00651988806203008)
--(axis cs:19500,0.00655012438073754)
--(axis cs:19400,0.00654185470193624)
--(axis cs:19300,0.00657198904082179)
--(axis cs:19200,0.00658026989549398)
--(axis cs:19100,0.00661669857800007)
--(axis cs:19000,0.00663797836750746)
--(axis cs:18900,0.00664813350886106)
--(axis cs:18800,0.00664794445037842)
--(axis cs:18700,0.00664764456450939)
--(axis cs:18600,0.00666815089061856)
--(axis cs:18500,0.00666482467204332)
--(axis cs:18400,0.00666527729481459)
--(axis cs:18300,0.00666277389973402)
--(axis cs:18200,0.00668241688981652)
--(axis cs:18100,0.00668177986517549)
--(axis cs:18000,0.0067030880600214)
--(axis cs:17900,0.00674375845119357)
--(axis cs:17800,0.00678477250039577)
--(axis cs:17700,0.00678908824920654)
--(axis cs:17600,0.00679538259282708)
--(axis cs:17500,0.00680287461727858)
--(axis cs:17400,0.00679948320612311)
--(axis cs:17300,0.00683676358312368)
--(axis cs:17200,0.00683769304305315)
--(axis cs:17100,0.006861821282655)
--(axis cs:17000,0.00687120901420712)
--(axis cs:16900,0.00690071564167738)
--(axis cs:16800,0.00687693897634745)
--(axis cs:16700,0.00691852578893304)
--(axis cs:16600,0.00692334165796638)
--(axis cs:16500,0.00696012983098626)
--(axis cs:16400,0.00697999028488994)
--(axis cs:16300,0.00699863443151116)
--(axis cs:16200,0.00699602952226996)
--(axis cs:16100,0.00701111136004329)
--(axis cs:16000,0.00701030110940337)
--(axis cs:15900,0.00700525753200054)
--(axis cs:15800,0.00698770396411419)
--(axis cs:15700,0.00699450215324759)
--(axis cs:15600,0.00699610728770494)
--(axis cs:15500,0.0070111989043653)
--(axis cs:15400,0.00701088923960924)
--(axis cs:15300,0.0070389392785728)
--(axis cs:15200,0.00706464517861605)
--(axis cs:15100,0.00707654701545835)
--(axis cs:15000,0.00714007159695029)
--(axis cs:14900,0.00717012863606215)
--(axis cs:14800,0.00718042301014066)
--(axis cs:14700,0.00718468381091952)
--(axis cs:14600,0.00719122076407075)
--(axis cs:14500,0.00714716920629144)
--(axis cs:14400,0.00717273820191622)
--(axis cs:14300,0.00720708351582289)
--(axis cs:14200,0.00720734614878893)
--(axis cs:14100,0.00721867103129625)
--(axis cs:14000,0.00725096138194203)
--(axis cs:13900,0.0072467545978725)
--(axis cs:13800,0.00723483087494969)
--(axis cs:13700,0.00725872348994017)
--(axis cs:13600,0.00727500813081861)
--(axis cs:13500,0.00728882476687431)
--(axis cs:13400,0.00731306057423353)
--(axis cs:13300,0.00738604087382555)
--(axis cs:13200,0.00740401679649949)
--(axis cs:13100,0.00739669427275658)
--(axis cs:13000,0.00740659004077315)
--(axis cs:12900,0.00743050174787641)
--(axis cs:12800,0.00742949452251196)
--(axis cs:12700,0.00745323859155178)
--(axis cs:12600,0.00750535493716598)
--(axis cs:12500,0.00749921379610896)
--(axis cs:12400,0.00753927230834961)
--(axis cs:12300,0.0075694085098803)
--(axis cs:12200,0.00760670471936464)
--(axis cs:12100,0.00762266386300325)
--(axis cs:12000,0.00761704426258802)
--(axis cs:11900,0.00763342762365937)
--(axis cs:11800,0.00762685760855675)
--(axis cs:11700,0.00766760995611548)
--(axis cs:11600,0.00770571967586875)
--(axis cs:11500,0.00774653255939484)
--(axis cs:11400,0.00776670640334487)
--(axis cs:11300,0.00781777035444975)
--(axis cs:11200,0.00782269332557917)
--(axis cs:11100,0.00785706751048565)
--(axis cs:11000,0.00786595325917006)
--(axis cs:10900,0.0079128984361887)
--(axis cs:10800,0.0078978780657053)
--(axis cs:10700,0.00792603474110365)
--(axis cs:10600,0.00793793238699436)
--(axis cs:10500,0.00795359630137682)
--(axis cs:10400,0.00794408284127712)
--(axis cs:10300,0.00801607966423035)
--(axis cs:10200,0.00804389175027609)
--(axis cs:10100,0.00806787051260471)
--(axis cs:10000,0.00808532256633043)
--(axis cs:9900,0.00812030490487814)
--(axis cs:9800,0.00813080184161663)
--(axis cs:9700,0.00812826119363308)
--(axis cs:9600,0.00816431734710932)
--(axis cs:9500,0.00818273983895779)
--(axis cs:9400,0.00822431687265635)
--(axis cs:9300,0.00824671890586615)
--(axis cs:9200,0.0082556726410985)
--(axis cs:9100,0.00827992055565119)
--(axis cs:9000,0.0083168838173151)
--(axis cs:8900,0.0083491550758481)
--(axis cs:8800,0.008379140868783)
--(axis cs:8700,0.00841499213129282)
--(axis cs:8600,0.00843815784901381)
--(axis cs:8500,0.00845225434750319)
--(axis cs:8400,0.00847639422863722)
--(axis cs:8300,0.00851132813841105)
--(axis cs:8200,0.00852229632437229)
--(axis cs:8100,0.00856379978358746)
--(axis cs:8000,0.00858151912689209)
--(axis cs:7900,0.00862834416329861)
--(axis cs:7800,0.0086601497605443)
--(axis cs:7700,0.00868547149002552)
--(axis cs:7600,0.00871133990585804)
--(axis cs:7500,0.00877509173005819)
--(axis cs:7400,0.00883149541914463)
--(axis cs:7300,0.00888761878013611)
--(axis cs:7200,0.00891011673957109)
--(axis cs:7100,0.00892579555511475)
--(axis cs:7000,0.00891035329550505)
--(axis cs:6900,0.00894223060458899)
--(axis cs:6800,0.00898073520511389)
--(axis cs:6700,0.00903828628361225)
--(axis cs:6600,0.00908056367188692)
--(axis cs:6500,0.0091228699311614)
--(axis cs:6400,0.00915632210671902)
--(axis cs:6300,0.00918144918978214)
--(axis cs:6200,0.00920643843710423)
--(axis cs:6100,0.0092843733727932)
--(axis cs:6000,0.0093438858166337)
--(axis cs:5900,0.0093970512971282)
--(axis cs:5800,0.00943869072943926)
--(axis cs:5700,0.00948349945247173)
--(axis cs:5600,0.00951544009149075)
--(axis cs:5500,0.00956014357507229)
--(axis cs:5400,0.00960821378976107)
--(axis cs:5300,0.00968102924525738)
--(axis cs:5200,0.00975377392023802)
--(axis cs:5100,0.0098196417093277)
--(axis cs:5000,0.00987078901380301)
--(axis cs:4900,0.00991247408092022)
--(axis cs:4800,0.0099507812410593)
--(axis cs:4700,0.0100187119096518)
--(axis cs:4600,0.0100942766293883)
--(axis cs:4500,0.0101769212633371)
--(axis cs:4400,0.010251940228045)
--(axis cs:4300,0.0103331794962287)
--(axis cs:4200,0.0103941354900599)
--(axis cs:4100,0.0104318428784609)
--(axis cs:4000,0.0104827610775828)
--(axis cs:3900,0.0105607630684972)
--(axis cs:3800,0.0106485188007355)
--(axis cs:3700,0.0107548180967569)
--(axis cs:3600,0.0108531564474106)
--(axis cs:3500,0.0109605230391026)
--(axis cs:3400,0.011052024550736)
--(axis cs:3300,0.0111840963363647)
--(axis cs:3200,0.0113219618797302)
--(axis cs:3100,0.0114828739315271)
--(axis cs:3000,0.0116145275533199)
--(axis cs:2900,0.0117637319490314)
--(axis cs:2800,0.0118762822821736)
--(axis cs:2700,0.0120199583470821)
--(axis cs:2600,0.0121446456760168)
--(axis cs:2500,0.0123099749907851)
--(axis cs:2400,0.0125218098983169)
--(axis cs:2300,0.0126814544200897)
--(axis cs:2200,0.0128805637359619)
--(axis cs:2100,0.0131098432466388)
--(axis cs:2000,0.0133815044537187)
--(axis cs:1900,0.0136804804205894)
--(axis cs:1800,0.0140497973188758)
--(axis cs:1700,0.0144479628652334)
--(axis cs:1600,0.0149785010144114)
--(axis cs:1500,0.0155085325241089)
--(axis cs:1400,0.0161406192928553)
--(axis cs:1300,0.0167877674102783)
--(axis cs:1200,0.0175414141267538)
--(axis cs:1100,0.0183536950498819)
--(axis cs:1000,0.0191886592656374)
--(axis cs:900,0.0202075075358152)
--(axis cs:800,0.0212784055620432)
--(axis cs:700,0.0223503522574902)
--(axis cs:600,0.0239617880433798)
--(axis cs:500,0.0268660485744476)
--(axis cs:400,0.0296337939798832)
--(axis cs:300,0.0322838500142097)
--(axis cs:200,0.0364052802324295)
--(axis cs:100,0.0431578680872917)
--(axis cs:0,0.0491982959210873)
--cycle;

\addplot [ultra thick, red]
table {%
0 0.0544580146670341
100 0.0542704574763775
200 0.0538766831159592
300 0.0533064268529415
400 0.052464172244072
500 0.0513866692781448
600 0.0500394143164158
700 0.0485865473747253
800 0.0471253134310246
900 0.0457724444568157
1000 0.0445105321705341
1100 0.0434617474675179
1400 0.0408168621361256
1500 0.04001235216856
1600 0.0393390245735645
1700 0.0387342125177383
1800 0.0382256507873535
1900 0.0377788990736008
2000 0.0373917557299137
2100 0.0369442813098431
2200 0.036414872854948
2300 0.0358754359185696
2400 0.0352378450334072
2500 0.0344973541796207
2600 0.033745676279068
2700 0.0330415181815624
2800 0.0322929210960865
2900 0.0316906832158566
3200 0.030158843845129
3300 0.0297135636210442
3500 0.0287914033979177
3600 0.0283913724124432
3700 0.02801757119596
3800 0.0276709068566561
3900 0.027309313416481
4300 0.0260236486792564
4400 0.025777593255043
4500 0.025513244792819
4600 0.025288037955761
4700 0.0250044278800488
4800 0.0247754212468863
5100 0.0240313708782196
5200 0.0238579753786325
5300 0.0236291587352753
5500 0.0232081431895494
5600 0.0230461768805981
5700 0.0228742249310017
5900 0.0225903075188398
6000 0.0224648304283619
6200 0.0221300013363361
6300 0.0219860877841711
6400 0.0218684077262878
6500 0.0216822102665901
6600 0.0215574279427528
6700 0.0214134231209755
6900 0.021071620285511
7000 0.0209593120962381
7100 0.0208218917250633
7300 0.0205920059233904
7400 0.0204966869205236
7500 0.0203801915049553
7600 0.0202500633895397
7700 0.0201496779918671
7800 0.0200602654367685
7900 0.0199365317821503
8100 0.0197397377341986
8200 0.019621642306447
8500 0.0193140376359224
8600 0.0192248970270157
8700 0.0191471241414547
8800 0.0190169960260391
8900 0.0189204830676317
9000 0.0188152622431517
9100 0.0187287982553244
9200 0.018619142472744
9300 0.0185727756470442
9400 0.0185021888464689
9500 0.0184599217027426
9600 0.0183704067021608
9800 0.0182033833116293
9900 0.0180918220430613
10000 0.017962533980608
10100 0.0178694054484367
10200 0.0177543498575687
10300 0.0176588073372841
10500 0.0174989383667707
10700 0.0173934604972601
10800 0.0173153709620237
10900 0.0172220394015312
11000 0.0171412937343121
11100 0.0170316491276026
11200 0.0169676952064037
11400 0.0168036464601755
11500 0.0167601257562637
11600 0.0166821628808975
11700 0.0165668316185474
11800 0.0164874698966742
11900 0.0164590999484062
12000 0.0163531918078661
12100 0.0163032226264477
12300 0.0162204261869192
12400 0.0161084327846766
12500 0.016071904450655
12800 0.0158610977232456
12900 0.0158600956201553
13100 0.0157244391739368
13200 0.0156792141497135
13300 0.0156196299940348
13400 0.0155038507655263
13500 0.0154104707762599
13600 0.0153341311961412
13700 0.0152724115177989
13800 0.015203857794404
13900 0.0151695245876908
14000 0.0151463663205504
14100 0.0150967901572585
14300 0.0149604612961411
14400 0.0149099184200168
14500 0.014843606390059
14600 0.0148123884573579
14700 0.014791346155107
14800 0.0147771183401346
14900 0.0147377494722605
15200 0.0145905986428261
15300 0.0145134432241321
15500 0.0144136594608426
15600 0.0143792005255818
15700 0.0142927002161741
15800 0.0143054639920592
15900 0.014242728240788
16000 0.0142049146816134
16100 0.0141588868573308
16200 0.0141407484188676
16300 0.0140512157231569
16500 0.0140340011566877
16600 0.0139999855309725
16700 0.0139376325532794
16800 0.0139248026534915
17000 0.0138608627021313
17100 0.0138021148741245
17200 0.0138110164552927
17300 0.0137335127219558
17400 0.0136742601171136
17500 0.0136511167511344
17600 0.0135886501520872
17700 0.0135458642616868
17800 0.0135488845407963
17900 0.0134980846196413
18000 0.0134716043248773
18100 0.0134827913716435
18200 0.0134320259094238
18300 0.0133959129452705
18400 0.0133938463404775
18500 0.0132926935330033
18600 0.0132384318858385
18700 0.0132275894284248
18900 0.0131007190793753
19000 0.0131120374426246
19400 0.0130110448226333
19600 0.0129259433597326
19700 0.0129063623026013
19800 0.0128953913226724
19900 0.0128756519407034
20100 0.0128565458580852
20200 0.0127760553732514
20300 0.0127369575202465
20400 0.0127216642722487
20500 0.0126699768006802
20600 0.0126441633328795
20700 0.0126420669257641
20900 0.0125611303374171
21000 0.0125522930175066
21100 0.0125107131898403
21200 0.0124879516661167
21300 0.0124733308330178
21400 0.0124403312802315
21500 0.012374971061945
21600 0.0123389568179846
21700 0.0123277986422181
21800 0.0123084373772144
22000 0.012323890812695
22100 0.0123391458764672
22300 0.0122507391497493
22400 0.0122160920873284
22500 0.012190249748528
22600 0.0121308974921703
22700 0.0121342642232776
22800 0.0121204070746899
22900 0.0120781920850277
23000 0.0120641691610217
23100 0.0120582561939955
23200 0.0120221106335521
23400 0.0120556820183992
23500 0.012033874168992
23700 0.012019157409668
23900 0.011939812451601
24000 0.0119178453460336
24100 0.011914286762476
24300 0.0118686025962234
24400 0.0118584949523211
24500 0.0118426308035851
24600 0.0117985429242253
24700 0.0118239084258676
25100 0.0117551805451512
25200 0.0117189101874828
25300 0.0117401434108615
25400 0.0117234857752919
25500 0.0117299715057015
25600 0.0117471674457192
25800 0.0117098167538643
25900 0.0117299715057015
26000 0.0117376977577806
26100 0.0117337554693222
};
\addlegendentry{Baseline}
\addplot [ultra thick, blue,  ]
table {%
0 0.0544329546391964
100 0.0542538948357105
200 0.0538675598800182
300 0.0532926768064499
400 0.052450206130743
500 0.0513713844120502
600 0.0500374063849449
700 0.0485850796103477
800 0.0471259616315365
900 0.0457695946097374
1000 0.0445034466683865
1100 0.0434341281652451
1400 0.0408206805586815
1500 0.0400197766721249
1600 0.0393495000898838
1700 0.0387455262243748
1800 0.0382350236177444
1900 0.0377727597951889
2000 0.0373697355389595
2100 0.0369039922952652
2300 0.0358095169067383
2400 0.0351712740957737
2500 0.034451637417078
2600 0.033703401684761
2700 0.0330094210803509
2800 0.0322677753865719
2900 0.031666737049818
3200 0.0301722250878811
3400 0.0292610004544258
3500 0.0287890732288361
3600 0.0284040402621031
3700 0.0280440784990788
3800 0.0277284868061543
3900 0.0273853316903114
4000 0.0270802900195122
4100 0.0267292894423008
4200 0.0264112558215857
4300 0.0260820537805557
4500 0.0255271084606647
4600 0.0253022145479918
4700 0.0250189080834389
4800 0.0247778203338385
4900 0.0245504919439554
5000 0.0242961123585701
5100 0.0240184664726257
5200 0.0238253846764565
5300 0.0235891602933407
5400 0.0233670528978109
5500 0.0231796987354755
5600 0.0230237189680338
5700 0.0228442512452602
5800 0.022703455761075
5900 0.0225359611213207
6100 0.0222535580396652
6200 0.0220827739685774
6300 0.0219365898519754
6400 0.0218022502958775
6500 0.021622022613883
6700 0.0213265437632799
6800 0.0211580879986286
6900 0.0210130866616964
7000 0.0208878833800554
7100 0.0207185577601194
7200 0.0206089969724417
7400 0.0203615501523018
7500 0.0202243458479643
7600 0.0201126895844936
7900 0.0198242645710707
8000 0.0197166744619608
8100 0.0195994861423969
8400 0.0192834865301847
8500 0.0192055869847536
8600 0.0191373508423567
8700 0.019048785790801
8800 0.0189191177487373
8900 0.0188135001808405
9000 0.0187192130833864
9100 0.0186352077871561
9200 0.0185146667063236
9300 0.0184420589357615
9400 0.0183891449123621
9500 0.0183021686971188
9600 0.0181869361549616
9700 0.0180993713438511
9800 0.0180008392781019
9900 0.0178767703473568
10000 0.0177760943770409
10100 0.0176884178072214
10200 0.0175838023424149
10300 0.0175022631883621
10500 0.0173247996717691
10700 0.0171729549765587
10800 0.0171127952635288
11000 0.0169262569397688
11100 0.0168566722422838
11200 0.0168075859546661
11300 0.016707656905055
11400 0.0166737399995327
11500 0.0166164096444845
11600 0.0165324974805117
11700 0.0164189003407955
11800 0.0163614265620708
11900 0.0162894111126661
12100 0.0161133781075478
12200 0.0160762947052717
12600 0.0158159397542477
12800 0.0156408753246069
13000 0.0155513137578964
13200 0.015403619967401
13300 0.015382400713861
13500 0.0151735479012132
13600 0.0151207279413939
13700 0.0150832170620561
13800 0.0149945104494691
13900 0.014954837039113
14000 0.014944520778954
14100 0.0148839000612497
14200 0.0148148853331804
14400 0.0146529683843255
14500 0.0145602207630873
14600 0.0145228682085872
14700 0.0144540155306458
14800 0.0144231459125876
14900 0.0144092096015811
15000 0.0143582969903946
15100 0.0143211362883449
15200 0.0142987901344895
15500 0.0141370464116335
15600 0.0140709728002548
15700 0.0139926746487617
15800 0.0139889372512698
15900 0.0139181157574058
16000 0.0138871362432837
16100 0.0138452844694257
16200 0.0138457287102938
16300 0.0137940244749188
16400 0.0137655586004257
16500 0.0137470411136746
16600 0.0137071944773197
16700 0.013616481795907
16800 0.0135802607983351
16900 0.0135372001677752
17000 0.0134795680642128
17100 0.0134095177054405
17200 0.0134109826758504
17300 0.0133547456935048
17400 0.0133197139948606
17500 0.0133050614967942
17600 0.0132798822596669
17700 0.0132426582276821
17900 0.0131350196897984
18000 0.0130956033244729
18100 0.0130707416683435
18200 0.0130211841315031
18400 0.0129545535892248
18500 0.0129052177071571
18600 0.0128809930756688
18700 0.0128457378596067
19200 0.01272246055305
19500 0.0125521654263139
19600 0.0124807041138411
19700 0.0124702770262957
19900 0.0124641414731741
20100 0.0124177942052484
20200 0.0123245874419808
20300 0.0123109817504883
20500 0.0122418412938714
20600 0.0122330039739609
20700 0.0122308721765876
20800 0.012161954306066
20900 0.0121272085234523
21000 0.0121113145723939
21100 0.0120745319873095
21200 0.012055748142302
21300 0.012029392644763
21400 0.0120164854452014
21500 0.0119615877047181
21600 0.0119199752807617
21800 0.0118838623166084
21900 0.0118325548246503
22100 0.0118004474788904
22200 0.0117649706080556
22300 0.0117218345403671
22400 0.011719798669219
22500 0.0117008527740836
22600 0.0116551714017987
22700 0.0116476686671376
22800 0.0116086006164551
22900 0.0115527464076877
23100 0.0115398727357388
23200 0.0115034431219101
23400 0.0115090049803257
23500 0.0114686647430062
23600 0.0114504173398018
23700 0.0114414850249887
23800 0.011411857791245
23900 0.011369195766747
24000 0.0113437036052346
24100 0.0113436067476869
24200 0.0112866079434752
24400 0.011227416805923
24500 0.0111809717491269
24600 0.0111235324293375
24900 0.0110973352566361
25000 0.0110740661621094
25100 0.0110714277252555
25200 0.0110331848263741
25300 0.0109899202361703
25400 0.0109410928562284
25500 0.0109192216768861
25600 0.0108782453462481
25700 0.0108676897361875
25800 0.0108914040029049
26000 0.0108920074999332
26100 0.0108674364164472
26200 0.0108532253652811
26300 0.0107914274558425
26400 0.0107691138982773
26500 0.0107230478897691
26600 0.0107118282467127
26700 0.010670599527657
26800 0.0106612835079432
26900 0.0106664970517159
27100 0.0106880497187376
27200 0.0106755886226892
27300 0.0106816617771983
27400 0.0106479655951262
27500 0.0106235183775425
27600 0.0105671556666493
27700 0.0105658527463675
28000 0.0104643832892179
28100 0.0104667646810412
28200 0.0104305585846305
28300 0.0104024549946189
28400 0.010402106679976
28500 0.0103946691378951
28600 0.0103486683219671
28700 0.0103195197880268
28800 0.01030816975981
28900 0.0102663049474359
29000 0.0102435136213899
29100 0.01026058383286
29200 0.0102458642795682
29300 0.0102194789797068
29400 0.0102159501984715
29500 0.0102061601355672
29600 0.0101382881402969
29900 0.0100852968171239
30000 0.0100390752777457
30100 0.0100714368745685
30200 0.0100418729707599
30300 0.0100369453430176
30400 0.0100267101079226
30500 0.0100234961137176
30600 0.00996039807796478
30700 0.00993919372558594
30800 0.00990711897611618
31000 0.0098753310739994
31100 0.00989650189876556
31200 0.00990324188023806
31300 0.00993493385612965
31400 0.00992488674819469
31500 0.00991977192461491
31600 0.00988527853041887
31700 0.00988003239035606
31800 0.00984630454331636
31900 0.00982281379401684
32100 0.009826535359025
32200 0.00982211250811815
32400 0.00977910216897726
32700 0.00972226541489363
32800 0.00969304982572794
32900 0.0096994424238801
33000 0.00967560149729252
33100 0.00968592707067728
33200 0.00967127270996571
33300 0.00967772584408522
33400 0.00967035442590714
33500 0.00965776480734348
33600 0.0096351308748126
33700 0.00963487755507231
33900 0.00961408577859402
34000 0.00962088629603386
34100 0.00959625281393528
34200 0.00957676488906145
34300 0.00956204440444708
34400 0.00955244805663824
34500 0.00954809132963419
34600 0.00955168250948191
34900 0.00953928381204605
35000 0.00954831670969725
35100 0.00954186078161001
35400 0.00953623652458191
35500 0.00952040310949087
35600 0.00952704809606075
35700 0.00951855815947056
35800 0.00952081568539143
35900 0.00951315648853779
36000 0.00949818547815084
36200 0.00950098037719727
36300 0.00947774108499289
36400 0.00948025472462177
36500 0.00949367042630911
36600 0.00947344955056906
36700 0.00946146436035633
36800 0.00948009267449379
36900 0.00946871284395456
37000 0.0094464598223567
37100 0.00944026466459036
37200 0.00944859161973
37300 0.009432727470994
37400 0.00942643266171217
37500 0.00943040754646063
37600 0.00944115128368139
37700 0.00942319352179766
37800 0.00942770577967167
37900 0.00942688249051571
38000 0.00942141376435757
38100 0.00940068624913692
38200 0.00939029268920422
38300 0.00938936974853277
38500 0.0093740476295352
38600 0.00938510801643133
38700 0.00942011084407568
38800 0.0094093345105648
39100 0.00939041655510664
39200 0.00935596134513617
39300 0.00935477949678898
39400 0.00936342682689428
39600 0.00934477057307959
39700 0.00934661272913218
39800 0.00934422668069601
39900 0.0093339579179883
40000 0.0093359611928463
40200 0.00932769849896431
40400 0.00930541381239891
40700 0.00928853545337915
40800 0.00927397329360247
40900 0.00927861221134663
41000 0.00927416700869799
41100 0.00927546992897987
41200 0.00926822237670422
41300 0.00927200354635715
41800 0.00926993694156408
42100 0.00924444012343884
42300 0.00924628786742687
42400 0.00925512425601482
42500 0.00924781057983637
42600 0.00924898870289326
42700 0.00924370996654034
42800 0.00923179183155298
42900 0.00921360589563847
43000 0.0092069311067462
43200 0.0092200618237257
43300 0.00921652931720018
43400 0.00922504905611277
43500 0.00922123622149229
43600 0.00920047890394926
43900 0.00915918499231339
44200 0.00917895697057247
44300 0.00919774174690247
44400 0.00919561181217432
44500 0.00920556206256151
44700 0.00919733289629221
44800 0.00917911343276501
44900 0.00917297787964344
};
\addlegendentry{K1}
\addplot [ultra thick, green!39.2156862745098!black,  ]
table {%
0 0.0636693313717842
100 0.0616101957857609
200 0.0591515451669693
300 0.056608609855175
400 0.0542661361396313
500 0.052734013646841
600 0.0520671382546425
700 0.0517956167459488
900 0.0515038184821606
1000 0.0511078648269176
1100 0.0502656362950802
1200 0.049069419503212
1300 0.0476103611290455
1400 0.0457979328930378
1500 0.0439452715218067
1600 0.0420238375663757
1700 0.039841677993536
1800 0.0371202230453491
1900 0.0341668166220188
2000 0.0311870444566011
2100 0.0285581424832344
2200 0.0263693351298571
2300 0.0247243661433458
2400 0.0234325230121613
2500 0.022318297997117
2600 0.0212215557694435
2700 0.020207554101944
2800 0.0193783231079578
2900 0.0187454055994749
3000 0.0182127896696329
3100 0.0177700202912092
3300 0.0169527269899845
3700 0.0154489735141397
3800 0.0150637710466981
3900 0.0147127136588097
4100 0.0140069387853146
4200 0.0136939836665988
4300 0.0134233459830284
4400 0.013206503354013
4500 0.0130100520327687
4600 0.0128278592601418
4700 0.0126698100939393
4800 0.0125195998698473
4900 0.0123492330312729
5000 0.0121871251612902
5100 0.0120611265301704
5200 0.0119048850610852
5400 0.0116539718583226
5600 0.0114352470263839
5800 0.0112469913437963
5900 0.011168478988111
6000 0.0110651720315218
6100 0.0109744854271412
6200 0.0109028182923794
6400 0.0106938667595387
6500 0.0106177488341928
6600 0.0105210524052382
6700 0.010431781411171
6800 0.0103582944720984
6900 0.010279942303896
7000 0.0102274091914296
7100 0.0101952403783798
7300 0.0100831184536219
7400 0.0100454483181238
7500 0.009974280372262
7600 0.0099115464836359
7700 0.00987546611577272
7800 0.00981199648231268
7900 0.00977888237684965
8000 0.00973082426935434
8100 0.00966986082494259
8200 0.00959778111428022
8300 0.00957708526402712
8400 0.00951219629496336
8800 0.00930551066994667
8900 0.00924687180668116
9400 0.00904380716383457
9500 0.00899581983685493
9600 0.00894397217780352
9900 0.00881303194910288
10000 0.00877923890948296
10100 0.00873635802417994
10200 0.00868757534772158
10300 0.0086481561884284
10400 0.00861290562897921
10500 0.00858748517930508
10600 0.00857675820589066
10700 0.00854484178125858
10800 0.00851850584149361
10900 0.00850006751716137
11000 0.00843782350420952
11100 0.00841876491904259
11200 0.00842550583183765
11300 0.00839595962315798
11400 0.00834767054766417
11500 0.00834363419562578
11600 0.00830729864537716
11700 0.00824049208313227
11800 0.00823257956653833
11900 0.00823179725557566
12000 0.00821755640208721
12100 0.00817333906888962
12200 0.00816441979259253
12300 0.00812389049679041
12400 0.00806570239365101
12500 0.00803945679217577
12600 0.00803368631750345
12800 0.00798416137695312
12900 0.00797977484762669
13000 0.00794460158795118
13100 0.00793042220175266
13200 0.00791227072477341
13300 0.00785581395030022
13400 0.00785370077937841
13700 0.00776792969554663
13800 0.00775742484256625
13900 0.00770573597401381
14000 0.0077065946534276
14100 0.00766707956790924
14200 0.00763509841635823
14300 0.00761585449799895
14400 0.00758828921243548
14500 0.00754766492173076
14600 0.00752871995791793
14700 0.00752995582297444
14800 0.00751180574297905
15000 0.00749993417412043
15100 0.00748572265729308
15200 0.00743690924718976
15300 0.00742654642090201
15400 0.00738267740234733
15500 0.00735791493207216
15600 0.00735327554866672
15800 0.00732340756803751
15900 0.00732366042211652
16000 0.0072951945476234
16100 0.00727213080972433
16200 0.00726671097800136
16300 0.00724473176524043
16400 0.00725755747407675
16500 0.00725650973618031
16700 0.00721756694838405
16800 0.00720739457756281
16900 0.00716118654236197
17100 0.00713297631591558
17200 0.00714020850136876
17300 0.00713144894689322
17400 0.00713521614670753
17500 0.00712566496804357
17600 0.00710163218900561
17700 0.00708444835618138
17800 0.00706219812855124
17900 0.00703598791733384
18000 0.00701454468071461
18100 0.00701524550095201
18200 0.00699186138808727
18400 0.00699354661628604
18500 0.00700252875685692
18600 0.00699510565027595
18700 0.00699543952941895
18900 0.00697299838066101
19100 0.00694476626813412
19200 0.00695042638108134
19300 0.00694147683680058
19400 0.00694136647507548
19500 0.00692575657740235
19800 0.00688729155808687
19900 0.00688367011025548
20000 0.00686950609087944
20100 0.00685879262164235
20200 0.00683749513700604
20300 0.00684309052303433
20400 0.00682314159348607
20600 0.00682562170550227
20700 0.00680058822035789
20800 0.00678429659456015
21100 0.0067614708095789
21200 0.00676824478432536
21300 0.00674325507134199
21500 0.00673011131584644
21600 0.00673046242445707
21700 0.00673577003180981
21800 0.00673368852585554
21900 0.00672745518386364
22000 0.00672728149220347
22100 0.00670728739351034
22200 0.00669614318758249
22300 0.00670383777469397
22400 0.00669413991272449
22500 0.00668069580569863
22600 0.00667899427935481
22800 0.00666111428290606
22900 0.00666390871629119
23000 0.00665836501866579
23200 0.00663631642237306
23300 0.0066325357183814
23400 0.00661565503105521
23500 0.00660448195412755
23700 0.00661436608061194
23800 0.00660608476027846
23900 0.00660921912640333
24100 0.00657957326620817
24200 0.0065732947550714
24300 0.00656286720186472
24400 0.00654955022037029
24500 0.00657332735136151
24600 0.00657051336020231
24700 0.00655317166820168
24900 0.00654082233086228
25000 0.00651992158964276
25100 0.00651804637163877
25200 0.00650363089516759
25300 0.00650592008605599
25600 0.00646909046918154
25700 0.00647222343832254
25800 0.00647991336882114
25900 0.00648098066449165
26000 0.00649002427235246
26100 0.006472856272012
26200 0.00646788300946355
26300 0.00642827246338129
26400 0.00643660267814994
26500 0.00642102444544435
26600 0.00642681121826172
26700 0.00640597240999341
26800 0.00642410945147276
26900 0.00641056708991528
27200 0.00640031648799777
27600 0.00635887775570154
27700 0.00637125829234719
27800 0.00637151347473264
27900 0.00639513274654746
28000 0.00639564171433449
28100 0.0064159082248807
28200 0.00640672165900469
28300 0.00637998385354877
28400 0.00634904112666845
28500 0.00633005984127522
28600 0.00629455083981156
28700 0.00627932650968432
28800 0.00628113653510809
28900 0.00628820946440101
29000 0.00630086380988359
29100 0.00630574300885201
29200 0.0063220513984561
29400 0.00630113342776895
29500 0.00628493446856737
29600 0.00627970602363348
29700 0.00626357551664114
29900 0.00626678438857198
30200 0.00626503676176071
30400 0.00627341400831938
};
\addlegendentry{K2}
\addplot [ultra thick, color0]
table {%
0 0.0487121939659119
100 0.0426958575844765
200 0.0361093617975712
300 0.0324471592903137
400 0.0297905020415783
500 0.0269802305847406
600 0.0240863561630249
700 0.0222672522068024
800 0.0212216656655073
900 0.0201710388064384
1000 0.0191998947411776
1100 0.018395995721221
1200 0.0176032297313213
1300 0.0168205741792917
1400 0.016115939244628
1500 0.0154903875663877
1600 0.0149311581626534
1700 0.0144285233691335
1800 0.014001926407218
1900 0.0136566897854209
2000 0.0133321834728122
2100 0.0130836386233568
2200 0.0128151923418045
2300 0.0126295424997807
2400 0.0124217243865132
2600 0.0120522808283567
2700 0.0119481533765793
2800 0.011776078492403
2900 0.0116331242024899
3000 0.0114999925717711
3100 0.0113804014399648
3200 0.0112479450181127
3400 0.0110076749697328
3500 0.0109060537070036
3600 0.0108167929574847
3700 0.0107152890414
3900 0.0105875888839364
4000 0.0104880267754197
4400 0.0101884780451655
4500 0.0101322596892715
4600 0.0100543973967433
4900 0.00988142658025026
5100 0.0097825713455677
5300 0.0096328305080533
5400 0.00958024058490992
5500 0.00954202376306057
5600 0.0094934981316328
5700 0.00945554487407207
5800 0.00942911859601736
5900 0.00938197132200003
6000 0.00931846536695957
6100 0.00926584098488092
6200 0.00921857357025146
6300 0.0091642402112484
6700 0.00903058052062988
6800 0.00898326002061367
6900 0.0089489771053195
7000 0.00893018115311861
7100 0.00890559982508421
7200 0.00887713301926851
7300 0.00885740295052528
7400 0.00881237909197807
7500 0.00877890642732382
7600 0.00872748531401157
7700 0.00872165616601706
7800 0.00868722703307867
7900 0.00865977630019188
8000 0.00860852282494307
8100 0.0085899094119668
8200 0.00853032153099775
8300 0.00850744359195232
8400 0.00847636722028255
8500 0.00845384784042835
8600 0.00844127964228392
8700 0.00842215772718191
8800 0.00838591810315847
8900 0.0083590978756547
9000 0.00834658928215504
9100 0.00829213485121727
9200 0.00825258903205395
9300 0.00823508854955435
9400 0.00822235830128193
9500 0.00818688794970512
9600 0.00815774407237768
9700 0.00814289320260286
9800 0.00811795610934496
9900 0.00808227062225342
10000 0.00805432163178921
10100 0.00804061349481344
10200 0.00801081117242575
10300 0.00799286272376776
10400 0.00796616729348898
10500 0.0079668927937746
10600 0.00796158984303474
10700 0.00794385932385921
10800 0.00789716467261314
10900 0.00788242090493441
11000 0.00782430823892355
11100 0.00779139390215278
11200 0.00777262169867754
11300 0.00777482846751809
11400 0.00773416506126523
11500 0.0077108689583838
11600 0.00767653062939644
11800 0.00763432309031487
12000 0.00764265097677708
12100 0.00763182574883103
12200 0.00760032562538981
12300 0.00757300807163119
12400 0.00753432232886553
12500 0.00750650418922305
12600 0.00748786795884371
12800 0.00746526848524809
12900 0.00748158106580377
13000 0.00746500631794333
13100 0.00745733035728335
13200 0.00743938377127051
13300 0.00740501051768661
13400 0.0073643121868372
13500 0.00734662171453238
13600 0.00732228578999639
13700 0.00730225862935185
13800 0.00727209867909551
13900 0.00727183138951659
14000 0.00725928274914622
14200 0.00722460728138685
14300 0.00721531640738249
14400 0.00717562157660723
14500 0.00714835477992892
14600 0.00713882502168417
14700 0.00713416654616594
14800 0.00713934237137437
14900 0.0071297069080174
15000 0.0071255280636251
15200 0.00708035798743367
15300 0.0070519121363759
15400 0.00702916597947478
15500 0.00702512310817838
15600 0.00701563432812691
15800 0.00700660469010472
15900 0.00700762402266264
16000 0.00697306729853153
16300 0.00691866176202893
16400 0.00690600974485278
16500 0.00690390216186643
16600 0.00690909288823605
16700 0.0069062071852386
16800 0.00690694665536284
16900 0.00691383564844728
17000 0.00691629946231842
17100 0.00689756823703647
17200 0.00689606880769134
17300 0.00687453849241138
17400 0.00686330907046795
17500 0.00684899464249611
17600 0.00685212761163712
17700 0.00684131775051355
17800 0.00684560043737292
17900 0.00682157604023814
18000 0.00681652966886759
18100 0.00679939705878496
18200 0.00678672920912504
18300 0.00676972744986415
18400 0.00676731206476688
18500 0.00675238622352481
18600 0.00676473043859005
18700 0.00675232335925102
18800 0.00677275704219937
18900 0.00677716778591275
19000 0.00677128462120891
19100 0.00674824696034193
19200 0.00675428844988346
19400 0.00670174043625593
19500 0.00671362737193704
19600 0.00670165941119194
19700 0.00669604772701859
19800 0.00668724207207561
19900 0.00669057993218303
20000 0.00667594093829393
20100 0.00667756469920278
20200 0.00666732667014003
20300 0.00667160283774137
20400 0.00666739232838154
20500 0.00665140151977539
20600 0.00665585044771433
20700 0.00663461489602923
20800 0.00661878660321236
21100 0.00658990442752838
21200 0.00661287363618612
21300 0.00662310840561986
21400 0.00663873227313161
21700 0.00661026779562235
21900 0.00658456329256296
22000 0.00659688329324126
22100 0.00658799847587943
22200 0.00657478906214237
22300 0.00656673032790422
22400 0.00656498223543167
22600 0.00654835626482964
22800 0.0065492014400661
22900 0.00653491076081991
23000 0.00653171492740512
23100 0.00653201621025801
23300 0.00652461219578981
23400 0.00652441848069429
23500 0.00651933439075947
23600 0.00652767904102802
23700 0.00653119152411819
23800 0.00652050832286477
23900 0.00652071600779891
24000 0.00652586575597525
24200 0.00650202436372638
24500 0.00650960672646761
24600 0.00650420226156712
24700 0.00650765234604478
24800 0.00650661624968052
24900 0.00650990707799792
25000 0.00649676145985723
25100 0.00650022923946381
25200 0.00649224780499935
25300 0.00649564899504185
25400 0.00648325122892857
25500 0.00648376019671559
25600 0.00648113759234548
25700 0.00647264998406172
25800 0.0064590941183269
25900 0.00646715192124248
26000 0.00647055404260755
26100 0.00646311277523637
26200 0.00646715192124248
26300 0.00646737543866038
26400 0.00645805848762393
26500 0.00645290920510888
26600 0.00645418139174581
26700 0.00644650403410196
26800 0.00644372310489416
26900 0.0064363656565547
27000 0.00642520608380437
27300 0.00644168956205249
27800 0.00643737986683846
27900 0.00644607609137893
28000 0.00644273636862636
28200 0.00642417278140783
28300 0.00642636697739363
28400 0.006411362439394
28500 0.00641881441697478
28600 0.00641814852133393
28700 0.00642293179407716
28800 0.0064142388291657
28900 0.00642024539411068
29000 0.00640676729381084
29100 0.00641617923974991
29200 0.00641408003866673
29300 0.00640381034463644
29400 0.00640069600194693
29500 0.00641500297933817
29600 0.00640007760375738
29700 0.00639019114896655
29800 0.00639793137088418
30000 0.00637311907485127
30100 0.00637235678732395
30200 0.00636432971805334
30300 0.00636077020317316
30400 0.00637532724067569
30600 0.00637446995824575
30700 0.0063773961737752
31100 0.00636162608861923
31200 0.00636359956115484
31300 0.00636226171627641
};
\addlegendentry{K3}
\addplot [ultra thick, white!40.2745098039216!black,  ]
table {%
0 0.0491654649376869
100 0.0431270524859428
200 0.0363886058330536
300 0.0322390757501125
400 0.029566241428256
500 0.0267833285033703
600 0.0239019766449928
700 0.0222393739968538
800 0.0211947374045849
1000 0.0191011186689138
1100 0.0183004960417747
1200 0.017491614446044
1300 0.0166925191879272
1400 0.0160186029970646
1500 0.0154156452044845
1600 0.0148615119978786
1700 0.0143752349540591
1800 0.0139840040355921
1900 0.0136323571205139
2000 0.0133131425827742
2100 0.0130619397386909
2200 0.0128217302262783
2300 0.0126251894980669
2400 0.0124376341700554
2500 0.0122464932501316
2600 0.0120835639536381
2700 0.0119637316092849
2800 0.0118101360276341
3000 0.0115632163360715
3100 0.0114359250292182
3200 0.0112884668633342
3300 0.011163629591465
3400 0.0110217668116093
3500 0.0109107429161668
3600 0.0107890255749226
3700 0.0106936963275075
3900 0.010522898286581
4000 0.0104267029091716
4200 0.0103143937885761
4500 0.0101122660562396
4600 0.0100573729723692
4700 0.00998013559728861
4800 0.00991978775709867
4900 0.00985534675419331
5000 0.00980902370065451
5100 0.00974320992827415
5200 0.00968482624739408
5300 0.00960940588265657
5500 0.00951881427317858
5600 0.0094665763899684
5700 0.00944928172975779
5800 0.00941809918731451
5900 0.00937694031745195
6100 0.00926348101347685
6200 0.00918970163911581
6500 0.00908433645963669
6700 0.00900416541844606
6800 0.00895731337368488
6900 0.00892392732203007
7000 0.00890197791159153
7200 0.008890968747437
7300 0.0088575342670083
7500 0.00876447465270758
7600 0.00869392044842243
7700 0.00865115225315094
7800 0.00863513350486755
7900 0.00860566459596157
8000 0.00856986735016108
8100 0.00854891911149025
8200 0.0085081160068512
8300 0.00847732182592154
8400 0.00845758896321058
8500 0.00843316502869129
8600 0.00841703172773123
8700 0.00839633774012327
8900 0.00832046195864677
9000 0.00829114764928818
9100 0.00825550686568022
9300 0.00821702461689711
9600 0.00814297422766685
9700 0.00810384564101696
9900 0.00806174520403147
10000 0.00805004313588142
10300 0.00795845221728086
10400 0.007919667288661
10600 0.0078977020457387
10700 0.00788183230906725
10800 0.00785555131733418
10900 0.00785235594958067
11000 0.00780161889269948
11100 0.00778468558564782
11200 0.00777348829433322
11300 0.00776983192190528
11400 0.00773034011945128
11500 0.00770722096785903
11600 0.00766965607181191
11700 0.00762546854093671
11800 0.007601547986269
12200 0.00759883597493172
12300 0.00756706530228257
12500 0.00749367056414485
12600 0.0074729691259563
12700 0.00743910623714328
12800 0.0074173379689455
12900 0.00741233956068754
13000 0.00738657312467694
13100 0.00735669955611229
13200 0.00735389301553369
13300 0.00732952076941729
13400 0.00729143479838967
13500 0.00728286989033222
13600 0.00726943230256438
13700 0.00723985722288489
13800 0.00721747940406203
13900 0.00722115766257048
14000 0.00720434868708253
14100 0.00717652728781104
14300 0.00716931745409966
14400 0.00714542763307691
14500 0.00713379448279738
14600 0.00715325772762299
14700 0.00713306991383433
14800 0.0071240495890379
14900 0.00712234852835536
15000 0.00710995309054852
15100 0.00706437323242426
15200 0.00705174589529634
15300 0.00702734850347042
15400 0.00698553072288632
15500 0.00696639018133283
15600 0.00696740765124559
15700 0.00695754634216428
15800 0.00695163989439607
15900 0.00696130562573671
16000 0.00695728277787566
16100 0.00694859120994806
16200 0.0069310967810452
16300 0.00693143159151077
16400 0.00692609883844852
16500 0.00692749815061688
16600 0.00690179551020265
16700 0.00690514175221324
16800 0.00687147118151188
16900 0.00686961924657226
17000 0.00683229090645909
17100 0.00682808784767985
17200 0.00680337753146887
17300 0.00679746409878135
17400 0.00677926652133465
17500 0.00678788777440786
17700 0.00675950758159161
17800 0.00674878805875778
17900 0.0067204306833446
18000 0.00667623756453395
18100 0.00666326470673084
18200 0.00666646286845207
18300 0.00663827266544104
18400 0.00662212306633592
18500 0.00662872800603509
18600 0.00663073733448982
18700 0.00661459844559431
18800 0.00662781484425068
18900 0.00662665441632271
19200 0.00656062643975019
19300 0.00654842099174857
19400 0.00652729533612728
19500 0.00652823410928249
19600 0.00649898778647184
19700 0.0065004825592041
19800 0.00647363811731339
20000 0.00646058702841401
20100 0.00646686414256692
20300 0.00644265860319138
20600 0.00641530239954591
20700 0.00640068203210831
20800 0.00640780152752995
21000 0.00639104750007391
21100 0.00638904422521591
21200 0.00638211378827691
21300 0.0063691632822156
21400 0.00637227622792125
21500 0.00636223005130887
21600 0.00636280281469226
21700 0.00635970523580909
21800 0.00635188585147262
21900 0.00635099364444613
22000 0.00634702015668154
22100 0.00633440166711807
22300 0.00633064704015851
22400 0.00632250960916281
22600 0.00632748520001769
22800 0.00632138177752495
22900 0.00632877415046096
23100 0.00631338777020574
23200 0.00631086155772209
23300 0.00631469069048762
23400 0.00630536209791899
23500 0.00630208477377892
23600 0.00630302261561155
23700 0.00631025526672602
23800 0.0063051232136786
23900 0.00630424777045846
24000 0.00629758881404996
24100 0.00630089500918984
24200 0.00629518646746874
24300 0.00630065612494946
24500 0.00629995763301849
24600 0.00629375595599413
24900 0.00625915499404073
25100 0.00625198800116777
25200 0.006259361281991
25300 0.00625726534053683
25400 0.0062523209489882
25500 0.00625461060553789
25600 0.00624918797984719
25700 0.00623656855896115
25800 0.00623590126633644
25900 0.00624297466129065
26000 0.00623871572315693
26100 0.00624200468882918
26200 0.00625492632389069
26400 0.00624556606635451
26500 0.00624944502487779
26600 0.00624449970200658
26700 0.00622663414105773
27000 0.00623025838285685
27100 0.00624888576567173
27300 0.00624442100524902
27400 0.00623548682779074
27500 0.00623049819841981
27600 0.00622153282165527
27800 0.00622361665591598
27900 0.00623060762882233
28200 0.00621622381731868
28500 0.00619111023843288
28600 0.00618561031296849
28800 0.0061962278559804
29000 0.00619509862735868
29300 0.00616957247257233
29400 0.00617508869618177
29500 0.00616917619481683
29600 0.00616701599210501
29700 0.00616855639964342
29800 0.00617361115291715
29900 0.00616327952593565
30000 0.00616409117355943
30100 0.00615948066115379
30200 0.00616207160055637
30300 0.00615123240277171
30400 0.00614937208592892
30500 0.00615022936835885
30700 0.00614166306331754
30800 0.00614929106086493
30900 0.00615096231922507
31000 0.00613563740625978
31100 0.00614048633724451
31300 0.00614302838221192
31400 0.00613815058022738
31500 0.00613794149830937
31600 0.0061268019489944
31700 0.00611918838694692
31800 0.00611540349200368
31900 0.00611745519563556
32000 0.00613055331632495
32100 0.0061316336505115
32300 0.00614123465493321
32400 0.00613233400508761
32500 0.00611991714686155
32600 0.00612808996811509
32700 0.00611928245052695
};
\addlegendentry{K4}
