# Supplementary material for: Neural Networks with Physics-Informed Architectures and Constraints for Dynamical Systems Modeling
Source: arXiv:2109.06407 source file (2022-12-12)
Supplement: Supplementary file 4 [file traj_err_data.tex]

\definecolor{color0}{rgb}{1,0,1}

\path [fill=red, fill opacity=0.4, ultra thick]
(axis cs:1,0.383586272763004)
--(axis cs:1,0.341202610256376)
--(axis cs:10,0.367361768217054)
--(axis cs:25,0.319796351289705)
--(axis cs:75,0.327496231149024)
--(axis cs:200,0.302293175970288)
--(axis cs:500,0.299483923885149)
--(axis cs:500,0.408135160747947)
--(axis cs:500,0.408135160747947)
--(axis cs:200,0.407625694391887)
--(axis cs:75,0.436331474775788)
--(axis cs:25,0.425815033510392)
--(axis cs:10,0.442076923031832)
--(axis cs:1,0.383586272763004)
--cycle;

\path [fill=blue, fill opacity=0.4, ultra thick]
(axis cs:1,0.378788589702575)
--(axis cs:1,0.334688626313886)
--(axis cs:10,0.247467385134213)
--(axis cs:25,0.191879685682561)
--(axis cs:75,0.168319706635742)
--(axis cs:200,0.130946656629393)
--(axis cs:500,0.135532023953662)
--(axis cs:500,0.167496070424621)
--(axis cs:500,0.167496070424621)
--(axis cs:200,0.175287994115066)
--(axis cs:75,0.203453582057347)
--(axis cs:25,0.236824416902666)
--(axis cs:10,0.298414471136665)
--(axis cs:1,0.378788589702575)
--cycle;

\path [fill=green!50.1960784313725!black, fill opacity=0.4, ultra thick]
(axis cs:1,0.605682180861764)
--(axis cs:1,0.531938436029615)
--(axis cs:10,0.156418200779452)
--(axis cs:25,0.128638107683799)
--(axis cs:75,0.10911213326964)
--(axis cs:200,0.115090025036464)
--(axis cs:500,0.111470364318783)
--(axis cs:500,0.147809566878869)
--(axis cs:500,0.147809566878869)
--(axis cs:200,0.153399032182911)
--(axis cs:75,0.140587884401561)
--(axis cs:25,0.165873101743983)
--(axis cs:10,0.2024450106049)
--(axis cs:1,0.605682180861764)
--cycle;

\path [fill=color0, fill opacity=0.4, ultra thick]
(axis cs:1,0.599461083321354)
--(axis cs:1,0.527050921055466)
--(axis cs:10,0.379342079288971)
--(axis cs:25,0.146077175817807)
--(axis cs:75,0.122862885020942)
--(axis cs:200,0.112970145249631)
--(axis cs:500,0.113280933710017)
--(axis cs:500,0.155025004017252)
--(axis cs:500,0.155025004017252)
--(axis cs:200,0.143993104548496)
--(axis cs:75,0.158711252659485)
--(axis cs:25,0.183024958214832)
--(axis cs:10,0.448118709653378)
--(axis cs:1,0.599461083321354)
--cycle;

\path [fill=white!50.1960784313725!black, fill opacity=0.4, ultra thick]
(axis cs:1,0.603132169970756)
--(axis cs:1,0.530037687536275)
--(axis cs:10,0.386128986556324)
--(axis cs:25,0.146518969815949)
--(axis cs:75,0.126070911216527)
--(axis cs:200,0.114498525452292)
--(axis cs:500,0.108960797960616)
--(axis cs:500,0.145501110774923)
--(axis cs:500,0.145501110774923)
--(axis cs:200,0.149259511014837)
--(axis cs:75,0.154341881685116)
--(axis cs:25,0.181061946002654)
--(axis cs:10,0.460149184044299)
--(axis cs:1,0.603132169970756)
--cycle;

\addplot [ ultra thick, red, mark=*, mark size=1.5, mark options={solid}]
table {%
1 0.362394481897354
10 0.404719293117523
25 0.372805684804916
75 0.381913870573044
200 0.354959458112717
500 0.353809475898743
};
\addplot [ ultra thick, blue, mark=*, mark size=1.5, mark options={solid}]
table {%
1 0.356738537549973
10 0.272940933704376
25 0.214352056384087
75 0.185886666178703
200 0.153117299079895
500 0.151514068245888
};
\addplot [ ultra thick, green!50.1960784313725!black, mark=*, mark size=1.5, mark options={solid}]
table {%
1 0.568810284137726
10 0.179431572556496
25 0.147255569696426
75 0.124850012362003
200 0.13424451649189
500 0.129639953374863
};
\addplot [ ultra thick, color0, mark=*, mark size=1.5, mark options={solid}]
table {%
1 0.563256025314331
10 0.413730323314667
25 0.164551079273224
75 0.140787035226822
200 0.128481641411781
500 0.134152933955193
};
\addplot [ ultra thick, white!50.1960784313725!black, mark=*, mark size=1.5, mark options={solid}]
table {%
1 0.566584944725037
10 0.423139154911041
25 0.163790449500084
75 0.140206411480904
200 0.131879016757011
500 0.127230957150459
};
