# Supplementary material for: Neural Networks with Physics-Informed Architectures and Constraints for Dynamical Systems Modeling
Source: arXiv:2109.06407 source file (2022-12-12)
Supplement: Supplementary file 6 [file error_vs_trajectory_count_data.tex]

\definecolor{color0}{rgb}{1,0,1}

\path [fill=red, fill opacity=0.4, ultra thick]
(axis cs:1,0.358156810349748)
--(axis cs:1,0.288685483626368)
--(axis cs:5,0.0153974990861162)
--(axis cs:10,0.016051068814258)
--(axis cs:20,0.029675446614998)
--(axis cs:100,0.014277179006959)
--(axis cs:100,0.0283372811794607)
--(axis cs:100,0.0283372811794607)
--(axis cs:20,0.0418484036759897)
--(axis cs:10,0.0231407828796545)
--(axis cs:5,0.0233957937561589)
--(axis cs:1,0.358156810349748)
--cycle;

\path [fill=blue, fill opacity=0.4, ultra thick]
(axis cs:1,0.112383269958444)
--(axis cs:1,0.08778626405545)
--(axis cs:5,0.0130619439732912)
--(axis cs:10,0.0160178190904799)
--(axis cs:20,0.0173217215759679)
--(axis cs:100,0.0127757712234337)
--(axis cs:100,0.0171697606795847)
--(axis cs:100,0.0171697606795847)
--(axis cs:20,0.0226137352424347)
--(axis cs:10,0.0264860883282459)
--(axis cs:5,0.0162948465391275)
--(axis cs:1,0.112383269958444)
--cycle;

\path [fill=color0, fill opacity=0.4, ultra thick]
(axis cs:1,0.0205045290709664)
--(axis cs:1,0.0120254340172996)
--(axis cs:5,0.0135003245620557)
--(axis cs:10,0.0129304084580649)
--(axis cs:20,0.0130269641273556)
--(axis cs:100,0.0146339844868641)
--(axis cs:100,0.0220763006689502)
--(axis cs:100,0.0220763006689502)
--(axis cs:20,0.0228135113984045)
--(axis cs:10,0.019268864106573)
--(axis cs:5,0.0222284630625251)
--(axis cs:1,0.0205045290709664)
--cycle;

\addplot [ultra thick, red, mark=*, mark size=1.5, mark options={solid}]
table {%
1 0.323421210050583
5 0.0193966459482908
10 0.0195959247648716
20 0.0357619263231754
100 0.0213072281330824
};
\addlegendentry{Baseline}
\addplot [ultra thick, blue, mark=*, mark size=1.5, mark options={solid}]
table {%
1 0.100084774196148
5 0.0146783944219351
10 0.0212519560009241
20 0.0199677310883999
100 0.014972765929997
};
\addlegendentry{K1}
\addplot [ultra thick, color0, mark=*, mark size=1.5, mark options={solid}]
table {%
1 0.0162649787962437
5 0.0178643949329853
10 0.0160996317863464
20 0.0179202351719141
100 0.0183551404625177
};
\addlegendentry{K2}
