# Supplementary material for: Neural Networks with Physics-Informed Architectures and Constraints for Dynamical Systems Modeling
Source: arXiv:2109.06407 source file (2022-12-12)
Supplement: Supplementary file 7 [file phi_1_dot_dynamics_data.tex]

\addplot [ultra thick, green!50.1960784313725!black, dashed]
table {%
0 -0.480681180953979
0.0199999809265137 -0.534592866897583
0.0399999618530273 -0.585776567459106
0.059999942779541 -0.63373589515686
0.0800000429153442 -0.677995204925537
0.0900000333786011 -0.698596954345703
0.100000023841858 -0.718109369277954
0.110000014305115 -0.736482381820679
0.120000004768372 -0.753669261932373
0.129999995231628 -0.769626379013062
0.139999985694885 -0.784313678741455
0.149999976158142 -0.797694206237793
0.159999966621399 -0.809736251831055
0.169999957084656 -0.820409178733826
0.180000066757202 -0.829691648483276
0.190000057220459 -0.837563276290894
0.200000047683716 -0.844009399414062
0.210000038146973 -0.84902012348175
0.220000028610229 -0.852590560913086
0.230000019073486 -0.854719758033752
0.240000009536743 -0.855414390563965
0.25 -0.854681968688965
0.259999990463257 -0.852537393569946
0.269999980926514 -0.848999261856079
0.279999971389771 -0.84408974647522
0.289999961853027 -0.837838292121887
0.299999952316284 -0.830274105072021
0.309999942779541 -0.821432113647461
0.319999933242798 -0.811350345611572
0.330000042915344 -0.800071477890015
0.340000033378601 -0.787639260292053
0.350000023841858 -0.774100303649902
0.360000014305115 -0.759504437446594
0.370000004768372 -0.743903517723083
0.379999995231628 -0.727352380752563
0.399999976158142 -0.691623210906982
0.419999957084656 -0.652780294418335
0.440000057220459 -0.61131489276886
0.460000038146973 -0.567732810974121
0.490000009536743 -0.499534368515015
0.579999923706055 -0.291450500488281
0.600000023841858 -0.247876167297363
0.620000004768372 -0.206328868865967
0.639999985694885 -0.16722583770752
0.660000085830688 -0.130927562713623
0.680000066757202 -0.0977267026901245
0.690000057220459 -0.0823591947555542
0.700000047683716 -0.0678414106369019
0.710000038146973 -0.0541881322860718
0.720000028610229 -0.0414085388183594
0.730000019073486 -0.0295075178146362
0.740000009536743 -0.018484354019165
0.75 -0.00833356380462646
0.759999990463257 0.000954508781433105
0.769999980926514 0.00939404964447021
0.779999971389771 0.0170028209686279
0.789999961853027 0.0238025188446045
0.799999952316284 0.0298178195953369
0.809999942779541 0.0350759029388428
0.819999933242798 0.0396065711975098
0.829999923706055 0.0434415340423584
0.839999914169312 0.0466139316558838
0.850000023841858 0.0491580963134766
0.860000014305115 0.0511091947555542
0.870000004768372 0.0525029897689819
0.879999995231628 0.053375244140625
0.889999985694885 0.0537617206573486
0.910000085830688 0.0532193183898926
0.930000066757202 0.0511544942855835
0.950000047683716 0.0478354692459106
0.970000028610229 0.043519139289856
0.990000009536743 0.0384513139724731
1.01999998092651 0.0299577713012695
1.08000004291534 0.0126293897628784
1.10000002384186 0.00762367248535156
1.12000000476837 0.0034252405166626
1.13999998569489 0.000308036804199219
1.1599999666214 -0.00143933296203613
1.16999995708466 -0.00170552730560303
1.17999994754791 -0.00151526927947998
1.19000005722046 -0.000829815864562988
1.20000004768372 0.000390052795410156
1.21000003814697 0.00218319892883301
1.22000002861023 0.00458788871765137
1.23000001907349 0.00764179229736328
1.24000000953674 0.0113810300827026
1.25 0.0158402919769287
1.25999999046326 0.0210517644882202
1.26999998092651 0.027045726776123
1.27999997138977 0.0338486433029175
1.28999996185303 0.0414841175079346
1.29999995231628 0.0499718189239502
1.30999994277954 0.0593267679214478
1.32000005245209 0.0695595741271973
1.33000004291534 0.0806763172149658
1.3400000333786 0.0926774740219116
1.35000002384186 0.105558276176453
1.36000001430511 0.119308710098267
1.37000000476837 0.133913040161133
1.37999999523163 0.149350166320801
1.39999997615814 0.182612419128418
1.41999995708466 0.218823313713074
1.44000005722046 0.25763726234436
1.46000003814697 0.298645615577698
1.48000001907349 0.341387271881104
1.49000000953674 0.363253593444824
};
\addplot [ultra thick, red]
table {%
0 -0.480681180953979
0.0199999809265137 -0.533937335014343
0.0399999618530273 -0.584865212440491
0.059999942779541 -0.63304328918457
0.0800000429153442 -0.678117394447327
0.100000023841858 -0.719638586044312
0.110000014305115 -0.738881587982178
0.120000004768372 -0.757035493850708
0.129999995231628 -0.774103164672852
0.139999985694885 -0.790076971054077
0.149999976158142 -0.804876804351807
0.159999966621399 -0.818463325500488
0.169999957084656 -0.830866694450378
0.180000066757202 -0.842046737670898
0.190000057220459 -0.851926326751709
0.200000047683716 -0.860478520393372
0.210000038146973 -0.867661118507385
0.220000028610229 -0.873458623886108
0.230000019073486 -0.8778235912323
0.240000009536743 -0.880852937698364
0.25 -0.882518291473389
0.259999990463257 -0.882696866989136
0.269999980926514 -0.881384611129761
0.279999971389771 -0.878733515739441
0.289999961853027 -0.874793529510498
0.299999952316284 -0.869491100311279
0.309999942779541 -0.862787485122681
0.319999933242798 -0.854731798171997
0.330000042915344 -0.84534478187561
0.340000033378601 -0.83466362953186
0.350000023841858 -0.822812676429749
0.360000014305115 -0.80984902381897
0.370000004768372 -0.795789003372192
0.379999995231628 -0.780634999275208
0.389999985694885 -0.764451861381531
0.399999976158142 -0.747335076332092
0.419999957084656 -0.710529088973999
0.440000057220459 -0.670581579208374
0.460000038146973 -0.628018140792847
0.480000019073486 -0.583622694015503
0.509999990463257 -0.514552474021912
0.589999914169312 -0.327289938926697
0.610000014305115 -0.283124804496765
0.629999995231628 -0.241012930870056
0.649999976158142 -0.201382875442505
0.670000076293945 -0.16428279876709
0.690000057220459 -0.129839062690735
0.700000047683716 -0.113773465156555
0.710000038146973 -0.0986599922180176
0.720000028610229 -0.084526538848877
0.730000019073486 -0.0713659524917603
0.740000009536743 -0.0591596364974976
0.75 -0.0478278398513794
0.759999990463257 -0.0373440980911255
0.769999980926514 -0.0277142524719238
0.779999971389771 -0.0189712047576904
0.789999961853027 -0.011139988899231
0.799999952316284 -0.00418102741241455
0.809999942779541 0.00199210643768311
0.819999933242798 0.00741851329803467
0.829999923706055 0.0121356248855591
0.839999914169312 0.0161707401275635
0.850000023841858 0.0195292234420776
0.860000014305115 0.0222147703170776
0.870000004768372 0.0242235660552979
0.879999995231628 0.0256065130233765
0.889999985694885 0.0263971090316772
0.899999976158142 0.0266557931900024
0.920000076293945 0.0257819890975952
0.940000057220459 0.0234013795852661
0.960000038146973 0.0196982622146606
0.980000019073486 0.0149115324020386
1 0.00930929183959961
1.02999997138977 1.19209289550781e-05
1.0900000333786 -0.0188620090484619
1.11000001430511 -0.0244046449661255
1.12999999523163 -0.0291825532913208
1.14999997615814 -0.0329784154891968
1.16999995708466 -0.0356303453445435
1.19000005722046 -0.0368642807006836
1.20000004768372 -0.0368552207946777
1.21000003814697 -0.0363630056381226
1.22000002861023 -0.035355806350708
1.23000001907349 -0.0337735414505005
1.24000000953674 -0.031586766242981
1.25 -0.0287792682647705
1.25999999046326 -0.0253281593322754
1.26999998092651 -0.021185040473938
1.27999997138977 -0.0162997245788574
1.28999996185303 -0.0105917453765869
1.29999995231628 -0.00401866436004639
1.30999994277954 0.00346684455871582
1.32000005245209 0.0118309259414673
1.33000004291534 0.0210983753204346
1.3400000333786 0.0313328504562378
1.35000002384186 0.0425665378570557
1.36000001430511 0.0547809600830078
1.37000000476837 0.0679537057876587
1.37999999523163 0.0821197032928467
1.38999998569489 0.0973066091537476
1.39999997615814 0.113386034965515
1.4099999666214 0.130399823188782
1.42999994754791 0.167182564735413
1.45000004768372 0.207137584686279
1.47000002861023 0.24984872341156
1.49000000953674 0.295053243637085
};
\addplot [ultra thick, blue]
table {%
0 -0.480681180953979
0.0199999809265137 -0.53441333770752
0.0399999618530273 -0.585434198379517
0.059999942779541 -0.633220195770264
0.0800000429153442 -0.677313566207886
0.0900000333786011 -0.697839498519897
0.100000023841858 -0.717310786247253
0.110000014305115 -0.735682368278503
0.120000004768372 -0.752912998199463
0.129999995231628 -0.768963932991028
0.139999985694885 -0.783799886703491
0.149999976158142 -0.797390818595886
0.159999966621399 -0.809711694717407
0.169999957084656 -0.820731163024902
0.180000066757202 -0.830418109893799
0.190000057220459 -0.838746190071106
0.200000047683716 -0.845715403556824
0.210000038146973 -0.851304769515991
0.220000028610229 -0.855487704277039
0.230000019073486 -0.858273029327393
0.240000009536743 -0.859590530395508
0.25 -0.859293460845947
0.259999990463257 -0.857344746589661
0.269999980926514 -0.85369610786438
0.279999971389771 -0.848421931266785
0.289999961853027 -0.841752052307129
0.299999952316284 -0.83400547504425
0.309999942779541 -0.825271129608154
0.319999933242798 -0.815570473670959
0.330000042915344 -0.804920673370361
0.340000033378601 -0.793414950370789
0.350000023841858 -0.781076908111572
0.360000014305115 -0.767951488494873
0.370000004768372 -0.754027009010315
0.379999995231628 -0.739176273345947
0.389999985694885 -0.723389625549316
0.399999976158142 -0.706707835197449
0.419999957084656 -0.67083215713501
0.440000057220459 -0.631972551345825
0.460000038146973 -0.590606212615967
0.480000019073486 -0.547114610671997
0.509999990463257 -0.478955626487732
0.589999914169312 -0.293729662895203
0.610000014305115 -0.249775290489197
0.629999995231628 -0.207550883293152
0.649999976158142 -0.167373061180115
0.670000076293945 -0.129587292671204
0.690000057220459 -0.0945466756820679
0.710000038146973 -0.0625811815261841
0.720000028610229 -0.0478248596191406
0.730000019073486 -0.0339134931564331
0.740000009536743 -0.0208667516708374
0.75 -0.00870442390441895
0.759999990463257 0.00255918502807617
0.769999980926514 0.012919545173645
0.779999971389771 0.022374153137207
0.789999961853027 0.0309228897094727
0.799999952316284 0.0385514497756958
0.809999942779541 0.0452582836151123
0.819999933242798 0.0510549545288086
0.829999923706055 0.0559570789337158
0.839999914169312 0.0599836111068726
0.850000023841858 0.0631511211395264
0.860000014305115 0.0654876232147217
0.870000004768372 0.0670340061187744
0.879999995231628 0.067826509475708
0.889999985694885 0.0679111480712891
0.899999976158142 0.0673277378082275
0.910000085830688 0.0661189556121826
0.920000076293945 0.0643236637115479
0.930000066757202 0.0619925260543823
0.940000057220459 0.0591762065887451
0.960000038146973 0.0522409677505493
0.980000019073486 0.0438448190689087
1 0.0343871116638184
1.02999997138977 0.0190199613571167
1.07000005245209 -0.00167667865753174
1.0900000333786 -0.0112566947937012
1.11000001430511 -0.0198639631271362
1.12999999523163 -0.027069091796875
1.13999998569489 -0.0300222635269165
1.14999997615814 -0.0324832201004028
1.1599999666214 -0.0343992710113525
1.16999995708466 -0.0357130765914917
1.17999994754791 -0.0363837480545044
1.19000005722046 -0.03635573387146
1.20000004768372 -0.035542368888855
1.21000003814697 -0.0339163541793823
1.22000002861023 -0.0314515829086304
1.23000001907349 -0.0281262397766113
1.24000000953674 -0.0239143371582031
1.25 -0.0187770128250122
1.25999999046326 -0.0126882791519165
1.26999998092651 -0.00563549995422363
1.27999997138977 0.00239253044128418
1.28999996185303 0.0114148855209351
1.29999995231628 0.0214848518371582
1.30999994277954 0.0326372385025024
1.32000005245209 0.0448756217956543
1.33000004291534 0.0581732988357544
1.3400000333786 0.0724983215332031
1.35000002384186 0.0878150463104248
1.36000001430511 0.104088187217712
1.37000000476837 0.121287822723389
1.38999998569489 0.158351421356201
1.4099999666214 0.198709726333618
1.42999994754791 0.241916656494141
1.45000004768372 0.287535667419434
1.47000002861023 0.335330963134766
1.49000000953674 0.385026454925537
};
\addplot [ultra thick, color0]
table {%
0 -0.480681180953979
0.0199999809265137 -0.533701658248901
0.0399999618530273 -0.584283113479614
0.059999942779541 -0.632001161575317
0.0800000429153442 -0.67646336555481
0.100000023841858 -0.717246770858765
0.110000014305115 -0.736133575439453
0.120000004768372 -0.753963232040405
0.129999995231628 -0.77069890499115
0.139999985694885 -0.786286473274231
0.149999976158142 -0.800630569458008
0.159999966621399 -0.813700675964355
0.169999957084656 -0.825458288192749
0.180000066757202 -0.835871696472168
0.190000057220459 -0.844941377639771
0.200000047683716 -0.852668285369873
0.210000038146973 -0.858974933624268
0.220000028610229 -0.863850116729736
0.230000019073486 -0.867307662963867
0.240000009536743 -0.869389057159424
0.25 -0.869999408721924
0.259999990463257 -0.869152784347534
0.269999980926514 -0.866823434829712
0.279999971389771 -0.863102197647095
0.289999961853027 -0.858016490936279
0.299999952316284 -0.851571798324585
0.309999942779541 -0.843706727027893
0.319999933242798 -0.834464073181152
0.330000042915344 -0.823864936828613
0.340000033378601 -0.811999201774597
0.350000023841858 -0.798947095870972
0.360000014305115 -0.78480863571167
0.370000004768372 -0.76961624622345
0.379999995231628 -0.753389477729797
0.389999985694885 -0.736169576644897
0.399999976158142 -0.717990279197693
0.419999957084656 -0.678910374641418
0.440000057220459 -0.636818170547485
0.460000038146973 -0.59248948097229
0.480000019073486 -0.546636343002319
0.509999990463257 -0.475138664245605
0.600000023841858 -0.25812292098999
0.620000004768372 -0.21274995803833
0.639999985694885 -0.169509649276733
0.660000085830688 -0.128895998001099
0.680000066757202 -0.0913856029510498
0.690000057220459 -0.0738834142684937
0.700000047683716 -0.0572869777679443
0.710000038146973 -0.0416333675384521
0.720000028610229 -0.0269546508789062
0.730000019073486 -0.0132768154144287
0.740000009536743 -0.000560283660888672
0.75 0.011197566986084
0.759999990463257 0.0219912528991699
0.769999980926514 0.0318268537521362
0.779999971389771 0.0407054424285889
0.789999961853027 0.0486379861831665
0.799999952316284 0.0556635856628418
0.809999942779541 0.0618016719818115
0.819999933242798 0.0670711994171143
0.829999923706055 0.0714943408966064
0.839999914169312 0.075096607208252
0.850000023841858 0.0779038667678833
0.860000014305115 0.0799545049667358
0.870000004768372 0.0812857151031494
0.879999995231628 0.0819382667541504
0.889999985694885 0.0819520950317383
0.899999976158142 0.0813683271408081
0.910000085830688 0.0802266597747803
0.920000076293945 0.0785661935806274
0.930000066757202 0.0764211416244507
0.950000047683716 0.0708441734313965
0.970000028610229 0.0638073682785034
0.990000009536743 0.0556156635284424
1.01999998092651 0.0418750047683716
1.07000005245209 0.0173666477203369
1.10000002384186 0.00310146808624268
1.12000000476837 -0.00552034378051758
1.13999998569489 -0.0130362510681152
1.1599999666214 -0.0190213918685913
1.16999995708466 -0.0213571786880493
1.17999994754791 -0.0232093334197998
1.19000005722046 -0.0245348215103149
1.20000004768372 -0.0253103971481323
1.21000003814697 -0.0255151987075806
1.22000002861023 -0.0251109600067139
1.23000001907349 -0.0240498781204224
1.24000000953674 -0.0222867727279663
1.25 -0.0197802782058716
1.25999999046326 -0.0164929628372192
1.26999998092651 -0.0123827457427979
1.27999997138977 -0.00740730762481689
1.28999996185303 -0.00152742862701416
1.29999995231628 0.0053260326385498
1.30999994277954 0.0132150650024414
1.32000005245209 0.0221627950668335
1.33000004291534 0.0321886539459229
1.3400000333786 0.0433094501495361
1.35000002384186 0.0555286407470703
1.36000001430511 0.0688440799713135
1.37000000476837 0.0832511186599731
1.37999999523163 0.0987035036087036
1.38999998569489 0.115163207054138
1.39999997615814 0.132624864578247
1.4099999666214 0.151066541671753
1.42999994754791 0.190645694732666
1.45000004768372 0.233394145965576
1.47000002861023 0.278836250305176
1.49000000953674 0.326687574386597
};
