# Supplementary material for: Neural Networks with Physics-Informed Architectures and Constraints for Dynamical Systems Modeling
Source: arXiv:2109.06407 source file (2022-12-12)
Supplement: Supplementary file 8 [file phi_1_dynamics_data.tex]

\addplot [ultra thick, green!50.1960784313725!black, dashed]
table {%
0 0.226413011550903
0.00999999046325684 0.221436381340027
0.0199999809265137 0.216188311576843
0.0299999713897705 0.210675477981567
0.0399999618530273 0.204905271530151
0.0499999523162842 0.198884606361389
0.059999942779541 0.192622780799866
0.0700000524520874 0.186128497123718
0.0800000429153442 0.1794114112854
0.0900000333786011 0.172481656074524
0.110000014305115 0.158027529716492
0.129999995231628 0.142857789993286
0.149999976158142 0.127071261405945
0.169999957084656 0.110773086547852
0.190000057220459 0.0940735340118408
0.220000028610229 0.0685198307037354
0.289999961853027 0.00855779647827148
0.309999942779541 -0.00815403461456299
0.330000042915344 -0.0244852304458618
0.350000023841858 -0.0403393507003784
0.370000004768372 -0.0556273460388184
0.389999985694885 -0.0702682733535767
0.409999966621399 -0.0841906070709229
0.419999957084656 -0.0908617973327637
0.430000066757202 -0.0973308086395264
0.440000057220459 -0.103590965270996
0.450000047683716 -0.109636902809143
0.460000038146973 -0.115463256835938
0.470000028610229 -0.121065855026245
0.480000019073486 -0.12644100189209
0.490000009536743 -0.131585836410522
0.5 -0.136497735977173
0.509999990463257 -0.141175150871277
0.519999980926514 -0.145617127418518
0.529999971389771 -0.149823427200317
0.539999961853027 -0.153794288635254
0.549999952316284 -0.157530903816223
0.559999942779541 -0.16103458404541
0.569999933242798 -0.164308309555054
0.579999923706055 -0.167354702949524
0.589999914169312 -0.170177459716797
0.600000023841858 -0.172780871391296
0.610000014305115 -0.175169706344604
0.620000004768372 -0.17734968662262
0.629999995231628 -0.179325461387634
0.639999985694885 -0.181105494499207
0.649999976158142 -0.182695150375366
0.660000085830688 -0.184101819992065
0.670000076293945 -0.185333609580994
0.690000057220459 -0.187304019927979
0.710000038146973 -0.188672780990601
0.730000019073486 -0.189509391784668
0.75 -0.189884424209595
0.769999980926514 -0.189867973327637
0.789999961853027 -0.189528465270996
0.809999942779541 -0.188930511474609
0.839999914169312 -0.187682032585144
0.879999995231628 -0.185638785362244
0.950000047683716 -0.181968092918396
0.990000009536743 -0.180220603942871
1.01999998092651 -0.179185748100281
1.04999995231628 -0.178414940834045
1.08000004291534 -0.177907943725586
1.12000000476837 -0.177595496177673
1.16999995708466 -0.177590131759644
1.22000002861023 -0.177575588226318
1.25 -0.177283048629761
1.26999998092651 -0.176856637001038
1.28999996185303 -0.176172375679016
1.30999994277954 -0.175163269042969
1.33000004291534 -0.173759937286377
1.35000002384186 -0.1718909740448
1.37000000476837 -0.169486045837402
1.38999998569489 -0.166476368904114
1.39999997615814 -0.164724588394165
1.4099999666214 -0.162797331809998
1.41999995708466 -0.160688042640686
1.42999994754791 -0.158389568328857
1.44000005722046 -0.155895709991455
1.45000004768372 -0.153200626373291
1.46000003814697 -0.150299072265625
1.47000002861023 -0.147186517715454
1.48000001907349 -0.143858432769775
1.49000000953674 -0.140312194824219
};
\addlegendentry{True dynamics}
\addplot [ultra thick, red]
table {%
0 0.226413011550903
0.00999999046325684 0.222060441970825
0.0199999809265137 0.217421650886536
0.0299999713897705 0.212526082992554
0.0399999618530273 0.207375764846802
0.0499999523162842 0.201975345611572
0.059999942779541 0.196334719657898
0.0700000524520874 0.190466165542603
0.0800000429153442 0.184371113777161
0.0900000333786011 0.178027868270874
0.100000023841858 0.17143452167511
0.110000014305115 0.164601802825928
0.120000004768372 0.157552480697632
0.139999985694885 0.14286470413208
0.159999966621399 0.127473592758179
0.180000066757202 0.111520767211914
0.200000047683716 0.0951055288314819
0.230000019073486 0.0698764324188232
0.279999971389771 0.0271990299224854
0.309999942779541 0.00162887573242188
0.330000042915344 -0.0150630474090576
0.350000023841858 -0.0313287973403931
0.370000004768372 -0.0470895767211914
0.389999985694885 -0.0622299909591675
0.409999966621399 -0.0766987800598145
0.419999957084656 -0.0836714506149292
0.430000066757202 -0.0904203653335571
0.440000057220459 -0.0969357490539551
0.450000047683716 -0.103223562240601
0.460000038146973 -0.109289646148682
0.470000028610229 -0.115159869194031
0.480000019073486 -0.120819807052612
0.490000009536743 -0.126265645027161
0.5 -0.131484389305115
0.509999990463257 -0.136478662490845
0.519999980926514 -0.141255617141724
0.529999971389771 -0.145810127258301
0.539999961853027 -0.150143504142761
0.549999952316284 -0.154259324073792
0.559999942779541 -0.158154010772705
0.569999933242798 -0.161819458007812
0.579999923706055 -0.165292620658875
0.589999914169312 -0.168593645095825
0.600000023841858 -0.17169713973999
0.610000014305115 -0.174598336219788
0.620000004768372 -0.177281022071838
0.629999995231628 -0.179733037948608
0.639999985694885 -0.181948065757751
0.649999976158142 -0.183930516242981
0.660000085830688 -0.18569016456604
0.670000076293945 -0.18723475933075
0.680000066757202 -0.188575506210327
0.690000057220459 -0.189700961112976
0.710000038146973 -0.191463708877563
0.730000019073486 -0.19281792640686
0.75 -0.193803071975708
0.769999980926514 -0.194424033164978
0.789999961853027 -0.194701671600342
0.809999942779541 -0.194672584533691
0.829999923706055 -0.194268465042114
0.850000023841858 -0.193553447723389
0.879999995231628 -0.19214403629303
0.920000076293945 -0.189854741096497
0.970000028610229 -0.186944246292114
0.990000009536743 -0.186100959777832
1.00999999046326 -0.185535550117493
1.02999997138977 -0.185217976570129
1.05999994277954 -0.185116529464722
1.11000001430511 -0.185573101043701
1.16999995708466 -0.18627667427063
1.21000003814697 -0.187150001525879
1.25999999046326 -0.18818473815918
1.28999996185303 -0.188607811927795
1.30999994277954 -0.188452243804932
1.33000004291534 -0.187934160232544
1.35000002384186 -0.187088966369629
1.37000000476837 -0.18592357635498
1.38999998569489 -0.184400677680969
1.39999997615814 -0.183433294296265
1.4099999666214 -0.18228816986084
1.41999995708466 -0.180956959724426
1.42999994754791 -0.179429650306702
1.44000005722046 -0.177713990211487
1.45000004768372 -0.175803422927856
1.46000003814697 -0.173690676689148
1.47000002861023 -0.171362042427063
1.48000001907349 -0.16879940032959
1.49000000953674 -0.165973424911499
};
\addlegendentry{Baseline}
\addplot [ultra thick, blue]
table {%
0 0.226413011550903
0.00999999046325684 0.221606135368347
0.0199999809265137 0.216527581214905
0.0299999713897705 0.211183428764343
0.0399999618530273 0.205580472946167
0.0499999523162842 0.199726223945618
0.059999942779541 0.193628549575806
0.0700000524520874 0.187296390533447
0.0800000429153442 0.180738806724548
0.0900000333786011 0.173965692520142
0.110000014305115 0.159814119338989
0.129999995231628 0.144928216934204
0.149999976158142 0.129400610923767
0.169999957084656 0.113329529762268
0.190000057220459 0.0968180894851685
0.220000028610229 0.0714603662490845
0.299999952316284 0.00312185287475586
0.319999933242798 -0.0134710073471069
0.340000033378601 -0.0296758413314819
0.360000014305115 -0.04542076587677
0.379999995231628 -0.0606405735015869
0.399999976158142 -0.0752662420272827
0.419999957084656 -0.0892250537872314
0.440000057220459 -0.102450728416443
0.450000047683716 -0.108770489692688
0.460000038146973 -0.114886283874512
0.470000028610229 -0.120792388916016
0.480000019073486 -0.12648332118988
0.490000009536743 -0.131954550743103
0.5 -0.13720166683197
0.509999990463257 -0.142221450805664
0.519999980926514 -0.147010922431946
0.529999971389771 -0.151568293571472
0.539999961853027 -0.1558917760849
0.549999952316284 -0.159980654716492
0.559999942779541 -0.163835048675537
0.569999933242798 -0.167456388473511
0.579999923706055 -0.170847296714783
0.589999914169312 -0.174010038375854
0.600000023841858 -0.176947355270386
0.610000014305115 -0.179662823677063
0.620000004768372 -0.182160615921021
0.629999995231628 -0.184444904327393
0.639999985694885 -0.186520338058472
0.649999976158142 -0.188392281532288
0.660000085830688 -0.190065979957581
0.670000076293945 -0.191547513008118
0.680000066757202 -0.192843437194824
0.690000057220459 -0.193960428237915
0.700000047683716 -0.194905877113342
0.720000028610229 -0.196313381195068
0.740000009536743 -0.197130799293518
0.759999990463257 -0.197426438331604
0.779999971389771 -0.197271704673767
0.799999952316284 -0.196738719940186
0.819999933242798 -0.195900678634644
0.850000023841858 -0.194230675697327
0.899999976158142 -0.190916538238525
0.940000057220459 -0.188318967819214
0.970000028610229 -0.18664562702179
1 -0.185332894325256
1.02999997138977 -0.184453010559082
1.05999994277954 -0.18403959274292
1.0900000333786 -0.184088230133057
1.12000000476837 -0.184556484222412
1.14999997615814 -0.185364127159119
1.21000003814697 -0.187472939491272
1.24000000953674 -0.188407897949219
1.25999999046326 -0.1888347864151
1.27999997138977 -0.18901801109314
1.29999995231628 -0.18887996673584
1.32000005245209 -0.188338756561279
1.3400000333786 -0.187308311462402
1.36000001430511 -0.185705065727234
1.37000000476837 -0.184664249420166
1.37999999523163 -0.183451414108276
1.38999998569489 -0.182057499885559
1.39999997615814 -0.180474042892456
1.4099999666214 -0.178692579269409
1.41999995708466 -0.176705479621887
1.42999994754791 -0.174505591392517
1.44000005722046 -0.172086358070374
1.45000004768372 -0.169441938400269
1.46000003814697 -0.166566610336304
1.47000002861023 -0.16345489025116
1.48000001907349 -0.160101532936096
1.49000000953674 -0.156501889228821
};
\addlegendentry{K1}
\addplot [ultra thick, color0]
table {%
0 0.226413011550903
0.00999999046325684 0.221606135368347
0.0199999809265137 0.21653139591217
0.0299999713897705 0.211194396018982
0.0399999618530273 0.205601215362549
0.0499999523162842 0.199758291244507
0.059999942779541 0.193673133850098
0.0700000524520874 0.187353134155273
0.0800000429153442 0.180806398391724
0.0900000333786011 0.174041748046875
0.100000023841858 0.167068362236023
0.120000004768372 0.152534604072571
0.139999985694885 0.137287974357605
0.159999966621399 0.121418833732605
0.180000066757202 0.105027198791504
0.200000047683716 0.0882190465927124
0.230000019073486 0.0624641180038452
0.299999952316284 0.00182628631591797
0.319999933242798 -0.0151265859603882
0.340000033378601 -0.0317097902297974
0.360000014305115 -0.0478192567825317
0.379999995231628 -0.0633635520935059
0.399999976158142 -0.0782591104507446
0.419999957084656 -0.0924277305603027
0.430000066757202 -0.0992168188095093
0.440000057220459 -0.105798602104187
0.450000047683716 -0.11216676235199
0.460000038146973 -0.118315577507019
0.470000028610229 -0.124240398406982
0.480000019073486 -0.129938125610352
0.490000009536743 -0.135404467582703
0.5 -0.140635132789612
0.509999990463257 -0.14562714099884
0.519999980926514 -0.150378465652466
0.529999971389771 -0.154887557029724
0.539999961853027 -0.159152984619141
0.549999952316284 -0.163173913955688
0.559999942779541 -0.166950583457947
0.569999933242798 -0.170484066009521
0.579999923706055 -0.173775553703308
0.589999914169312 -0.176827192306519
0.600000023841858 -0.179641962051392
0.610000014305115 -0.182223200798035
0.620000004768372 -0.184575080871582
0.629999995231628 -0.186702609062195
0.639999985694885 -0.188611030578613
0.649999976158142 -0.190306067466736
0.660000085830688 -0.191794395446777
0.670000076293945 -0.19308340549469
0.680000066757202 -0.194180727005005
0.690000057220459 -0.195094585418701
0.700000047683716 -0.195833444595337
0.720000028610229 -0.196822643280029
0.740000009536743 -0.197224974632263
0.759999990463257 -0.197118639945984
0.779999971389771 -0.196580410003662
0.799999952316284 -0.195687055587769
0.819999933242798 -0.194512367248535
0.850000023841858 -0.192375779151917
0.899999976158142 -0.188345432281494
0.940000057220459 -0.185179591178894
0.970000028610229 -0.183057904243469
1 -0.181265354156494
1.02999997138977 -0.179868698120117
1.05999994277954 -0.178903818130493
1.0900000333786 -0.178382158279419
1.12000000476837 -0.178287267684937
1.14999997615814 -0.178567171096802
1.19000005722046 -0.179365515708923
1.26999998092651 -0.181196331977844
1.29999995231628 -0.181409597396851
1.32000005245209 -0.18122410774231
1.3400000333786 -0.180680632591248
1.36000001430511 -0.179692268371582
1.37999999523163 -0.178171277046204
1.38999998569489 -0.177184224128723
1.39999997615814 -0.176032662391663
1.4099999666214 -0.174706339836121
1.41999995708466 -0.173195719718933
1.42999994754791 -0.171491384506226
1.44000005722046 -0.169584989547729
1.45000004768372 -0.167468428611755
1.46000003814697 -0.16513454914093
1.47000002861023 -0.16257643699646
1.48000001907349 -0.159788012504578
1.49000000953674 -0.156763195991516
};
\addlegendentry{K2}
