# Supplementary material for: Neural Networks with Physics-Informed Architectures and Constraints for Dynamical Systems Modeling
Source: arXiv:2109.06407 source file (2022-12-12)
Supplement: Supplementary file 9 [file phi_2_dot_dynamics_data.tex]

\addplot [ultra thick, green!50.1960784313725!black, dashed]
table {%
0 -0.375052809715271
0.0199999809265137 -0.35399341583252
0.0399999618530273 -0.334224462509155
0.059999942779541 -0.316332697868347
0.0700000524520874 -0.308269381523132
0.0800000429153442 -0.300885796546936
0.0900000333786011 -0.29424774646759
0.100000023841858 -0.288418173789978
0.110000014305115 -0.283456802368164
0.120000004768372 -0.279419541358948
0.129999995231628 -0.276358604431152
0.139999985694885 -0.274320960044861
0.149999976158142 -0.273349285125732
0.159999966621399 -0.273480415344238
0.169999957084656 -0.274746417999268
0.180000066757202 -0.277171015739441
0.190000057220459 -0.280774235725403
0.200000047683716 -0.285568475723267
0.210000038146973 -0.291559100151062
0.220000028610229 -0.298745393753052
0.230000019073486 -0.307118773460388
0.240000009536743 -0.316665053367615
0.25 -0.327363014221191
0.259999990463257 -0.339184641838074
0.269999980926514 -0.35209596157074
0.279999971389771 -0.366056680679321
0.289999961853027 -0.381022095680237
0.299999952316284 -0.396940469741821
0.309999942779541 -0.413755893707275
0.330000042915344 -0.44983434677124
0.350000023841858 -0.488729000091553
0.370000004768372 -0.529859304428101
0.399999976158142 -0.594385385513306
0.460000038146973 -0.725439786911011
0.480000019073486 -0.767227411270142
0.5 -0.806927680969238
0.519999980926514 -0.843864440917969
0.529999971389771 -0.86108922958374
0.539999961853027 -0.87737512588501
0.549999952316284 -0.892645597457886
0.559999942779541 -0.906818866729736
0.569999933242798 -0.919820547103882
0.579999923706055 -0.931578755378723
0.589999914169312 -0.94202184677124
0.600000023841858 -0.951083421707153
0.610000014305115 -0.958698153495789
0.620000004768372 -0.964807629585266
0.629999995231628 -0.969357848167419
0.639999985694885 -0.972296476364136
0.649999976158142 -0.97357964515686
0.660000085830688 -0.973169803619385
0.670000076293945 -0.971033573150635
0.680000066757202 -0.967144966125488
0.690000057220459 -0.961483359336853
0.700000047683716 -0.954036235809326
0.710000038146973 -0.944798707962036
0.720000028610229 -0.933772563934326
0.730000019073486 -0.920961380004883
0.740000009536743 -0.906385183334351
0.75 -0.890064120292664
0.759999990463257 -0.872025728225708
0.769999980926514 -0.852305054664612
0.779999971389771 -0.830939650535583
0.789999961853027 -0.807975053787231
0.799999952316284 -0.783461570739746
0.809999942779541 -0.757452011108398
0.819999933242798 -0.730002164840698
0.829999923706055 -0.701175212860107
0.850000023841858 -0.639637231826782
0.870000004768372 -0.573366403579712
0.889999985694885 -0.502910971641541
0.910000085830688 -0.428828954696655
0.930000066757202 -0.351680755615234
0.960000038146973 -0.23142421245575
0.990000009536743 -0.107361912727356
1.0900000333786 0.310541868209839
1.12000000476837 0.43026065826416
1.13999998569489 0.506898164749146
1.1599999666214 0.580328583717346
1.17999994754791 0.649967312812805
1.20000004768372 0.715232372283936
1.22000002861023 0.775550961494446
1.23000001907349 0.803682088851929
1.24000000953674 0.830371856689453
1.25 0.85555899143219
1.25999999046326 0.879183053970337
1.26999998092651 0.901188492774963
1.27999997138977 0.921524286270142
1.28999996185303 0.940145015716553
1.29999995231628 0.957009553909302
1.30999994277954 0.972084283828735
1.32000005245209 0.985340714454651
1.33000004291534 0.996757984161377
1.3400000333786 1.0063214302063
1.35000002384186 1.01402401924133
1.36000001430511 1.01987266540527
1.37000000476837 1.02386713027954
1.37999999523163 1.0260261297226
1.38999998569489 1.02637195587158
1.39999997615814 1.02493739128113
1.4099999666214 1.02175486087799
1.41999995708466 1.01687121391296
1.42999994754791 1.01033282279968
1.44000005722046 1.00219297409058
1.45000004768372 0.992514371871948
1.46000003814697 0.981356978416443
1.47000002861023 0.968791961669922
1.48000001907349 0.954890608787537
1.49000000953674 0.939724683761597
};
\addplot [ultra thick, red]
table {%
0 -0.375052809715271
0.0299999713897705 -0.34479296207428
0.0499999523162842 -0.325867176055908
0.0700000524520874 -0.30856192111969
0.0800000429153442 -0.300646305084229
0.0900000333786011 -0.293282032012939
0.100000023841858 -0.286518573760986
0.110000014305115 -0.28044605255127
0.120000004768372 -0.275131464004517
0.129999995231628 -0.27057421207428
0.139999985694885 -0.266843795776367
0.149999976158142 -0.263944029808044
0.159999966621399 -0.261911869049072
0.169999957084656 -0.260740756988525
0.180000066757202 -0.260581970214844
0.190000057220459 -0.261608242988586
0.200000047683716 -0.263932943344116
0.210000038146973 -0.267612457275391
0.220000028610229 -0.272644281387329
0.230000019073486 -0.279072165489197
0.240000009536743 -0.286825656890869
0.25 -0.29586136341095
0.259999990463257 -0.306235909461975
0.269999980926514 -0.317941546440125
0.279999971389771 -0.330834150314331
0.289999961853027 -0.344872117042542
0.299999952316284 -0.360018730163574
0.309999942779541 -0.376288890838623
0.319999933242798 -0.393571615219116
0.340000033378601 -0.430786609649658
0.360000014305115 -0.470796346664429
0.379999995231628 -0.513087749481201
0.409999966621399 -0.579582691192627
0.490000009536743 -0.760274410247803
0.509999990463257 -0.802544593811035
0.529999971389771 -0.842248201370239
0.539999961853027 -0.860876798629761
0.549999952316284 -0.878507494926453
0.559999942779541 -0.895048856735229
0.569999933242798 -0.910327196121216
0.579999923706055 -0.924288749694824
0.589999914169312 -0.936930894851685
0.600000023841858 -0.948229789733887
0.610000014305115 -0.958139657974243
0.620000004768372 -0.966625452041626
0.629999995231628 -0.97360360622406
0.639999985694885 -0.979060411453247
0.649999976158142 -0.983085989952087
0.660000085830688 -0.985669374465942
0.670000076293945 -0.98673677444458
0.680000066757202 -0.986242532730103
0.690000057220459 -0.984138607978821
0.700000047683716 -0.980235576629639
0.710000038146973 -0.974430084228516
0.720000028610229 -0.966770648956299
0.730000019073486 -0.957227349281311
0.740000009536743 -0.945815086364746
0.75 -0.932609558105469
0.759999990463257 -0.917635917663574
0.769999980926514 -0.900911092758179
0.779999971389771 -0.882425308227539
0.789999961853027 -0.862182140350342
0.799999952316284 -0.840234756469727
0.809999942779541 -0.816640377044678
0.819999933242798 -0.791443228721619
0.829999923706055 -0.764711260795593
0.839999914169312 -0.736555337905884
0.850000023841858 -0.707006692886353
0.870000004768372 -0.643865346908569
0.889999985694885 -0.575729608535767
0.910000085830688 -0.503252506256104
0.930000066757202 -0.427269220352173
0.950000047683716 -0.348373770713806
0.980000019073486 -0.225610256195068
1.00999999046326 -0.0990240573883057
1.11000001430511 0.327710628509521
1.13999998569489 0.450340986251831
1.1599999666214 0.529210329055786
1.17999994754791 0.605208396911621
1.20000004768372 0.677639484405518
1.22000002861023 0.745837688446045
1.24000000953674 0.809105634689331
1.25 0.838767528533936
1.25999999046326 0.867063999176025
1.26999998092651 0.893930792808533
1.27999997138977 0.919314622879028
1.28999996185303 0.943103671073914
1.29999995231628 0.965176939964294
1.30999994277954 0.985450744628906
1.32000005245209 1.00395512580872
1.33000004291534 1.02058684825897
1.3400000333786 1.03518092632294
1.35000002384186 1.04772818088531
1.36000001430511 1.05824744701385
1.37000000476837 1.06683325767517
1.37999999523163 1.073481798172
1.38999998569489 1.07815301418304
1.39999997615814 1.08098721504211
1.4099999666214 1.08187830448151
1.41999995708466 1.0807683467865
1.42999994754791 1.07772707939148
1.44000005722046 1.07285761833191
1.45000004768372 1.0662556886673
1.46000003814697 1.05798184871674
1.47000002861023 1.04802083969116
1.48000001907349 1.036465883255
1.49000000953674 1.02337205410004
};
\addplot [ultra thick, blue]
table {%
0 -0.375052809715271
0.0199999809265137 -0.354439616203308
0.0399999618530273 -0.335317254066467
0.0499999523162842 -0.326518654823303
0.059999942779541 -0.318325757980347
0.0700000524520874 -0.310792446136475
0.0800000429153442 -0.303995490074158
0.0900000333786011 -0.297987341880798
0.100000023841858 -0.292775273323059
0.110000014305115 -0.28840959072113
0.120000004768372 -0.284934759140015
0.129999995231628 -0.282394170761108
0.139999985694885 -0.280826330184937
0.149999976158142 -0.28026270866394
0.159999966621399 -0.280729413032532
0.169999957084656 -0.282263040542603
0.180000066757202 -0.284902334213257
0.190000057220459 -0.288683891296387
0.200000047683716 -0.293604731559753
0.210000038146973 -0.299673557281494
0.220000028610229 -0.306903600692749
0.230000019073486 -0.315272569656372
0.240000009536743 -0.324841260910034
0.25 -0.335751533508301
0.259999990463257 -0.348031997680664
0.269999980926514 -0.361712574958801
0.279999971389771 -0.37670111656189
0.299999952316284 -0.409523010253906
0.319999933242798 -0.444836497306824
0.340000033378601 -0.482085943222046
0.370000004768372 -0.540358304977417
0.389999985694885 -0.580827951431274
0.419999957084656 -0.643582582473755
0.470000028610229 -0.748948454856873
0.5 -0.809882879257202
0.519999980926514 -0.848361015319824
0.539999961853027 -0.88438355922699
0.549999952316284 -0.901211738586426
0.559999942779541 -0.91693913936615
0.569999933242798 -0.931445121765137
0.579999923706055 -0.944803357124329
0.589999914169312 -0.956969976425171
0.600000023841858 -0.967820525169373
0.610000014305115 -0.977311134338379
0.620000004768372 -0.985439300537109
0.629999995231628 -0.992175221443176
0.639999985694885 -0.997470855712891
0.649999976158142 -1.00127410888672
0.660000085830688 -1.00353848934174
0.670000076293945 -1.00421047210693
0.680000066757202 -1.00323903560638
0.690000057220459 -1.00056374073029
0.700000047683716 -0.996142625808716
0.710000038146973 -0.989949107170105
0.720000028610229 -0.981957197189331
0.730000019073486 -0.972152471542358
0.740000009536743 -0.960522413253784
0.75 -0.947054862976074
0.759999990463257 -0.931743860244751
0.769999980926514 -0.91459846496582
0.779999971389771 -0.895631790161133
0.789999961853027 -0.874860048294067
0.799999952316284 -0.852285861968994
0.809999942779541 -0.827928781509399
0.819999933242798 -0.801822423934937
0.829999923706055 -0.774008512496948
0.839999914169312 -0.744529366493225
0.850000023841858 -0.713431119918823
0.860000014305115 -0.680772542953491
0.879999995231628 -0.611066102981567
0.899999976158142 -0.53601598739624
0.920000076293945 -0.456254005432129
0.940000057220459 -0.372455358505249
0.960000038146973 -0.28530216217041
0.990000009536743 -0.149757981300354
1.02999997138977 0.0361281633377075
1.08000004291534 0.26858651638031
1.11000001430511 0.403778553009033
1.12999999523163 0.490597486495972
1.14999997615814 0.573909044265747
1.16999995708466 0.652990341186523
1.19000005722046 0.727120876312256
1.21000003814697 0.795507907867432
1.22000002861023 0.827368378639221
1.23000001907349 0.857600092887878
1.24000000953674 0.886144757270813
1.25 0.912933230400085
1.25999999046326 0.937911510467529
1.26999998092651 0.961040735244751
1.27999997138977 0.982285499572754
1.28999996185303 1.00160574913025
1.29999995231628 1.0189266204834
1.30999994277954 1.03419637680054
1.32000005245209 1.04739475250244
1.33000004291534 1.05853724479675
1.3400000333786 1.06764805316925
1.35000002384186 1.07475459575653
1.36000001430511 1.07989060878754
1.37000000476837 1.08308219909668
1.37999999523163 1.08435726165771
1.38999998569489 1.08373987674713
1.39999997615814 1.08127665519714
1.4099999666214 1.07704019546509
1.41999995708466 1.07109928131104
1.42999994754791 1.0635232925415
1.44000005722046 1.05437934398651
1.45000004768372 1.04370725154877
1.46000003814697 1.03148508071899
1.47000002861023 1.01768612861633
1.48000001907349 1.00236880779266
1.49000000953674 0.985586047172546
};
\addplot [ultra thick, color0]
table {%
0 -0.375052809715271
0.0199999809265137 -0.355425119400024
0.0399999618530273 -0.336840867996216
0.059999942779541 -0.319757342338562
0.0800000429153442 -0.304588794708252
0.0900000333786011 -0.297880053520203
0.100000023841858 -0.291837811470032
0.110000014305115 -0.28652012348175
0.120000004768372 -0.281968474388123
0.129999995231628 -0.278219938278198
0.139999985694885 -0.275350451469421
0.149999976158142 -0.273462414741516
0.159999966621399 -0.272584915161133
0.169999957084656 -0.272766351699829
0.180000066757202 -0.274045586585999
0.190000057220459 -0.276425719261169
0.200000047683716 -0.279907703399658
0.210000038146973 -0.284570932388306
0.220000028610229 -0.290427684783936
0.230000019073486 -0.297469973564148
0.240000009536743 -0.305666923522949
0.25 -0.315110445022583
0.259999990463257 -0.325777769088745
0.269999980926514 -0.337688446044922
0.279999971389771 -0.350744009017944
0.289999961853027 -0.364902019500732
0.299999952316284 -0.380129218101501
0.309999942779541 -0.396454095840454
0.319999933242798 -0.413812398910522
0.340000033378601 -0.451374053955078
0.360000014305115 -0.491986989974976
0.379999995231628 -0.534942388534546
0.399999976158142 -0.579834222793579
0.440000057220459 -0.672948837280273
0.460000038146973 -0.71928083896637
0.490000009536743 -0.785741806030273
0.509999990463257 -0.827916502952576
0.529999971389771 -0.867523908615112
0.549999952316284 -0.904052257537842
0.559999942779541 -0.920892953872681
0.569999933242798 -0.936716794967651
0.579999923706055 -0.951441168785095
0.589999914169312 -0.964968681335449
0.600000023841858 -0.977202653884888
0.610000014305115 -0.988062143325806
0.620000004768372 -0.997481465339661
0.629999995231628 -1.00540602207184
0.639999985694885 -1.01176905632019
0.649999976158142 -1.01650047302246
0.660000085830688 -1.01947629451752
0.670000076293945 -1.02064990997314
0.680000066757202 -1.02004015445709
0.690000057220459 -1.01760029792786
0.700000047683716 -1.01327621936798
0.710000038146973 -1.00703191757202
0.720000028610229 -0.998838663101196
0.730000019073486 -0.988676786422729
0.740000009536743 -0.976596593856812
0.75 -0.962610483169556
0.759999990463257 -0.94672703742981
0.769999980926514 -0.928970575332642
0.779999971389771 -0.909358620643616
0.789999961853027 -0.887919902801514
0.799999952316284 -0.864713668823242
0.809999942779541 -0.839781522750854
0.819999933242798 -0.813165903091431
0.829999923706055 -0.784915089607239
0.839999914169312 -0.755081415176392
0.850000023841858 -0.723716020584106
0.870000004768372 -0.656666159629822
0.889999985694885 -0.584355354309082
0.910000085830688 -0.507404923439026
0.930000066757202 -0.426422834396362
0.950000047683716 -0.342018842697144
0.980000019073486 -0.210339784622192
1.00999999046326 -0.0744529962539673
1.11000001430511 0.382781505584717
1.13999998569489 0.513292193412781
1.1599999666214 0.596461772918701
1.17999994754791 0.675846099853516
1.20000004768372 0.750841617584229
1.22000002861023 0.82090950012207
1.24000000953674 0.885424852371216
1.25 0.915406346321106
1.25999999046326 0.943779826164246
1.26999998092651 0.970473289489746
1.27999997138977 0.995416164398193
1.28999996185303 1.01854228973389
1.29999995231628 1.03975772857666
1.30999994277954 1.05897724628448
1.32000005245209 1.07615685462952
1.33000004291534 1.09125804901123
1.3400000333786 1.10424113273621
1.35000002384186 1.11508738994598
1.36000001430511 1.12378740310669
1.37000000476837 1.13032913208008
1.37999999523163 1.13474428653717
1.38999998569489 1.13707137107849
1.39999997615814 1.137286901474
1.4099999666214 1.13539743423462
1.41999995708466 1.13148009777069
1.42999994754791 1.1256285905838
1.44000005722046 1.11791825294495
1.45000004768372 1.10841405391693
1.46000003814697 1.09718346595764
1.47000002861023 1.08432006835938
1.48000001907349 1.06974589824677
1.49000000953674 1.05349922180176
};
