# Supplementary material for: Neural Networks with Physics-Informed Architectures and Constraints for Dynamical Systems Modeling
Source: arXiv:2109.06407 source file (2022-12-12)
Supplement: Supplementary file 10 [file phi_2_dynamics_data.tex]

\addplot [ultra thick, green!50.1960784313725!black, dashed]
table {%
0 0.1720130443573
0.0199999809265137 0.16467559337616
0.0399999618530273 0.157750248908997
0.059999942779541 0.151204943656921
0.0900000333786011 0.142001271247864
0.120000004768372 0.13335919380188
0.220000028610229 0.105218172073364
0.240000009536743 0.0990309715270996
0.259999990463257 0.0924361944198608
0.279999971389771 0.0853438377380371
0.299999952316284 0.0776693820953369
0.319999933242798 0.0693362951278687
0.340000033378601 0.0602772235870361
0.360000014305115 0.0504356622695923
0.379999995231628 0.0397665500640869
0.399999976158142 0.0282371044158936
0.419999957084656 0.0158283710479736
0.440000057220459 0.00253379344940186
0.460000038146973 -0.0116386413574219
0.480000019073486 -0.0266677141189575
0.5 -0.0425183773040771
0.519999980926514 -0.0591415166854858
0.539999961853027 -0.0764749050140381
0.559999942779541 -0.0944430828094482
0.579999923706055 -0.112958073616028
0.610000014305115 -0.141533374786377
0.649999976158142 -0.180522561073303
0.700000047683716 -0.229218721389771
0.720000028610229 -0.248234748840332
0.740000009536743 -0.266770958900452
0.759999990463257 -0.284685373306274
0.779999971389771 -0.301839113235474
0.799999952316284 -0.318100929260254
0.819999933242798 -0.333346486091614
0.829999923706055 -0.340551495552063
0.839999914169312 -0.347459435462952
0.850000023841858 -0.354057192802429
0.860000014305115 -0.360333204269409
0.870000004768372 -0.366275548934937
0.879999995231628 -0.371873378753662
0.889999985694885 -0.377116560935974
0.899999976158142 -0.381995558738708
0.910000085830688 -0.386501550674438
0.920000076293945 -0.390627145767212
0.930000066757202 -0.394363522529602
0.940000057220459 -0.397705316543579
0.950000047683716 -0.400645971298218
0.960000038146973 -0.403180360794067
0.970000028610229 -0.405303835868835
0.980000019073486 -0.407012462615967
0.990000009536743 -0.408303260803223
1 -0.409173369407654
1.00999999046326 -0.409621000289917
1.01999998092651 -0.409644842147827
1.02999997138977 -0.409244537353516
1.03999996185303 -0.408419847488403
1.04999995231628 -0.407171845436096
1.05999994277954 -0.405501842498779
1.07000005245209 -0.403411984443665
1.08000004291534 -0.400905013084412
1.0900000333786 -0.397984266281128
1.10000002384186 -0.394654154777527
1.11000001430511 -0.390919208526611
1.12000000476837 -0.386785745620728
1.12999999523163 -0.382259011268616
1.13999998569489 -0.377346158027649
1.14999997615814 -0.372056841850281
1.1599999666214 -0.366396188735962
1.16999995708466 -0.360375642776489
1.17999994754791 -0.354004383087158
1.19000005722046 -0.347293257713318
1.20000004768372 -0.340253591537476
1.21000003814697 -0.332897305488586
1.23000001907349 -0.317287445068359
1.25 -0.30057430267334
1.26999998092651 -0.282878994941711
1.28999996185303 -0.264331340789795
1.30999994277954 -0.24506950378418
1.33000004291534 -0.225237607955933
1.36000001430511 -0.194744348526001
1.44000005722046 -0.112576484680176
1.46000003814697 -0.0925986766815186
1.48000001907349 -0.0730980634689331
1.49000000953674 -0.0635608434677124
};
\addplot [ultra thick, red]
table {%
0 0.1720130443573
0.0199999809265137 0.164787292480469
0.0499999523162842 0.154523491859436
0.0800000429153442 0.144828796386719
0.110000014305115 0.135755896568298
0.190000057220459 0.112717151641846
0.220000028610229 0.10397732257843
0.25 0.0946859121322632
0.279999971389771 0.0847444534301758
0.299999952316284 0.077631950378418
0.319999933242798 0.0700103044509888
0.340000033378601 0.0618181228637695
0.360000014305115 0.0528779029846191
0.379999995231628 0.0430694818496704
0.399999976158142 0.032381534576416
0.419999957084656 0.020869255065918
0.440000057220459 0.00843179225921631
0.460000038146973 -0.0049128532409668
0.480000019073486 -0.0191214084625244
0.5 -0.034176230430603
0.519999980926514 -0.05002760887146
0.539999961853027 -0.0666161775588989
0.559999942779541 -0.0839835405349731
0.579999923706055 -0.102072358131409
0.610000014305115 -0.130043983459473
0.639999985694885 -0.158814430236816
0.680000066757202 -0.198253631591797
0.75 -0.267154812812805
0.769999980926514 -0.286407947540283
0.789999961853027 -0.305055618286133
0.809999942779541 -0.322777986526489
0.829999923706055 -0.339400053024292
0.839999914169312 -0.347267985343933
0.850000023841858 -0.354826688766479
0.860000014305115 -0.362074136734009
0.870000004768372 -0.368971586227417
0.879999995231628 -0.375504016876221
0.889999985694885 -0.381661534309387
0.899999976158142 -0.387444615364075
0.910000085830688 -0.392851710319519
0.920000076293945 -0.397881150245667
0.930000066757202 -0.402544021606445
0.940000057220459 -0.406829595565796
0.950000047683716 -0.410747766494751
0.960000038146973 -0.414315342903137
0.970000028610229 -0.417531609535217
0.980000019073486 -0.420383930206299
0.990000009536743 -0.422860622406006
1 -0.424949169158936
1.00999999046326 -0.426622033119202
1.01999998092651 -0.427864551544189
1.02999997138977 -0.428663015365601
1.03999996185303 -0.429016470909119
1.04999995231628 -0.428964734077454
1.05999994277954 -0.428489089012146
1.07000005245209 -0.427588105201721
1.08000004291534 -0.42623233795166
1.0900000333786 -0.424414277076721
1.10000002384186 -0.42213237285614
1.11000001430511 -0.419396042823792
1.12000000476837 -0.416221380233765
1.12999999523163 -0.412630438804626
1.13999998569489 -0.408641934394836
1.14999997615814 -0.404266595840454
1.1599999666214 -0.399503469467163
1.16999995708466 -0.39435613155365
1.17999994754791 -0.388819932937622
1.19000005722046 -0.382902383804321
1.20000004768372 -0.376608371734619
1.21000003814697 -0.369920969009399
1.22000002861023 -0.362843871116638
1.23000001907349 -0.35540759563446
1.24000000953674 -0.347633838653564
1.25 -0.339545249938965
1.26999998092651 -0.322505474090576
1.28999996185303 -0.304490566253662
1.30999994277954 -0.285367965698242
1.33000004291534 -0.265298843383789
1.35000002384186 -0.244558930397034
1.37999999523163 -0.212616205215454
1.45000004768372 -0.137471556663513
1.48000001907349 -0.105811476707458
1.49000000953674 -0.0954482555389404
};
\addplot [ultra thick, blue]
table {%
0 0.1720130443573
0.0199999809265137 0.164616465568542
0.0399999618530273 0.157625555992126
0.059999942779541 0.151007175445557
0.0900000333786011 0.141676068305969
0.120000004768372 0.13288426399231
0.220000028610229 0.104301571846008
0.240000009536743 0.0980798006057739
0.259999990463257 0.0914738178253174
0.279999971389771 0.0843764543533325
0.299999952316284 0.0766818523406982
0.319999933242798 0.0683176517486572
0.340000033378601 0.0592365264892578
0.360000014305115 0.0494033098220825
0.379999995231628 0.0387929677963257
0.399999976158142 0.0273805856704712
0.419999957084656 0.0151405334472656
0.440000057220459 0.00205683708190918
0.460000038146973 -0.0118739604949951
0.480000019073486 -0.0266444683074951
0.5 -0.0422395467758179
0.519999980926514 -0.0586323738098145
0.539999961853027 -0.0757832527160645
0.559999942779541 -0.0936392545700073
0.579999923706055 -0.112123131752014
0.600000023841858 -0.131140828132629
0.629999995231628 -0.160446524620056
0.670000076293945 -0.200391054153442
0.720000028610229 -0.250332117080688
0.75 -0.279478430747986
0.769999980926514 -0.298266410827637
0.789999961853027 -0.316368699073792
0.809999942779541 -0.333640217781067
0.829999923706055 -0.349937677383423
0.839999914169312 -0.357677817344666
0.850000023841858 -0.36512303352356
0.860000014305115 -0.372257471084595
0.870000004768372 -0.379065155982971
0.879999995231628 -0.385531425476074
0.889999985694885 -0.391642093658447
0.899999976158142 -0.397383689880371
0.910000085830688 -0.402743935585022
0.920000076293945 -0.407710790634155
0.930000066757202 -0.412273287773132
0.940000057220459 -0.416421413421631
0.950000047683716 -0.420145988464355
0.960000038146973 -0.423438549041748
0.970000028610229 -0.426291584968567
0.980000019073486 -0.428698301315308
0.990000009536743 -0.430652856826782
1 -0.432150363922119
1.00999999046326 -0.433187007904053
1.01999998092651 -0.433759450912476
1.02999997138977 -0.433865785598755
1.03999996185303 -0.433504462242126
1.04999995231628 -0.432675361633301
1.05999994277954 -0.431378841400146
1.07000005245209 -0.429616570472717
1.08000004291534 -0.427390813827515
1.0900000333786 -0.424704909324646
1.10000002384186 -0.421563148498535
1.11000001430511 -0.417970418930054
1.12000000476837 -0.41393256187439
1.12999999523163 -0.409456729888916
1.13999998569489 -0.404550790786743
1.14999997615814 -0.399223446846008
1.1599999666214 -0.393484354019165
1.16999995708466 -0.387344121932983
1.17999994754791 -0.38081419467926
1.19000005722046 -0.373906970024109
1.20000004768372 -0.366635799407959
1.21000003814697 -0.359014987945557
1.22000002861023 -0.351059913635254
1.23000001907349 -0.342786312103271
1.25 -0.325348854064941
1.26999998092651 -0.306840419769287
1.28999996185303 -0.287407159805298
1.30999994277954 -0.267201781272888
1.33000004291534 -0.246385812759399
1.36000001430511 -0.214376449584961
1.44000005722046 -0.128136396408081
1.47000002861023 -0.0968406200408936
1.49000000953674 -0.0766401290893555
};
\addplot [ultra thick, color0]
table {%
0 0.1720130443573
0.0199999809265137 0.164611101150513
0.0399999618530273 0.157597064971924
0.059999942779541 0.15094780921936
0.0900000333786011 0.141585350036621
0.120000004768372 0.13282299041748
0.159999966621399 0.121732950210571
0.210000038146973 0.107975602149963
0.240000009536743 0.0992509126663208
0.259999990463257 0.0930432081222534
0.279999971389771 0.0864084959030151
0.299999952316284 0.0792520046234131
0.319999933242798 0.071486234664917
0.340000033378601 0.0630265474319458
0.360000014305115 0.0537991523742676
0.379999995231628 0.0437474250793457
0.399999976158142 0.0328261852264404
0.419999957084656 0.0209991931915283
0.440000057220459 0.00824284553527832
0.460000038146973 -0.00544953346252441
0.480000019073486 -0.0200598239898682
0.5 -0.0355559587478638
0.519999980926514 -0.0519064664840698
0.539999961853027 -0.0690622329711914
0.559999942779541 -0.0869650840759277
0.579999923706055 -0.105541110038757
0.600000023841858 -0.12470531463623
0.629999995231628 -0.154332756996155
0.670000076293945 -0.194864273071289
0.720000028610229 -0.245650291442871
0.75 -0.275291323661804
0.769999980926514 -0.294384717941284
0.789999961853027 -0.31276798248291
0.809999942779541 -0.330294370651245
0.829999923706055 -0.346823811531067
0.839999914169312 -0.354672908782959
0.850000023841858 -0.362223744392395
0.860000014305115 -0.369460940361023
0.870000004768372 -0.376369833946228
0.879999995231628 -0.382936477661133
0.889999985694885 -0.389147758483887
0.899999976158142 -0.394991278648376
0.910000085830688 -0.400455474853516
0.920000076293945 -0.405529618263245
0.930000066757202 -0.410203456878662
0.940000057220459 -0.414467573165894
0.950000047683716 -0.41831374168396
0.960000038146973 -0.421733856201172
0.970000028610229 -0.424721121788025
0.980000019073486 -0.427269220352173
0.990000009536743 -0.429372549057007
1 -0.431026697158813
1.00999999046326 -0.432227492332458
1.01999998092651 -0.432971954345703
1.02999997138977 -0.433257937431335
1.03999996185303 -0.433083772659302
1.04999995231628 -0.432448506355286
1.05999994277954 -0.431352019309998
1.07000005245209 -0.429794549942017
1.08000004291534 -0.427777528762817
1.0900000333786 -0.425302624702454
1.10000002384186 -0.422372817993164
1.11000001430511 -0.418991684913635
1.12000000476837 -0.41516387462616
1.12999999523163 -0.410894632339478
1.13999998569489 -0.406190037727356
1.14999997615814 -0.401057124137878
1.1599999666214 -0.395503878593445
1.16999995708466 -0.389539241790771
1.17999994754791 -0.383172631263733
1.19000005722046 -0.376414179801941
1.20000004768372 -0.369274973869324
1.21000003814697 -0.361766576766968
1.22000002861023 -0.353901267051697
1.23000001907349 -0.345692157745361
1.24000000953674 -0.337153077125549
1.25999999046326 -0.31914484500885
1.27999997138977 -0.300002336502075
1.29999995231628 -0.279862642288208
1.32000005245209 -0.258875370025635
1.3400000333786 -0.23720121383667
1.37000000476837 -0.203770041465759
1.46000003814697 -0.102187395095825
1.48000001907349 -0.0803723335266113
1.49000000953674 -0.0696748495101929
};
