# Supplementary material for: Neural Networks with Physics-Informed Architectures and Constraints for Dynamical Systems Modeling
Source: arXiv:2109.06407 source file (2022-12-12)
Supplement: Supplementary file 11 [file constraint_loss_data.tex]

\path [fill=color0, fill opacity=0.4, ultra thick]
(axis cs:0,237.925003051758)
--(axis cs:0,211.867477416992)
--(axis cs:100,261.10009765625)
--(axis cs:200,262.886291503906)
--(axis cs:300,264.170318603516)
--(axis cs:400,250.576416015625)
--(axis cs:500,42.0327339172363)
--(axis cs:600,8.49201679229736)
--(axis cs:700,6.70053720474243)
--(axis cs:800,5.01216506958008)
--(axis cs:900,5.6209602355957)
--(axis cs:1000,1.58914947509766)
--(axis cs:1100,2.20554208755493)
--(axis cs:1200,7.27553176879883)
--(axis cs:1300,18.8865242004395)
--(axis cs:1400,24.5383987426758)
--(axis cs:1500,25.6514453887939)
--(axis cs:1600,27.448802947998)
--(axis cs:1700,27.9536628723145)
--(axis cs:1800,36.5069351196289)
--(axis cs:1900,40.7017097473145)
--(axis cs:2000,51.571533203125)
--(axis cs:2100,57.1563720703125)
--(axis cs:2200,55.919921875)
--(axis cs:2300,49.2231636047363)
--(axis cs:2400,50.0492973327637)
--(axis cs:2500,49.9380569458008)
--(axis cs:2600,74.3858108520508)
--(axis cs:2700,95.0464477539062)
--(axis cs:2800,120.612426757812)
--(axis cs:2900,142.361602783203)
--(axis cs:3000,153.484115600586)
--(axis cs:3100,128.602340698242)
--(axis cs:3200,127.2255859375)
--(axis cs:3300,116.761131286621)
--(axis cs:3400,114.569725036621)
--(axis cs:3500,139.926849365234)
--(axis cs:3600,139.1123046875)
--(axis cs:3700,152.905471801758)
--(axis cs:3800,173.743255615234)
--(axis cs:3900,173.795211791992)
--(axis cs:4000,196.888641357422)
--(axis cs:4100,200.711715698242)
--(axis cs:4200,209.338851928711)
--(axis cs:4300,192.587890625)
--(axis cs:4400,196.642456054688)
--(axis cs:4500,201.365905761719)
--(axis cs:4600,235.114715576172)
--(axis cs:4700,267.549224853516)
--(axis cs:4800,287.324890136719)
--(axis cs:4900,305.640167236328)
--(axis cs:5000,286.992828369141)
--(axis cs:5100,279.767883300781)
--(axis cs:5200,266.716400146484)
--(axis cs:5300,279.102081298828)
--(axis cs:5400,269.178314208984)
--(axis cs:5500,268.493011474609)
--(axis cs:5600,296.209136962891)
--(axis cs:5700,270.897277832031)
--(axis cs:5800,253.700988769531)
--(axis cs:5900,245.279434204102)
--(axis cs:6000,244.083770751953)
--(axis cs:6100,250.990478515625)
--(axis cs:6200,267.476318359375)
--(axis cs:6300,289.775970458984)
--(axis cs:6400,320.691009521484)
--(axis cs:6500,367.428771972656)
--(axis cs:6600,371.674072265625)
--(axis cs:6700,380.967041015625)
--(axis cs:6800,390.760345458984)
--(axis cs:6900,384.492889404297)
--(axis cs:7000,377.940002441406)
--(axis cs:7100,380.7158203125)
--(axis cs:7200,357.402374267578)
--(axis cs:7300,348.420562744141)
--(axis cs:7400,338.81591796875)
--(axis cs:7500,347.926788330078)
--(axis cs:7600,349.229766845703)
--(axis cs:7700,351.05419921875)
--(axis cs:7800,373.931243896484)
--(axis cs:7900,339.962554931641)
--(axis cs:8000,301.172424316406)
--(axis cs:8100,286.989044189453)
--(axis cs:8200,266.140869140625)
--(axis cs:8300,249.476959228516)
--(axis cs:8400,241.918914794922)
--(axis cs:8500,243.216400146484)
--(axis cs:8600,227.677200317383)
--(axis cs:8700,240.705856323242)
--(axis cs:8800,232.158203125)
--(axis cs:8900,250.845336914062)
--(axis cs:9000,251.595260620117)
--(axis cs:9100,252.255874633789)
--(axis cs:9200,254.892929077148)
--(axis cs:9300,248.598831176758)
--(axis cs:9400,265.6015625)
--(axis cs:9500,259.362609863281)
--(axis cs:9600,263.972106933594)
--(axis cs:9700,269.340667724609)
--(axis cs:9800,267.110595703125)
--(axis cs:9900,252.569519042969)
--(axis cs:10000,242.525619506836)
--(axis cs:10100,248.816482543945)
--(axis cs:10200,258.380310058594)
--(axis cs:10300,268.520355224609)
--(axis cs:10400,267.990142822266)
--(axis cs:10500,292.061828613281)
--(axis cs:10600,287.885040283203)
--(axis cs:10700,305.611541748047)
--(axis cs:10800,332.221557617188)
--(axis cs:10900,331.977416992188)
--(axis cs:11000,333.077209472656)
--(axis cs:11100,325.018371582031)
--(axis cs:11200,297.157897949219)
--(axis cs:11300,289.728485107422)
--(axis cs:11400,294.464263916016)
--(axis cs:11500,311.208190917969)
--(axis cs:11600,338.119537353516)
--(axis cs:11700,329.016662597656)
--(axis cs:11800,321.089263916016)
--(axis cs:11900,310.486999511719)
--(axis cs:12000,289.543518066406)
--(axis cs:12100,245.758865356445)
--(axis cs:12200,233.767761230469)
--(axis cs:12300,224.598876953125)
--(axis cs:12400,226.233612060547)
--(axis cs:12500,220.864166259766)
--(axis cs:12600,227.955490112305)
--(axis cs:12700,238.660308837891)
--(axis cs:12800,242.254653930664)
--(axis cs:12900,243.898971557617)
--(axis cs:13000,239.410293579102)
--(axis cs:13100,234.766128540039)
--(axis cs:13200,228.69921875)
--(axis cs:13300,246.186050415039)
--(axis cs:13400,242.430404663086)
--(axis cs:13500,250.6484375)
--(axis cs:13600,245.861877441406)
--(axis cs:13700,227.515487670898)
--(axis cs:13800,235.252349853516)
--(axis cs:13900,228.483596801758)
--(axis cs:14000,228.192962646484)
--(axis cs:14100,246.778121948242)
--(axis cs:14200,247.583587646484)
--(axis cs:14300,268.993743896484)
--(axis cs:14400,269.806060791016)
--(axis cs:14500,263.996887207031)
--(axis cs:14600,232.641876220703)
--(axis cs:14700,211.809677124023)
--(axis cs:14800,210.583709716797)
--(axis cs:14900,215.782806396484)
--(axis cs:15000,208.26513671875)
--(axis cs:15100,202.674713134766)
--(axis cs:15200,223.060623168945)
--(axis cs:15300,234.86003112793)
--(axis cs:15400,252.891403198242)
--(axis cs:15500,252.021881103516)
--(axis cs:15600,252.737503051758)
--(axis cs:15700,243.077346801758)
--(axis cs:15800,240.858596801758)
--(axis cs:15900,240.606262207031)
--(axis cs:16000,253.314056396484)
--(axis cs:16100,247.667190551758)
--(axis cs:16200,245.511352539062)
--(axis cs:16300,239.692123413086)
--(axis cs:16400,239.402252197266)
--(axis cs:16500,268.3828125)
--(axis cs:16600,259.651550292969)
--(axis cs:16700,261.959381103516)
--(axis cs:16800,289.94921875)
--(axis cs:16900,310.45654296875)
--(axis cs:17000,297.407806396484)
--(axis cs:17100,309.493011474609)
--(axis cs:17200,296.561706542969)
--(axis cs:17300,286.059387207031)
--(axis cs:17400,271.989837646484)
--(axis cs:17500,257.9140625)
--(axis cs:17600,246.754531860352)
--(axis cs:17700,246.188720703125)
--(axis cs:17800,236.026473999023)
--(axis cs:17900,227.731918334961)
--(axis cs:18000,216.261016845703)
--(axis cs:18100,204.853118896484)
--(axis cs:18200,215.9599609375)
--(axis cs:18300,231.124389648438)
--(axis cs:18400,232.56591796875)
--(axis cs:18500,261.956451416016)
--(axis cs:18600,285.498809814453)
--(axis cs:18700,305.319702148438)
--(axis cs:18800,303.158935546875)
--(axis cs:18900,285.684265136719)
--(axis cs:19000,255.546615600586)
--(axis cs:19100,246.903244018555)
--(axis cs:19200,252.369934082031)
--(axis cs:19300,282.061706542969)
--(axis cs:19400,286.267913818359)
--(axis cs:19500,286.360931396484)
--(axis cs:19600,271.086700439453)
--(axis cs:19700,238.127166748047)
--(axis cs:19800,203.004486083984)
--(axis cs:19900,194.085052490234)
--(axis cs:20000,206.0341796875)
--(axis cs:20100,211.15234375)
--(axis cs:20200,221.022659301758)
--(axis cs:20300,225.532028198242)
--(axis cs:20400,230.149993896484)
--(axis cs:20500,213.61328125)
--(axis cs:20600,216.249435424805)
--(axis cs:20700,207.887634277344)
--(axis cs:20800,210.308471679688)
--(axis cs:20900,209.821426391602)
--(axis cs:21000,222.740509033203)
--(axis cs:21100,237.649780273438)
--(axis cs:21200,254.386932373047)
--(axis cs:21300,258.989898681641)
--(axis cs:21400,255.463623046875)
--(axis cs:21500,239.509536743164)
--(axis cs:21600,235.169494628906)
--(axis cs:21700,237.678115844727)
--(axis cs:21800,246.940628051758)
--(axis cs:21900,243.8486328125)
--(axis cs:22000,259.929412841797)
--(axis cs:22100,274.756469726562)
--(axis cs:22200,265.448913574219)
--(axis cs:22300,250.444488525391)
--(axis cs:22400,251.248199462891)
--(axis cs:22500,250.243957519531)
--(axis cs:22600,237.177780151367)
--(axis cs:22700,247.9453125)
--(axis cs:22800,252.951370239258)
--(axis cs:22900,260.182800292969)
--(axis cs:23000,258.938201904297)
--(axis cs:23100,257.724700927734)
--(axis cs:23200,263.081573486328)
--(axis cs:23300,266.703857421875)
--(axis cs:23400,263.668273925781)
--(axis cs:23500,261.455932617188)
--(axis cs:23600,284.378601074219)
--(axis cs:23700,285.6875)
--(axis cs:23800,285.6875)
--(axis cs:23900,285.6875)
--(axis cs:24000,285.6875)
--(axis cs:24100,285.6875)
--(axis cs:24200,285.932098388672)
--(axis cs:24300,285.873718261719)
--(axis cs:24400,285.6875)
--(axis cs:24500,285.769714355469)
--(axis cs:24600,285.6875)
--(axis cs:24700,285.6875)
--(axis cs:24800,285.6875)
--(axis cs:24900,285.6875)
--(axis cs:25000,285.6875)
--(axis cs:25100,285.6875)
--(axis cs:25200,285.6875)
--(axis cs:25300,285.6875)
--(axis cs:25400,285.6875)
--(axis cs:25500,285.6875)
--(axis cs:25600,285.6875)
--(axis cs:25700,285.6875)
--(axis cs:25800,285.6875)
--(axis cs:25900,285.6875)
--(axis cs:26000,285.6875)
--(axis cs:26100,285.6875)
--(axis cs:26200,285.6875)
--(axis cs:26300,285.6875)
--(axis cs:26400,285.6875)
--(axis cs:26500,285.6875)
--(axis cs:26600,285.6875)
--(axis cs:26700,285.6875)
--(axis cs:26800,274.797149658203)
--(axis cs:26900,269.342041015625)
--(axis cs:27000,268.369934082031)
--(axis cs:27100,272.777191162109)
--(axis cs:27200,285.6875)
--(axis cs:27300,285.6875)
--(axis cs:27400,285.6875)
--(axis cs:27500,285.6875)
--(axis cs:27600,285.6875)
--(axis cs:27700,285.6875)
--(axis cs:27800,285.6875)
--(axis cs:27900,285.6875)
--(axis cs:28000,285.6875)
--(axis cs:28100,285.6875)
--(axis cs:28200,285.6875)
--(axis cs:28300,285.6875)
--(axis cs:28400,285.6875)
--(axis cs:28500,285.6875)
--(axis cs:28600,285.6875)
--(axis cs:28700,285.6875)
--(axis cs:28800,285.6875)
--(axis cs:28900,285.6875)
--(axis cs:29000,285.6875)
--(axis cs:29100,285.6875)
--(axis cs:29200,285.6875)
--(axis cs:29300,285.6875)
--(axis cs:29400,285.6875)
--(axis cs:29500,285.6875)
--(axis cs:29600,285.6875)
--(axis cs:29700,285.6875)
--(axis cs:29800,285.6875)
--(axis cs:29900,285.6875)
--(axis cs:30000,285.6875)
--(axis cs:30100,285.6875)
--(axis cs:30200,285.6875)
--(axis cs:30300,285.6875)
--(axis cs:30400,285.6875)
--(axis cs:30500,285.6875)
--(axis cs:30600,285.6875)
--(axis cs:30700,285.6875)
--(axis cs:30800,285.6875)
--(axis cs:30900,285.6875)
--(axis cs:31000,285.6875)
--(axis cs:31100,285.6875)
--(axis cs:31200,285.6875)
--(axis cs:31300,285.6875)
--(axis cs:31400,285.6875)
--(axis cs:31500,285.6875)
--(axis cs:31600,285.6875)
--(axis cs:31700,285.6875)
--(axis cs:31800,285.6875)
--(axis cs:31900,285.6875)
--(axis cs:32000,285.6875)
--(axis cs:32100,285.6875)
--(axis cs:32200,285.6875)
--(axis cs:32300,285.6875)
--(axis cs:32400,285.6875)
--(axis cs:32500,285.6875)
--(axis cs:32600,285.6875)
--(axis cs:32700,285.6875)
--(axis cs:32800,285.6875)
--(axis cs:32900,285.6875)
--(axis cs:33000,285.6875)
--(axis cs:33100,285.6875)
--(axis cs:33200,285.6875)
--(axis cs:33300,285.6875)
--(axis cs:33400,285.6875)
--(axis cs:33500,285.6875)
--(axis cs:33600,285.6875)
--(axis cs:33700,285.6875)
--(axis cs:33800,285.6875)
--(axis cs:33900,285.6875)
--(axis cs:34000,285.6875)
--(axis cs:34100,285.6875)
--(axis cs:34200,285.6875)
--(axis cs:34300,285.6875)
--(axis cs:34300,423.303894042969)
--(axis cs:34300,423.303894042969)
--(axis cs:34200,426.1103515625)
--(axis cs:34100,447.194183349609)
--(axis cs:34000,454.480743408203)
--(axis cs:33900,453.176849365234)
--(axis cs:33800,449.891296386719)
--(axis cs:33700,440.137725830078)
--(axis cs:33600,417.440765380859)
--(axis cs:33500,400.848449707031)
--(axis cs:33400,403.414764404297)
--(axis cs:33300,397.858459472656)
--(axis cs:33200,402.381195068359)
--(axis cs:33100,395.231811523438)
--(axis cs:33000,418.085815429688)
--(axis cs:32900,426.741577148438)
--(axis cs:32800,443.639556884766)
--(axis cs:32700,447.576416015625)
--(axis cs:32600,451.904357910156)
--(axis cs:32500,428.763458251953)
--(axis cs:32400,411.598968505859)
--(axis cs:32300,385.782745361328)
--(axis cs:32200,380.465362548828)
--(axis cs:32100,372.159301757812)
--(axis cs:32000,376.937255859375)
--(axis cs:31900,390.487762451172)
--(axis cs:31800,393.432495117188)
--(axis cs:31700,393.844909667969)
--(axis cs:31600,406.589630126953)
--(axis cs:31500,415.806213378906)
--(axis cs:31400,407.352844238281)
--(axis cs:31300,409.271606445312)
--(axis cs:31200,400.725250244141)
--(axis cs:31100,378.241119384766)
--(axis cs:31000,362.846252441406)
--(axis cs:30900,374.049133300781)
--(axis cs:30800,385.992706298828)
--(axis cs:30700,388.165405273438)
--(axis cs:30600,407.340270996094)
--(axis cs:30500,405.955902099609)
--(axis cs:30400,420.927459716797)
--(axis cs:30300,420.116455078125)
--(axis cs:30200,421.469421386719)
--(axis cs:30100,405.439147949219)
--(axis cs:30000,395.42041015625)
--(axis cs:29900,360.395690917969)
--(axis cs:29800,341.53125)
--(axis cs:29700,336.831695556641)
--(axis cs:29600,324.767852783203)
--(axis cs:29500,317.884307861328)
--(axis cs:29400,314.407745361328)
--(axis cs:29300,314.092254638672)
--(axis cs:29200,308.791564941406)
--(axis cs:29100,325.811248779297)
--(axis cs:29000,349.921081542969)
--(axis cs:28900,380.364807128906)
--(axis cs:28800,384.231170654297)
--(axis cs:28700,400.120452880859)
--(axis cs:28600,421.600158691406)
--(axis cs:28500,426.593231201172)
--(axis cs:28400,399.029052734375)
--(axis cs:28300,403.903839111328)
--(axis cs:28200,394.860870361328)
--(axis cs:28100,372.686157226562)
--(axis cs:28000,346.086364746094)
--(axis cs:27900,344.776275634766)
--(axis cs:27800,346.005859375)
--(axis cs:27700,341.035919189453)
--(axis cs:27600,344.290985107422)
--(axis cs:27500,336.118835449219)
--(axis cs:27400,329.934692382812)
--(axis cs:27300,313.548065185547)
--(axis cs:27200,300.628784179688)
--(axis cs:27100,287.2578125)
--(axis cs:27000,287.2578125)
--(axis cs:26900,287.2578125)
--(axis cs:26800,287.2578125)
--(axis cs:26700,295.732971191406)
--(axis cs:26600,321.601257324219)
--(axis cs:26500,340.592132568359)
--(axis cs:26400,338.689880371094)
--(axis cs:26300,340.038909912109)
--(axis cs:26200,335.466339111328)
--(axis cs:26100,315.330261230469)
--(axis cs:26000,302.696563720703)
--(axis cs:25900,306.469696044922)
--(axis cs:25800,309.546752929688)
--(axis cs:25700,310.959197998047)
--(axis cs:25600,325.657867431641)
--(axis cs:25500,342.846374511719)
--(axis cs:25400,345.069213867188)
--(axis cs:25300,349.711120605469)
--(axis cs:25200,347.238037109375)
--(axis cs:25100,361.294708251953)
--(axis cs:25000,358.025665283203)
--(axis cs:24900,343.165710449219)
--(axis cs:24800,328.155792236328)
--(axis cs:24700,321.509490966797)
--(axis cs:24600,300.238403320312)
--(axis cs:24500,290.101135253906)
--(axis cs:24400,298.841796875)
--(axis cs:24300,289.376831054688)
--(axis cs:24200,288.927276611328)
--(axis cs:24100,292.501098632812)
--(axis cs:24000,307.531951904297)
--(axis cs:23900,300.203918457031)
--(axis cs:23800,302.109527587891)
--(axis cs:23700,298.977294921875)
--(axis cs:23600,286.972961425781)
--(axis cs:23500,287.259368896484)
--(axis cs:23400,287.260162353516)
--(axis cs:23300,287.260925292969)
--(axis cs:23200,287.26171875)
--(axis cs:23100,287.26171875)
--(axis cs:23000,284.798797607422)
--(axis cs:22900,282.794311523438)
--(axis cs:22800,285.949157714844)
--(axis cs:22700,287.26171875)
--(axis cs:22600,302.432037353516)
--(axis cs:22500,314.482055664062)
--(axis cs:22400,321.604400634766)
--(axis cs:22300,325.252960205078)
--(axis cs:22200,319.682037353516)
--(axis cs:22100,334.602355957031)
--(axis cs:22000,332.938323974609)
--(axis cs:21900,316.407043457031)
--(axis cs:21800,312.165740966797)
--(axis cs:21700,287.209899902344)
--(axis cs:21600,265.375)
--(axis cs:21500,275.420166015625)
--(axis cs:21400,273.435150146484)
--(axis cs:21300,266.299163818359)
--(axis cs:21200,281.853912353516)
--(axis cs:21100,287.825775146484)
--(axis cs:21000,297.366394042969)
--(axis cs:20900,306.028900146484)
--(axis cs:20800,301.384368896484)
--(axis cs:20700,287.578918457031)
--(axis cs:20600,293.21826171875)
--(axis cs:20500,279.391326904297)
--(axis cs:20400,273.23193359375)
--(axis cs:20300,271.995758056641)
--(axis cs:20200,279.98583984375)
--(axis cs:20100,282.037780761719)
--(axis cs:20000,290.362152099609)
--(axis cs:19900,297.908142089844)
--(axis cs:19800,321.540863037109)
--(axis cs:19700,312.855682373047)
--(axis cs:19600,322.525299072266)
--(axis cs:19500,329.427642822266)
--(axis cs:19400,330.453460693359)
--(axis cs:19300,318.516967773438)
--(axis cs:19200,322.565490722656)
--(axis cs:19100,326.964996337891)
--(axis cs:19000,319.727355957031)
--(axis cs:18900,338.8359375)
--(axis cs:18800,321.98583984375)
--(axis cs:18700,324.135162353516)
--(axis cs:18600,319.84765625)
--(axis cs:18500,322.227355957031)
--(axis cs:18400,328.284118652344)
--(axis cs:18300,307.211547851562)
--(axis cs:18200,295.89892578125)
--(axis cs:18100,297.737945556641)
--(axis cs:18000,299.992645263672)
--(axis cs:17900,294.327453613281)
--(axis cs:17800,304.335021972656)
--(axis cs:17700,331.684753417969)
--(axis cs:17600,349.946472167969)
--(axis cs:17500,333.514007568359)
--(axis cs:17400,323.348358154297)
--(axis cs:17300,332.954315185547)
--(axis cs:17200,331.974945068359)
--(axis cs:17100,318.535125732422)
--(axis cs:17000,317.773529052734)
--(axis cs:16900,332.32421875)
--(axis cs:16800,346.114471435547)
--(axis cs:16700,351.121490478516)
--(axis cs:16600,338.334228515625)
--(axis cs:16500,336.270812988281)
--(axis cs:16400,320.193572998047)
--(axis cs:16300,299.598480224609)
--(axis cs:16200,298.365783691406)
--(axis cs:16100,300.647644042969)
--(axis cs:16000,287.111328125)
--(axis cs:15900,279.617980957031)
--(axis cs:15800,289.385467529297)
--(axis cs:15700,282.564117431641)
--(axis cs:15600,302.230926513672)
--(axis cs:15500,310.106811523438)
--(axis cs:15400,305.464324951172)
--(axis cs:15300,290.171722412109)
--(axis cs:15200,276.847198486328)
--(axis cs:15100,255.845306396484)
--(axis cs:15000,243.896331787109)
--(axis cs:14900,261.492706298828)
--(axis cs:14800,295.735534667969)
--(axis cs:14700,320.909606933594)
--(axis cs:14600,326.273223876953)
--(axis cs:14500,316.463134765625)
--(axis cs:14400,302.500762939453)
--(axis cs:14300,306.286071777344)
--(axis cs:14200,333.935791015625)
--(axis cs:14100,340.712005615234)
--(axis cs:14000,336.438293457031)
--(axis cs:13900,331.115356445312)
--(axis cs:13800,321.774047851562)
--(axis cs:13700,313.203247070312)
--(axis cs:13600,295.786560058594)
--(axis cs:13500,273.373565673828)
--(axis cs:13400,265.134704589844)
--(axis cs:13300,249.544525146484)
--(axis cs:13200,255.209487915039)
--(axis cs:13100,259.443237304688)
--(axis cs:13000,270.556243896484)
--(axis cs:12900,293.8828125)
--(axis cs:12800,299.880859375)
--(axis cs:12700,326.412506103516)
--(axis cs:12600,318.673828125)
--(axis cs:12500,324.419525146484)
--(axis cs:12400,321.278900146484)
--(axis cs:12300,338.112884521484)
--(axis cs:12200,322.028076171875)
--(axis cs:12100,339.405975341797)
--(axis cs:12000,333.503356933594)
--(axis cs:11900,355.829895019531)
--(axis cs:11800,355.744140625)
--(axis cs:11700,380.437744140625)
--(axis cs:11600,361.261627197266)
--(axis cs:11500,358.161529541016)
--(axis cs:11400,350.674835205078)
--(axis cs:11300,356.474395751953)
--(axis cs:11200,348.189453125)
--(axis cs:11100,350.110931396484)
--(axis cs:11000,352.801696777344)
--(axis cs:10900,352.771484375)
--(axis cs:10800,344.261779785156)
--(axis cs:10700,364.205871582031)
--(axis cs:10600,401.819366455078)
--(axis cs:10500,444.548034667969)
--(axis cs:10400,461.614074707031)
--(axis cs:10300,474.380859375)
--(axis cs:10200,522.602355957031)
--(axis cs:10100,534.526245117188)
--(axis cs:10000,492.624206542969)
--(axis cs:9900,468.660949707031)
--(axis cs:9800,460.585144042969)
--(axis cs:9700,383.435943603516)
--(axis cs:9600,361.928527832031)
--(axis cs:9500,327.735168457031)
--(axis cs:9400,325.326568603516)
--(axis cs:9300,301.502502441406)
--(axis cs:9200,312.359161376953)
--(axis cs:9100,318.175964355469)
--(axis cs:9000,312.702911376953)
--(axis cs:8900,297.044006347656)
--(axis cs:8800,297.390197753906)
--(axis cs:8700,257.573120117188)
--(axis cs:8600,237.922271728516)
--(axis cs:8500,258.31640625)
--(axis cs:8400,287.350860595703)
--(axis cs:8300,290.197601318359)
--(axis cs:8200,333.932800292969)
--(axis cs:8100,365.895690917969)
--(axis cs:8000,381.023315429688)
--(axis cs:7900,363.215240478516)
--(axis cs:7800,388.418853759766)
--(axis cs:7700,448.563293457031)
--(axis cs:7600,502.245147705078)
--(axis cs:7500,526.680847167969)
--(axis cs:7400,533.376159667969)
--(axis cs:7300,523.060852050781)
--(axis cs:7200,509.383087158203)
--(axis cs:7100,477.540344238281)
--(axis cs:7000,497.174560546875)
--(axis cs:6900,525.52734375)
--(axis cs:6800,537.726196289062)
--(axis cs:6700,507.900207519531)
--(axis cs:6600,463.028503417969)
--(axis cs:6500,430.086059570312)
--(axis cs:6400,420.608032226562)
--(axis cs:6300,368.781890869141)
--(axis cs:6200,366.047302246094)
--(axis cs:6100,365.952545166016)
--(axis cs:6000,403.075103759766)
--(axis cs:5900,421.165222167969)
--(axis cs:5800,412.1591796875)
--(axis cs:5700,433.427124023438)
--(axis cs:5600,419.231781005859)
--(axis cs:5500,372.352722167969)
--(axis cs:5400,345.239074707031)
--(axis cs:5300,359.612609863281)
--(axis cs:5200,313.469635009766)
--(axis cs:5100,313.383087158203)
--(axis cs:5000,330.706390380859)
--(axis cs:4900,337.056304931641)
--(axis cs:4800,331.103881835938)
--(axis cs:4700,358.553955078125)
--(axis cs:4600,356.223663330078)
--(axis cs:4500,361.139068603516)
--(axis cs:4400,380.112731933594)
--(axis cs:4300,368.809509277344)
--(axis cs:4200,305.40673828125)
--(axis cs:4100,316.763366699219)
--(axis cs:4000,322.122833251953)
--(axis cs:3900,334.707702636719)
--(axis cs:3800,365.058410644531)
--(axis cs:3700,365.880920410156)
--(axis cs:3600,328.037231445312)
--(axis cs:3500,278.644287109375)
--(axis cs:3400,224.760604858398)
--(axis cs:3300,191.840270996094)
--(axis cs:3200,181.021011352539)
--(axis cs:3100,204.642532348633)
--(axis cs:3000,220.413558959961)
--(axis cs:2900,218.617645263672)
--(axis cs:2800,199.951293945312)
--(axis cs:2700,196.722106933594)
--(axis cs:2600,184.029632568359)
--(axis cs:2500,160.153564453125)
--(axis cs:2400,160.087005615234)
--(axis cs:2300,144.508728027344)
--(axis cs:2200,149.102935791016)
--(axis cs:2100,123.597869873047)
--(axis cs:2000,113.937240600586)
--(axis cs:1900,99.9110794067383)
--(axis cs:1800,93.7909088134766)
--(axis cs:1700,79.0804672241211)
--(axis cs:1600,73.0702285766602)
--(axis cs:1500,70.9086151123047)
--(axis cs:1400,94.2665328979492)
--(axis cs:1300,90.9848937988281)
--(axis cs:1200,100.095748901367)
--(axis cs:1100,104.388732910156)
--(axis cs:1000,96.9970092773438)
--(axis cs:900,62.9253273010254)
--(axis cs:800,60.1164665222168)
--(axis cs:700,56.8890686035156)
--(axis cs:600,63.3722305297852)
--(axis cs:500,100.656539916992)
--(axis cs:400,310.820098876953)
--(axis cs:300,322.988311767578)
--(axis cs:200,306.850463867188)
--(axis cs:100,286.942504882812)
--(axis cs:0,237.925003051758)
--cycle;

\path [fill=white!40.1960784313725!black, fill opacity=0.4, ultra thick]
(axis cs:0,0.00546552613377571)
--(axis cs:0,0.00483751576393843)
--(axis cs:100,0.00483698956668377)
--(axis cs:200,0.00271829543635249)
--(axis cs:300,0.000903920852579176)
--(axis cs:400,6.10426059211022e-06)
--(axis cs:500,0)
--(axis cs:600,0)
--(axis cs:700,0)
--(axis cs:800,0)
--(axis cs:900,1.67334255820606e-05)
--(axis cs:1000,8.72332602739334e-05)
--(axis cs:1100,8.72332602739334e-05)
--(axis cs:1200,0.000130596759845503)
--(axis cs:1300,0.000191313039977103)
--(axis cs:1400,0.000166424026247114)
--(axis cs:1500,0.000149114988744259)
--(axis cs:1600,0.000694442540407181)
--(axis cs:1700,0.000593376404140145)
--(axis cs:1800,0.000740136136300862)
--(axis cs:1900,0.000910972594283521)
--(axis cs:2000,0.00115554046351463)
--(axis cs:2100,0.000687542837113142)
--(axis cs:2200,0.0013356547569856)
--(axis cs:2300,0.000495161104481667)
--(axis cs:2400,0.000901719904504716)
--(axis cs:2500,0.000662741076666862)
--(axis cs:2600,0.000930432230234146)
--(axis cs:2700,0.00092057790607214)
--(axis cs:2800,0.00213234964758158)
--(axis cs:2900,0.00220429827459157)
--(axis cs:3000,0.00167833059094846)
--(axis cs:3100,0.00168134330306202)
--(axis cs:3200,0.00222564116120338)
--(axis cs:3300,0.00168862869031727)
--(axis cs:3400,0.00132358376868069)
--(axis cs:3500,0.00168128393124789)
--(axis cs:3600,0.00169371941592544)
--(axis cs:3700,0.00126785563770682)
--(axis cs:3800,0.00104487361386418)
--(axis cs:3900,0.00144222029484808)
--(axis cs:4000,0.00341570097953081)
--(axis cs:4100,0.00186446949373931)
--(axis cs:4200,0.00308691547252238)
--(axis cs:4300,0.002515465952456)
--(axis cs:4400,0.000986131140962243)
--(axis cs:4500,0.000595399062149227)
--(axis cs:4600,0.000737183494493365)
--(axis cs:4700,0.000612314732279629)
--(axis cs:4800,0.000978122581727803)
--(axis cs:4900,0.000997256487607956)
--(axis cs:5000,0.00105053244624287)
--(axis cs:5100,0.0010830641258508)
--(axis cs:5200,0.00166286085732281)
--(axis cs:5300,0.00133092363830656)
--(axis cs:5400,0.00143646053038538)
--(axis cs:5500,0.00201174290850759)
--(axis cs:5600,0.00213901605457067)
--(axis cs:5700,0.00149803597014397)
--(axis cs:5800,0.00236350880004466)
--(axis cs:5900,0.00192027376033366)
--(axis cs:6000,0.00150494265835732)
--(axis cs:6100,0.00276569416746497)
--(axis cs:6200,0.00299112359061837)
--(axis cs:6300,0.00239076768048108)
--(axis cs:6400,0.00338934501633048)
--(axis cs:6500,0.00337997521273792)
--(axis cs:6600,0.00196414301171899)
--(axis cs:6700,0.0019818632863462)
--(axis cs:6800,0.00218252534978092)
--(axis cs:6900,0.0013943666126579)
--(axis cs:7000,0.0027922778390348)
--(axis cs:7100,0.00435074558481574)
--(axis cs:7200,0.00452185655012727)
--(axis cs:7300,0.00533555448055267)
--(axis cs:7400,0.00214294088073075)
--(axis cs:7500,0.00293785729445517)
--(axis cs:7600,0.00284295971505344)
--(axis cs:7700,0.00272319605574012)
--(axis cs:7800,0.00262545933946967)
--(axis cs:7900,0.0018497024429962)
--(axis cs:8000,0.00130684673786163)
--(axis cs:8100,0.00141834549140185)
--(axis cs:8200,0.00184761837590486)
--(axis cs:8300,0.00211975281126797)
--(axis cs:8400,0.00209931377321482)
--(axis cs:8500,0.00178852677345276)
--(axis cs:8600,0.00241603259928524)
--(axis cs:8700,0.00189135072287172)
--(axis cs:8800,0.00188021757639945)
--(axis cs:8900,0.00384205020964146)
--(axis cs:9000,0.00416135555133224)
--(axis cs:9100,0.00387640669941902)
--(axis cs:9200,0.00507509708404541)
--(axis cs:9300,0.0036198329180479)
--(axis cs:9400,0.00233557214960456)
--(axis cs:9500,0.00245482753962278)
--(axis cs:9600,0.00192187773063779)
--(axis cs:9700,0.00183289649430662)
--(axis cs:9800,0.00195123453158885)
--(axis cs:9900,0.00113551015965641)
--(axis cs:10000,0.00103186967317015)
--(axis cs:10100,0.00237001175992191)
--(axis cs:10200,0.00203695590607822)
--(axis cs:10300,0.00358482031151652)
--(axis cs:10400,0.00296826963312924)
--(axis cs:10500,0.00314995343796909)
--(axis cs:10600,0.00276533956639469)
--(axis cs:10700,0.0026103975251317)
--(axis cs:10800,0.00124095077626407)
--(axis cs:10900,0.000994336558505893)
--(axis cs:11000,0.00172268750611693)
--(axis cs:11100,0.00222566118463874)
--(axis cs:11200,0.00243891472928226)
--(axis cs:11300,0.00285938964225352)
--(axis cs:11400,0.00296008097939193)
--(axis cs:11500,0.00243562995456159)
--(axis cs:11600,0.00163811119273305)
--(axis cs:11700,0.00220730691216886)
--(axis cs:11800,0.00183904636651278)
--(axis cs:11900,0.0022596896160394)
--(axis cs:12000,0.00233743595890701)
--(axis cs:12100,0.00299625401385128)
--(axis cs:12200,0.00432268995791674)
--(axis cs:12300,0.00276877102442086)
--(axis cs:12400,0.00276521313935518)
--(axis cs:12500,0.00378331495448947)
--(axis cs:12600,0.00338948960416019)
--(axis cs:12700,0.00293023604899645)
--(axis cs:12800,0.00308385118842125)
--(axis cs:12900,0.00309920916333795)
--(axis cs:13000,0.00258896639570594)
--(axis cs:13100,0.00249582529067993)
--(axis cs:13200,0.00244441628456116)
--(axis cs:13300,0.0023071407340467)
--(axis cs:13400,0.00345491315238178)
--(axis cs:13500,0.00344536988995969)
--(axis cs:13600,0.00355582241900265)
--(axis cs:13700,0.00340813770890236)
--(axis cs:13800,0.00353825464844704)
--(axis cs:13900,0.00303652859292924)
--(axis cs:14000,0.0030118846334517)
--(axis cs:14100,0.00288993725553155)
--(axis cs:14200,0.00419694511219859)
--(axis cs:14300,0.00325419893488288)
--(axis cs:14400,0.00293771037831903)
--(axis cs:14500,0.00266131572425365)
--(axis cs:14600,0.00294919102452695)
--(axis cs:14700,0.00174391525797546)
--(axis cs:14800,0.00249302503652871)
--(axis cs:14900,0.00234586698934436)
--(axis cs:15000,0.00203636894002557)
--(axis cs:15100,0.00197851657867432)
--(axis cs:15200,0.00426848279312253)
--(axis cs:15300,0.00371221313253045)
--(axis cs:15400,0.0042867548763752)
--(axis cs:15500,0.00355703826062381)
--(axis cs:15600,0.0035890459548682)
--(axis cs:15700,0.00240503158420324)
--(axis cs:15800,0.00283912662416697)
--(axis cs:15900,0.00273391371592879)
--(axis cs:16000,0.00262057385407388)
--(axis cs:16100,0.00256977090612054)
--(axis cs:16200,0.0023155331145972)
--(axis cs:16300,0.00133770704269409)
--(axis cs:16400,0.00251871347427368)
--(axis cs:16500,0.00263789901509881)
--(axis cs:16600,0.00264016096480191)
--(axis cs:16700,0.00350009673275054)
--(axis cs:16800,0.00352751603350043)
--(axis cs:16900,0.00253958068788052)
--(axis cs:17000,0.00244067911989987)
--(axis cs:17100,0.00252106273546815)
--(axis cs:17200,0.00220823707059026)
--(axis cs:17300,0.00235371547751129)
--(axis cs:17400,0.00304657546803355)
--(axis cs:17500,0.00237484718672931)
--(axis cs:17600,0.00309207942336798)
--(axis cs:17700,0.00294109573587775)
--(axis cs:17800,0.00393783301115036)
--(axis cs:17900,0.00330180791206658)
--(axis cs:18000,0.00333225727081299)
--(axis cs:18100,0.00196844339370728)
--(axis cs:18200,0.00179911847226322)
--(axis cs:18300,0.00223048916086555)
--(axis cs:18400,0.00258115539327264)
--(axis cs:18500,0.00278441328555346)
--(axis cs:18600,0.00270497403107584)
--(axis cs:18700,0.00227294093929231)
--(axis cs:18800,0.0031800998840481)
--(axis cs:18900,0.00359323644079268)
--(axis cs:19000,0.00362445856444538)
--(axis cs:19100,0.00341089186258614)
--(axis cs:19200,0.00401407293975353)
--(axis cs:19300,0.00493527669459581)
--(axis cs:19400,0.00239985249936581)
--(axis cs:19500,0.00246105180121958)
--(axis cs:19600,0.00270561757497489)
--(axis cs:19700,0.00278289546258748)
--(axis cs:19800,0.00273652328178287)
--(axis cs:19900,0.00338268000632524)
--(axis cs:20000,0.00305422442033887)
--(axis cs:20100,0.00426567438989878)
--(axis cs:20200,0.00390973314642906)
--(axis cs:20300,0.0044286185875535)
--(axis cs:20400,0.00576056260615587)
--(axis cs:20500,0.00591312628239393)
--(axis cs:20600,0.00502048386260867)
--(axis cs:20700,0.00496227154508233)
--(axis cs:20800,0.00416136672720313)
--(axis cs:20900,0.00327011034823954)
--(axis cs:21000,0.00346823898144066)
--(axis cs:21100,0.00350130931474268)
--(axis cs:21200,0.00474364450201392)
--(axis cs:21300,0.00519083021208644)
--(axis cs:21400,0.00467483140528202)
--(axis cs:21500,0.00501247914507985)
--(axis cs:21600,0.00463953753933311)
--(axis cs:21700,0.00341665185987949)
--(axis cs:21800,0.00322266737930477)
--(axis cs:21900,0.00306874443776906)
--(axis cs:22000,0.00245116301812232)
--(axis cs:22100,0.00254172482527792)
--(axis cs:22200,0.0025615612976253)
--(axis cs:22300,0.00225329003296793)
--(axis cs:22400,0.00237437034957111)
--(axis cs:22500,0.00276885414496064)
--(axis cs:22600,0.00316216051578522)
--(axis cs:22700,0.00391185563057661)
--(axis cs:22800,0.0043192645534873)
--(axis cs:22900,0.00515468325465918)
--(axis cs:23000,0.00535854138433933)
--(axis cs:23100,0.00508613279089332)
--(axis cs:23200,0.00438877008855343)
--(axis cs:23300,0.00392786599695683)
--(axis cs:23400,0.0036476687528193)
--(axis cs:23500,0.00331310811452568)
--(axis cs:23600,0.00459592789411545)
--(axis cs:23700,0.00440153665840626)
--(axis cs:23800,0.00555700063705444)
--(axis cs:23900,0.00501228636130691)
--(axis cs:24000,0.00479469262063503)
--(axis cs:24100,0.00347996759228408)
--(axis cs:24200,0.00362211838364601)
--(axis cs:24300,0.00509118940681219)
--(axis cs:24400,0.0051051820628345)
--(axis cs:24500,0.00565676670521498)
--(axis cs:24600,0.00599058857187629)
--(axis cs:24700,0.00592584628611803)
--(axis cs:24800,0.00345480465330184)
--(axis cs:24900,0.00403713714331388)
--(axis cs:25000,0.00415077293291688)
--(axis cs:25100,0.00442524719983339)
--(axis cs:25200,0.00480891577899456)
--(axis cs:25300,0.00457455916330218)
--(axis cs:25400,0.00417455192655325)
--(axis cs:25500,0.00359273934736848)
--(axis cs:25600,0.00308434548787773)
--(axis cs:25700,0.00300519471056759)
--(axis cs:25800,0.00407980522140861)
--(axis cs:25900,0.00405621435493231)
--(axis cs:26000,0.00423480663448572)
--(axis cs:26100,0.00418767239898443)
--(axis cs:26200,0.00416082050651312)
--(axis cs:26300,0.00323889055289328)
--(axis cs:26400,0.0030115032568574)
--(axis cs:26500,0.00272920029237866)
--(axis cs:26600,0.00368376052938402)
--(axis cs:26700,0.00373112084344029)
--(axis cs:26800,0.00444256421178579)
--(axis cs:26900,0.00435787718743086)
--(axis cs:27000,0.00463553983718157)
--(axis cs:27100,0.00424590660259128)
--(axis cs:27200,0.00462279887869954)
--(axis cs:27300,0.00447339378297329)
--(axis cs:27400,0.00480052269995213)
--(axis cs:27500,0.00465881079435349)
--(axis cs:27600,0.00447263568639755)
--(axis cs:27700,0.00361617328599095)
--(axis cs:27800,0.00284483167342842)
--(axis cs:27900,0.00326508423313498)
--(axis cs:28000,0.00357314571738243)
--(axis cs:28100,0.00316453236155212)
--(axis cs:28100,0.00972661748528481)
--(axis cs:28100,0.00972661748528481)
--(axis cs:28000,0.00967986043542624)
--(axis cs:27900,0.00971476547420025)
--(axis cs:27800,0.00976560357958078)
--(axis cs:27700,0.0096751693636179)
--(axis cs:27600,0.00959421973675489)
--(axis cs:27500,0.00958068296313286)
--(axis cs:27400,0.00957168359309435)
--(axis cs:27300,0.00959416013211012)
--(axis cs:27200,0.00958315655589104)
--(axis cs:27100,0.00961296819150448)
--(axis cs:27000,0.0095822736620903)
--(axis cs:26900,0.00960342213511467)
--(axis cs:26800,0.0095965713262558)
--(axis cs:26700,0.00966288521885872)
--(axis cs:26600,0.00966790225356817)
--(axis cs:26500,0.0097801461815834)
--(axis cs:26400,0.009745042771101)
--(axis cs:26300,0.00971783231943846)
--(axis cs:26200,0.00962056778371334)
--(axis cs:26100,0.00961813796311617)
--(axis cs:26000,0.00961394235491753)
--(axis cs:25900,0.00963029079139233)
--(axis cs:25800,0.00962806306779385)
--(axis cs:25700,0.00974581204354763)
--(axis cs:25600,0.00973621569573879)
--(axis cs:25500,0.00967771746218204)
--(axis cs:25400,0.00961932167410851)
--(axis cs:25300,0.00958658382296562)
--(axis cs:25200,0.00957118906080723)
--(axis cs:25100,0.00959794502705336)
--(axis cs:25000,0.00962148420512676)
--(axis cs:24900,0.0096321078017354)
--(axis cs:24800,0.00969300325959921)
--(axis cs:24700,0.00955609232187271)
--(axis cs:24600,0.00955805368721485)
--(axis cs:24500,0.00955090299248695)
--(axis cs:24400,0.00955691747367382)
--(axis cs:24300,0.00955743901431561)
--(axis cs:24200,0.00967452581971884)
--(axis cs:24100,0.0096901785582304)
--(axis cs:24000,0.00957203004509211)
--(axis cs:23900,0.00956068374216557)
--(axis cs:23800,0.00955010950565338)
--(axis cs:23700,0.00959984865039587)
--(axis cs:23600,0.00958504993468523)
--(axis cs:23500,0.00970917940139771)
--(axis cs:23400,0.0096717681735754)
--(axis cs:23300,0.00964275281876326)
--(axis cs:23200,0.00960088428109884)
--(axis cs:23100,0.00955763272941113)
--(axis cs:23000,0.00955055933445692)
--(axis cs:22900,0.00955520290881395)
--(axis cs:22800,0.00960665289312601)
--(axis cs:22700,0.00964434631168842)
--(axis cs:22600,0.00972689967602491)
--(axis cs:22500,0.00977513380348682)
--(axis cs:22400,0.00982604082673788)
--(axis cs:22300,0.00984209775924683)
--(axis cs:22200,0.00980161130428314)
--(axis cs:22100,0.00980418547987938)
--(axis cs:22000,0.00981598254293203)
--(axis cs:21900,0.00973813235759735)
--(axis cs:21800,0.00971978157758713)
--(axis cs:21700,0.00969735626131296)
--(axis cs:21600,0.00958204455673695)
--(axis cs:21500,0.00956072099506855)
--(axis cs:21400,0.00957965198904276)
--(axis cs:21300,0.00955413468182087)
--(axis cs:21200,0.00957519561052322)
--(axis cs:21100,0.00968784000724554)
--(axis cs:21000,0.00969153642654419)
--(axis cs:20900,0.00971422158181667)
--(axis cs:20800,0.00962056219577789)
--(axis cs:20700,0.00956303812563419)
--(axis cs:20600,0.00956036895513535)
--(axis cs:20500,0.00955578871071339)
--(axis cs:20400,0.00955240707844496)
--(axis cs:20300,0.00959772150963545)
--(axis cs:20200,0.00964460149407387)
--(axis cs:20100,0.00961128808557987)
--(axis cs:20000,0.00973989628255367)
--(axis cs:19900,0.00941066257655621)
--(axis cs:19800,0.00918510556221008)
--(axis cs:19700,0.00949182361364365)
--(axis cs:19600,0.00934605859220028)
--(axis cs:19500,0.00908891391009092)
--(axis cs:19400,0.00916974153369665)
--(axis cs:19300,0.00925514288246632)
--(axis cs:19200,0.00988036580383778)
--(axis cs:19100,0.0097278393805027)
--(axis cs:19000,0.0097913546487689)
--(axis cs:18900,0.0102973580360413)
--(axis cs:18800,0.0102973580360413)
--(axis cs:18700,0.0094796409830451)
--(axis cs:18600,0.00809080991894007)
--(axis cs:18500,0.00643750419840217)
--(axis cs:18400,0.00483478838577867)
--(axis cs:18300,0.00341312028467655)
--(axis cs:18200,0.00450510997325182)
--(axis cs:18100,0.00438620056957006)
--(axis cs:18000,0.00480936793610454)
--(axis cs:17900,0.0051271915435791)
--(axis cs:17800,0.0052429111674428)
--(axis cs:17700,0.00556178949773312)
--(axis cs:17600,0.0054587796330452)
--(axis cs:17500,0.00437994860112667)
--(axis cs:17400,0.00360985659062862)
--(axis cs:17300,0.00333795580081642)
--(axis cs:17200,0.00253121857531369)
--(axis cs:17100,0.00323015777394176)
--(axis cs:17000,0.00437927059829235)
--(axis cs:16900,0.00482456665486097)
--(axis cs:16800,0.00451077241450548)
--(axis cs:16700,0.00502599030733109)
--(axis cs:16600,0.00432963250204921)
--(axis cs:16500,0.00432313233613968)
--(axis cs:16400,0.00421633338555694)
--(axis cs:16300,0.00649840990081429)
--(axis cs:16200,0.0067102937027812)
--(axis cs:16100,0.00695659127086401)
--(axis cs:16000,0.0064244382083416)
--(axis cs:15900,0.00421866588294506)
--(axis cs:15800,0.00377162685617805)
--(axis cs:15700,0.00412330636754632)
--(axis cs:15600,0.00850956793874502)
--(axis cs:15500,0.0077411001548171)
--(axis cs:15400,0.00849411729723215)
--(axis cs:15300,0.00793438218533993)
--(axis cs:15200,0.00748604582622647)
--(axis cs:15100,0.00423459988087416)
--(axis cs:15000,0.00463910866528749)
--(axis cs:14900,0.00347792496904731)
--(axis cs:14800,0.00382573087699711)
--(axis cs:14700,0.00324236298911273)
--(axis cs:14600,0.00432484783232212)
--(axis cs:14500,0.00462356396019459)
--(axis cs:14400,0.00480239558964968)
--(axis cs:14300,0.00495634879916906)
--(axis cs:14200,0.00646419962868094)
--(axis cs:14100,0.0062364786863327)
--(axis cs:14000,0.00625646254047751)
--(axis cs:13900,0.00834075827151537)
--(axis cs:13800,0.011661565862596)
--(axis cs:13700,0.00999101530760527)
--(axis cs:13600,0.00961694680154324)
--(axis cs:13500,0.00936242006719112)
--(axis cs:13400,0.00742164626717567)
--(axis cs:13300,0.00408290978521109)
--(axis cs:13200,0.00319207459688187)
--(axis cs:13100,0.00568880699574947)
--(axis cs:13000,0.00653011118993163)
--(axis cs:12900,0.00654194178059697)
--(axis cs:12800,0.00595997367054224)
--(axis cs:12700,0.00567395612597466)
--(axis cs:12600,0.00709152920171618)
--(axis cs:12500,0.00655442243441939)
--(axis cs:12400,0.00599974580109119)
--(axis cs:12300,0.00597625970840454)
--(axis cs:12200,0.00698094163089991)
--(axis cs:12100,0.00429215282201767)
--(axis cs:12000,0.00400269031524658)
--(axis cs:11900,0.00513026677072048)
--(axis cs:11800,0.00548080494627357)
--(axis cs:11700,0.00671393517404795)
--(axis cs:11600,0.00662817480042577)
--(axis cs:11500,0.00740686897188425)
--(axis cs:11400,0.00728370808064938)
--(axis cs:11300,0.0071267606690526)
--(axis cs:11200,0.00680378079414368)
--(axis cs:11100,0.00791123695671558)
--(axis cs:11000,0.00648015318438411)
--(axis cs:10900,0.00594560708850622)
--(axis cs:10800,0.00588031858205795)
--(axis cs:10700,0.00509979343041778)
--(axis cs:10600,0.00481646927073598)
--(axis cs:10500,0.0055448180064559)
--(axis cs:10400,0.00537041295319796)
--(axis cs:10300,0.00728061003610492)
--(axis cs:10200,0.00598663184791803)
--(axis cs:10100,0.00617004372179508)
--(axis cs:10000,0.00780967809259892)
--(axis cs:9900,0.00796798430383205)
--(axis cs:9800,0.00408003805205226)
--(axis cs:9700,0.00583626981824636)
--(axis cs:9600,0.00585760734975338)
--(axis cs:9500,0.00495925499126315)
--(axis cs:9400,0.00532786967232823)
--(axis cs:9300,0.00661035813391209)
--(axis cs:9200,0.00717759039252996)
--(axis cs:9100,0.00727905612438917)
--(axis cs:9000,0.00665484368801117)
--(axis cs:8900,0.00668072886765003)
--(axis cs:8800,0.00563851278275251)
--(axis cs:8700,0.00501798512414098)
--(axis cs:8600,0.00510468473657966)
--(axis cs:8500,0.00419219303876162)
--(axis cs:8400,0.00486432481557131)
--(axis cs:8300,0.00449492828920484)
--(axis cs:8200,0.00402408232912421)
--(axis cs:8100,0.00349775003269315)
--(axis cs:8000,0.00522793829441071)
--(axis cs:7900,0.00482235988602042)
--(axis cs:7800,0.00791468936949968)
--(axis cs:7700,0.00621026521548629)
--(axis cs:7600,0.00635387748479843)
--(axis cs:7500,0.00843485537916422)
--(axis cs:7400,0.00953948777168989)
--(axis cs:7300,0.00693160388618708)
--(axis cs:7200,0.00729643041267991)
--(axis cs:7100,0.00712104002013803)
--(axis cs:7000,0.00513294991105795)
--(axis cs:6900,0.00635908730328083)
--(axis cs:6800,0.00402952311560512)
--(axis cs:6700,0.0038591306656599)
--(axis cs:6600,0.00424620695412159)
--(axis cs:6500,0.00622361246496439)
--(axis cs:6400,0.00481010926887393)
--(axis cs:6300,0.0035680322907865)
--(axis cs:6200,0.00423457426950336)
--(axis cs:6100,0.00370505452156067)
--(axis cs:6000,0.00199205987155437)
--(axis cs:5900,0.00228475616313517)
--(axis cs:5800,0.00276757567189634)
--(axis cs:5700,0.00265825679525733)
--(axis cs:5600,0.00391737837344408)
--(axis cs:5500,0.00302409683354199)
--(axis cs:5400,0.00277384370565414)
--(axis cs:5300,0.00252642622217536)
--(axis cs:5200,0.00240896106697619)
--(axis cs:5100,0.00128835497889668)
--(axis cs:5000,0.00151407637167722)
--(axis cs:4900,0.00186747591942549)
--(axis cs:4800,0.00207759882323444)
--(axis cs:4700,0.00173316267319024)
--(axis cs:4600,0.00303433928638697)
--(axis cs:4500,0.00283001735806465)
--(axis cs:4400,0.00580459740012884)
--(axis cs:4300,0.00590650178492069)
--(axis cs:4200,0.00566292461007833)
--(axis cs:4100,0.00550371734425426)
--(axis cs:4000,0.0055136363953352)
--(axis cs:3900,0.00547897256910801)
--(axis cs:3800,0.00506046507507563)
--(axis cs:3700,0.00447312230244279)
--(axis cs:3600,0.0045601618476212)
--(axis cs:3500,0.0050100376829505)
--(axis cs:3400,0.00476583791896701)
--(axis cs:3300,0.00342303281649947)
--(axis cs:3200,0.00376981263980269)
--(axis cs:3100,0.00458634970709682)
--(axis cs:3000,0.00273564527742565)
--(axis cs:2900,0.002783905249089)
--(axis cs:2800,0.00227103987708688)
--(axis cs:2700,0.00286986422725022)
--(axis cs:2600,0.00293836602941155)
--(axis cs:2500,0.00292103295214474)
--(axis cs:2400,0.00213274220004678)
--(axis cs:2300,0.00220579328015447)
--(axis cs:2200,0.00181057641748339)
--(axis cs:2100,0.00180232245475054)
--(axis cs:2000,0.00171651144046336)
--(axis cs:1900,0.00145908107515424)
--(axis cs:1800,0.00136423006188124)
--(axis cs:1700,0.000751428829971701)
--(axis cs:1600,0.0013703202130273)
--(axis cs:1500,0.00137883971910924)
--(axis cs:1400,0.00143318506889045)
--(axis cs:1300,0.00142068066634238)
--(axis cs:1200,0.00129664211999625)
--(axis cs:1100,0.000266197515884414)
--(axis cs:1000,0.000246120675001293)
--(axis cs:900,9.17654469958507e-05)
--(axis cs:800,7.33741326257586e-05)
--(axis cs:700,5.99576388538026e-10)
--(axis cs:600,5.99576388538026e-10)
--(axis cs:500,5.99576388538026e-10)
--(axis cs:400,0.000154673092765734)
--(axis cs:300,0.00116706255357713)
--(axis cs:200,0.00322034885175526)
--(axis cs:100,0.00546487607061863)
--(axis cs:0,0.00546552613377571)
--cycle;

\addplot [ultra thick, color0]
table {%
0 224.896194458008
100 272.092132568359
200 281.175018310547
300 288.550933837891
400 276.11962890625
500 71.3446426391602
600 32.4839477539062
700 31.3121242523193
800 32.5643119812012
900 34.2731437683105
1000 49.293083190918
1100 53.1637954711914
1200 53.6856422424316
1300 54.9357032775879
1400 59.402458190918
1500 48.5678939819336
1600 47.9450950622559
1700 50.6780242919922
1800 61.2941246032715
1900 67.5493927001953
2000 77.6405639648438
2100 86.8087692260742
2200 101.4970703125
2300 96.8659439086914
2400 105.068138122559
2500 105.04581451416
2600 129.207748413086
2700 145.884246826172
2800 160.281829833984
2900 180.489654541016
3000 186.948852539062
3100 164.702911376953
3200 152.406478881836
3300 149.977005004883
3400 164.423477172852
3500 199.915008544922
3700 252.624710083008
3800 259.022338867188
3900 246.61311340332
4000 259.505706787109
4100 265.581268310547
4200 261.547637939453
4300 280.943756103516
4400 288.377532958984
4500 283.536560058594
4600 295.669219970703
4700 312.109375
4800 307.619750976562
4900 321.348205566406
5000 308.849609375
5100 294.108306884766
5200 293.770080566406
5300 322.961151123047
5400 311.358764648438
5500 325.018127441406
5600 357.720489501953
5700 352.162139892578
5800 332.929992675781
5900 333.222381591797
6000 323.579437255859
6100 318.118377685547
6200 316.761871337891
6300 327.505249023438
6400 368.017608642578
6500 398.757385253906
6600 420.60498046875
6700 447.806976318359
6800 467.347900390625
6900 455.010040283203
7100 422.75927734375
7200 433.392700195312
7500 437.303863525391
7600 425.737396240234
7700 399.808868408203
7800 381.175109863281
7900 353.242401123047
8000 341.097961425781
8100 332.720245361328
8200 300.515167236328
8300 269.408081054688
8400 264.634826660156
8500 250.766403198242
8600 233.633331298828
8700 248.902206420898
8800 263.352508544922
8900 273.944671630859
9000 282.149017333984
9100 285.215911865234
9200 283.626068115234
9300 274.730987548828
9400 292.791961669922
9500 295.114776611328
9600 317.216766357422
9700 335.182189941406
9800 366.11474609375
9900 364.543975830078
10000 371.141326904297
10100 391.671295166016
10200 399.588989257812
10300 388.746398925781
10400 373.124176025391
10500 377.047027587891
10600 344.852142333984
10700 335.624847412109
10800 338.241607666016
10900 343.907043457031
11000 342.939514160156
11100 337.588989257812
11200 325.555999755859
11300 323.101409912109
11400 322.569549560547
11500 330.868530273438
11600 349.310729980469
11700 354.727264404297
11800 339.962646484375
11900 333.158355712891
12100 292.582458496094
12200 277.89794921875
12300 282.622161865234
12400 278.998077392578
12600 277.471405029297
12700 287.135406494141
12800 273.946014404297
12900 270.205413818359
13000 256.417388916016
13100 247.104644775391
13200 241.727355957031
13500 260.538604736328
13600 270.82421875
13700 270.359436035156
13800 274.620300292969
14000 278.190093994141
14100 285.719573974609
14200 286.774169921875
14300 284.7578125
14400 286.153442382812
14500 289.977416992188
14600 279.457489013672
14800 253.159637451172
14900 235.199996948242
15000 226.08073425293
15100 229.932525634766
15200 249.953979492188
15400 275.209350585938
15500 277.589782714844
15600 273.837463378906
15700 260.391906738281
15800 265.088500976562
15900 261.282012939453
16000 268.692474365234
16100 273.015625
16300 269.645263671875
16400 279.797973632812
16500 297.685394287109
16600 295.365692138672
16700 304.633575439453
16800 317.283813476562
16900 321.390380859375
17000 306.805145263672
17100 314.014129638672
17200 313.384704589844
17300 307.532623291016
17400 294.057464599609
17500 295.014831542969
17600 298.350433349609
17700 288.936767578125
17800 270.180786132812
17900 261.029663085938
18000 258.126770019531
18100 250.059936523438
18200 255.929382324219
18300 269.167999267578
18400 280.425079345703
18500 295.785461425781
18700 315.725067138672
18800 312.572326660156
18900 312.462524414062
19000 291.030792236328
19100 286.934173583984
19200 287.467712402344
19300 299.346282958984
19400 308.360656738281
19500 307.894287109375
19600 296.805999755859
19700 275.491424560547
19800 262.272735595703
19900 245.996673583984
20000 248.198135375977
20100 246.179458618164
20200 250.442260742188
20300 246.643035888672
20400 249.870010375977
20500 245.553161621094
20600 254.733871459961
20700 253.540313720703
20800 262.412719726562
20900 259.824157714844
21100 264.274780273438
21200 269.705230712891
21300 262.644470214844
21400 264.512969970703
21500 257.464874267578
21600 252.525024414062
21700 262.444000244141
21800 276.177368164062
21900 280.127807617188
22000 296.433898925781
22100 304.679382324219
22300 287.848785400391
22400 286.426300048828
22500 282.363006591797
22600 271.194976806641
22700 268.724029541016
23000 271.868469238281
23300 278.292419433594
23500 276.116729736328
23600 285.675811767578
23700 291.640625
23800 292.940368652344
23900 292.149749755859
24000 295.188842773438
24100 288.945648193359
24200 287.4296875
24300 287.625244140625
24400 291.584442138672
24500 287.935394287109
24600 292.164001464844
24700 300.981262207031
24800 303.734832763672
25000 316.108856201172
25100 317.463104248047
25200 311.640075683594
25300 312.664672851562
25500 309.82080078125
25700 296.609405517578
26000 293.183807373047
26100 298.420867919922
26200 306.763549804688
26300 308.65771484375
26500 308.887084960938
26600 301.019287109375
26700 290.292633056641
26800 281.649017333984
26900 279.385406494141
27000 278.982299804688
27100 280.810363769531
27200 292.326049804688
27400 304.471893310547
27600 310.419219970703
27700 309.070770263672
27800 311.129638671875
28000 311.163116455078
28100 322.181793212891
28200 331.367156982422
28300 335.113037109375
28400 333.093811035156
28500 344.511566162109
28600 342.443237304688
28700 333.545776367188
28800 326.964141845703
28900 325.362487792969
29000 312.751525878906
29100 302.763610839844
29200 295.7109375
29300 297.907867431641
29500 299.479095458984
29600 302.331268310547
29700 307.329071044922
29800 309.275970458984
29900 317.090515136719
30000 331.598999023438
30100 335.748870849609
30200 342.389099121094
30400 342.16455078125
30500 335.962951660156
30600 336.536468505859
30700 328.593719482422
30800 327.693725585938
31000 318.105804443359
31100 324.482757568359
31200 333.796356201172
31300 337.336456298828
31400 336.541656494141
31500 340.043273925781
31700 330.9462890625
31900 329.555694580078
32000 323.942749023438
32100 321.963592529297
32300 327.606842041016
32400 338.300476074219
32500 345.410339355469
32600 354.995910644531
32800 351.572418212891
32900 344.572845458984
33000 340.987487792969
33100 331.520904541016
33200 334.482238769531
33300 332.608856201172
33400 334.910339355469
33500 333.847320556641
33600 340.720275878906
33700 350.121887207031
33800 354.162017822266
34000 356.062957763672
34100 353.044830322266
34200 344.3115234375
34300 343.14892578125
};
\addplot [ultra thick, white!66.2745098039216!black, dash pattern=on 10pt off 5pt]
table {%
0 0.00515152141451836
100 0.00515093328431249
200 0.00298795290291309
300 0.00103488506283611
400 8.00003545009531e-05
500 2.48352838294608e-10
700 2.48352838294608e-10
800 3.03927809000015e-05
900 5.78296749154106e-05
1000 0.000164446042617783
1100 0.000173289939993992
1200 0.000633029616437852
1300 0.000805997056886554
1400 0.000799804634880275
1500 0.000763977353926748
1600 0.000994294881820679
1700 0.000672402500640601
1800 0.00105218321550637
1900 0.00118502660188824
2000 0.00143602560274303
2100 0.00124493287876248
2200 0.00157311570364982
2300 0.00132322299759835
2400 0.00141520402394235
2500 0.00177029706537724
2600 0.00186610058881342
2700 0.0018952211830765
2800 0.00220169546082616
2900 0.00245455862022936
3000 0.00220698839984834
3100 0.00313384691253304
3200 0.00299772713333368
3300 0.00248759193345904
3400 0.00283817504532635
3500 0.00334566156379879
3600 0.0031269402243197
3700 0.0028704886790365
3800 0.00305266887880862
3900 0.00346059631556273
4000 0.00446466961875558
4100 0.00368409371003509
4200 0.0043749213218689
4300 0.00421098247170448
4400 0.00339536461979151
4500 0.00171270803548396
4600 0.00188576127402484
4700 0.00117273861542344
4800 0.00156451866496354
4900 0.0014323660871014
5000 0.00128230464179069
5100 0.00118127488531172
5200 0.00203591072931886
5300 0.00193080306053162
5400 0.00214729411527514
5500 0.00252287788316607
5600 0.00302819791249931
5700 0.00216047838330269
5800 0.00256554246880114
5900 0.00210251519456506
6000 0.00174850143957883
6100 0.00318082049489021
6200 0.00357732269912958
6300 0.00306223123334348
6400 0.00402462901547551
6500 0.00478911679238081
6600 0.00301301316358149
6700 0.00288524804636836
6800 0.00301765650510788
6900 0.00387672684155405
7000 0.00391104491427541
7100 0.00573589187115431
7200 0.00590914208441973
7300 0.00604609632864594
7400 0.00584121374413371
7500 0.00568635761737823
7600 0.00459841964766383
7700 0.0043972977437079
7800 0.00491735385730863
7900 0.00333603098988533
8000 0.00325876055285335
8100 0.00245804828591645
8200 0.00294238142669201
8300 0.00321975094266236
8400 0.00348181929439306
8500 0.0029171125497669
8600 0.00378416874445975
8700 0.00338901253417134
8800 0.00386511348187923
8900 0.00526138814166188
9000 0.00559398671612144
9100 0.00557773094624281
9200 0.00595642672851682
9300 0.00511509506031871
9400 0.00378898321650922
9500 0.00370704126544297
9600 0.00388974160887301
9700 0.00373165146447718
9800 0.0030156362336129
9900 0.00445743277668953
10000 0.00437084026634693
10100 0.00402471702545881
10200 0.00386106502264738
10300 0.00543271377682686
10400 0.0040701269172132
10500 0.00434738583862782
10600 0.0036601850297302
10700 0.00385509640909731
10900 0.00327993743121624
11000 0.00373714161105454
11100 0.00486401654779911
11200 0.00447667110711336
11300 0.00499307457357645
11400 0.00512189511209726
11500 0.00492125051096082
11600 0.00413314439356327
11700 0.00446062255650759
11800 0.00365992565639317
11900 0.00361040094867349
12000 0.00317006278783083
12100 0.00362234865315259
12200 0.00544229010120034
12300 0.00437251524999738
12400 0.00438247853890061
12500 0.00516886962577701
12600 0.00497969705611467
12700 0.00430209608748555
12800 0.00452191149815917
12900 0.0048200530000031
13000 0.00455953972414136
13100 0.00406061904504895
13200 0.002780357375741
13300 0.00315156020224094
13400 0.00543827889487147
13500 0.00640389462932944
13600 0.00663481885567307
13700 0.00669957743957639
13800 0.00759990839287639
13900 0.00568864308297634
14000 0.00463417312130332
14100 0.00454873917624354
14200 0.00533057097345591
14300 0.00398258771747351
14400 0.00376789621077478
14500 0.00364243914373219
14600 0.00363702024333179
14700 0.00249313982203603
14800 0.00315937818959355
14900 0.00291313091292977
15000 0.00316380569711328
15100 0.00301427231170237
15200 0.00587726524099708
15300 0.00580383464694023
15400 0.00639043701812625
15500 0.0056417933665216
15600 0.00600409274920821
15700 0.00332801719196141
15800 0.0033622863702476
15900 0.00347629003226757
16000 0.00452250754460692
16100 0.00462112482637167
16200 0.00445491820573807
16300 0.00390920741483569
16400 0.00333251827396452
16600 0.00348489615134895
16700 0.00426304340362549
16800 0.00409733178094029
16900 0.00383320590481162
17000 0.00329230213537812
17100 0.00287561002187431
17200 0.00239169597625732
17300 0.00284583563916385
17400 0.00332821626216173
17500 0.00337739684619009
17600 0.00427542999386787
17700 0.0042381682433188
17800 0.00459037162363529
17900 0.0042667118832469
18000 0.00406006863340735
18100 0.00305927218869328
18200 0.00310161500237882
18300 0.00280284858308733
18400 0.00369284930638969
18500 0.00470620766282082
18600 0.00539789255708456
18700 0.00587629107758403
18800 0.00682799005880952
18900 0.0071806930936873
19000 0.00670790579169989
19100 0.00656936643645167
19200 0.00694721844047308
19300 0.00673875119537115
19400 0.00578479655086994
19500 0.00577498227357864
19600 0.00602583680301905
19700 0.00613735895603895
19800 0.00596081325784326
19900 0.00639667036011815
20000 0.00639706011861563
20100 0.0069384821690619
20200 0.00677716778591275
20300 0.00701317004859447
20400 0.00760613149031997
20500 0.00765698868781328
20600 0.00729042617604136
20700 0.00726265506818891
20800 0.00689096376299858
20900 0.00649216584861279
21000 0.0065798875875771
21100 0.00659457314759493
21200 0.00715942168608308
21300 0.00737248314544559
21400 0.00712724169716239
21500 0.00728660076856613
21600 0.00711079221218824
21700 0.00655700406059623
21900 0.00640343734994531
22000 0.00613357266411185
22200 0.00618158746510744
22300 0.00604769308120012
22400 0.00610020384192467
22600 0.00644452963024378
22700 0.00677810190245509
22800 0.00696295686066151
22900 0.00735494261607528
23000 0.0074545512907207
23100 0.00732188392430544
23200 0.00699482904747128
23300 0.00678530987352133
23500 0.00651114387437701
23600 0.00709048705175519
23700 0.0070006912574172
23800 0.00753826089203358
23900 0.00728648481890559
24000 0.00718336226418614
24100 0.00658507319167256
24200 0.00664832023903728
24300 0.00732431607320905
24400 0.0073310500010848
24500 0.00757151562720537
24600 0.00768278678879142
24700 0.00766120571643114
24800 0.00657390477135777
24900 0.00683462060987949
25000 0.00688612693920732
25100 0.00701159564778209
25200 0.00719005381688476
25300 0.00708057172596455
25400 0.0068969358690083
25600 0.00641028210520744
25700 0.00637550232931972
25800 0.00685393344610929
25900 0.00684325210750103
26000 0.00692437263205647
26200 0.0068906950764358
26300 0.00647836271673441
26500 0.0062546725384891
26600 0.00667583104223013
26700 0.00669700372964144
26800 0.0070195677690208
26900 0.00698065059259534
27000 0.00710890674963593
27100 0.00692943762987852
27200 0.00710297748446465
27300 0.00703377509489655
27400 0.00718610361218452
27600 0.00703342771157622
27800 0.00630521681159735
27900 0.00648992462083697
28000 0.00662650121375918
28100 0.00644557364284992
};
