# Supplementary material for: Neural Networks with Physics-Informed Architectures and Constraints for Dynamical Systems Modeling
Source: arXiv:2109.06407 source file (2022-12-12)
Supplement: Supplementary file 12 [file geomrelerr.tex]

% This file was created with tikzplotlib v0.9.12.
\begin{tikzpicture}

\definecolor{color0}{rgb}{1,0,1}

\begin{axis}[
legend cell align={left},
legend style={fill opacity=0.8, draw opacity=1, text opacity=1, draw=white!80!black},
log basis y={10},
tick align=outside,
tick pos=left,
x grid style={white!69.0196078431373!black},
xlabel={\(\displaystyle \mathrm{Number \ of \ training \ trajectories }\)},
xmajorgrids,
xmin=-23.95, xmax=524.95,
xtick style={color=black},
y grid style={white!69.0196078431373!black},
ylabel={\(\displaystyle \mathrm{Geometric \ mean \ of \ relative \ error }\)},
ymajorgrids,
ymin=0.06299942014023, ymax=0.517269287287668,
ymode=log,
ytick style={color=black}
]
\path [fill=blue, fill opacity=0.4, semithick]
(axis cs:1,0.450832588657663)
--(axis cs:1,0.342277254094566)
--(axis cs:10,0.193951732104943)
--(axis cs:25,0.150299187024981)
--(axis cs:75,0.139574592806006)
--(axis cs:200,0.127053163665148)
--(axis cs:500,0.12671936290503)
--(axis cs:500,0.173708148227355)
--(axis cs:500,0.173708148227355)
--(axis cs:200,0.153499872891358)
--(axis cs:75,0.175308678055132)
--(axis cs:25,0.200064418380496)
--(axis cs:10,0.242821759343827)
--(axis cs:1,0.450832588657663)
--cycle;

\path [fill=red, fill opacity=0.4, semithick]
(axis cs:1,0.470060717754753)
--(axis cs:1,0.349116601596732)
--(axis cs:10,0.128702420635964)
--(axis cs:25,0.103147952468473)
--(axis cs:75,0.0909859729168512)
--(axis cs:200,0.0821552220450362)
--(axis cs:500,0.0887728774389657)
--(axis cs:500,0.123950443219074)
--(axis cs:500,0.123950443219074)
--(axis cs:200,0.105308444634118)
--(axis cs:75,0.1225136292467)
--(axis cs:25,0.146719670927311)
--(axis cs:10,0.183442881853881)
--(axis cs:1,0.470060717754753)
--cycle;

\path [fill=green!50.1960784313725!black, fill opacity=0.4, semithick]
(axis cs:1,0.460758098853286)
--(axis cs:1,0.332549681437606)
--(axis cs:10,0.104416636058916)
--(axis cs:25,0.0929826811626782)
--(axis cs:75,0.0840021843585121)
--(axis cs:200,0.0737448759121545)
--(axis cs:500,0.0693265017147747)
--(axis cs:500,0.0930321786056807)
--(axis cs:500,0.0930321786056807)
--(axis cs:200,0.0942462047210047)
--(axis cs:75,0.107495555657725)
--(axis cs:25,0.119711127995211)
--(axis cs:10,0.131280766537419)
--(axis cs:1,0.460758098853286)
--cycle;

\path [fill=color0, fill opacity=0.4, semithick]
(axis cs:1,0.457690971213657)
--(axis cs:1,0.329526233032621)
--(axis cs:10,0.103653766848593)
--(axis cs:25,0.0935290442563888)
--(axis cs:75,0.0827389188560648)
--(axis cs:200,0.075193272762717)
--(axis cs:500,0.073899063733729)
--(axis cs:500,0.098851571947577)
--(axis cs:500,0.098851571947577)
--(axis cs:200,0.0969252035812792)
--(axis cs:75,0.100867508333778)
--(axis cs:25,0.134153717115168)
--(axis cs:10,0.131659006313328)
--(axis cs:1,0.457690971213657)
--cycle;

\addplot [semithick, blue, mark=asterisk, mark size=4, mark options={solid}]
table {%
1 0.396554887294769
10 0.218386724591255
25 0.175181820988655
75 0.157441630959511
200 0.140276536345482
500 0.150213733315468
};
\addlegendentry{No si.}
\addplot [semithick, red, mark=asterisk, mark size=4, mark options={solid}]
table {%
1 0.409588694572449
10 0.156072616577148
25 0.124933794140816
75 0.106749795377254
200 0.0937318354845047
500 0.106361664831638
};
\addlegendentry{Si 2}
\addplot [semithick, green!50.1960784313725!black, mark=asterisk, mark size=4, mark options={solid}]
table {%
1 0.396653860807419
10 0.117848709225655
25 0.106346897780895
75 0.0957488790154457
200 0.0839955359697342
500 0.0811793431639671
};
\addlegendentry{si 3}
\addplot [semithick, color0, mark=asterisk, mark size=4, mark options={solid}]
table {%
1 0.393608659505844
10 0.117656394839287
25 0.113841384649277
75 0.0918032079935074
200 0.0860592424869537
500 0.0863753259181976
};
\addlegendentry{si 4}
\end{axis}

\end{tikzpicture}
