# Supplementary material for: Neural Networks with Physics-Informed Architectures and Constraints for Dynamical Systems Modeling
Source: arXiv:2109.06407 source file (2022-12-12)
Supplement: Supplementary file 13 [file relerr_500.tex]

% This file was created with tikzplotlib v0.9.12.
\begin{tikzpicture}

\definecolor{color0}{rgb}{1,0,1}

\begin{axis}[
legend cell align={left},
legend style={
  fill opacity=0.8,
  draw opacity=1,
  text opacity=1,
  at={(0.03,0.97)},
  anchor=north west,
  draw=white!80!black
},
log basis y={10},
tick align=outside,
tick pos=left,
x grid style={white!69.0196078431373!black},
xlabel={\(\displaystyle \mathrm{Time \ (seconds)}\)},
xmajorgrids,
xmin=0.000499999988824129, xmax=0.0994999977760017,
xtick style={color=black},
y grid style={white!69.0196078431373!black},
ylabel={\(\displaystyle \mathrm{Relative \ error}\) (\(\displaystyle N_{\mathrm{train}}=500\))},
ymajorgrids,
ymin=0.0403423932359269, ymax=0.186214482340161,
ymode=log,
ytick style={color=black}
]
\path [fill=blue, fill opacity=0.4, semithick]
(axis cs:0.00499999988824129,0.0981471371189214)
--(axis cs:0.00499999988824129,0.0693458930148139)
--(axis cs:0.00999999977648258,0.0768913576643062)
--(axis cs:0.0149999996647239,0.0805582154812716)
--(axis cs:0.0199999995529652,0.0845196110592269)
--(axis cs:0.0249999994412065,0.0910616688263388)
--(axis cs:0.0299999993294477,0.0960605583494559)
--(axis cs:0.034999999217689,0.0995347371251724)
--(axis cs:0.0399999991059303,0.102204599471983)
--(axis cs:0.0449999989941716,0.105266256553993)
--(axis cs:0.0499999988824129,0.107840601840457)
--(axis cs:0.0549999987706542,0.11024953719084)
--(axis cs:0.0599999986588955,0.112444513695491)
--(axis cs:0.0649999985471368,0.114894346999308)
--(axis cs:0.0699999984353781,0.117045373991443)
--(axis cs:0.0749999983236194,0.119135580434824)
--(axis cs:0.0799999982118607,0.121087367134153)
--(axis cs:0.0849999981001019,0.123097295652794)
--(axis cs:0.0899999979883432,0.124914798373905)
--(axis cs:0.0949999978765845,0.12671936290503)
--(axis cs:0.0949999978765845,0.173708148227355)
--(axis cs:0.0949999978765845,0.173708148227355)
--(axis cs:0.0899999979883432,0.169887707845062)
--(axis cs:0.0849999981001019,0.165865428211006)
--(axis cs:0.0799999982118607,0.161634229731955)
--(axis cs:0.0749999983236194,0.157497989129546)
--(axis cs:0.0699999984353781,0.153176988531972)
--(axis cs:0.0649999985471368,0.148494744088243)
--(axis cs:0.0599999986588955,0.143608795563009)
--(axis cs:0.0549999987706542,0.139183186266431)
--(axis cs:0.0499999988824129,0.134703444736652)
--(axis cs:0.0449999989941716,0.130206618772106)
--(axis cs:0.0399999991059303,0.125438398773785)
--(axis cs:0.034999999217689,0.121120112118062)
--(axis cs:0.0299999993294477,0.116526519213719)
--(axis cs:0.0249999994412065,0.111403463333061)
--(axis cs:0.0199999995529652,0.108039080407262)
--(axis cs:0.0149999996647239,0.105659266717689)
--(axis cs:0.00999999977648258,0.103238590486459)
--(axis cs:0.00499999988824129,0.0981471371189214)
--cycle;

\path [fill=red, fill opacity=0.4, semithick]
(axis cs:0.00499999988824129,0.0830617524482067)
--(axis cs:0.00499999988824129,0.0577385334961019)
--(axis cs:0.00999999977648258,0.0609472347238716)
--(axis cs:0.0149999996647239,0.062344939486539)
--(axis cs:0.0199999995529652,0.0645523857627769)
--(axis cs:0.0249999994412065,0.0688552481509171)
--(axis cs:0.0299999993294477,0.0721968693716407)
--(axis cs:0.034999999217689,0.0740155351438639)
--(axis cs:0.0399999991059303,0.0747251433342523)
--(axis cs:0.0449999989941716,0.076196688060175)
--(axis cs:0.0499999988824129,0.078265236166539)
--(axis cs:0.0549999987706542,0.0799868066050893)
--(axis cs:0.0599999986588955,0.0811944321399374)
--(axis cs:0.0649999985471368,0.0826790375067071)
--(axis cs:0.0699999984353781,0.0842147872536796)
--(axis cs:0.0749999983236194,0.0852262409253277)
--(axis cs:0.0799999982118607,0.0858964548859035)
--(axis cs:0.0849999981001019,0.0869284669749143)
--(axis cs:0.0899999979883432,0.0880689473886511)
--(axis cs:0.0949999978765845,0.0887728774389657)
--(axis cs:0.0949999978765845,0.123950443219074)
--(axis cs:0.0949999978765845,0.123950443219074)
--(axis cs:0.0899999979883432,0.122065787742204)
--(axis cs:0.0849999981001019,0.119591672074542)
--(axis cs:0.0799999982118607,0.117123474651583)
--(axis cs:0.0749999983236194,0.114965108071722)
--(axis cs:0.0699999984353781,0.112221726189995)
--(axis cs:0.0649999985471368,0.108807137019256)
--(axis cs:0.0599999986588955,0.105237598566073)
--(axis cs:0.0549999987706542,0.102156176573968)
--(axis cs:0.0499999988824129,0.0986413392759387)
--(axis cs:0.0449999989941716,0.0947838197919073)
--(axis cs:0.0399999991059303,0.0911599179141883)
--(axis cs:0.034999999217689,0.0883223634854195)
--(axis cs:0.0299999993294477,0.0853904199404792)
--(axis cs:0.0249999994412065,0.0822060938997066)
--(axis cs:0.0199999995529652,0.0802182975294789)
--(axis cs:0.0149999996647239,0.0799168495767018)
--(axis cs:0.00999999977648258,0.0798972512640844)
--(axis cs:0.00499999988824129,0.0830617524482067)
--cycle;

\path [fill=green!50.1960784313725!black, fill opacity=0.4, semithick]
(axis cs:0.00499999988824129,0.0691418707714119)
--(axis cs:0.00499999988824129,0.0432468939969296)
--(axis cs:0.00999999977648258,0.0516324535170185)
--(axis cs:0.0149999996647239,0.0515130633290674)
--(axis cs:0.0199999995529652,0.0512873514591298)
--(axis cs:0.0249999994412065,0.0531749001829137)
--(axis cs:0.0299999993294477,0.0547475864476341)
--(axis cs:0.034999999217689,0.0563171018417981)
--(axis cs:0.0399999991059303,0.0571659570531023)
--(axis cs:0.0449999989941716,0.0586610050907562)
--(axis cs:0.0499999988824129,0.0600586372681437)
--(axis cs:0.0549999987706542,0.0612916019755903)
--(axis cs:0.0599999986588955,0.0622983017165615)
--(axis cs:0.0649999985471368,0.0635656407422943)
--(axis cs:0.0699999984353781,0.064995355484257)
--(axis cs:0.0749999983236194,0.0661467390966307)
--(axis cs:0.0799999982118607,0.066896883721782)
--(axis cs:0.0849999981001019,0.0678902986932688)
--(axis cs:0.0899999979883432,0.0688010277693822)
--(axis cs:0.0949999978765845,0.0693265017147747)
--(axis cs:0.0949999978765845,0.0930321786056807)
--(axis cs:0.0949999978765845,0.0930321786056807)
--(axis cs:0.0899999979883432,0.0919125371334513)
--(axis cs:0.0849999981001019,0.0902283378317776)
--(axis cs:0.0799999982118607,0.0886564630415355)
--(axis cs:0.0749999983236194,0.0875976061835957)
--(axis cs:0.0699999984353781,0.0861671861597333)
--(axis cs:0.0649999985471368,0.0842818920139673)
--(axis cs:0.0599999986588955,0.0822768049447333)
--(axis cs:0.0549999987706542,0.0810396972361705)
--(axis cs:0.0499999988824129,0.0796091263396972)
--(axis cs:0.0449999989941716,0.0775728662310419)
--(axis cs:0.0399999991059303,0.0749869548046289)
--(axis cs:0.034999999217689,0.0727956040974394)
--(axis cs:0.0299999993294477,0.0707275527701303)
--(axis cs:0.0249999994412065,0.0679617527078296)
--(axis cs:0.0199999995529652,0.0666160932079101)
--(axis cs:0.0149999996647239,0.0669410170690395)
--(axis cs:0.00999999977648258,0.0704492526822372)
--(axis cs:0.00499999988824129,0.0691418707714119)
--cycle;

\path [fill=color0, fill opacity=0.4, semithick]
(axis cs:0.00499999988824129,0.0728660114739282)
--(axis cs:0.00499999988824129,0.0472793839221152)
--(axis cs:0.00999999977648258,0.0522475106476856)
--(axis cs:0.0149999996647239,0.0543423041579315)
--(axis cs:0.0199999995529652,0.0549865341125751)
--(axis cs:0.0249999994412065,0.0575579704268763)
--(axis cs:0.0299999993294477,0.0597066606806348)
--(axis cs:0.034999999217689,0.0611029359784349)
--(axis cs:0.0399999991059303,0.0618320840140064)
--(axis cs:0.0449999989941716,0.0631873537919674)
--(axis cs:0.0499999988824129,0.064806731440754)
--(axis cs:0.0549999987706542,0.0661392594038266)
--(axis cs:0.0599999986588955,0.0671212654631985)
--(axis cs:0.0649999985471368,0.0684943794472619)
--(axis cs:0.0699999984353781,0.0698058700151522)
--(axis cs:0.0749999983236194,0.0707865738041196)
--(axis cs:0.0799999982118607,0.0714254531301117)
--(axis cs:0.0849999981001019,0.0722892435519938)
--(axis cs:0.0899999979883432,0.0731936281646384)
--(axis cs:0.0949999978765845,0.073899063733729)
--(axis cs:0.0949999978765845,0.098851571947577)
--(axis cs:0.0949999978765845,0.098851571947577)
--(axis cs:0.0899999979883432,0.0974827054803171)
--(axis cs:0.0849999981001019,0.0955383551671605)
--(axis cs:0.0799999982118607,0.093652007236664)
--(axis cs:0.0749999983236194,0.0923510896217436)
--(axis cs:0.0699999984353781,0.0907468745546822)
--(axis cs:0.0649999985471368,0.0885441239818889)
--(axis cs:0.0599999986588955,0.0862765882982384)
--(axis cs:0.0549999987706542,0.0849457619405477)
--(axis cs:0.0499999988824129,0.0830950683301027)
--(axis cs:0.0449999989941716,0.0807032698346358)
--(axis cs:0.0399999991059303,0.0778895897794887)
--(axis cs:0.034999999217689,0.0758716613948973)
--(axis cs:0.0299999993294477,0.0730464991303921)
--(axis cs:0.0249999994412065,0.0692151823749083)
--(axis cs:0.0199999995529652,0.0667704042014442)
--(axis cs:0.0149999996647239,0.0689100804883708)
--(axis cs:0.00999999977648258,0.0732407344645434)
--(axis cs:0.00499999988824129,0.0728660114739282)
--cycle;

\addplot [semithick, blue]
table {%
0.00499999523162842 0.0837465077638626
0.00999999046325684 0.0900649651885033
0.0149999856948853 0.0931087359786034
0.0199999809265137 0.0962793454527855
0.0249999761581421 0.101232580840588
0.0299999713897705 0.106293544173241
0.0349999666213989 0.110327422618866
0.0399999618530273 0.113821513950825
0.0449999570846558 0.117736451327801
0.0499999523162842 0.121272020041943
0.0549999475479126 0.124716356396675
0.059999942779541 0.128026649355888
0.065000057220459 0.131694540381432
0.0700000524520874 0.135111182928085
0.0750000476837158 0.138316780328751
0.0850000381469727 0.144481375813484
0.0900000333786011 0.147401243448257
0.0950000286102295 0.150213733315468
};
\addlegendentry{No si.}
\addplot [semithick, red]
table {%
0.00499999523162842 0.0704001411795616
0.00999999046325684 0.0704222470521927
0.0149999856948853 0.0711309015750885
0.0199999809265137 0.0723853409290314
0.0249999761581421 0.0755306631326675
0.0299999713897705 0.0787936374545097
0.0349999666213989 0.081168957054615
0.0399999618530273 0.0829425230622292
0.0449999570846558 0.0854902490973473
0.0499999523162842 0.0884532779455185
0.0549999475479126 0.0910714864730835
0.059999942779541 0.0932160168886185
0.065000057220459 0.0957430973649025
0.0700000524520874 0.0982182696461678
0.0750000476837158 0.100095674395561
0.0800000429153442 0.101509973406792
0.0850000381469727 0.103260084986687
0.0900000333786011 0.105067357420921
0.0950000286102295 0.106361664831638
};
\addlegendentry{Si 2}
\addplot [semithick, green!50.1960784313725!black]
table {%
0.00499999523162842 0.0561943836510181
0.00999999046325684 0.061040848493576
0.0149999856948853 0.0592270456254482
0.0199999809265137 0.0589517205953598
0.0249999761581421 0.0605683177709579
0.0299999713897705 0.0627375692129135
0.0349999666213989 0.0645563378930092
0.0399999618530273 0.0660764425992966
0.0449999570846558 0.0681169256567955
0.0499999523162842 0.0698338747024536
0.0549999475479126 0.071165643632412
0.059999942779541 0.0722875520586967
0.065000057220459 0.0739237666130066
0.0700000524520874 0.0755812674760818
0.0750000476837158 0.0768721699714661
0.0800000429153442 0.0777766704559326
0.0900000333786011 0.080356776714325
0.0950000286102295 0.0811793431639671
};
\addlegendentry{si 3}
\addplot [semithick, color0]
table {%
0.00499999523162842 0.0600726939737797
0.00999999046325684 0.0627441257238388
0.0149999856948853 0.0616261959075928
0.0199999809265137 0.060878474265337
0.0249999761581421 0.0633865743875504
0.0299999713897705 0.0663765668869019
0.0349999666213989 0.0684873014688492
0.0399999618530273 0.0698608309030533
0.0449999570846558 0.0719453096389771
0.0499999523162842 0.0739509016275406
0.0549999475479126 0.0755425170063972
0.059999942779541 0.0766989141702652
0.065000057220459 0.0785192474722862
0.0700000524520874 0.0802763700485229
0.0750000476837158 0.0815688446164131
0.0800000429153442 0.0825387313961983
0.0850000381469727 0.0839137956500053
0.0900000333786011 0.0853381603956223
0.0950000286102295 0.0863753259181976
};
\addlegendentry{si 4}
\end{axis}

\end{tikzpicture}
