# Supplementary material for: Neural Networks with Physics-Informed Architectures and Constraints for Dynamical Systems Modeling
Source: arXiv:2109.06407 source file (2022-12-12)
Supplement: Supplementary file 15 [file traj_err_data.tex]

\path [fill=red, fill opacity=0.4, ultra thick]
(axis cs:1,0.450832588657663)
--(axis cs:1,0.342277254094566)
--(axis cs:10,0.193951732104943)
--(axis cs:25,0.150299187024981)
--(axis cs:75,0.139574592806006)
--(axis cs:200,0.127053163665148)
--(axis cs:500,0.12671936290503)
--(axis cs:500,0.173708148227355)
--(axis cs:500,0.173708148227355)
--(axis cs:200,0.153499872891358)
--(axis cs:75,0.175308678055132)
--(axis cs:25,0.200064418380496)
--(axis cs:10,0.242821759343827)
--(axis cs:1,0.450832588657663)
--cycle;

\path [fill=green!50.1960784313725!black, fill opacity=0.4, ultra thick]
(axis cs:1,0.470060717754753)
--(axis cs:1,0.349116601596732)
--(axis cs:10,0.128702420635964)
--(axis cs:25,0.103147952468473)
--(axis cs:75,0.0909859729168512)
--(axis cs:200,0.0821552220450362)
--(axis cs:500,0.0887728774389657)
--(axis cs:500,0.123950443219074)
--(axis cs:500,0.123950443219074)
--(axis cs:200,0.105308444634118)
--(axis cs:75,0.1225136292467)
--(axis cs:25,0.146719670927311)
--(axis cs:10,0.183442881853881)
--(axis cs:1,0.470060717754753)
--cycle;

\path [fill=color0, fill opacity=0.4, ultra thick]
(axis cs:1,0.460758098853286)
--(axis cs:1,0.332549681437606)
--(axis cs:10,0.104416636058916)
--(axis cs:25,0.0929826811626782)
--(axis cs:75,0.0840021843585121)
--(axis cs:200,0.0737448759121545)
--(axis cs:500,0.0693265017147747)
--(axis cs:500,0.0930321786056807)
--(axis cs:500,0.0930321786056807)
--(axis cs:200,0.0942462047210047)
--(axis cs:75,0.107495555657725)
--(axis cs:25,0.119711127995211)
--(axis cs:10,0.131280766537419)
--(axis cs:1,0.460758098853286)
--cycle;

\path [fill=white!40!black, fill opacity=0.4, ultra thick]
(axis cs:1,0.457690971213657)
--(axis cs:1,0.329526233032621)
--(axis cs:10,0.103653766848593)
--(axis cs:25,0.0935290442563888)
--(axis cs:75,0.0827389188560648)
--(axis cs:200,0.075193272762717)
--(axis cs:500,0.073899063733729)
--(axis cs:500,0.098851571947577)
--(axis cs:500,0.098851571947577)
--(axis cs:200,0.0969252035812792)
--(axis cs:75,0.100867508333778)
--(axis cs:25,0.134153717115168)
--(axis cs:10,0.131659006313328)
--(axis cs:1,0.457690971213657)
--cycle;

\addplot [ultra thick, red, mark=*, mark size=1.5, mark options={solid}]
table {%
1 0.396554887294769
10 0.218386724591255
25 0.175181820988655
75 0.157441630959511
200 0.140276536345482
500 0.150213733315468
};
% \addlegendentry{No si.}
\addplot [ultra thick, green!50.1960784313725!black, mark=asterisk, mark size=1.5, mark options={solid}]
table {%
1 0.409588694572449
10 0.156072616577148
25 0.124933794140816
75 0.106749795377254
200 0.0937318354845047
500 0.106361664831638
};
% \addlegendentry{Si 2}
\addplot [ultra thick, color0, mark=*, mark size=1.5, mark options={solid}]
table {%
1 0.396653860807419
10 0.117848709225655
25 0.106346897780895
75 0.0957488790154457
200 0.0839955359697342
500 0.0811793431639671
};
% \addlegendentry{si 3}
\addplot [ultra thick, white!40!black, mark=*, mark size=1.5, mark options={solid}]
table {%
1 0.393608659505844
10 0.117656394839287
25 0.113841384649277
75 0.0918032079935074
200 0.0860592424869537
500 0.0863753259181976
};
% \addlegendentry{si 4}
