# Supplementary material for: Neural Networks with Physics-Informed Architectures and Constraints for Dynamical Systems Modeling
Source: arXiv:2109.06407 source file (2022-12-12)
Supplement: Supplementary file 16 [file constraint_loss_data.tex]

\path [fill=color0, fill opacity=0.4, ultra thick]
(axis cs:0,5223.42333984375)
--(axis cs:0,1456.70703125)
--(axis cs:100,1457.14331054688)
--(axis cs:200,1455.37463378906)
--(axis cs:300,557.868896484375)
--(axis cs:400,617.975952148438)
--(axis cs:500,695.533813476562)
--(axis cs:600,57.2175788879395)
--(axis cs:700,617.562866210938)
--(axis cs:800,683.730834960938)
--(axis cs:900,717.829711914062)
--(axis cs:1000,898.556640625)
--(axis cs:1100,1187.13903808594)
--(axis cs:1200,1202.84143066406)
--(axis cs:1300,1389.24645996094)
--(axis cs:1400,1409.875)
--(axis cs:1500,1507.22302246094)
--(axis cs:1600,2015.07971191406)
--(axis cs:1600,5391.03759765625)
--(axis cs:1600,5391.03759765625)
--(axis cs:1500,8856.5546875)
--(axis cs:1400,8659.91796875)
--(axis cs:1300,8451.9052734375)
--(axis cs:1200,8276.607421875)
--(axis cs:1100,8233.419921875)
--(axis cs:1000,7407.00146484375)
--(axis cs:900,7061.953125)
--(axis cs:800,4261.2734375)
--(axis cs:700,4154.76220703125)
--(axis cs:600,4034.8134765625)
--(axis cs:500,4255.35595703125)
--(axis cs:400,4237.27294921875)
--(axis cs:300,4240.666015625)
--(axis cs:200,5221.0107421875)
--(axis cs:100,5223.4228515625)
--(axis cs:0,5223.42333984375)
--cycle;

\path [fill=white!40.1960784313725!black, fill opacity=0.4, ultra thick]
(axis cs:0,14.111156463623)
--(axis cs:0,7.47982849134132e-05)
--(axis cs:100,7.2385802923236e-05)
--(axis cs:200,7.23291959729977e-05)
--(axis cs:300,7.23291959729977e-05)
--(axis cs:400,7.23291959729977e-05)
--(axis cs:500,7.23291959729977e-05)
--(axis cs:600,7.23291959729977e-05)
--(axis cs:700,7.23291595932096e-05)
--(axis cs:800,7.19058007234707e-05)
--(axis cs:900,7.19058007234707e-05)
--(axis cs:1000,0)
--(axis cs:1100,0)
--(axis cs:1200,0)
--(axis cs:1300,0)
--(axis cs:1400,0)
--(axis cs:1500,0)
--(axis cs:1600,0)
--(axis cs:1600,0.000755777466110885)
--(axis cs:1600,0.000755777466110885)
--(axis cs:1500,0.000755777466110885)
--(axis cs:1400,0.000755777466110885)
--(axis cs:1300,0.000777501205448061)
--(axis cs:1200,0.000858554907608777)
--(axis cs:1100,0.102439239621162)
--(axis cs:1000,0.102252602577209)
--(axis cs:900,0.102258905768394)
--(axis cs:800,0.102342382073402)
--(axis cs:700,0.102342419326305)
--(axis cs:600,0.101785019040108)
--(axis cs:500,0.101785019040108)
--(axis cs:400,14.2128505706787)
--(axis cs:300,14.2128276824951)
--(axis cs:200,14.2127466201782)
--(axis cs:100,14.1111545562744)
--(axis cs:0,14.111156463623)
--cycle;

\addplot [ultra thick, color0]
table {%
0 3340.064453125
200 3338.19287109375
300 2399.26806640625
400 2427.6240234375
500 2475.4443359375
600 1772.1611328125
700 2114.14135742188
800 2240.84790039062
900 3416.64111328125
1000 3819.67358398438
1100 4368.2060546875
1200 4427.52783203125
1300 4642.56591796875
1500 4868.39208984375
1600 3703.05883789062
};
\addplot [ultra thick, white!66.2745098039216!black]
table {%
0 5.84526538848877
100 5.84526348114014
200 5.8873438835144
400 5.8873872756958
500 0.04239222407341
600 0.04239222407341
700 0.0426875613629818
800 0.0426874347031116
900 0.0424427315592766
1100 0.0424983836710453
1200 0.000418209296185523
1300 0.000384131184546277
1400 0.000374975992599502
1600 0.000374975992599502
};
