# Supplementary material for: Neural Networks with Physics-Informed Architectures and Constraints for Dynamical Systems Modeling
Source: arXiv:2109.06407 source file (2022-12-12)
Supplement: Supplementary file 18 [file relerr_data.tex]

\path [fill=red, fill opacity=0.4, ultra thick]
(axis cs:0.00187499995809048,0.223284651023948)
--(axis cs:0.00187499995809048,0.187695007463598)
--(axis cs:0.00374999991618097,0.238073378583014)
--(axis cs:0.00562499987427145,0.272915417762303)
--(axis cs:0.00749999983236194,0.296941764426831)
--(axis cs:0.00937499979045242,0.31378301041161)
--(axis cs:0.0112499997485429,0.326169058022026)
--(axis cs:0.0131249997066334,0.33603125434734)
--(axis cs:0.0149999996647239,0.344396583523761)
--(axis cs:0.0168749996228144,0.350577990730298)
--(axis cs:0.0187499995809048,0.355902759398283)
--(axis cs:0.0206249995389953,0.360659122884723)
--(axis cs:0.0224999994970858,0.364959140525023)
--(axis cs:0.0243749994551763,0.369079666832317)
--(axis cs:0.0262499994132668,0.373418755106175)
--(axis cs:0.0281249993713573,0.378105818071183)
--(axis cs:0.0299999993294477,0.383109354021729)
--(axis cs:0.0318749992875382,0.387992539662234)
--(axis cs:0.0337499992456287,0.392863938891101)
--(axis cs:0.0356249992037192,0.397422771456937)
--(axis cs:0.0374999991618097,0.40157376413107)
--(axis cs:0.0393749991199002,0.405325760221273)
--(axis cs:0.0412499990779907,0.408780934590834)
--(axis cs:0.0431249990360811,0.411984581000991)
--(axis cs:0.0449999989941716,0.415001821315762)
--(axis cs:0.0468749989522621,0.417721495614524)
--(axis cs:0.0487499989103526,0.420274014769265)
--(axis cs:0.0506249988684431,0.422661631274987)
--(axis cs:0.0524999988265336,0.424919836282206)
--(axis cs:0.054374998784624,0.427128184097617)
--(axis cs:0.0562499987427145,0.429352510089324)
--(axis cs:0.058124998700805,0.43160122785948)
--(axis cs:0.0599999986588955,0.433904146684153)
--(axis cs:0.061874998616986,0.436364983593702)
--(axis cs:0.0637499985750765,0.43889829952594)
--(axis cs:0.0656249985331669,0.441331483302928)
--(axis cs:0.0674999984912574,0.443539617436761)
--(axis cs:0.0693749984493479,0.445540446356029)
--(axis cs:0.0712499984074384,0.447387163250341)
--(axis cs:0.0731249983655289,0.449112071455718)
--(axis cs:0.0731249983655289,0.541743363602843)
--(axis cs:0.0731249983655289,0.541743363602843)
--(axis cs:0.0712499984074384,0.539869819107963)
--(axis cs:0.0693749984493479,0.537857723342209)
--(axis cs:0.0674999984912574,0.535690275685537)
--(axis cs:0.0656249985331669,0.533342389927295)
--(axis cs:0.0637499985750765,0.530805451220647)
--(axis cs:0.061874998616986,0.528177473863705)
--(axis cs:0.0599999986588955,0.525507110434785)
--(axis cs:0.058124998700805,0.522819855880136)
--(axis cs:0.0562499987427145,0.520140647615703)
--(axis cs:0.054374998784624,0.517448198944522)
--(axis cs:0.0524999988265336,0.514722708497198)
--(axis cs:0.0506249988684431,0.511921049201876)
--(axis cs:0.0487499989103526,0.509019604200708)
--(axis cs:0.0468749989522621,0.506061053914449)
--(axis cs:0.0449999989941716,0.503107116256956)
--(axis cs:0.0431249990360811,0.500062132028918)
--(axis cs:0.0412499990779907,0.496999294073496)
--(axis cs:0.0393749991199002,0.493914921542748)
--(axis cs:0.0374999991618097,0.490837674689559)
--(axis cs:0.0356249992037192,0.487716660234649)
--(axis cs:0.0337499992456287,0.484548615123408)
--(axis cs:0.0318749992875382,0.481389369746183)
--(axis cs:0.0299999993294477,0.478257875172665)
--(axis cs:0.0281249993713573,0.474712558954193)
--(axis cs:0.0262499994132668,0.47126126845787)
--(axis cs:0.0243749994551763,0.467746910053326)
--(axis cs:0.0224999994970858,0.463758677179827)
--(axis cs:0.0206249995389953,0.458758689862794)
--(axis cs:0.0187499995809048,0.452237133988835)
--(axis cs:0.0168749996228144,0.44391572654426)
--(axis cs:0.0149999996647239,0.433191093951257)
--(axis cs:0.0131249997066334,0.418590449681734)
--(axis cs:0.0112499997485429,0.401780542791275)
--(axis cs:0.00937499979045242,0.38194061610734)
--(axis cs:0.00749999983236194,0.357533872117525)
--(axis cs:0.00562499987427145,0.325905423696999)
--(axis cs:0.00374999991618097,0.283117501415678)
--(axis cs:0.00187499995809048,0.223284651023948)
--cycle;

\path [fill=blue, fill opacity=0.4, ultra thick]
(axis cs:0.00187499995809048,0.214541418636306)
--(axis cs:0.00187499995809048,0.185881351688115)
--(axis cs:0.00374999991618097,0.236092069616369)
--(axis cs:0.00562499987427145,0.271175634381049)
--(axis cs:0.00749999983236194,0.296051392355213)
--(axis cs:0.00937499979045242,0.314141038170178)
--(axis cs:0.0112499997485429,0.3280265826775)
--(axis cs:0.0131249997066334,0.339346058426552)
--(axis cs:0.0149999996647239,0.34899721967944)
--(axis cs:0.0168749996228144,0.356445171778196)
--(axis cs:0.0187499995809048,0.362689152513271)
--(axis cs:0.0206249995389953,0.367938546340262)
--(axis cs:0.0224999994970858,0.372345878750611)
--(axis cs:0.0243749994551763,0.376289462166616)
--(axis cs:0.0262499994132668,0.380256637769328)
--(axis cs:0.0281249993713573,0.384495361509867)
--(axis cs:0.0299999993294477,0.389011506668433)
--(axis cs:0.0318749992875382,0.39352650055273)
--(axis cs:0.0337499992456287,0.39812376351268)
--(axis cs:0.0356249992037192,0.402566676493214)
--(axis cs:0.0374999991618097,0.406716369576053)
--(axis cs:0.0393749991199002,0.410544983942511)
--(axis cs:0.0412499990779907,0.414152290405695)
--(axis cs:0.0431249990360811,0.417577750791763)
--(axis cs:0.0449999989941716,0.420872654527487)
--(axis cs:0.0468749989522621,0.42399662833414)
--(axis cs:0.0487499989103526,0.427030362276816)
--(axis cs:0.0506249988684431,0.429913438051283)
--(axis cs:0.0524999988265336,0.432640506463098)
--(axis cs:0.054374998784624,0.435272782940318)
--(axis cs:0.0562499987427145,0.437885461904852)
--(axis cs:0.058124998700805,0.440479101953634)
--(axis cs:0.0599999986588955,0.443074451307937)
--(axis cs:0.061874998616986,0.445799145197709)
--(axis cs:0.0637499985750765,0.448588006041982)
--(axis cs:0.0656249985331669,0.451279282940277)
--(axis cs:0.0674999984912574,0.453746066072114)
--(axis cs:0.0693749984493479,0.455947271603313)
--(axis cs:0.0712499984074384,0.457936324876151)
--(axis cs:0.0731249983655289,0.459758101681661)
--(axis cs:0.0731249983655289,0.531010585830433)
--(axis cs:0.0731249983655289,0.531010585830433)
--(axis cs:0.0712499984074384,0.529213091286003)
--(axis cs:0.0693749984493479,0.527306959496213)
--(axis cs:0.0674999984912574,0.525269641013705)
--(axis cs:0.0656249985331669,0.523073621225886)
--(axis cs:0.0637499985750765,0.520718964308791)
--(axis cs:0.061874998616986,0.51832670763358)
--(axis cs:0.0599999986588955,0.51601151724239)
--(axis cs:0.058124998700805,0.513819501844797)
--(axis cs:0.0562499987427145,0.511618501072789)
--(axis cs:0.054374998784624,0.509336496679038)
--(axis cs:0.0524999988265336,0.506909567254102)
--(axis cs:0.0506249988684431,0.504237280426706)
--(axis cs:0.0487499989103526,0.501272665257261)
--(axis cs:0.0468749989522621,0.498086043918768)
--(axis cs:0.0449999989941716,0.494759610080264)
--(axis cs:0.0431249990360811,0.491254702194686)
--(axis cs:0.0412499990779907,0.487655851538596)
--(axis cs:0.0393749991199002,0.483947944470614)
--(axis cs:0.0374999991618097,0.480127945177385)
--(axis cs:0.0356249992037192,0.476048111458795)
--(axis cs:0.0337499992456287,0.471695563026587)
--(axis cs:0.0318749992875382,0.467160454267312)
--(axis cs:0.0299999993294477,0.462623765795768)
--(axis cs:0.0281249993713573,0.457876112381823)
--(axis cs:0.0262499994132668,0.453198691698332)
--(axis cs:0.0243749994551763,0.448520028145378)
--(axis cs:0.0224999994970858,0.443587264911232)
--(axis cs:0.0206249995389953,0.437967936147307)
--(axis cs:0.0187499995809048,0.431224243438415)
--(axis cs:0.0168749996228144,0.423152576787881)
--(axis cs:0.0149999996647239,0.413234024557788)
--(axis cs:0.0131249997066334,0.399866766466688)
--(axis cs:0.0112499997485429,0.384516966802067)
--(axis cs:0.00937499979045242,0.366280408742227)
--(axis cs:0.00749999983236194,0.343492654281299)
--(axis cs:0.00562499987427145,0.313434715046863)
--(axis cs:0.00374999991618097,0.272308633158595)
--(axis cs:0.00187499995809048,0.214541418636306)
--cycle;

\path [fill=green!50.1960784313725!black, fill opacity=0.4, ultra thick]
(axis cs:0.00187499995809048,0.139223652861534)
--(axis cs:0.00187499995809048,0.105741159496303)
--(axis cs:0.00374999991618097,0.130081037698578)
--(axis cs:0.00562499987427145,0.145344502749689)
--(axis cs:0.00749999983236194,0.155538276775949)
--(axis cs:0.00937499979045242,0.162851166227453)
--(axis cs:0.0112499997485429,0.16854483471046)
--(axis cs:0.0131249997066334,0.17323162891121)
--(axis cs:0.0149999996647239,0.17710652105921)
--(axis cs:0.0168749996228144,0.179192809077768)
--(axis cs:0.0187499995809048,0.180742702540436)
--(axis cs:0.0206249995389953,0.182042745454178)
--(axis cs:0.0224999994970858,0.183330904036916)
--(axis cs:0.0243749994551763,0.185059589750292)
--(axis cs:0.0262499994132668,0.18762430784414)
--(axis cs:0.0281249993713573,0.191170815435446)
--(axis cs:0.0299999993294477,0.19535752526746)
--(axis cs:0.0318749992875382,0.200197318555072)
--(axis cs:0.0337499992456287,0.205232080108991)
--(axis cs:0.0356249992037192,0.20991473089874)
--(axis cs:0.0374999991618097,0.213931126117727)
--(axis cs:0.0393749991199002,0.217303303752117)
--(axis cs:0.0412499990779907,0.220375086672446)
--(axis cs:0.0431249990360811,0.223513034823706)
--(axis cs:0.0449999989941716,0.226709565601887)
--(axis cs:0.0468749989522621,0.229841097745072)
--(axis cs:0.0487499989103526,0.23264512668181)
--(axis cs:0.0506249988684431,0.235163623049129)
--(axis cs:0.0524999988265336,0.237790583013786)
--(axis cs:0.054374998784624,0.240892445845379)
--(axis cs:0.0562499987427145,0.24437878226566)
--(axis cs:0.058124998700805,0.247946664915851)
--(axis cs:0.0599999986588955,0.251236190330465)
--(axis cs:0.061874998616986,0.254082495381524)
--(axis cs:0.0637499985750765,0.256574401815768)
--(axis cs:0.0656249985331669,0.259223628749858)
--(axis cs:0.0674999984912574,0.262275033318818)
--(axis cs:0.0693749984493479,0.265598345626652)
--(axis cs:0.0712499984074384,0.26876608361511)
--(axis cs:0.0731249983655289,0.271321338504818)
--(axis cs:0.0731249983655289,0.327037261321266)
--(axis cs:0.0731249983655289,0.327037261321266)
--(axis cs:0.0712499984074384,0.324144004961088)
--(axis cs:0.0693749984493479,0.320903415497655)
--(axis cs:0.0674999984912574,0.317652840440192)
--(axis cs:0.0656249985331669,0.314767869357176)
--(axis cs:0.0637499985750765,0.312341667669991)
--(axis cs:0.061874998616986,0.310126103779903)
--(axis cs:0.0599999986588955,0.307741916582576)
--(axis cs:0.058124998700805,0.305010713663764)
--(axis cs:0.0562499987427145,0.302126260144018)
--(axis cs:0.054374998784624,0.29944380865218)
--(axis cs:0.0524999988265336,0.297301963275048)
--(axis cs:0.0506249988684431,0.295602584773287)
--(axis cs:0.0487499989103526,0.293733062814552)
--(axis cs:0.0468749989522621,0.291290218401913)
--(axis cs:0.0449999989941716,0.288283273457827)
--(axis cs:0.0431249990360811,0.284950308630874)
--(axis cs:0.0412499990779907,0.28149293622296)
--(axis cs:0.0393749991199002,0.277974996359727)
--(axis cs:0.0374999991618097,0.274133549937828)
--(axis cs:0.0356249992037192,0.269673038143413)
--(axis cs:0.0337499992456287,0.264654724215236)
--(axis cs:0.0318749992875382,0.259418435072314)
--(axis cs:0.0299999993294477,0.25433494525116)
--(axis cs:0.0281249993713573,0.249593491941907)
--(axis cs:0.0262499994132668,0.245551320257324)
--(axis cs:0.0243749994551763,0.242392477243696)
--(axis cs:0.0224999994970858,0.239940114478288)
--(axis cs:0.0206249995389953,0.237501059915317)
--(axis cs:0.0187499995809048,0.234658085927116)
--(axis cs:0.0168749996228144,0.231387851935076)
--(axis cs:0.0149999996647239,0.227544491887659)
--(axis cs:0.0131249997066334,0.221702686322528)
--(axis cs:0.0112499997485429,0.215498548701432)
--(axis cs:0.00937499979045242,0.208935629761116)
--(axis cs:0.00749999983236194,0.201164197886453)
--(axis cs:0.00562499987427145,0.18970785286867)
--(axis cs:0.00374999991618097,0.17097152676592)
--(axis cs:0.00187499995809048,0.139223652861534)
--cycle;

\path [fill=color0, fill opacity=0.4, ultra thick]
(axis cs:0.00187499995809048,0.117463438879036)
--(axis cs:0.00187499995809048,0.0912719625240553)
--(axis cs:0.00374999991618097,0.113974005292587)
--(axis cs:0.00562499987427145,0.126456958104897)
--(axis cs:0.00749999983236194,0.134376362646999)
--(axis cs:0.00937499979045242,0.139649923252697)
--(axis cs:0.0112499997485429,0.143570466878104)
--(axis cs:0.0131249997066334,0.14692980482776)
--(axis cs:0.0149999996647239,0.149992049360603)
--(axis cs:0.0168749996228144,0.152569900447804)
--(axis cs:0.0187499995809048,0.155193620709437)
--(axis cs:0.0206249995389953,0.157404737589173)
--(axis cs:0.0224999994970858,0.15904492845752)
--(axis cs:0.0243749994551763,0.160577645881319)
--(axis cs:0.0262499994132668,0.162770347610003)
--(axis cs:0.0281249993713573,0.165986073421327)
--(axis cs:0.0299999993294477,0.169972610874701)
--(axis cs:0.0318749992875382,0.174787893912113)
--(axis cs:0.0337499992456287,0.179844558135913)
--(axis cs:0.0356249992037192,0.184497631220257)
--(axis cs:0.0374999991618097,0.188472614381626)
--(axis cs:0.0393749991199002,0.191930809201438)
--(axis cs:0.0412499990779907,0.195221413537243)
--(axis cs:0.0431249990360811,0.198535490173261)
--(axis cs:0.0449999989941716,0.201646595313717)
--(axis cs:0.0468749989522621,0.204421541246067)
--(axis cs:0.0487499989103526,0.206635196416506)
--(axis cs:0.0506249988684431,0.208624619831706)
--(axis cs:0.0524999988265336,0.211077499334522)
--(axis cs:0.054374998784624,0.214279868504342)
--(axis cs:0.0562499987427145,0.21790023147521)
--(axis cs:0.058124998700805,0.221502920183717)
--(axis cs:0.0599999986588955,0.224698767143723)
--(axis cs:0.061874998616986,0.227365984709238)
--(axis cs:0.0637499985750765,0.229800577682563)
--(axis cs:0.0656249985331669,0.232709447289886)
--(axis cs:0.0674999984912574,0.236307066992831)
--(axis cs:0.0693749984493479,0.240244046008091)
--(axis cs:0.0712499984074384,0.243962185196731)
--(axis cs:0.0731249983655289,0.246882484426964)
--(axis cs:0.0731249983655289,0.282463641182809)
--(axis cs:0.0731249983655289,0.282463641182809)
--(axis cs:0.0712499984074384,0.27993067975894)
--(axis cs:0.0693749984493479,0.276753552462606)
--(axis cs:0.0674999984912574,0.273378836622982)
--(axis cs:0.0656249985331669,0.270310353610835)
--(axis cs:0.0637499985750765,0.267897293959115)
--(axis cs:0.061874998616986,0.266007466769658)
--(axis cs:0.0599999986588955,0.264001024058852)
--(axis cs:0.058124998700805,0.261471338385212)
--(axis cs:0.0562499987427145,0.258527813714269)
--(axis cs:0.054374998784624,0.255592067583558)
--(axis cs:0.0524999988265336,0.253133966377224)
--(axis cs:0.0506249988684431,0.251335330752219)
--(axis cs:0.0487499989103526,0.249766818085744)
--(axis cs:0.0468749989522621,0.247874916102284)
--(axis cs:0.0449999989941716,0.245406628222752)
--(axis cs:0.0431249990360811,0.24259799748098)
--(axis cs:0.0412499990779907,0.239590833706201)
--(axis cs:0.0393749991199002,0.236640348914503)
--(axis cs:0.0374999991618097,0.233622114574902)
--(axis cs:0.0356249992037192,0.230256881082203)
--(axis cs:0.0337499992456287,0.226397797422095)
--(axis cs:0.0318749992875382,0.222264566381443)
--(axis cs:0.0299999993294477,0.218287332357348)
--(axis cs:0.0281249993713573,0.214733950275605)
--(axis cs:0.0262499994132668,0.212118548550569)
--(axis cs:0.0243749994551763,0.210731919357376)
--(axis cs:0.0224999994970858,0.210172821623505)
--(axis cs:0.0206249995389953,0.209504963358523)
--(axis cs:0.0187499995809048,0.207966222939919)
--(axis cs:0.0168749996228144,0.205569037212601)
--(axis cs:0.0149999996647239,0.202258655362648)
--(axis cs:0.0131249997066334,0.196733665161906)
--(axis cs:0.0112499997485429,0.190600388473145)
--(axis cs:0.00937499979045242,0.183650578860782)
--(axis cs:0.00749999983236194,0.175254160782464)
--(axis cs:0.00562499987427145,0.163919504748079)
--(axis cs:0.00374999991618097,0.146870469800431)
--(axis cs:0.00187499995809048,0.117463438879036)
--cycle;

\path [fill=white!50.1960784313725!black, fill opacity=0.4, ultra thick]
(axis cs:0.00187499995809048,0.117603619176082)
--(axis cs:0.00187499995809048,0.0888441738299863)
--(axis cs:0.00374999991618097,0.11137469706396)
--(axis cs:0.00562499987427145,0.123780651602935)
--(axis cs:0.00749999983236194,0.131747545180364)
--(axis cs:0.00937499979045242,0.137328273856982)
--(axis cs:0.0112499997485429,0.141557728839315)
--(axis cs:0.0131249997066334,0.145191110209191)
--(axis cs:0.0149999996647239,0.148601741457914)
--(axis cs:0.0168749996228144,0.151641514377504)
--(axis cs:0.0187499995809048,0.154778988535269)
--(axis cs:0.0206249995389953,0.157511837005123)
--(axis cs:0.0224999994970858,0.15963717738536)
--(axis cs:0.0243749994551763,0.161476834422451)
--(axis cs:0.0262499994132668,0.163769501583791)
--(axis cs:0.0281249993713573,0.166942267589799)
--(axis cs:0.0299999993294477,0.170762495499165)
--(axis cs:0.0318749992875382,0.175384745806747)
--(axis cs:0.0337499992456287,0.180229647992369)
--(axis cs:0.0356249992037192,0.184684989126684)
--(axis cs:0.0374999991618097,0.188495082444062)
--(axis cs:0.0393749991199002,0.191838485302774)
--(axis cs:0.0412499990779907,0.195097590847782)
--(axis cs:0.0431249990360811,0.198361967564248)
--(axis cs:0.0449999989941716,0.201384174581453)
--(axis cs:0.0468749989522621,0.204059307945596)
--(axis cs:0.0487499989103526,0.206216849448362)
--(axis cs:0.0506249988684431,0.208184822026091)
--(axis cs:0.0524999988265336,0.210663466691116)
--(axis cs:0.054374998784624,0.213854682628959)
--(axis cs:0.0562499987427145,0.217381772425103)
--(axis cs:0.058124998700805,0.220810076721044)
--(axis cs:0.0599999986588955,0.223743002878156)
--(axis cs:0.061874998616986,0.226132402915462)
--(axis cs:0.0637499985750765,0.228378979529105)
--(axis cs:0.0656249985331669,0.23121383084439)
--(axis cs:0.0674999984912574,0.234711256629856)
--(axis cs:0.0693749984493479,0.238442252490448)
--(axis cs:0.0712499984074384,0.241875778707065)
--(axis cs:0.0731249983655289,0.24446312947722)
--(axis cs:0.0731249983655289,0.281672105413093)
--(axis cs:0.0731249983655289,0.281672105413093)
--(axis cs:0.0712499984074384,0.278987435559975)
--(axis cs:0.0693749984493479,0.275733615839314)
--(axis cs:0.0674999984912574,0.272356431467571)
--(axis cs:0.0656249985331669,0.269324097082861)
--(axis cs:0.0637499985750765,0.266926629429727)
--(axis cs:0.061874998616986,0.264977610749758)
--(axis cs:0.0599999986588955,0.262791811651001)
--(axis cs:0.058124998700805,0.260098198197488)
--(axis cs:0.0562499987427145,0.257039281191368)
--(axis cs:0.054374998784624,0.254000338592551)
--(axis cs:0.0524999988265336,0.25145098051572)
--(axis cs:0.0506249988684431,0.249482763107709)
--(axis cs:0.0487499989103526,0.247715881087006)
--(axis cs:0.0468749989522621,0.245619917228538)
--(axis cs:0.0449999989941716,0.242986635613337)
--(axis cs:0.0431249990360811,0.240025822840973)
--(axis cs:0.0412499990779907,0.236915183477949)
--(axis cs:0.0393749991199002,0.233907749917004)
--(axis cs:0.0374999991618097,0.230888977148963)
--(axis cs:0.0356249992037192,0.227593341939591)
--(axis cs:0.0337499992456287,0.223821108825077)
--(axis cs:0.0318749992875382,0.219775673376735)
--(axis cs:0.0299999993294477,0.21591848966033)
--(axis cs:0.0281249993713573,0.212530340667989)
--(axis cs:0.0262499994132668,0.210113049145438)
--(axis cs:0.0243749994551763,0.20886632358114)
--(axis cs:0.0224999994970858,0.208346137249713)
--(axis cs:0.0206249995389953,0.207610912135445)
--(axis cs:0.0187499995809048,0.206043567551835)
--(axis cs:0.0168749996228144,0.20377580072798)
--(axis cs:0.0149999996647239,0.200675237237315)
--(axis cs:0.0131249997066334,0.195232168191872)
--(axis cs:0.0112499997485429,0.18925342768493)
--(axis cs:0.00937499979045242,0.182536833705559)
--(axis cs:0.00749999983236194,0.174442184109951)
--(axis cs:0.00562499987427145,0.163246432102678)
--(axis cs:0.00374999991618097,0.146761480506058)
--(axis cs:0.00187499995809048,0.117603619176082)
--cycle;

\addplot [ultra thick, red]
table {%
0.00187504291534424 0.205489858984947
0.00374996662139893 0.260595411062241
0.00562500953674316 0.299410372972488
0.0075000524520874 0.327237814664841
0.00937497615814209 0.347861796617508
0.0112500190734863 0.363974869251251
0.013124942779541 0.377310812473297
0.0149999856948853 0.388793766498566
0.0168750286102295 0.397246927022934
0.0187499523162842 0.404069930315018
0.0206249952316284 0.409708887338638
0.0225000381469727 0.414358913898468
0.0243749618530273 0.41841322183609
0.0262500047683716 0.422340005636215
0.0281250476837158 0.426409184932709
0.0299999713897705 0.430683642625809
0.033750057220459 0.438706308603287
0.0356249809265137 0.442569702863693
0.0375000238418579 0.446205765008926
0.0393749475479126 0.449620366096497
0.0412499904632568 0.452890127897263
0.0431250333786011 0.456023305654526
0.0449999570846558 0.459054529666901
0.046875 0.461891323328018
0.0487500429153442 0.464646816253662
0.0506249666213989 0.467291325330734
0.0525000095367432 0.46982130408287
0.0562499761581421 0.474746555089951
0.059999942779541 0.479705661535263
0.0637500286102295 0.484851896762848
0.0656249523162842 0.487336844205856
0.0674999952316284 0.489614903926849
0.0693750381469727 0.491699069738388
0.0712499618530273 0.493628531694412
0.0731250047683716 0.495427817106247
};
\addplot [ultra thick, blue]
table {%
0.00187504291534424 0.200211375951767
0.00374996662139893 0.254200369119644
0.00562500953674316 0.292305201292038
0.0075000524520874 0.319772034883499
0.00937497615814209 0.340210765600204
0.0112500190734863 0.356271773576736
0.013124942779541 0.369606405496597
0.0149999856948853 0.381115585565567
0.0168750286102295 0.389798879623413
0.0187499523162842 0.396956771612167
0.0206249952316284 0.402953237295151
0.0225000381469727 0.407966554164886
0.0243749618530273 0.412404745817184
0.0262500047683716 0.416727632284164
0.0281250476837158 0.42118564248085
0.0299999713897705 0.425817579030991
0.033750057220459 0.434909731149673
0.0356249809265137 0.439307391643524
0.0375000238418579 0.443422228097916
0.0393749475479126 0.447246462106705
0.0412499904632568 0.450904130935669
0.0431250333786011 0.454416155815125
0.0449999570846558 0.457816064357758
0.046875 0.461041390895844
0.0487500429153442 0.464151591062546
0.0506249666213989 0.467075377702713
0.0525000095367432 0.469775140285492
0.0543750524520874 0.472304672002792
0.0562499761581421 0.474752008914948
0.059999942779541 0.479542940855026
0.0618749856948853 0.482062995433807
0.0637500286102295 0.484653502702713
0.0656249523162842 0.487176477909088
0.0674999952316284 0.4895079433918
0.0693750381469727 0.491627126932144
0.0712499618530273 0.493574768304825
0.0731250047683716 0.495384305715561
};
\addplot [ultra thick, green!50.1960784313725!black]
table {%
0.00187504291534424 0.122482411563396
0.00374996662139893 0.150526270270348
0.00562500953674316 0.167526185512543
0.0075000524520874 0.178351238369942
0.00937497615814209 0.185893401503563
0.0112500190734863 0.192021667957306
0.013124942779541 0.197467178106308
0.0149999856948853 0.202325522899628
0.0168750286102295 0.205290332436562
0.0187499523162842 0.207700431346893
0.0206249952316284 0.209771901369095
0.0225000381469727 0.211635529994965
0.0243749618530273 0.213725998997688
0.0262500047683716 0.216587796807289
0.0281250476837158 0.220382124185562
0.0299999713897705 0.224846199154854
0.0318750143051147 0.229807838797569
0.033750057220459 0.234943449497223
0.0356249809265137 0.239793881773949
0.0375000238418579 0.244032323360443
0.0393749475479126 0.247639164328575
0.0412499904632568 0.25093400478363
0.0431250333786011 0.254231631755829
0.0449999570846558 0.257496386766434
0.046875 0.260565638542175
0.0487500429153442 0.263189047574997
0.0506249666213989 0.265383064746857
0.0525000095367432 0.26754629611969
0.0543750524520874 0.270168095827103
0.0562499761581421 0.273252546787262
0.0581250190734863 0.27647864818573
0.059999942779541 0.279489040374756
0.0618749856948853 0.282104253768921
0.0637500286102295 0.284458041191101
0.0656249523162842 0.286995768547058
0.0674999952316284 0.289963901042938
0.0693750381469727 0.293250918388367
0.0712499618530273 0.296455055475235
0.0731250047683716 0.299179285764694
};
\addplot [ultra thick, color0]
table {%
0.00187504291534424 0.104367703199387
0.00374996662139893 0.130422249436378
0.00562500953674316 0.145188227295876
0.0075000524520874 0.15481524169445
0.00937497615814209 0.161650270223618
0.0112500190734863 0.167085409164429
0.013124942779541 0.171831727027893
0.0149999856948853 0.176125332713127
0.0168750286102295 0.179069444537163
0.0187499523162842 0.181579902768135
0.0206249952316284 0.183454841375351
0.0225000381469727 0.184608846902847
0.0243749618530273 0.185654759407043
0.0262500047683716 0.187444448471069
0.0281250476837158 0.190360009670258
0.0299999713897705 0.19412998855114
0.0318750143051147 0.198526248335838
0.033750057220459 0.203121185302734
0.0356249809265137 0.207377254962921
0.0375000238418579 0.211047351360321
0.0393749475479126 0.214285582304001
0.0431250333786011 0.220566764473915
0.0449999570846558 0.223526611924171
0.046875 0.226148262619972
0.0487500429153442 0.228201031684875
0.0506249666213989 0.229979991912842
0.0525000095367432 0.232105776667595
0.0543750524520874 0.234935969114304
0.0562499761581421 0.238214015960693
0.0581250190734863 0.24148716032505
0.059999942779541 0.244349896907806
0.0618749856948853 0.246686711907387
0.0637500286102295 0.248848930001259
0.0656249523162842 0.251509934663773
0.0674999952316284 0.254842966794968
0.0693750381469727 0.258498817682266
0.0712499618530273 0.261946380138397
0.0731250047683716 0.26467302441597
};
\addplot [ultra thick, white!40.1960784313725!black]
table {%
0.00187504291534424 0.103223890066147
0.00374996662139893 0.129068076610565
0.00562500953674316 0.143513545393944
0.0075000524520874 0.153094857931137
0.00937497615814209 0.159932538866997
0.0112500190734863 0.165405601263046
0.013124942779541 0.170211628079414
0.0149999856948853 0.174638524651527
0.0168750286102295 0.177708685398102
0.0187499523162842 0.180411294102669
0.0206249952316284 0.182561337947845
0.0225000381469727 0.183991670608521
0.0243749618530273 0.185171574354172
0.0262500047683716 0.186941251158714
0.0281250476837158 0.189736306667328
0.0299999713897705 0.193340495228767
0.0318750143051147 0.197580218315125
0.033750057220459 0.202025398612022
0.0356249809265137 0.206139206886292
0.0375000238418579 0.209692046046257
0.0393749475479126 0.212873116135597
0.0431250333786011 0.219193875789642
0.0449999570846558 0.222185358405113
0.046875 0.224839597940445
0.0487500429153442 0.226966395974159
0.0506249666213989 0.228833809494972
0.0525000095367432 0.231057241559029
0.0543750524520874 0.233927488327026
0.0562499761581421 0.237210541963577
0.0581250190734863 0.240454122424126
0.059999942779541 0.243267357349396
0.0618749856948853 0.245555058121681
0.0637500286102295 0.247652754187584
0.0656249523162842 0.250268965959549
0.0674999952316284 0.253533840179443
0.0693750381469727 0.257087886333466
0.0712499618530273 0.26043164730072
0.0731250047683716 0.263067573308945
};
