# Supplementary material for: Neural Networks with Physics-Informed Architectures and Constraints for Dynamical Systems Modeling
Source: arXiv:2109.06407 source file (2022-12-12)
Supplement: Supplementary file 19 [file train_test_loss_data.tex]

\path [fill=red, fill opacity=0.4, ultra thick]
(axis cs:0,0.157891631126404)
--(axis cs:0,0.156707122921944)
--(axis cs:100,0.152500689029694)
--(axis cs:200,0.147555321455002)
--(axis cs:300,0.142711475491524)
--(axis cs:400,0.13894097507)
--(axis cs:500,0.136075586080551)
--(axis cs:600,0.133588179945946)
--(axis cs:700,0.13145424425602)
--(axis cs:800,0.130239441990852)
--(axis cs:900,0.129831120371819)
--(axis cs:1000,0.129790559411049)
--(axis cs:1100,0.129808112978935)
--(axis cs:1200,0.130750745534897)
--(axis cs:1300,0.131993338465691)
--(axis cs:1400,0.133178263902664)
--(axis cs:1500,0.13405454158783)
--(axis cs:1600,0.135351493954659)
--(axis cs:1700,0.136895939707756)
--(axis cs:1800,0.138367012143135)
--(axis cs:1800,0.140710845589638)
--(axis cs:1800,0.140710845589638)
--(axis cs:1700,0.1396644115448)
--(axis cs:1600,0.137976124882698)
--(axis cs:1500,0.136463105678558)
--(axis cs:1400,0.134592816233635)
--(axis cs:1300,0.133277282118797)
--(axis cs:1200,0.131870120763779)
--(axis cs:1100,0.131040781736374)
--(axis cs:1000,0.1307003647089)
--(axis cs:900,0.130977004766464)
--(axis cs:800,0.131350114941597)
--(axis cs:700,0.132590159773827)
--(axis cs:600,0.134512767195702)
--(axis cs:500,0.136909961700439)
--(axis cs:400,0.139808893203735)
--(axis cs:300,0.143705025315285)
--(axis cs:200,0.14826825261116)
--(axis cs:100,0.153138846158981)
--(axis cs:0,0.157891631126404)
--cycle;

\path [fill=blue, fill opacity=0.4, ultra thick]
(axis cs:0,0.16883285343647)
--(axis cs:0,0.168774530291557)
--(axis cs:100,0.166224166750908)
--(axis cs:200,0.163298755884171)
--(axis cs:300,0.160059332847595)
--(axis cs:400,0.15654131770134)
--(axis cs:500,0.152967691421509)
--(axis cs:600,0.149806439876556)
--(axis cs:700,0.147015690803528)
--(axis cs:800,0.14439769089222)
--(axis cs:900,0.141728043556213)
--(axis cs:1000,0.139089226722717)
--(axis cs:1100,0.136542022228241)
--(axis cs:1200,0.134253308176994)
--(axis cs:1300,0.13244840502739)
--(axis cs:1400,0.130785629153252)
--(axis cs:1500,0.129413813352585)
--(axis cs:1600,0.128441333770752)
--(axis cs:1700,0.12728314101696)
--(axis cs:1800,0.126819714903831)
--(axis cs:1900,0.126506358385086)
--(axis cs:2000,0.126513361930847)
--(axis cs:2100,0.126674488186836)
--(axis cs:2200,0.126767784357071)
--(axis cs:2300,0.126931846141815)
--(axis cs:2400,0.12742093205452)
--(axis cs:2500,0.128065273165703)
--(axis cs:2600,0.128324285149574)
--(axis cs:2700,0.129224315285683)
--(axis cs:2800,0.129832699894905)
--(axis cs:2900,0.130365759134293)
--(axis cs:3000,0.130714654922485)
--(axis cs:3100,0.131480172276497)
--(axis cs:3200,0.132055059075356)
--(axis cs:3200,0.137156561017036)
--(axis cs:3200,0.137156561017036)
--(axis cs:3100,0.136083915829659)
--(axis cs:3000,0.134891837835312)
--(axis cs:2900,0.133804440498352)
--(axis cs:2800,0.132485538721085)
--(axis cs:2700,0.131375342607498)
--(axis cs:2600,0.130737736821175)
--(axis cs:2500,0.129947856068611)
--(axis cs:2400,0.128819033503532)
--(axis cs:2300,0.128465577960014)
--(axis cs:2200,0.128268837928772)
--(axis cs:2100,0.127889558672905)
--(axis cs:2000,0.12802392244339)
--(axis cs:1900,0.127600520849228)
--(axis cs:1800,0.127773091197014)
--(axis cs:1700,0.128536894917488)
--(axis cs:1600,0.129573613405228)
--(axis cs:1500,0.130521804094315)
--(axis cs:1400,0.131793335080147)
--(axis cs:1300,0.133387237787247)
--(axis cs:1200,0.135041922330856)
--(axis cs:1100,0.137195900082588)
--(axis cs:1000,0.139632970094681)
--(axis cs:900,0.142248421907425)
--(axis cs:800,0.144854798913002)
--(axis cs:700,0.147579938173294)
--(axis cs:600,0.150275200605392)
--(axis cs:500,0.153362989425659)
--(axis cs:400,0.156814098358154)
--(axis cs:300,0.160316914319992)
--(axis cs:200,0.163508355617523)
--(axis cs:100,0.16631506383419)
--(axis cs:0,0.16883285343647)
--cycle;

\path [fill=green!50.1960784313725!black, fill opacity=0.4, ultra thick]
(axis cs:0,0.115993812680244)
--(axis cs:0,0.115573808550835)
--(axis cs:100,0.108277775347233)
--(axis cs:200,0.101100146770477)
--(axis cs:300,0.0948384553194046)
--(axis cs:400,0.0887349992990494)
--(axis cs:500,0.0835918784141541)
--(axis cs:600,0.0803125351667404)
--(axis cs:700,0.0779219642281532)
--(axis cs:800,0.0763957276940346)
--(axis cs:900,0.0757012367248535)
--(axis cs:1000,0.0756266117095947)
--(axis cs:1100,0.0761700719594955)
--(axis cs:1200,0.0771142095327377)
--(axis cs:1300,0.0775865316390991)
--(axis cs:1400,0.0780411511659622)
--(axis cs:1500,0.0787514299154282)
--(axis cs:1600,0.0792547017335892)
--(axis cs:1600,0.0813008844852448)
--(axis cs:1600,0.0813008844852448)
--(axis cs:1500,0.0810655206441879)
--(axis cs:1400,0.0807349681854248)
--(axis cs:1300,0.0793756246566772)
--(axis cs:1200,0.0779962241649628)
--(axis cs:1100,0.0770085155963898)
--(axis cs:1000,0.0768293887376785)
--(axis cs:900,0.0770425051450729)
--(axis cs:800,0.0773364081978798)
--(axis cs:700,0.0786337628960609)
--(axis cs:600,0.0811715871095657)
--(axis cs:500,0.0843863561749458)
--(axis cs:400,0.0890617370605469)
--(axis cs:300,0.0950746387243271)
--(axis cs:200,0.101643040776253)
--(axis cs:100,0.108931817114353)
--(axis cs:0,0.115993812680244)
--cycle;

\path [fill=color0, fill opacity=0.4, ultra thick]
(axis cs:0,0.0974255204200745)
--(axis cs:0,0.0967491120100021)
--(axis cs:100,0.0878203138709068)
--(axis cs:200,0.0793911516666412)
--(axis cs:300,0.0724547430872917)
--(axis cs:400,0.0675220042467117)
--(axis cs:500,0.0640111118555069)
--(axis cs:600,0.0615299679338932)
--(axis cs:700,0.0598497688770294)
--(axis cs:800,0.0589690469205379)
--(axis cs:900,0.0585705898702145)
--(axis cs:1000,0.058612909168005)
--(axis cs:1100,0.0590603426098824)
--(axis cs:1200,0.0596427395939827)
--(axis cs:1300,0.0601931884884834)
--(axis cs:1400,0.0610491149127483)
--(axis cs:1500,0.0618468336760998)
--(axis cs:1600,0.0621525123715401)
--(axis cs:1600,0.063120000064373)
--(axis cs:1600,0.063120000064373)
--(axis cs:1500,0.062134362757206)
--(axis cs:1400,0.0614040978252888)
--(axis cs:1300,0.0610441267490387)
--(axis cs:1200,0.0601691231131554)
--(axis cs:1100,0.0597608983516693)
--(axis cs:1000,0.0595056377351284)
--(axis cs:900,0.0595943070948124)
--(axis cs:800,0.0598804466426373)
--(axis cs:700,0.0609363839030266)
--(axis cs:600,0.0625469014048576)
--(axis cs:500,0.0650931745767593)
--(axis cs:400,0.0685819536447525)
--(axis cs:300,0.0733053311705589)
--(axis cs:200,0.0803433060646057)
--(axis cs:100,0.0886920019984245)
--(axis cs:0,0.0974255204200745)
--cycle;

\path [fill=white!40.1960784313725!black, fill opacity=0.4, ultra thick]
(axis cs:0,0.0974728986620903)
--(axis cs:0,0.0966551229357719)
--(axis cs:100,0.087830938398838)
--(axis cs:200,0.079444631934166)
--(axis cs:300,0.0724884644150734)
--(axis cs:400,0.0676380023360252)
--(axis cs:500,0.0641438663005829)
--(axis cs:600,0.0616008266806602)
--(axis cs:700,0.0600851774215698)
--(axis cs:800,0.0592496693134308)
--(axis cs:900,0.0586629025638103)
--(axis cs:1000,0.0587406978011131)
--(axis cs:1100,0.0591305866837502)
--(axis cs:1200,0.0600960850715637)
--(axis cs:1300,0.0608675964176655)
--(axis cs:1400,0.0614956505596638)
--(axis cs:1500,0.0622464530169964)
--(axis cs:1600,0.0631800815463066)
--(axis cs:1600,0.0636094138026237)
--(axis cs:1600,0.0636094138026237)
--(axis cs:1500,0.0632269307971001)
--(axis cs:1400,0.0628291890025139)
--(axis cs:1300,0.0619762763381004)
--(axis cs:1200,0.0609938502311707)
--(axis cs:1100,0.0602083057165146)
--(axis cs:1000,0.0598639845848083)
--(axis cs:900,0.0598933361470699)
--(axis cs:800,0.060356643050909)
--(axis cs:700,0.061256542801857)
--(axis cs:600,0.0628817081451416)
--(axis cs:500,0.0653250515460968)
--(axis cs:400,0.0686143413186073)
--(axis cs:300,0.0734104439616203)
--(axis cs:200,0.0804402083158493)
--(axis cs:100,0.0887273177504539)
--(axis cs:0,0.0974728986620903)
--cycle;

\addplot [ultra thick, red  ]
table {%
0 0.157305002212524
100 0.152832016348839
200 0.147967681288719
300 0.143208265304565
400 0.139409884810448
500 0.136492773890495
600 0.134050458669662
700 0.132003650069237
800 0.130794763565063
900 0.13043338060379
1000 0.130187004804611
1100 0.130454942584038
1200 0.131313025951385
1400 0.133978575468063
1500 0.135258823633194
1600 0.136663794517517
1700 0.138177812099457
1800 0.139382258057594
};
\addlegendentry{Baseline}
\addplot [ultra thick, blue  ]
table {%
0 0.168808653950691
100 0.166276067495346
200 0.163403555750847
300 0.160191714763641
400 0.156698480248451
500 0.153174802660942
600 0.150040820240974
1000 0.139361098408699
1100 0.136889770627022
1200 0.134687200188637
1300 0.13292770087719
1400 0.131289467215538
1500 0.12996780872345
1600 0.129007488489151
1700 0.127900809049606
1800 0.127296417951584
1900 0.127019703388214
2100 0.127282023429871
2200 0.127518326044083
2300 0.127727806568146
2400 0.128180429339409
2500 0.129006564617157
2600 0.129530996084213
2700 0.130361154675484
2800 0.131262004375458
2900 0.132085114717484
3000 0.132803231477737
3100 0.133782044053078
3200 0.134605824947357
};
\addlegendentry{K1}
\addplot [ultra thick, green!39.2156862745098!black,  ]
table {%
0 0.11578381806612
100 0.108604818582535
200 0.101371616125107
300 0.0949505195021629
400 0.0889095664024353
500 0.0839678272604942
600 0.0807565152645111
700 0.0783044919371605
800 0.0768660679459572
900 0.0763718634843826
1000 0.0762280002236366
1100 0.0765892863273621
1200 0.0775552168488503
1300 0.0784810706973076
1400 0.0793880671262741
1500 0.0798000916838646
1600 0.0802777856588364
};
\addlegendentry{K2}
\addplot [ultra thick, color0 ]
table {%
0 0.0970873087644577
100 0.0882561504840851
200 0.0798672139644623
300 0.0728800296783447
400 0.0680519640445709
500 0.0645295530557632
600 0.0620384365320206
700 0.060393076390028
800 0.0594247542321682
900 0.0590824522078037
1000 0.0590592809021473
1100 0.0594106130301952
1200 0.0599059388041496
1300 0.0606186650693417
1400 0.0612562485039234
1500 0.0620062239468098
1600 0.0626362562179565
};
\addlegendentry{K3}
\addplot [ultra thick, white!60.2745098039216!black,  ]
table {%
0 0.0970640182495117
100 0.0882791206240654
200 0.0799424275755882
300 0.0729494616389275
400 0.0681261643767357
500 0.0647266060113907
600 0.0622388310730457
700 0.0606431774795055
800 0.0597685612738132
900 0.0592781156301498
1000 0.0593023486435413
1100 0.059669453650713
1200 0.0605449639260769
1300 0.0614907294511795
1400 0.0621624104678631
1500 0.0627366900444031
1600 0.0633947402238846
};
\addlegendentry{K4}
