# Supplementary material for: Neural Networks with Physics-Informed Architectures and Constraints for Dynamical Systems Modeling
Source: arXiv:2109.06407 source file (2022-12-12)
Supplement: Supplementary file 20 [file traj_err_data.tex]

\path [fill=red, fill opacity=0.4, ultra thick]
(axis cs:1,0.541743363602843)
--(axis cs:1,0.449112071455718)
--(axis cs:10,0.222851933182839)
--(axis cs:25,0.218278809800564)
--(axis cs:75,0.203373653824151)
--(axis cs:200,0.202344693428683)
--(axis cs:500,0.205319745054706)
--(axis cs:500,0.24492664882946)
--(axis cs:500,0.24492664882946)
--(axis cs:200,0.239061668396655)
--(axis cs:75,0.260088453237498)
--(axis cs:25,0.255254397050033)
--(axis cs:10,0.273922619095674)
--(axis cs:1,0.541743363602843)
--cycle;

\path [fill=blue, fill opacity=0.4, ultra thick]
(axis cs:1,0.531010585830433)
--(axis cs:1,0.459758101681661)
--(axis cs:10,0.229730335009316)
--(axis cs:25,0.191273754876949)
--(axis cs:75,0.175796832901461)
--(axis cs:200,0.164071554922007)
--(axis cs:500,0.170048621804538)
--(axis cs:500,0.202470236594375)
--(axis cs:500,0.202470236594375)
--(axis cs:200,0.206555843340007)
--(axis cs:75,0.231836704110698)
--(axis cs:25,0.224161883102382)
--(axis cs:10,0.27300405791108)
--(axis cs:1,0.531010585830433)
--cycle;

\path [fill=green!50.1960784313725!black, fill opacity=0.4, ultra thick]
(axis cs:1,0.327037261321266)
--(axis cs:1,0.271321338504818)
--(axis cs:10,0.153216160419598)
--(axis cs:25,0.162110887475575)
--(axis cs:75,0.14101120413756)
--(axis cs:200,0.131378655409453)
--(axis cs:500,0.133331697770542)
--(axis cs:500,0.172200606977037)
--(axis cs:500,0.172200606977037)
--(axis cs:200,0.160043838253535)
--(axis cs:75,0.165050957437437)
--(axis cs:25,0.196078888437663)
--(axis cs:10,0.187416813983647)
--(axis cs:1,0.327037261321266)
--cycle;

\path [fill=color0, fill opacity=0.4, ultra thick]
(axis cs:1,0.282463641182809)
--(axis cs:1,0.246882484426964)
--(axis cs:10,0.161905684649898)
--(axis cs:25,0.148348927125901)
--(axis cs:75,0.129090951546991)
--(axis cs:200,0.124358420615673)
--(axis cs:500,0.122476188880835)
--(axis cs:500,0.152916463115796)
--(axis cs:500,0.152916463115796)
--(axis cs:200,0.18128134913412)
--(axis cs:75,0.160261962288737)
--(axis cs:25,0.189036696377846)
--(axis cs:10,0.189963946263115)
--(axis cs:1,0.282463641182809)
--cycle;

\path [fill=white!50.1960784313725!black, fill opacity=0.4, ultra thick]
(axis cs:1,0.281672105413093)
--(axis cs:1,0.24446312947722)
--(axis cs:10,0.162119355053934)
--(axis cs:25,0.159594768858239)
--(axis cs:75,0.166204760461526)
--(axis cs:200,0.145110190962717)
--(axis cs:500,0.162198415650703)
--(axis cs:500,0.630858549893925)
--(axis cs:500,0.630858549893925)
--(axis cs:200,0.175752334968792)
--(axis cs:75,0.194949935788108)
--(axis cs:25,0.191690811891073)
--(axis cs:10,0.202372520726317)
--(axis cs:1,0.281672105413093)
--cycle;

\addplot [ultra thick, red, mark=*, mark size=1.5, mark options={solid}]
table {%
1 0.495427817106247
10 0.248387262225151
25 0.236766636371613
75 0.231731072068214
200 0.220703214406967
500 0.22512324154377
};
\addplot [ultra thick, blue,  mark=*, mark size=1.5, mark options={solid}]
table {%
1 0.495384305715561
10 0.251367211341858
25 0.207717821002007
75 0.203816741704941
200 0.185313686728477
500 0.186259418725967
};
\addplot [ultra thick, green!50.1960784313725!black,  mark=*, mark size=1.5, mark options={solid}]
table {%
1 0.299179285764694
10 0.170316502451897
25 0.179094910621643
75 0.153031080961227
200 0.145711228251457
500 0.152766168117523
};
\addplot [ultra thick, color0,  mark=*, mark size=1.5, mark options={solid}]
table {%
1 0.26467302441597
10 0.175934821367264
25 0.168692797422409
75 0.144676461815834
200 0.152819901704788
500 0.137696325778961
};
\addplot [ultra thick, white!40.1960784313725!black,  mark=*, mark size=1.5, mark options={solid}]
table {%
1 0.263067573308945
10 0.182245910167694
25 0.175642788410187
75 0.180577367544174
200 0.160431265830994
500 0.160534837245941
};
