# Supplementary material for: Neural Networks with Physics-Informed Architectures and Constraints for Dynamical Systems Modeling
Source: arXiv:2109.06407 source file (2022-12-12)
Supplement: Supplementary file 21 [file train_test_loss_data.tex]

\path [fill=red, fill opacity=0.2, semithick]
(axis cs:0,0.00794493036430928)
--(axis cs:0,0.00792317748604364)
--(axis cs:100,0.0065848743385515)
--(axis cs:200,0.00505695469397237)
--(axis cs:300,0.00338619162290507)
--(axis cs:400,0.00178837855409415)
--(axis cs:500,0.000985278690901584)
--(axis cs:600,0.000611077999596422)
--(axis cs:700,0.000411842297425804)
--(axis cs:800,0.000362620296763487)
--(axis cs:900,0.00032752720172402)
--(axis cs:1000,0.000298620624552315)
--(axis cs:1100,0.000274931584658309)
--(axis cs:1200,0.000256637012007072)
--(axis cs:1300,0.000239079197735861)
--(axis cs:1400,0.000227048416274827)
--(axis cs:1500,0.000220975328405741)
--(axis cs:1600,0.000218077592382846)
--(axis cs:1700,0.000218268167210757)
--(axis cs:1800,0.000223572788044673)
--(axis cs:1900,0.000216262209326544)
--(axis cs:2000,0.000216134550285422)
--(axis cs:2100,0.000206434984208891)
--(axis cs:2200,0.000196638351471821)
--(axis cs:2300,0.000192853864107725)
--(axis cs:2400,0.000192488475725672)
--(axis cs:2500,0.000181977671597006)
--(axis cs:2600,0.000193789453890256)
--(axis cs:2700,0.000191861720970051)
--(axis cs:2800,0.000189198273112381)
--(axis cs:2900,0.000186987592602992)
--(axis cs:3000,0.000188927373928458)
--(axis cs:3100,0.000178195244880903)
--(axis cs:3200,0.000177978741144972)
--(axis cs:3300,0.000168760374247822)
--(axis cs:3400,0.000172218884219902)
--(axis cs:3500,0.000173278593058551)
--(axis cs:3600,0.000173642177965453)
--(axis cs:3700,0.000175903710590367)
--(axis cs:3800,0.000175616518978398)
--(axis cs:3900,0.000171243987413393)
--(axis cs:4000,0.000169711803702109)
--(axis cs:4100,0.000172825859043403)
--(axis cs:4200,0.00017236576936298)
--(axis cs:4300,0.000167693011248602)
--(axis cs:4400,0.000165745695194825)
--(axis cs:4500,0.000157824339609176)
--(axis cs:4600,0.000155564772431313)
--(axis cs:4700,0.000148252324687529)
--(axis cs:4800,0.000149367310081661)
--(axis cs:4900,0.000152981530923669)
--(axis cs:5000,0.000152889420849398)
--(axis cs:5100,0.000147283398922225)
--(axis cs:5200,0.000145814326850031)
--(axis cs:5300,0.000147103999147593)
--(axis cs:5400,0.00014019135093937)
--(axis cs:5500,0.000138729337938435)
--(axis cs:5600,0.000135316352496103)
--(axis cs:5700,0.000134348546188495)
--(axis cs:5800,0.000132778985794949)
--(axis cs:5900,0.000127986694617333)
--(axis cs:6000,0.000122391485642451)
--(axis cs:6100,0.000119164870861333)
--(axis cs:6200,0.00011835470386704)
--(axis cs:6300,0.000118808475676171)
--(axis cs:6400,0.000127250914921902)
--(axis cs:6500,0.000131158108964106)
--(axis cs:6600,0.000130498443353996)
--(axis cs:6700,0.000129413847596205)
--(axis cs:6800,0.000125474108149665)
--(axis cs:6900,0.000120387282425768)
--(axis cs:7000,0.000119421465560608)
--(axis cs:7100,0.000115416109527837)
--(axis cs:7200,0.00011377626160185)
--(axis cs:7300,0.000110506571396613)
--(axis cs:7400,0.000109320596650683)
--(axis cs:7500,0.000110172643009107)
--(axis cs:7600,0.000108654176890762)
--(axis cs:7700,0.000110822891665448)
--(axis cs:7800,0.000111526415500908)
--(axis cs:7900,0.000107629612079876)
--(axis cs:8000,0.000106519207011028)
--(axis cs:8100,0.000114105240695766)
--(axis cs:8200,0.00011192825895394)
--(axis cs:8300,0.000110275823562246)
--(axis cs:8400,0.00010731690121422)
--(axis cs:8500,0.000104498582287293)
--(axis cs:8600,0.000101130344683152)
--(axis cs:8700,9.7064374837615e-05)
--(axis cs:8800,9.55297146709891e-05)
--(axis cs:8900,9.49607405595845e-05)
--(axis cs:9000,9.60820538784582e-05)
--(axis cs:9100,9.53089628301208e-05)
--(axis cs:9200,9.67427625011389e-05)
--(axis cs:9300,9.72594501880651e-05)
--(axis cs:9400,9.68474497851896e-05)
--(axis cs:9500,9.65894041970606e-05)
--(axis cs:9600,9.21167071537533e-05)
--(axis cs:9700,9.26127978979672e-05)
--(axis cs:9800,9.19084957854828e-05)
--(axis cs:9900,9.12098430058818e-05)
--(axis cs:10000,9.03305944269132e-05)
--(axis cs:10100,9.28310957138549e-05)
--(axis cs:10200,9.29976050804488e-05)
--(axis cs:10300,9.49488040776608e-05)
--(axis cs:10400,9.47096782704783e-05)
--(axis cs:10500,9.61527941204935e-05)
--(axis cs:10600,9.43855082559888e-05)
--(axis cs:10700,9.36486474895074e-05)
--(axis cs:10800,9.33742647764567e-05)
--(axis cs:10900,9.2190950556113e-05)
--(axis cs:11000,8.92080258762501e-05)
--(axis cs:11100,8.5679747917207e-05)
--(axis cs:11200,8.63538395311443e-05)
--(axis cs:11300,8.70492305019831e-05)
--(axis cs:11400,8.98741150221174e-05)
--(axis cs:11500,9.27909559756554e-05)
--(axis cs:11600,9.39604507751447e-05)
--(axis cs:11700,9.34806069832737e-05)
--(axis cs:11800,9.17766170002406e-05)
--(axis cs:11900,8.9181388285441e-05)
--(axis cs:12000,8.84940236975647e-05)
--(axis cs:12100,8.80666981372847e-05)
--(axis cs:12200,8.86013060442862e-05)
--(axis cs:12300,8.59349481294773e-05)
--(axis cs:12400,8.71945962378165e-05)
--(axis cs:12500,8.84944876808836e-05)
--(axis cs:12600,8.8029088221035e-05)
--(axis cs:12700,8.82447335970224e-05)
--(axis cs:12800,8.83636920626717e-05)
--(axis cs:12900,8.56956435743977e-05)
--(axis cs:13000,8.63622709150731e-05)
--(axis cs:13100,8.66251762703017e-05)
--(axis cs:13200,8.54606810729679e-05)
--(axis cs:13300,8.50161033227789e-05)
--(axis cs:13400,8.60783544904851e-05)
--(axis cs:13500,8.67805893501232e-05)
--(axis cs:13600,8.4347776174095e-05)
--(axis cs:13700,8.46066353589163e-05)
--(axis cs:13800,8.35187667107613e-05)
--(axis cs:13900,8.36384131956795e-05)
--(axis cs:14000,8.20011899932928e-05)
--(axis cs:14100,8.20695569435454e-05)
--(axis cs:14200,8.15318789526242e-05)
--(axis cs:14300,8.32358559580136e-05)
--(axis cs:14400,8.32642403535338e-05)
--(axis cs:14500,8.25459769360737e-05)
--(axis cs:14600,8.23704208177882e-05)
--(axis cs:14700,8.36477270763379e-05)
--(axis cs:14800,8.04299475858256e-05)
--(axis cs:14900,7.91436596050231e-05)
--(axis cs:15000,7.79270213966436e-05)
--(axis cs:15100,7.75396331603952e-05)
--(axis cs:15200,7.55497428870005e-05)
--(axis cs:15300,7.67525877888417e-05)
--(axis cs:15400,7.84932585196413e-05)
--(axis cs:15500,7.94264469060556e-05)
--(axis cs:15600,7.8085255372489e-05)
--(axis cs:15700,7.82438081586132e-05)
--(axis cs:15800,7.80856239388613e-05)
--(axis cs:15900,7.63595080269357e-05)
--(axis cs:16000,7.5460649638751e-05)
--(axis cs:16100,7.46196097397629e-05)
--(axis cs:16200,7.5903055897795e-05)
--(axis cs:16300,7.58335417131963e-05)
--(axis cs:16400,7.70768168157377e-05)
--(axis cs:16500,7.54256031061275e-05)
--(axis cs:16600,7.63348006004477e-05)
--(axis cs:16700,7.54307535155135e-05)
--(axis cs:16800,7.43807592522468e-05)
--(axis cs:16900,7.3736714129013e-05)
--(axis cs:17000,7.42769088927572e-05)
--(axis cs:17100,7.34832200798359e-05)
--(axis cs:17200,7.28710887031161e-05)
--(axis cs:17300,7.4204123397513e-05)
--(axis cs:17400,7.49344799023913e-05)
--(axis cs:17500,7.46213388153844e-05)
--(axis cs:17600,7.52874054039201e-05)
--(axis cs:17700,7.48927131702648e-05)
--(axis cs:17800,7.40453719209013e-05)
--(axis cs:17900,7.19245245512281e-05)
--(axis cs:18000,7.33578404874997e-05)
--(axis cs:18100,7.42160416268778e-05)
--(axis cs:18200,7.40627210928966e-05)
--(axis cs:18300,7.45572609541029e-05)
--(axis cs:18400,7.47634906466555e-05)
--(axis cs:18500,7.35666419237113e-05)
--(axis cs:18600,7.14857202751341e-05)
--(axis cs:18700,7.09770022904407e-05)
--(axis cs:18800,7.16626408077917e-05)
--(axis cs:18900,7.14616258339688e-05)
--(axis cs:19000,7.20721489187934e-05)
--(axis cs:19100,7.34633483038463e-05)
--(axis cs:19200,7.37075197535939e-05)
--(axis cs:19300,7.42347211622872e-05)
--(axis cs:19400,7.46640853860299e-05)
--(axis cs:19500,7.42388061509685e-05)
--(axis cs:19600,7.27306758206246e-05)
--(axis cs:19700,7.29040922719206e-05)
--(axis cs:19800,7.16890926129019e-05)
--(axis cs:19900,7.10565889017966e-05)
--(axis cs:20000,7.03462727306229e-05)
--(axis cs:20100,7.14104196090918e-05)
--(axis cs:20200,7.16507847541647e-05)
--(axis cs:20300,7.36060615740641e-05)
--(axis cs:20400,7.42676700619262e-05)
--(axis cs:20500,7.40111675739607e-05)
--(axis cs:20600,7.31077953366388e-05)
--(axis cs:20700,7.31965385373868e-05)
--(axis cs:20800,7.12968702897036e-05)
--(axis cs:20900,7.14124880913654e-05)
--(axis cs:21000,7.16170533260604e-05)
--(axis cs:21100,7.13899477860111e-05)
--(axis cs:21200,7.09489684907658e-05)
--(axis cs:21300,7.02368598766867e-05)
--(axis cs:21400,6.98624675983925e-05)
--(axis cs:21500,6.96665501465548e-05)
--(axis cs:21600,7.04190586709522e-05)
--(axis cs:21700,7.07105144436147e-05)
--(axis cs:21800,7.07483719544172e-05)
--(axis cs:21900,7.19195168427021e-05)
--(axis cs:22000,7.10528053734549e-05)
--(axis cs:22100,7.12202407139552e-05)
--(axis cs:22200,6.95015629673265e-05)
--(axis cs:22300,6.97350830707862e-05)
--(axis cs:22400,6.89426750344256e-05)
--(axis cs:22500,6.89246765286983e-05)
--(axis cs:22600,6.76330911186871e-05)
--(axis cs:22700,6.78451532285383e-05)
--(axis cs:22800,6.70843058416883e-05)
--(axis cs:22900,6.67929934421954e-05)
--(axis cs:23000,6.70843289817083e-05)
--(axis cs:23100,6.78242036725681e-05)
--(axis cs:23200,6.90571766078277e-05)
--(axis cs:23300,6.89457622451572e-05)
--(axis cs:23400,6.98363685248496e-05)
--(axis cs:23500,6.96262648772451e-05)
--(axis cs:23600,7.01659608131377e-05)
--(axis cs:23700,6.86628355803345e-05)
--(axis cs:23800,6.87498834435233e-05)
--(axis cs:23900,6.84284833825952e-05)
--(axis cs:24000,6.82793248242338e-05)
--(axis cs:24100,6.79880178527122e-05)
--(axis cs:24200,6.92752146496692e-05)
--(axis cs:24300,6.8843109935723e-05)
--(axis cs:24400,6.85384142048596e-05)
--(axis cs:24500,6.83184156041719e-05)
--(axis cs:24600,6.73594546287464e-05)
--(axis cs:24700,6.73095012931081e-05)
--(axis cs:24800,6.73684105802712e-05)
--(axis cs:24900,6.64009526094589e-05)
--(axis cs:25000,6.55053337791316e-05)
--(axis cs:25100,6.58480979859444e-05)
--(axis cs:25200,6.57219587425822e-05)
--(axis cs:25300,6.57552460248583e-05)
--(axis cs:25400,6.57391665638293e-05)
--(axis cs:25500,6.64376728685177e-05)
--(axis cs:25600,6.56948340151946e-05)
--(axis cs:25700,6.58319944352881e-05)
--(axis cs:25800,6.61122446801713e-05)
--(axis cs:25900,6.626389214239e-05)
--(axis cs:26000,6.59013438419499e-05)
--(axis cs:26100,6.61835691913976e-05)
--(axis cs:26200,6.58787345647683e-05)
--(axis cs:26300,6.60659145475971e-05)
--(axis cs:26400,6.59565868945148e-05)
--(axis cs:26500,6.57882429986464e-05)
--(axis cs:26600,6.5244260908148e-05)
--(axis cs:26700,6.51380424601179e-05)
--(axis cs:26800,6.51656649538671e-05)
--(axis cs:26900,6.51529735151676e-05)
--(axis cs:27000,6.45814763201072e-05)
--(axis cs:27100,6.42804429928451e-05)
--(axis cs:27200,6.41661852927335e-05)
--(axis cs:27300,6.38788239454142e-05)
--(axis cs:27400,6.41202570635051e-05)
--(axis cs:27500,6.48989302683124e-05)
--(axis cs:27600,6.52201841775685e-05)
--(axis cs:27700,6.53009780458412e-05)
--(axis cs:27800,6.49674332740775e-05)
--(axis cs:27900,6.46572846144236e-05)
--(axis cs:28000,6.46290614645067e-05)
--(axis cs:28100,6.46342242204233e-05)
--(axis cs:28200,6.45448333388738e-05)
--(axis cs:28300,6.49180989119943e-05)
--(axis cs:28400,6.49763207367949e-05)
--(axis cs:28500,6.53680924184854e-05)
--(axis cs:28600,6.56755132748502e-05)
--(axis cs:28700,6.54337871336116e-05)
--(axis cs:28800,6.50589041017106e-05)
--(axis cs:28900,6.48777925701976e-05)
--(axis cs:29000,6.42724983886354e-05)
--(axis cs:29100,6.40650955277576e-05)
--(axis cs:29200,6.41449436048882e-05)
--(axis cs:29300,6.48019684853355e-05)
--(axis cs:29400,6.50493228966052e-05)
--(axis cs:29500,6.47546491567011e-05)
--(axis cs:29500,6.91619904497673e-05)
--(axis cs:29500,6.91619904497673e-05)
--(axis cs:29400,6.93031252281437e-05)
--(axis cs:29300,6.96568240657747e-05)
--(axis cs:29200,6.98749593024238e-05)
--(axis cs:29100,7.0252898512369e-05)
--(axis cs:29000,7.03048573469894e-05)
--(axis cs:28900,7.03708866706574e-05)
--(axis cs:28800,6.99189339227865e-05)
--(axis cs:28700,6.96442408272327e-05)
--(axis cs:28600,6.9209126523503e-05)
--(axis cs:28500,6.91665796393916e-05)
--(axis cs:28400,6.90388760811321e-05)
--(axis cs:28300,6.93251390292212e-05)
--(axis cs:28200,6.9099871717339e-05)
--(axis cs:28100,6.91869839259775e-05)
--(axis cs:28000,6.89130380374309e-05)
--(axis cs:27900,6.8741163231018e-05)
--(axis cs:27800,6.87219801163553e-05)
--(axis cs:27700,6.89914987258687e-05)
--(axis cs:27600,6.8952917412757e-05)
--(axis cs:27500,6.88829372603323e-05)
--(axis cs:27400,6.89959874301681e-05)
--(axis cs:27300,6.92185137298667e-05)
--(axis cs:27200,6.89500145750664e-05)
--(axis cs:27100,6.962891192486e-05)
--(axis cs:27000,7.00201461893524e-05)
--(axis cs:26900,7.05470391972613e-05)
--(axis cs:26800,7.0141827307575e-05)
--(axis cs:26700,7.04632801333599e-05)
--(axis cs:26600,6.9588373255562e-05)
--(axis cs:26500,6.92868124909806e-05)
--(axis cs:26400,6.84054858669663e-05)
--(axis cs:26300,6.86043571070162e-05)
--(axis cs:26200,6.84492915657168e-05)
--(axis cs:26100,6.90382540048397e-05)
--(axis cs:26000,6.8978203756201e-05)
--(axis cs:25900,6.95363153570247e-05)
--(axis cs:25800,6.95054303855126e-05)
--(axis cs:25700,7.03898713000391e-05)
--(axis cs:25600,6.98537572881341e-05)
--(axis cs:25500,7.03163990923289e-05)
--(axis cs:25400,7.03759599031702e-05)
--(axis cs:25300,7.01766553372454e-05)
--(axis cs:25200,6.98380373817747e-05)
--(axis cs:25100,7.01521498414763e-05)
--(axis cs:25000,6.97261809926478e-05)
--(axis cs:24900,6.95579687488408e-05)
--(axis cs:24800,6.96263083429622e-05)
--(axis cs:24700,6.97302354350758e-05)
--(axis cs:24600,7.06168860491531e-05)
--(axis cs:24500,7.10122456305844e-05)
--(axis cs:24400,7.0802675902477e-05)
--(axis cs:24300,7.08978716527276e-05)
--(axis cs:24200,7.06873935778371e-05)
--(axis cs:24100,7.1554361136957e-05)
--(axis cs:24000,7.18045095882739e-05)
--(axis cs:23900,7.27557096219484e-05)
--(axis cs:23800,7.26332701369163e-05)
--(axis cs:23700,7.28456633472439e-05)
--(axis cs:23600,7.30108948226916e-05)
--(axis cs:23500,7.23178708560141e-05)
--(axis cs:23400,7.06909937119035e-05)
--(axis cs:23300,7.08533406628431e-05)
--(axis cs:23200,7.13172760439611e-05)
--(axis cs:23100,7.02004134691655e-05)
--(axis cs:23000,7.00795937910345e-05)
--(axis cs:22900,7.08855403503003e-05)
--(axis cs:22800,7.14441791258489e-05)
--(axis cs:22700,7.19818088361029e-05)
--(axis cs:22600,7.29256528083198e-05)
--(axis cs:22500,7.43890156166616e-05)
--(axis cs:22400,7.44422002295931e-05)
--(axis cs:22300,7.47949406102136e-05)
--(axis cs:22200,7.41654913952686e-05)
--(axis cs:22100,7.38757486657662e-05)
--(axis cs:22000,7.3356216222038e-05)
--(axis cs:21900,7.35241401047616e-05)
--(axis cs:21800,7.32776568140527e-05)
--(axis cs:21700,7.27547727637006e-05)
--(axis cs:21600,7.26289737099987e-05)
--(axis cs:21500,7.30937617665009e-05)
--(axis cs:21400,7.29121789212908e-05)
--(axis cs:21300,7.38453344339263e-05)
--(axis cs:21200,7.37480490888841e-05)
--(axis cs:21100,7.3278517965833e-05)
--(axis cs:21000,7.34776690669084e-05)
--(axis cs:20900,7.48121992502352e-05)
--(axis cs:20800,7.71818543936209e-05)
--(axis cs:20700,7.74985010428789e-05)
--(axis cs:20600,7.8283045040399e-05)
--(axis cs:20500,7.86529052376428e-05)
--(axis cs:20400,7.81492462305449e-05)
--(axis cs:20300,7.59295347578278e-05)
--(axis cs:20200,7.69959417904712e-05)
--(axis cs:20100,7.76766886357172e-05)
--(axis cs:20000,7.7841823042016e-05)
--(axis cs:19900,7.7932574282121e-05)
--(axis cs:19800,7.75639326888302e-05)
--(axis cs:19700,7.71267241676186e-05)
--(axis cs:19600,7.65657976194687e-05)
--(axis cs:19500,7.66572109006438e-05)
--(axis cs:19400,7.69232533828472e-05)
--(axis cs:19300,7.76938493472906e-05)
--(axis cs:19200,7.80679626675261e-05)
--(axis cs:19100,7.87813955484089e-05)
--(axis cs:19000,7.85902720584241e-05)
--(axis cs:18900,7.78911683686967e-05)
--(axis cs:18800,7.8636883537333e-05)
--(axis cs:18700,7.82909755892524e-05)
--(axis cs:18600,7.75761122630509e-05)
--(axis cs:18500,7.78622740245853e-05)
--(axis cs:18400,7.76135922031973e-05)
--(axis cs:18300,7.66414504861747e-05)
--(axis cs:18200,7.65465902443758e-05)
--(axis cs:18100,7.62305783280137e-05)
--(axis cs:18000,7.66674219710606e-05)
--(axis cs:17900,7.73792141750749e-05)
--(axis cs:17800,7.79882352829225e-05)
--(axis cs:17700,8.1604125535039e-05)
--(axis cs:17600,8.22660983127549e-05)
--(axis cs:17500,8.31279512194114e-05)
--(axis cs:17400,8.34596229584717e-05)
--(axis cs:17300,8.36190263382159e-05)
--(axis cs:17200,8.23526989814983e-05)
--(axis cs:17100,8.20951065868918e-05)
--(axis cs:17000,8.09267049867124e-05)
--(axis cs:16900,8.1084149455354e-05)
--(axis cs:16800,8.10379600680008e-05)
--(axis cs:16700,8.07754378466787e-05)
--(axis cs:16600,8.18477358454209e-05)
--(axis cs:16500,8.25109817191896e-05)
--(axis cs:16400,8.27559407714964e-05)
--(axis cs:16300,8.46424726153033e-05)
--(axis cs:16200,8.57161927857694e-05)
--(axis cs:16100,8.65288340395244e-05)
--(axis cs:16000,8.70853523180471e-05)
--(axis cs:15900,8.76210877017572e-05)
--(axis cs:15800,8.67758777989469e-05)
--(axis cs:15700,8.62128214625622e-05)
--(axis cs:15600,8.60368703434596e-05)
--(axis cs:15500,8.67120077059785e-05)
--(axis cs:15400,8.51255824172405e-05)
--(axis cs:15300,8.51943351010689e-05)
--(axis cs:15200,8.44609060431344e-05)
--(axis cs:15100,8.37985831155128e-05)
--(axis cs:15000,8.38048833639804e-05)
--(axis cs:14900,8.38162046416359e-05)
--(axis cs:14800,8.43295083613798e-05)
--(axis cs:14700,8.5107807028665e-05)
--(axis cs:14600,8.55294111952749e-05)
--(axis cs:14500,8.51578310775865e-05)
--(axis cs:14400,8.79181011320609e-05)
--(axis cs:14300,8.79159061329202e-05)
--(axis cs:14200,8.90919968913577e-05)
--(axis cs:14100,8.95045657557426e-05)
--(axis cs:14000,8.91202080713255e-05)
--(axis cs:13900,8.88254203915646e-05)
--(axis cs:13800,9.08230584755137e-05)
--(axis cs:13700,9.11135928337907e-05)
--(axis cs:13600,9.50887230400153e-05)
--(axis cs:13500,9.56267842511371e-05)
--(axis cs:13400,9.35233991833415e-05)
--(axis cs:13300,9.26955816325051e-05)
--(axis cs:13200,9.28609221857933e-05)
--(axis cs:13100,9.04664942627196e-05)
--(axis cs:13000,8.93851984629413e-05)
--(axis cs:12900,8.98846213872598e-05)
--(axis cs:12800,8.99240847840774e-05)
--(axis cs:12700,8.98435665659039e-05)
--(axis cs:12600,9.04488113384281e-05)
--(axis cs:12500,8.89450987725666e-05)
--(axis cs:12400,9.0823362877279e-05)
--(axis cs:12300,9.2780443537151e-05)
--(axis cs:12200,9.13512913953134e-05)
--(axis cs:12100,9.30159079066923e-05)
--(axis cs:12000,9.36248504232718e-05)
--(axis cs:11900,9.53062601780565e-05)
--(axis cs:11800,9.55877986146251e-05)
--(axis cs:11700,9.68399516298925e-05)
--(axis cs:11600,9.68284602595188e-05)
--(axis cs:11500,9.87916126350525e-05)
--(axis cs:11400,0.000100291295921522)
--(axis cs:11300,9.93126765092253e-05)
--(axis cs:11200,9.77097622420879e-05)
--(axis cs:11100,9.79798936594134e-05)
--(axis cs:11000,0.000101270247364289)
--(axis cs:10900,0.000103350020333738)
--(axis cs:10800,0.000102261975562139)
--(axis cs:10700,0.000105462992808611)
--(axis cs:10600,0.000104946542141072)
--(axis cs:10500,0.00010309171777532)
--(axis cs:10400,0.000101618817048213)
--(axis cs:10300,0.00010442035467336)
--(axis cs:10200,0.000105192919356395)
--(axis cs:10100,0.000105976663729443)
--(axis cs:10000,0.000102889131585796)
--(axis cs:9900,0.000100706984067749)
--(axis cs:9800,0.000101071154670044)
--(axis cs:9700,0.000100728794584013)
--(axis cs:9600,0.000101813803277775)
--(axis cs:9500,0.000100794071021218)
--(axis cs:9400,0.000102762088172978)
--(axis cs:9300,0.000103140569148116)
--(axis cs:9200,0.000104656016865337)
--(axis cs:9100,0.000107681648602931)
--(axis cs:9000,0.000107483620140588)
--(axis cs:8900,0.000106798393704457)
--(axis cs:8800,0.0001051147302749)
--(axis cs:8700,0.000106148314343864)
--(axis cs:8600,0.000106449966036246)
--(axis cs:8500,0.000114142248235731)
--(axis cs:8400,0.000115653796387726)
--(axis cs:8300,0.00011626685215021)
--(axis cs:8200,0.000118023586101196)
--(axis cs:8100,0.000118395520741153)
--(axis cs:8000,0.000116107462942239)
--(axis cs:7900,0.00011755555135565)
--(axis cs:7800,0.000115459865646008)
--(axis cs:7700,0.000115909083121321)
--(axis cs:7600,0.000114017379900218)
--(axis cs:7500,0.000120457840313981)
--(axis cs:7400,0.000121880895094816)
--(axis cs:7300,0.000122250096141002)
--(axis cs:7200,0.000123237601720164)
--(axis cs:7100,0.000124571133051002)
--(axis cs:7000,0.000121984774047384)
--(axis cs:6900,0.000136805625700783)
--(axis cs:6800,0.000150518503661521)
--(axis cs:6700,0.000148748587683023)
--(axis cs:6600,0.000150864835079374)
--(axis cs:6500,0.000147152632644236)
--(axis cs:6400,0.000145773039243887)
--(axis cs:6300,0.000140859944121113)
--(axis cs:6200,0.00014010768521033)
--(axis cs:6100,0.000142531782268821)
--(axis cs:6000,0.000144817633792639)
--(axis cs:5900,0.000143207791795818)
--(axis cs:5800,0.000140155969827431)
--(axis cs:5700,0.0001450835679476)
--(axis cs:5600,0.000155043374921327)
--(axis cs:5500,0.000155513180006611)
--(axis cs:5400,0.000153316120663661)
--(axis cs:5300,0.000160129250232971)
--(axis cs:5200,0.000159388779016257)
--(axis cs:5100,0.000152628706236988)
--(axis cs:5000,0.00015620427925158)
--(axis cs:4900,0.000158546074012022)
--(axis cs:4800,0.000161689020407954)
--(axis cs:4700,0.000170593690649705)
--(axis cs:4600,0.000171985255631423)
--(axis cs:4500,0.000173564966814389)
--(axis cs:4400,0.00018204455295394)
--(axis cs:4300,0.000184299546740831)
--(axis cs:4200,0.000183282939865283)
--(axis cs:4100,0.00018467234622349)
--(axis cs:4000,0.00018381312140751)
--(axis cs:3900,0.000181656276362368)
--(axis cs:3800,0.000183107974244534)
--(axis cs:3700,0.000183286917342181)
--(axis cs:3600,0.000189150277936249)
--(axis cs:3500,0.000190583405329372)
--(axis cs:3400,0.000186250201547963)
--(axis cs:3300,0.000192229863817698)
--(axis cs:3200,0.000190940866572572)
--(axis cs:3100,0.000197574587678648)
--(axis cs:3000,0.000207758539509519)
--(axis cs:2900,0.000214278501228518)
--(axis cs:2800,0.000213409303576371)
--(axis cs:2700,0.000218547457614763)
--(axis cs:2600,0.000217739182190267)
--(axis cs:2500,0.000216569751940814)
--(axis cs:2400,0.000209891373191033)
--(axis cs:2300,0.000211435046687278)
--(axis cs:2200,0.000211742117447431)
--(axis cs:2100,0.0002152653824086)
--(axis cs:2000,0.000226381764511681)
--(axis cs:1900,0.000238366702551749)
--(axis cs:1800,0.000234648231123401)
--(axis cs:1700,0.000244962568023539)
--(axis cs:1600,0.000247852969385046)
--(axis cs:1500,0.000246498755010423)
--(axis cs:1400,0.000250404794349108)
--(axis cs:1300,0.000263884536977211)
--(axis cs:1200,0.00027354119651791)
--(axis cs:1100,0.000287363608815189)
--(axis cs:1000,0.000316635532918552)
--(axis cs:900,0.000336890663030776)
--(axis cs:800,0.000370540757322453)
--(axis cs:700,0.000442363081526322)
--(axis cs:600,0.000663961720752591)
--(axis cs:500,0.00103819168757927)
--(axis cs:400,0.00186996323304045)
--(axis cs:300,0.00346133319078174)
--(axis cs:200,0.00511083696938624)
--(axis cs:100,0.0066082193052827)
--(axis cs:0,0.00794493036430928)
--cycle;

\path [fill=blue, fill opacity=0.2, semithick]
(axis cs:0,0.00720213678466435)
--(axis cs:0,0.00706319136433646)
--(axis cs:100,0.00577221439616148)
--(axis cs:200,0.00437417259646036)
--(axis cs:300,0.00282089913568673)
--(axis cs:400,0.00136047739749201)
--(axis cs:500,0.00077469900148994)
--(axis cs:600,0.000496558219041754)
--(axis cs:700,0.00030810862638953)
--(axis cs:800,0.000285933100774087)
--(axis cs:900,0.000265588027901413)
--(axis cs:1000,0.000242055493928945)
--(axis cs:1100,0.000211403978837982)
--(axis cs:1200,0.000198701190636847)
--(axis cs:1300,0.000188256568195119)
--(axis cs:1400,0.000182206979851282)
--(axis cs:1500,0.00017908389568628)
--(axis cs:1600,0.000169238035150954)
--(axis cs:1700,0.000163385214052475)
--(axis cs:1800,0.000160370126617323)
--(axis cs:1900,0.000155548191553739)
--(axis cs:2000,0.000154881252626218)
--(axis cs:2100,0.000153664180802631)
--(axis cs:2200,0.000144987952941353)
--(axis cs:2300,0.000136861704128159)
--(axis cs:2400,0.000130871424616827)
--(axis cs:2500,0.000132241600212644)
--(axis cs:2600,0.000132929589784729)
--(axis cs:2700,0.00013109479561135)
--(axis cs:2800,0.000133114026358595)
--(axis cs:2900,0.000123390086199334)
--(axis cs:3000,0.000125517524186516)
--(axis cs:3100,0.000126149054528304)
--(axis cs:3200,0.000121162026848257)
--(axis cs:3300,0.000112764267625281)
--(axis cs:3400,0.000116631922919917)
--(axis cs:3500,0.000111669668139284)
--(axis cs:3600,0.000105183232985002)
--(axis cs:3700,9.7802978012536e-05)
--(axis cs:3800,9.77233266676977e-05)
--(axis cs:3900,9.91469780786126e-05)
--(axis cs:4000,0.000100614156694267)
--(axis cs:4100,9.79694216878478e-05)
--(axis cs:4200,9.91715470346761e-05)
--(axis cs:4300,9.6317229487025e-05)
--(axis cs:4400,9.40337711327546e-05)
--(axis cs:4500,9.00317882660934e-05)
--(axis cs:4600,9.4740007765207e-05)
--(axis cs:4700,9.20050667851291e-05)
--(axis cs:4800,8.80454828334114e-05)
--(axis cs:4900,8.29170278520576e-05)
--(axis cs:5000,7.82815912057926e-05)
--(axis cs:5100,7.87812087001077e-05)
--(axis cs:5200,7.82469831003933e-05)
--(axis cs:5300,7.85129213016319e-05)
--(axis cs:5400,7.47607263862246e-05)
--(axis cs:5500,7.41085851649445e-05)
--(axis cs:5600,7.37033814928695e-05)
--(axis cs:5700,7.0544428886813e-05)
--(axis cs:5800,7.08079930139044e-05)
--(axis cs:5900,6.91807208571154e-05)
--(axis cs:6000,6.91162982179064e-05)
--(axis cs:6100,6.60846709223607e-05)
--(axis cs:6200,6.49503448796098e-05)
--(axis cs:6300,6.25422492970282e-05)
--(axis cs:6400,6.56521623567763e-05)
--(axis cs:6500,6.66362198326674e-05)
--(axis cs:6600,6.88057136976539e-05)
--(axis cs:6700,6.92103519582625e-05)
--(axis cs:6800,6.80141312091571e-05)
--(axis cs:6900,6.51011834458477e-05)
--(axis cs:7000,6.65326936615343e-05)
--(axis cs:7100,6.7397650247664e-05)
--(axis cs:7200,6.52705484436963e-05)
--(axis cs:7300,6.36224732986686e-05)
--(axis cs:7400,6.26280954158098e-05)
--(axis cs:7500,6.10055686207734e-05)
--(axis cs:7600,6.10377387396744e-05)
--(axis cs:7700,6.280401568195e-05)
--(axis cs:7800,6.24553621242084e-05)
--(axis cs:7900,6.08046810681856e-05)
--(axis cs:8000,6.20443091752337e-05)
--(axis cs:8100,6.20841647410181e-05)
--(axis cs:8200,6.10104611950603e-05)
--(axis cs:8300,6.10349664206641e-05)
--(axis cs:8400,6.05256270235834e-05)
--(axis cs:8500,5.77774128819773e-05)
--(axis cs:8600,5.95845166465777e-05)
--(axis cs:8700,5.84384282610086e-05)
--(axis cs:8800,5.4735706419128e-05)
--(axis cs:8900,5.40258237078303e-05)
--(axis cs:9000,5.5526856524376e-05)
--(axis cs:9100,5.42293906217722e-05)
--(axis cs:9200,5.4841631987728e-05)
--(axis cs:9300,5.70718487677459e-05)
--(axis cs:9400,5.49419563023293e-05)
--(axis cs:9500,5.54033201597231e-05)
--(axis cs:9600,5.49950598664233e-05)
--(axis cs:9700,5.60037581940378e-05)
--(axis cs:9800,5.63077568048105e-05)
--(axis cs:9900,5.60716843123014e-05)
--(axis cs:10000,5.63102866784549e-05)
--(axis cs:10100,5.75382788069966e-05)
--(axis cs:10200,5.52797739673536e-05)
--(axis cs:10300,5.52897748716874e-05)
--(axis cs:10400,5.40251794142322e-05)
--(axis cs:10500,5.30424289663948e-05)
--(axis cs:10600,5.5465258790601e-05)
--(axis cs:10700,5.41210931723209e-05)
--(axis cs:10800,5.43041570537651e-05)
--(axis cs:10900,5.37592554503919e-05)
--(axis cs:11000,5.16405348140156e-05)
--(axis cs:11100,4.82689686671494e-05)
--(axis cs:11200,4.98641667624403e-05)
--(axis cs:11300,5.0602842958679e-05)
--(axis cs:11400,5.17053538030205e-05)
--(axis cs:11500,5.25023035117707e-05)
--(axis cs:11600,5.20464327593676e-05)
--(axis cs:11700,5.30923157407788e-05)
--(axis cs:11800,5.25839820329661e-05)
--(axis cs:11900,5.15252053025331e-05)
--(axis cs:12000,4.97656534430524e-05)
--(axis cs:12100,5.06811755202665e-05)
--(axis cs:12200,5.00071348003669e-05)
--(axis cs:12300,4.82671777861011e-05)
--(axis cs:12400,4.82424257567556e-05)
--(axis cs:12500,4.87852536057573e-05)
--(axis cs:12600,4.86974927147951e-05)
--(axis cs:12700,4.91464950191291e-05)
--(axis cs:12800,4.91397908869691e-05)
--(axis cs:12900,4.93310022679003e-05)
--(axis cs:13000,4.72517338884877e-05)
--(axis cs:13100,5.00814928860332e-05)
--(axis cs:13200,4.8717069447104e-05)
--(axis cs:13300,4.74390614446605e-05)
--(axis cs:13400,4.8964915507706e-05)
--(axis cs:13500,4.68144138326579e-05)
--(axis cs:13600,4.58292159908577e-05)
--(axis cs:13700,4.51842287095966e-05)
--(axis cs:13800,4.56782587143971e-05)
--(axis cs:13900,4.73403977355977e-05)
--(axis cs:14000,4.73536003036408e-05)
--(axis cs:14100,4.64808062224246e-05)
--(axis cs:14200,4.60850053050127e-05)
--(axis cs:14300,4.60878014381667e-05)
--(axis cs:14400,4.40438263077243e-05)
--(axis cs:14500,4.54394970399111e-05)
--(axis cs:14600,4.74550721312535e-05)
--(axis cs:14700,4.84666334895731e-05)
--(axis cs:14800,4.72641356234924e-05)
--(axis cs:14900,4.80943371609573e-05)
--(axis cs:15000,4.64693051589498e-05)
--(axis cs:15100,4.54545903720093e-05)
--(axis cs:15200,4.45208684711475e-05)
--(axis cs:15300,4.50445274389382e-05)
--(axis cs:15400,4.41609335396579e-05)
--(axis cs:15500,4.37829478946518e-05)
--(axis cs:15600,4.26522150698282e-05)
--(axis cs:15700,4.22515689190656e-05)
--(axis cs:15800,4.15713976657436e-05)
--(axis cs:15900,4.12029642459861e-05)
--(axis cs:16000,4.13976885467813e-05)
--(axis cs:16100,4.20190708337453e-05)
--(axis cs:16200,4.24673091498373e-05)
--(axis cs:16300,4.3292515840797e-05)
--(axis cs:16400,4.23728882992894e-05)
--(axis cs:16500,4.23943805797954e-05)
--(axis cs:16600,4.07719897851463e-05)
--(axis cs:16700,4.0481905602146e-05)
--(axis cs:16800,4.10341376556345e-05)
--(axis cs:16900,4.06161416936638e-05)
--(axis cs:17000,4.12047184201416e-05)
--(axis cs:17100,4.16022295710486e-05)
--(axis cs:17200,4.09656989023333e-05)
--(axis cs:17300,4.05614785059299e-05)
--(axis cs:17400,4.12486373995452e-05)
--(axis cs:17500,3.97352641970383e-05)
--(axis cs:17600,4.03139910517701e-05)
--(axis cs:17700,3.99391260841412e-05)
--(axis cs:17800,3.87285037624204e-05)
--(axis cs:17900,3.81054293074747e-05)
--(axis cs:18000,3.91568350246911e-05)
--(axis cs:18100,3.88519784507477e-05)
--(axis cs:18200,3.90312253710471e-05)
--(axis cs:18300,3.97602238213474e-05)
--(axis cs:18400,3.99829663506013e-05)
--(axis cs:18500,3.99041829071979e-05)
--(axis cs:18600,3.93868875260377e-05)
--(axis cs:18700,3.99190818865908e-05)
--(axis cs:18800,3.96964898896059e-05)
--(axis cs:18900,3.9010189283625e-05)
--(axis cs:19000,3.97541330383624e-05)
--(axis cs:19100,4.06890009303233e-05)
--(axis cs:19200,4.08721090363477e-05)
--(axis cs:19300,4.09115275098928e-05)
--(axis cs:19400,3.96158693614142e-05)
--(axis cs:19500,3.83522701816274e-05)
--(axis cs:19600,3.7608433293249e-05)
--(axis cs:19700,3.67386779706204e-05)
--(axis cs:19800,3.62074605933528e-05)
--(axis cs:19900,3.66512574263734e-05)
--(axis cs:20000,3.71565481036511e-05)
--(axis cs:20100,3.73322432799091e-05)
--(axis cs:20200,3.6917290051917e-05)
--(axis cs:20300,3.65120793586581e-05)
--(axis cs:20400,3.66685380628456e-05)
--(axis cs:20500,3.72314685755394e-05)
--(axis cs:20600,3.76741962450594e-05)
--(axis cs:20700,3.73901974692333e-05)
--(axis cs:20800,3.79194220655756e-05)
--(axis cs:20900,3.73744950129641e-05)
--(axis cs:21000,3.62831093868596e-05)
--(axis cs:21100,3.57933518126519e-05)
--(axis cs:21200,3.6485979004698e-05)
--(axis cs:21300,3.52353525150885e-05)
--(axis cs:21400,3.50850485614013e-05)
--(axis cs:21500,3.66351549544233e-05)
--(axis cs:21600,3.66028227632385e-05)
--(axis cs:21700,3.6605132446809e-05)
--(axis cs:21800,3.69052376857737e-05)
--(axis cs:21900,3.73105573865435e-05)
--(axis cs:22000,3.61963174956502e-05)
--(axis cs:22100,3.693090463107e-05)
--(axis cs:22200,3.52409326390055e-05)
--(axis cs:22300,3.54268641151968e-05)
--(axis cs:22400,3.44003287108338e-05)
--(axis cs:22500,3.4695980468063e-05)
--(axis cs:22600,3.34461610766644e-05)
--(axis cs:22700,3.42714972141682e-05)
--(axis cs:22800,3.32913099413783e-05)
--(axis cs:22900,3.31488524010863e-05)
--(axis cs:23000,3.2931827101704e-05)
--(axis cs:23100,3.34058686720704e-05)
--(axis cs:23200,3.34250374584675e-05)
--(axis cs:23300,3.39521514719616e-05)
--(axis cs:23400,3.37477290105011e-05)
--(axis cs:23500,3.35166731431999e-05)
--(axis cs:23600,3.40363471992204e-05)
--(axis cs:23700,3.3942291150978e-05)
--(axis cs:23800,3.35693091152037e-05)
--(axis cs:23900,3.37868478020123e-05)
--(axis cs:24000,3.41911919908111e-05)
--(axis cs:24100,3.37967035296673e-05)
--(axis cs:24200,3.29314938724174e-05)
--(axis cs:24300,3.28876295980991e-05)
--(axis cs:24400,3.23736112183717e-05)
--(axis cs:24500,3.21912815269417e-05)
--(axis cs:24600,3.20948335801269e-05)
--(axis cs:24700,3.20475478394499e-05)
--(axis cs:24800,3.2165695284819e-05)
--(axis cs:24900,3.21732907499491e-05)
--(axis cs:25000,3.14864657747581e-05)
--(axis cs:25100,3.16565075859894e-05)
--(axis cs:25200,3.21920901055323e-05)
--(axis cs:25300,3.20012925374529e-05)
--(axis cs:25400,3.203463643662e-05)
--(axis cs:25500,3.19545111949365e-05)
--(axis cs:25600,3.19728481944439e-05)
--(axis cs:25700,3.20102585702372e-05)
--(axis cs:25800,3.2071952875533e-05)
--(axis cs:25900,3.21948850331592e-05)
--(axis cs:26000,3.25313008421233e-05)
--(axis cs:26100,3.23180512302583e-05)
--(axis cs:26200,3.27070065634908e-05)
--(axis cs:26300,3.29213744416118e-05)
--(axis cs:26400,3.21702513720013e-05)
--(axis cs:26500,3.19943125588622e-05)
--(axis cs:26600,3.16706324249326e-05)
--(axis cs:26700,3.08080753536871e-05)
--(axis cs:26800,3.03615977898636e-05)
--(axis cs:26900,3.02972637328791e-05)
--(axis cs:27000,3.00350565439973e-05)
--(axis cs:27100,2.98849284695719e-05)
--(axis cs:27200,2.96830704151674e-05)
--(axis cs:27300,2.97293066915623e-05)
--(axis cs:27400,3.01253529303379e-05)
--(axis cs:27500,3.01355754066362e-05)
--(axis cs:27600,2.99782098715779e-05)
--(axis cs:27700,3.01719873345313e-05)
--(axis cs:27800,2.98428551620278e-05)
--(axis cs:27900,2.95494862050136e-05)
--(axis cs:28000,2.97255455095266e-05)
--(axis cs:28100,2.97177266101585e-05)
--(axis cs:28200,2.96837146462982e-05)
--(axis cs:28300,2.99967285577377e-05)
--(axis cs:28400,3.01990492702662e-05)
--(axis cs:28500,3.00986949263421e-05)
--(axis cs:28600,3.00345980058584e-05)
--(axis cs:28700,2.99414323676473e-05)
--(axis cs:28800,2.97716036075847e-05)
--(axis cs:28900,2.97758136596494e-05)
--(axis cs:29000,2.95766487138792e-05)
--(axis cs:29100,2.97845818149107e-05)
--(axis cs:29200,2.99098398131834e-05)
--(axis cs:29300,3.01235356853252e-05)
--(axis cs:29400,2.98650407819179e-05)
--(axis cs:29500,2.96251221720614e-05)
--(axis cs:29500,3.52258680906748e-05)
--(axis cs:29500,3.52258680906748e-05)
--(axis cs:29400,3.52264123614776e-05)
--(axis cs:29300,3.54372669282927e-05)
--(axis cs:29200,3.55091044249584e-05)
--(axis cs:29100,3.51494450715655e-05)
--(axis cs:29000,3.55821812522151e-05)
--(axis cs:28900,3.51811511682694e-05)
--(axis cs:28800,3.46270515267461e-05)
--(axis cs:28700,3.48478347339882e-05)
--(axis cs:28600,3.53014694370791e-05)
--(axis cs:28500,3.50085424369696e-05)
--(axis cs:28400,3.54898463346174e-05)
--(axis cs:28300,3.59386881326466e-05)
--(axis cs:28200,3.58825735542969e-05)
--(axis cs:28100,3.57745665566919e-05)
--(axis cs:28000,3.60997956434319e-05)
--(axis cs:27900,3.60175630607479e-05)
--(axis cs:27800,3.62507342985271e-05)
--(axis cs:27700,3.57993226248915e-05)
--(axis cs:27600,3.53317611367167e-05)
--(axis cs:27500,3.49072694892581e-05)
--(axis cs:27400,3.49251571869029e-05)
--(axis cs:27300,3.51125304164953e-05)
--(axis cs:27200,3.50779477810311e-05)
--(axis cs:27100,3.53049060496399e-05)
--(axis cs:27000,3.46449424089757e-05)
--(axis cs:26900,3.44998502465114e-05)
--(axis cs:26800,3.3914549378266e-05)
--(axis cs:26700,3.42092406322583e-05)
--(axis cs:26600,3.43102973205838e-05)
--(axis cs:26500,3.48555018585993e-05)
--(axis cs:26400,3.50308385180516e-05)
--(axis cs:26300,3.52104258724893e-05)
--(axis cs:26200,3.51779321502933e-05)
--(axis cs:26100,3.58490258367394e-05)
--(axis cs:26000,3.58410290489152e-05)
--(axis cs:25900,3.55667679145547e-05)
--(axis cs:25800,3.53759399221122e-05)
--(axis cs:25700,3.58583616258097e-05)
--(axis cs:25600,3.47759633196729e-05)
--(axis cs:25500,3.44734645428637e-05)
--(axis cs:25400,3.51704809385042e-05)
--(axis cs:25300,3.57895321496555e-05)
--(axis cs:25200,3.54645533115107e-05)
--(axis cs:25100,3.56770260754507e-05)
--(axis cs:25000,3.61978418032617e-05)
--(axis cs:24900,3.61536832466417e-05)
--(axis cs:24800,3.60269553180011e-05)
--(axis cs:24700,3.57855870262488e-05)
--(axis cs:24600,3.6346762214739e-05)
--(axis cs:24500,3.61358159183966e-05)
--(axis cs:24400,3.57921991044054e-05)
--(axis cs:24300,3.58649187973241e-05)
--(axis cs:24200,3.60491737415726e-05)
--(axis cs:24100,3.59796970060106e-05)
--(axis cs:24000,3.65151748809829e-05)
--(axis cs:23900,3.6885624263768e-05)
--(axis cs:23800,3.66397116141282e-05)
--(axis cs:23700,3.75814994848115e-05)
--(axis cs:23600,3.77432069284951e-05)
--(axis cs:23500,3.76120839258427e-05)
--(axis cs:23400,3.70752952299766e-05)
--(axis cs:23300,3.71439166597758e-05)
--(axis cs:23200,3.64862321678022e-05)
--(axis cs:23100,3.61548210631559e-05)
--(axis cs:23000,3.6457365402173e-05)
--(axis cs:22900,3.67605710722048e-05)
--(axis cs:22800,3.71738118843131e-05)
--(axis cs:22700,3.78443439134535e-05)
--(axis cs:22600,3.8746559759364e-05)
--(axis cs:22500,3.8992352745732e-05)
--(axis cs:22400,3.90799281223023e-05)
--(axis cs:22300,3.86903043391013e-05)
--(axis cs:22200,3.80372145837792e-05)
--(axis cs:22100,3.79687207901213e-05)
--(axis cs:22000,3.75923341964099e-05)
--(axis cs:21900,3.86825396902699e-05)
--(axis cs:21800,3.80599150096908e-05)
--(axis cs:21700,3.80512708080639e-05)
--(axis cs:21600,3.85255660413003e-05)
--(axis cs:21500,3.89647556787495e-05)
--(axis cs:21400,3.90787616915868e-05)
--(axis cs:21300,3.91018704863568e-05)
--(axis cs:21200,3.91590318942782e-05)
--(axis cs:21100,3.84042334355812e-05)
--(axis cs:21000,3.93887672580112e-05)
--(axis cs:20900,3.87019297258938e-05)
--(axis cs:20800,4.05295639093497e-05)
--(axis cs:20700,4.14261220167378e-05)
--(axis cs:20600,4.19541899598477e-05)
--(axis cs:20500,4.18539531729199e-05)
--(axis cs:20400,4.21244309348862e-05)
--(axis cs:20300,4.11868625853537e-05)
--(axis cs:20200,4.09879849533094e-05)
--(axis cs:20100,4.08369045145362e-05)
--(axis cs:20000,4.0926346608725e-05)
--(axis cs:19900,4.12468114704318e-05)
--(axis cs:19800,4.03968528177762e-05)
--(axis cs:19700,4.07349484238253e-05)
--(axis cs:19600,4.03560602459353e-05)
--(axis cs:19500,4.03595078602793e-05)
--(axis cs:19400,4.13417232199846e-05)
--(axis cs:19300,4.21217711174253e-05)
--(axis cs:19200,4.22156152091161e-05)
--(axis cs:19100,4.22207655184936e-05)
--(axis cs:19000,4.30120976842165e-05)
--(axis cs:18900,4.30596139396993e-05)
--(axis cs:18800,4.43323028331657e-05)
--(axis cs:18700,4.52526808314522e-05)
--(axis cs:18600,4.5862914202992e-05)
--(axis cs:18500,4.61763454616651e-05)
--(axis cs:18400,4.56244472399739e-05)
--(axis cs:18300,4.33254355073455e-05)
--(axis cs:18200,4.1195973115635e-05)
--(axis cs:18100,4.08775489006987e-05)
--(axis cs:18000,4.01458007370629e-05)
--(axis cs:17900,4.02180774426917e-05)
--(axis cs:17800,4.10999872839834e-05)
--(axis cs:17700,4.1431808798681e-05)
--(axis cs:17600,4.15220589364749e-05)
--(axis cs:17500,4.19084608886548e-05)
--(axis cs:17400,4.29479466668309e-05)
--(axis cs:17300,4.35811446334602e-05)
--(axis cs:17200,4.42497811645026e-05)
--(axis cs:17100,4.58451698964917e-05)
--(axis cs:17000,4.65855843180953e-05)
--(axis cs:16900,4.63951276582694e-05)
--(axis cs:16800,4.60762942674309e-05)
--(axis cs:16700,4.63567600878166e-05)
--(axis cs:16600,4.50573526392575e-05)
--(axis cs:16500,4.43965587087289e-05)
--(axis cs:16400,4.49466871448849e-05)
--(axis cs:16300,4.39344463642256e-05)
--(axis cs:16200,4.45990164032347e-05)
--(axis cs:16100,4.53005385648979e-05)
--(axis cs:16000,4.66941740157969e-05)
--(axis cs:15900,4.73498719469409e-05)
--(axis cs:15800,4.79374576421968e-05)
--(axis cs:15700,4.87939070338825e-05)
--(axis cs:15600,4.8602824954579e-05)
--(axis cs:15500,5.01036711510578e-05)
--(axis cs:15400,4.98913018233934e-05)
--(axis cs:15300,5.00072644292344e-05)
--(axis cs:15200,5.01897673262836e-05)
--(axis cs:15100,5.08280422614135e-05)
--(axis cs:15000,4.94069904650406e-05)
--(axis cs:14900,5.00181634027723e-05)
--(axis cs:14800,5.11542796677424e-05)
--(axis cs:14700,5.01189299506132e-05)
--(axis cs:14600,4.89092079030688e-05)
--(axis cs:14500,4.79702649599779e-05)
--(axis cs:14400,4.82928808586718e-05)
--(axis cs:14300,4.76636448669866e-05)
--(axis cs:14200,4.73194185673066e-05)
--(axis cs:14100,4.81499313143174e-05)
--(axis cs:14000,4.88650577448635e-05)
--(axis cs:13900,4.84382914020623e-05)
--(axis cs:13800,4.82666174687377e-05)
--(axis cs:13700,4.86191456199853e-05)
--(axis cs:13600,4.82314429908555e-05)
--(axis cs:13500,5.08873273946014e-05)
--(axis cs:13400,5.05172302348072e-05)
--(axis cs:13300,5.18381312432657e-05)
--(axis cs:13200,5.32705367778104e-05)
--(axis cs:13100,5.47239830685541e-05)
--(axis cs:13000,5.31102157980942e-05)
--(axis cs:12900,5.11645679549469e-05)
--(axis cs:12800,5.23811121335072e-05)
--(axis cs:12700,5.19918560973556e-05)
--(axis cs:12600,5.12818478302619e-05)
--(axis cs:12500,5.17402280788418e-05)
--(axis cs:12400,5.06805204425535e-05)
--(axis cs:12300,5.05172754106604e-05)
--(axis cs:12200,5.06229048204672e-05)
--(axis cs:12100,5.1787851716148e-05)
--(axis cs:12000,5.48671878054785e-05)
--(axis cs:11900,5.67454052055102e-05)
--(axis cs:11800,5.7493489827408e-05)
--(axis cs:11700,5.63875123566131e-05)
--(axis cs:11600,5.61296839170126e-05)
--(axis cs:11500,5.66999991895349e-05)
--(axis cs:11400,5.55459357886384e-05)
--(axis cs:11300,5.3919011317469e-05)
--(axis cs:11200,5.26194099638834e-05)
--(axis cs:11100,5.24149096445828e-05)
--(axis cs:11000,5.66514068614971e-05)
--(axis cs:10900,5.90040037408294e-05)
--(axis cs:10800,6.08327654385701e-05)
--(axis cs:10700,6.25288588851177e-05)
--(axis cs:10600,6.19282088235158e-05)
--(axis cs:10500,6.00052740864761e-05)
--(axis cs:10400,5.68773006683542e-05)
--(axis cs:10300,5.65235571212989e-05)
--(axis cs:10200,5.98337951263593e-05)
--(axis cs:10100,6.10873581622307e-05)
--(axis cs:10000,6.13929606518518e-05)
--(axis cs:9900,6.01620267022004e-05)
--(axis cs:9800,6.03484724637938e-05)
--(axis cs:9700,6.21695601389547e-05)
--(axis cs:9600,6.1119339995121e-05)
--(axis cs:9500,5.83959301369044e-05)
--(axis cs:9400,6.01851198790986e-05)
--(axis cs:9300,5.85909634487719e-05)
--(axis cs:9200,5.7390902848008e-05)
--(axis cs:9100,5.76553878795385e-05)
--(axis cs:9000,5.85478702586736e-05)
--(axis cs:8900,5.83001111406074e-05)
--(axis cs:8800,5.77998279104292e-05)
--(axis cs:8700,5.89545770872678e-05)
--(axis cs:8600,6.02451908995819e-05)
--(axis cs:8500,6.27622986152811e-05)
--(axis cs:8400,6.49630569652225e-05)
--(axis cs:8300,6.62792975340945e-05)
--(axis cs:8200,6.38595854677274e-05)
--(axis cs:8100,6.73654671419686e-05)
--(axis cs:8000,6.72054618533682e-05)
--(axis cs:7900,6.56651953937871e-05)
--(axis cs:7800,6.56937772214151e-05)
--(axis cs:7700,6.65257118150018e-05)
--(axis cs:7600,6.45381713692657e-05)
--(axis cs:7500,6.93051505329152e-05)
--(axis cs:7400,6.9704034162762e-05)
--(axis cs:7300,6.93117592347751e-05)
--(axis cs:7200,6.92929766666317e-05)
--(axis cs:7100,7.07249648269196e-05)
--(axis cs:7000,6.99428056503934e-05)
--(axis cs:6900,7.56039158835047e-05)
--(axis cs:6800,7.94906386385712e-05)
--(axis cs:6700,7.69414778243005e-05)
--(axis cs:6600,7.73126044793297e-05)
--(axis cs:6500,7.59698830093941e-05)
--(axis cs:6400,7.55309261574014e-05)
--(axis cs:6300,7.24992548117845e-05)
--(axis cs:6200,7.09441294415904e-05)
--(axis cs:6100,6.97511751875759e-05)
--(axis cs:6000,7.39075149254661e-05)
--(axis cs:5900,7.76214020027897e-05)
--(axis cs:5800,7.6667530394598e-05)
--(axis cs:5700,7.71926603472809e-05)
--(axis cs:5600,7.84601995372633e-05)
--(axis cs:5500,7.99338499077284e-05)
--(axis cs:5400,8.20192528141882e-05)
--(axis cs:5300,8.50702800546003e-05)
--(axis cs:5200,8.88243938268036e-05)
--(axis cs:5100,8.94076670350088e-05)
--(axis cs:5000,9.48983188467752e-05)
--(axis cs:4900,9.55010070684113e-05)
--(axis cs:4800,9.92151271792366e-05)
--(axis cs:4700,0.000101165263236401)
--(axis cs:4600,0.00010816631121382)
--(axis cs:4500,0.000111570544260725)
--(axis cs:4400,0.000109140962773298)
--(axis cs:4300,0.000103356775395859)
--(axis cs:4200,0.000104631785953497)
--(axis cs:4100,0.000103370446675145)
--(axis cs:4000,0.000105538947775534)
--(axis cs:3900,0.000107561824258525)
--(axis cs:3800,0.000111813005930569)
--(axis cs:3700,0.000111566569264532)
--(axis cs:3600,0.000112784911973526)
--(axis cs:3500,0.000115898386936931)
--(axis cs:3400,0.000117767426896847)
--(axis cs:3300,0.000130722811459259)
--(axis cs:3200,0.000135836618060633)
--(axis cs:3100,0.000140923699879308)
--(axis cs:3000,0.000149643347686472)
--(axis cs:2900,0.000153332140208977)
--(axis cs:2800,0.000153309726191441)
--(axis cs:2700,0.000152838796339955)
--(axis cs:2600,0.000147734518598429)
--(axis cs:2500,0.00014053650807651)
--(axis cs:2400,0.000154731657151862)
--(axis cs:2300,0.000150816833878571)
--(axis cs:2200,0.000156231594264872)
--(axis cs:2100,0.000156670534762726)
--(axis cs:2000,0.000167734768134591)
--(axis cs:1900,0.000171919730722768)
--(axis cs:1800,0.000177243061112989)
--(axis cs:1700,0.000189536650586251)
--(axis cs:1600,0.00019663661922965)
--(axis cs:1500,0.000197576977806279)
--(axis cs:1400,0.000204715766502191)
--(axis cs:1300,0.000216412745185997)
--(axis cs:1200,0.000222121371469727)
--(axis cs:1100,0.000232344064391201)
--(axis cs:1000,0.000248391880442246)
--(axis cs:900,0.000274278822499551)
--(axis cs:800,0.000289193789163781)
--(axis cs:700,0.000346820978302233)
--(axis cs:600,0.000558749793250035)
--(axis cs:500,0.000872374700310218)
--(axis cs:400,0.00158550812338741)
--(axis cs:300,0.00303829922734546)
--(axis cs:200,0.00456458383344036)
--(axis cs:100,0.00593542234886424)
--(axis cs:0,0.00720213678466435)
--cycle;

\path [fill=green!50.1960784313725!black, fill opacity=0.2, semithick]
(axis cs:0,0.00449837547693887)
--(axis cs:0,0.00445945200232925)
--(axis cs:100,0.00352351291189394)
--(axis cs:200,0.00246974431810779)
--(axis cs:300,0.00139723591805478)
--(axis cs:400,0.000421370500234841)
--(axis cs:500,0.000216971571399304)
--(axis cs:600,6.91006405808362e-05)
--(axis cs:700,4.63637142932481e-05)
--(axis cs:800,4.24799811598135e-05)
--(axis cs:900,4.15213910157181e-05)
--(axis cs:1000,4.0478461836091e-05)
--(axis cs:1100,3.75924312312409e-05)
--(axis cs:1200,3.56021672569982e-05)
--(axis cs:1300,3.31457199784438e-05)
--(axis cs:1400,3.06518838320572e-05)
--(axis cs:1500,2.83983358201886e-05)
--(axis cs:1600,2.40241218088796e-05)
--(axis cs:1700,1.9745692758179e-05)
--(axis cs:1800,1.64624814564277e-05)
--(axis cs:1900,1.32978115518751e-05)
--(axis cs:2000,1.03327662406265e-05)
--(axis cs:2100,8.07260090997263e-06)
--(axis cs:2200,8.29290126586312e-06)
--(axis cs:2300,9.27048956268279e-06)
--(axis cs:2400,9.44797900827402e-06)
--(axis cs:2500,8.63404210434559e-06)
--(axis cs:2600,8.29023022485574e-06)
--(axis cs:2700,8.41399354215724e-06)
--(axis cs:2800,7.64645779037612e-06)
--(axis cs:2900,6.62409801876726e-06)
--(axis cs:3000,5.86446345196679e-06)
--(axis cs:3100,6.33813767931426e-06)
--(axis cs:3200,6.09676840364437e-06)
--(axis cs:3300,5.38150144945564e-06)
--(axis cs:3400,5.0792154161001e-06)
--(axis cs:3500,5.4248875683209e-06)
--(axis cs:3600,5.60523339300165e-06)
--(axis cs:3700,4.65859504124485e-06)
--(axis cs:3800,5.54493732410941e-06)
--(axis cs:3900,7.29823998768081e-06)
--(axis cs:4000,7.55405075732103e-06)
--(axis cs:4100,7.57265195803507e-06)
--(axis cs:4200,6.62052326989399e-06)
--(axis cs:4300,4.89903037206679e-06)
--(axis cs:4400,3.32889378724159e-06)
--(axis cs:4500,3.39908289013855e-06)
--(axis cs:4600,2.98309937301594e-06)
--(axis cs:4700,3.11471838510394e-06)
--(axis cs:4800,4.19249322204491e-06)
--(axis cs:4900,5.09647022836376e-06)
--(axis cs:5000,5.01127723360426e-06)
--(axis cs:5100,4.94662450645089e-06)
--(axis cs:5200,3.8242925326116e-06)
--(axis cs:5300,3.36871805104896e-06)
--(axis cs:5400,3.25021855352917e-06)
--(axis cs:5500,2.98221489541751e-06)
--(axis cs:5600,2.94823781695411e-06)
--(axis cs:5700,2.90812043008226e-06)
--(axis cs:5800,3.86406425158883e-06)
--(axis cs:5900,2.86888852941347e-06)
--(axis cs:6000,2.66851615026582e-06)
--(axis cs:6100,2.0374045103609e-06)
--(axis cs:6200,1.95796915001008e-06)
--(axis cs:6300,2.06477645195743e-06)
--(axis cs:6400,2.60072651227414e-06)
--(axis cs:6500,3.61788715636313e-06)
--(axis cs:6600,4.38730125413529e-06)
--(axis cs:6700,3.5657669463309e-06)
--(axis cs:6800,2.88221395862267e-06)
--(axis cs:6900,2.85906968151521e-06)
--(axis cs:7000,2.68281896679848e-06)
--(axis cs:7100,2.45430058717989e-06)
--(axis cs:7200,2.07947565340931e-06)
--(axis cs:7300,1.63675386567432e-06)
--(axis cs:7400,1.64192193274382e-06)
--(axis cs:7500,1.44037692334462e-06)
--(axis cs:7600,3.7303380778439e-06)
--(axis cs:7700,3.76095979882007e-06)
--(axis cs:7800,3.33871441927903e-06)
--(axis cs:7900,2.04856485380417e-06)
--(axis cs:8000,1.79411681769998e-06)
--(axis cs:8100,1.63503915025145e-06)
--(axis cs:8200,1.72032580391565e-06)
--(axis cs:8300,1.7874774206667e-06)
--(axis cs:8400,1.97885601696949e-06)
--(axis cs:8500,2.14917846547462e-06)
--(axis cs:8600,2.39335736076688e-06)
--(axis cs:8700,2.09123897783466e-06)
--(axis cs:8800,1.90677128411918e-06)
--(axis cs:8900,1.94973716737513e-06)
--(axis cs:9000,2.01249387171979e-06)
--(axis cs:9100,2.15883856467456e-06)
--(axis cs:9200,1.7498822738093e-06)
--(axis cs:9300,1.19981254579661e-06)
--(axis cs:9400,1.38425716381686e-06)
--(axis cs:9500,1.26674987447627e-06)
--(axis cs:9600,1.00581652064655e-06)
--(axis cs:9700,1.14706576725308e-06)
--(axis cs:9800,1.33568486205104e-06)
--(axis cs:9900,1.1340092784812e-06)
--(axis cs:10000,9.64580993404274e-07)
--(axis cs:10100,1.4964353281989e-06)
--(axis cs:10200,1.08938301606765e-06)
--(axis cs:10300,7.89977619845803e-07)
--(axis cs:10400,9.63297112332554e-07)
--(axis cs:10500,3.16080095406717e-06)
--(axis cs:10600,2.11524423124246e-06)
--(axis cs:10700,1.84692817842832e-06)
--(axis cs:10800,1.91939513547296e-06)
--(axis cs:10900,2.17579439588671e-06)
--(axis cs:11000,1.73914009933789e-06)
--(axis cs:11100,1.08151008724651e-06)
--(axis cs:11200,1.01987991716817e-06)
--(axis cs:11300,1.05871913284336e-06)
--(axis cs:11400,1.18119814472279e-06)
--(axis cs:11500,1.32081721643084e-06)
--(axis cs:11600,1.44070107052567e-06)
--(axis cs:11700,1.60393920776416e-06)
--(axis cs:11800,1.38865207437599e-06)
--(axis cs:11900,1.28274418224753e-06)
--(axis cs:12000,1.28447879527369e-06)
--(axis cs:12100,1.3611302145807e-06)
--(axis cs:12200,1.29062446651353e-06)
--(axis cs:12300,1.09106861162727e-06)
--(axis cs:12400,1.4898247830599e-06)
--(axis cs:12500,1.84846577030112e-06)
--(axis cs:12600,2.14017433299595e-06)
--(axis cs:12700,1.79835494820691e-06)
--(axis cs:12800,1.52634928469357e-06)
--(axis cs:12900,1.16920145212692e-06)
--(axis cs:13000,1.0363116150529e-06)
--(axis cs:13100,1.2189664101681e-06)
--(axis cs:13200,1.02901454194821e-06)
--(axis cs:13300,1.13029670642714e-06)
--(axis cs:13400,1.18069721664129e-06)
--(axis cs:13500,1.17416440260043e-06)
--(axis cs:13600,1.30959653594775e-06)
--(axis cs:13700,1.08750432740075e-06)
--(axis cs:13800,1.13198490658828e-06)
--(axis cs:13900,1.19216911399216e-06)
--(axis cs:14000,1.17536917526159e-06)
--(axis cs:14100,1.1764806912782e-06)
--(axis cs:14200,9.33928595951547e-07)
--(axis cs:14300,8.95431794781332e-07)
--(axis cs:14400,8.96653418112718e-07)
--(axis cs:14500,8.17962215314668e-07)
--(axis cs:14600,7.48350548697843e-07)
--(axis cs:14700,7.49843657966543e-07)
--(axis cs:14800,9.06537027758013e-07)
--(axis cs:14900,1.05878452241717e-06)
--(axis cs:15000,1.16693563474571e-06)
--(axis cs:15100,1.1202556632813e-06)
--(axis cs:15200,1.06783214657186e-06)
--(axis cs:15300,1.15694915625948e-06)
--(axis cs:15400,1.1336248534076e-06)
--(axis cs:15500,1.14860615727918e-06)
--(axis cs:15600,1.15545360029924e-06)
--(axis cs:15700,1.17784168862599e-06)
--(axis cs:15800,8.91993920469887e-07)
--(axis cs:15900,8.72812258874893e-07)
--(axis cs:16000,9.2726008512246e-07)
--(axis cs:16100,9.22806993191877e-07)
--(axis cs:16200,9.89536219783453e-07)
--(axis cs:16300,1.01789984919965e-06)
--(axis cs:16400,1.13888275730859e-06)
--(axis cs:16500,1.09271618544443e-06)
--(axis cs:16600,1.15272084037823e-06)
--(axis cs:16700,1.16111347291579e-06)
--(axis cs:16800,1.16643964728845e-06)
--(axis cs:16900,1.17694745111674e-06)
--(axis cs:17000,9.2225779297503e-07)
--(axis cs:17100,8.68480498694259e-07)
--(axis cs:17200,7.50128619257662e-07)
--(axis cs:17300,7.21676023189354e-07)
--(axis cs:17400,6.88200420964277e-07)
--(axis cs:17500,7.21302507223292e-07)
--(axis cs:17600,9.67895674190774e-07)
--(axis cs:17700,1.25651267156862e-06)
--(axis cs:17800,1.25932682884233e-06)
--(axis cs:17900,1.12851759439886e-06)
--(axis cs:18000,1.10385384400018e-06)
--(axis cs:18100,9.81499530024514e-07)
--(axis cs:18200,7.86068978843684e-07)
--(axis cs:18300,7.62663657789036e-07)
--(axis cs:18400,8.64752885536999e-07)
--(axis cs:18500,9.17892168856732e-07)
--(axis cs:18600,1.08026046420359e-06)
--(axis cs:18700,1.15645968556931e-06)
--(axis cs:18800,9.66568223626273e-07)
--(axis cs:18900,8.16289166475721e-07)
--(axis cs:19000,8.81218332408752e-07)
--(axis cs:19100,9.13682890642854e-07)
--(axis cs:19200,8.69407958111729e-07)
--(axis cs:19300,8.75135654400552e-07)
--(axis cs:19400,8.8016426792582e-07)
--(axis cs:19500,8.78864402996416e-07)
--(axis cs:19600,9.4109696885563e-07)
--(axis cs:19700,1.13467412881162e-06)
--(axis cs:19800,8.88583413228817e-07)
--(axis cs:19900,8.50456678732006e-07)
--(axis cs:20000,8.30955843575499e-07)
--(axis cs:20100,7.62059729339421e-07)
--(axis cs:20200,7.45455258382823e-07)
--(axis cs:20300,7.43392132456848e-07)
--(axis cs:20400,7.41484944209227e-07)
--(axis cs:20500,7.85318216632383e-07)
--(axis cs:20600,8.26704986907649e-07)
--(axis cs:20700,8.6156122463453e-07)
--(axis cs:20800,9.40350047196766e-07)
--(axis cs:20900,1.04589411351445e-06)
--(axis cs:21000,1.02801791918053e-06)
--(axis cs:21100,9.85953472655906e-07)
--(axis cs:21200,8.51849874204178e-07)
--(axis cs:21300,6.92058664301961e-07)
--(axis cs:21400,6.96528797418244e-07)
--(axis cs:21500,7.50293746110954e-07)
--(axis cs:21600,7.52624525249565e-07)
--(axis cs:21700,7.37993228552054e-07)
--(axis cs:21800,7.86783628401386e-07)
--(axis cs:21900,8.08500205891203e-07)
--(axis cs:22000,8.30197691384983e-07)
--(axis cs:22100,8.09689607603351e-07)
--(axis cs:22200,7.74563721434166e-07)
--(axis cs:22300,7.38805985695783e-07)
--(axis cs:22400,7.5686096417335e-07)
--(axis cs:22500,7.08669161387273e-07)
--(axis cs:22600,7.00556281926737e-07)
--(axis cs:22700,7.20375852049946e-07)
--(axis cs:22800,7.34747689829762e-07)
--(axis cs:22900,7.44516696567714e-07)
--(axis cs:23000,7.48417041480538e-07)
--(axis cs:23100,7.44362294661131e-07)
--(axis cs:23200,7.43339319616696e-07)
--(axis cs:23300,7.04413875259323e-07)
--(axis cs:23400,6.96482909035663e-07)
--(axis cs:23500,7.15576916664534e-07)
--(axis cs:23600,7.01943419844788e-07)
--(axis cs:23700,6.89241940548449e-07)
--(axis cs:23800,6.78289604885683e-07)
--(axis cs:23900,6.76664719078444e-07)
--(axis cs:24000,6.75618145123006e-07)
--(axis cs:24100,6.52205592196682e-07)
--(axis cs:24200,6.51264262979963e-07)
--(axis cs:24300,6.52336179876227e-07)
--(axis cs:24400,6.57396116609503e-07)
--(axis cs:24500,6.71039983455245e-07)
--(axis cs:24600,6.81025202583525e-07)
--(axis cs:24700,6.86328362581838e-07)
--(axis cs:24800,6.92713636219897e-07)
--(axis cs:24900,6.88766045498569e-07)
--(axis cs:25000,6.58902087501817e-07)
--(axis cs:25100,6.52223718092291e-07)
--(axis cs:25200,6.58080766591838e-07)
--(axis cs:25300,6.69998120240141e-07)
--(axis cs:25400,6.78555736302025e-07)
--(axis cs:25500,6.45330933887989e-07)
--(axis cs:25600,6.28560536826791e-07)
--(axis cs:25700,6.23585294005598e-07)
--(axis cs:25800,6.40790121215028e-07)
--(axis cs:25900,6.55680734698577e-07)
--(axis cs:26000,6.656685871104e-07)
--(axis cs:26100,6.75138779025977e-07)
--(axis cs:26200,6.82958176267104e-07)
--(axis cs:26300,6.87832627067779e-07)
--(axis cs:26400,6.27604226880886e-07)
--(axis cs:26500,6.24671495204417e-07)
--(axis cs:26600,6.15967672639773e-07)
--(axis cs:26700,6.20228189855352e-07)
--(axis cs:26800,6.22344903600859e-07)
--(axis cs:26900,6.24896461230576e-07)
--(axis cs:27000,6.22154168692314e-07)
--(axis cs:27100,6.23391673505881e-07)
--(axis cs:27200,6.28321679936884e-07)
--(axis cs:27300,6.23109631903793e-07)
--(axis cs:27400,6.20127382330595e-07)
--(axis cs:27500,6.19483361916895e-07)
--(axis cs:27600,6.20820352091082e-07)
--(axis cs:27700,6.24596320926956e-07)
--(axis cs:27800,6.16587829768518e-07)
--(axis cs:27900,6.20374478223586e-07)
--(axis cs:28000,6.13044793506284e-07)
--(axis cs:28100,6.08137308263284e-07)
--(axis cs:28200,6.01015315178087e-07)
--(axis cs:28300,5.99848913815914e-07)
--(axis cs:28400,5.93979597285368e-07)
--(axis cs:28500,5.95352882744806e-07)
--(axis cs:28600,5.91386179061839e-07)
--(axis cs:28700,5.89659418042565e-07)
--(axis cs:28800,5.92259216720724e-07)
--(axis cs:28900,5.9142527519535e-07)
--(axis cs:29000,5.88848052361848e-07)
--(axis cs:29100,5.9146064865902e-07)
--(axis cs:29200,5.88905003916932e-07)
--(axis cs:29300,5.86003464254472e-07)
--(axis cs:29400,5.83239884529111e-07)
--(axis cs:29500,5.84348976688852e-07)
--(axis cs:29500,6.04817286134616e-07)
--(axis cs:29500,6.04817286134616e-07)
--(axis cs:29400,6.06831916694177e-07)
--(axis cs:29300,6.08622608950576e-07)
--(axis cs:29200,6.08594147892771e-07)
--(axis cs:29100,6.10892734064211e-07)
--(axis cs:29000,6.11591101704316e-07)
--(axis cs:28900,6.13002573993155e-07)
--(axis cs:28800,6.10038717142189e-07)
--(axis cs:28700,6.12776387638014e-07)
--(axis cs:28600,6.16021750782986e-07)
--(axis cs:28500,6.1942385654413e-07)
--(axis cs:28400,7.23076316525929e-07)
--(axis cs:28300,7.27595422798852e-07)
--(axis cs:28200,7.28486616775234e-07)
--(axis cs:28100,7.29521631559196e-07)
--(axis cs:28000,7.30585934002772e-07)
--(axis cs:27900,6.41570278231513e-07)
--(axis cs:27800,6.48708907305577e-07)
--(axis cs:27700,6.49687193928337e-07)
--(axis cs:27600,6.46208434272192e-07)
--(axis cs:27500,6.45249344438773e-07)
--(axis cs:27400,6.31955177376359e-07)
--(axis cs:27300,6.35182176977248e-07)
--(axis cs:27200,6.43874067093123e-07)
--(axis cs:27100,6.65985125719887e-07)
--(axis cs:27000,6.79161923702386e-07)
--(axis cs:26900,6.83013452593732e-07)
--(axis cs:26800,6.75496229332919e-07)
--(axis cs:26700,6.75009143117599e-07)
--(axis cs:26600,6.85815369493063e-07)
--(axis cs:26500,7.85026867696788e-07)
--(axis cs:26400,7.91631794742382e-07)
--(axis cs:26300,8.0508887419934e-07)
--(axis cs:26200,8.17877846423436e-07)
--(axis cs:26100,8.1797780127555e-07)
--(axis cs:26000,7.31848140179464e-07)
--(axis cs:25900,7.31437701770305e-07)
--(axis cs:25800,7.33557493816458e-07)
--(axis cs:25700,7.64702002316635e-07)
--(axis cs:25600,7.70694447053592e-07)
--(axis cs:25500,7.71535050650173e-07)
--(axis cs:25400,8.23948807472776e-07)
--(axis cs:25300,7.93918458119062e-07)
--(axis cs:25200,8.11048557913209e-07)
--(axis cs:25100,8.39118453204322e-07)
--(axis cs:25000,8.08155188278039e-07)
--(axis cs:24900,7.13491339553939e-07)
--(axis cs:24800,7.11837267096807e-07)
--(axis cs:24700,6.9660360156268e-07)
--(axis cs:24600,6.86504355099631e-07)
--(axis cs:24500,7.3037852157996e-07)
--(axis cs:24400,7.70758303951635e-07)
--(axis cs:24300,7.85027041281057e-07)
--(axis cs:24200,7.95592536722837e-07)
--(axis cs:24100,7.89154009313173e-07)
--(axis cs:24000,7.46513919846137e-07)
--(axis cs:23900,7.34411391871742e-07)
--(axis cs:23800,7.54587624604576e-07)
--(axis cs:23700,7.52295239801927e-07)
--(axis cs:23600,7.63116135664379e-07)
--(axis cs:23500,8.58524429434129e-07)
--(axis cs:23400,8.89725562320898e-07)
--(axis cs:23300,8.93245248079397e-07)
--(axis cs:23200,8.95799295326478e-07)
--(axis cs:23100,8.93264489976653e-07)
--(axis cs:23000,7.97213035305597e-07)
--(axis cs:22900,8.08748989933297e-07)
--(axis cs:22800,8.64801909196063e-07)
--(axis cs:22700,8.33509617194712e-07)
--(axis cs:22600,8.38634769428031e-07)
--(axis cs:22500,8.44508220757319e-07)
--(axis cs:22400,8.04007893398175e-07)
--(axis cs:22300,7.85920340656028e-07)
--(axis cs:22200,8.35344870662403e-07)
--(axis cs:22100,8.49547733697117e-07)
--(axis cs:22000,8.4213882925671e-07)
--(axis cs:21900,9.12248293295002e-07)
--(axis cs:21800,8.91068159061328e-07)
--(axis cs:21700,8.52026055921426e-07)
--(axis cs:21600,8.06350491504458e-07)
--(axis cs:21500,7.94084706803968e-07)
--(axis cs:21400,8.06027723978762e-07)
--(axis cs:21300,9.5940837869742e-07)
--(axis cs:21200,1.27884557046823e-06)
--(axis cs:21100,1.32145947558035e-06)
--(axis cs:21000,1.32329029774966e-06)
--(axis cs:20900,1.33757887618691e-06)
--(axis cs:20800,1.36910109382441e-06)
--(axis cs:20700,9.94992780888489e-07)
--(axis cs:20600,8.56827026977621e-07)
--(axis cs:20500,8.51859990060242e-07)
--(axis cs:20400,8.29981383522969e-07)
--(axis cs:20300,8.16271485473255e-07)
--(axis cs:20200,8.95950901171688e-07)
--(axis cs:20100,1.11340082172756e-06)
--(axis cs:20000,1.22762864625989e-06)
--(axis cs:19900,1.26209012506879e-06)
--(axis cs:19800,1.22826896122754e-06)
--(axis cs:19700,1.20833685890377e-06)
--(axis cs:19600,1.18178350616759e-06)
--(axis cs:19500,1.15354191135978e-06)
--(axis cs:19400,1.20144281457149e-06)
--(axis cs:19300,1.18292558797466e-06)
--(axis cs:19200,1.0383925419851e-06)
--(axis cs:19100,1.17335654307516e-06)
--(axis cs:19000,1.2887435683059e-06)
--(axis cs:18900,1.35071629286573e-06)
--(axis cs:18800,1.44844099463697e-06)
--(axis cs:18700,1.26830619774019e-06)
--(axis cs:18600,1.18690206083083e-06)
--(axis cs:18500,1.29423661197885e-06)
--(axis cs:18400,1.30971393949272e-06)
--(axis cs:18300,1.20511607005523e-06)
--(axis cs:18200,1.11533656084008e-06)
--(axis cs:18100,1.29413677230456e-06)
--(axis cs:18000,1.35165925090093e-06)
--(axis cs:17900,1.36617718405916e-06)
--(axis cs:17800,1.34864034575996e-06)
--(axis cs:17700,1.35723996557234e-06)
--(axis cs:17600,1.43770323734603e-06)
--(axis cs:17500,1.55538054013718e-06)
--(axis cs:17400,1.55626909712989e-06)
--(axis cs:17300,1.56394858490739e-06)
--(axis cs:17200,1.51858016803572e-06)
--(axis cs:17100,1.32958915387974e-06)
--(axis cs:17000,1.30602667572953e-06)
--(axis cs:16900,2.24305478442677e-06)
--(axis cs:16800,2.37747090344851e-06)
--(axis cs:16700,2.3776580765374e-06)
--(axis cs:16600,2.3646253406918e-06)
--(axis cs:16500,2.44682835113491e-06)
--(axis cs:16400,1.2424552769507e-06)
--(axis cs:16300,1.15628025004621e-06)
--(axis cs:16200,1.19635500314803e-06)
--(axis cs:16100,1.27878377569916e-06)
--(axis cs:16000,1.26760115057122e-06)
--(axis cs:15900,1.53713716751398e-06)
--(axis cs:15800,1.59668336061367e-06)
--(axis cs:15700,1.63672736350818e-06)
--(axis cs:15600,1.72335823158271e-06)
--(axis cs:15500,1.73973625442441e-06)
--(axis cs:15400,1.61406940952397e-06)
--(axis cs:15300,1.6218061242523e-06)
--(axis cs:15200,1.54932273592862e-06)
--(axis cs:15100,1.48078674750676e-06)
--(axis cs:15000,1.59082414247458e-06)
--(axis cs:14900,1.64440357938753e-06)
--(axis cs:14800,1.62011059604741e-06)
--(axis cs:14700,1.67634083244141e-06)
--(axis cs:14600,1.55026098435656e-06)
--(axis cs:14500,1.14816864411002e-06)
--(axis cs:14400,1.12840435337297e-06)
--(axis cs:14300,1.53728311769639e-06)
--(axis cs:14200,1.72322293041249e-06)
--(axis cs:14100,2.28017649995824e-06)
--(axis cs:14000,2.53679374194422e-06)
--(axis cs:13900,2.52459662705424e-06)
--(axis cs:13800,2.56923831275883e-06)
--(axis cs:13700,2.52727410355221e-06)
--(axis cs:13600,1.88625601612962e-06)
--(axis cs:13500,1.95303587414567e-06)
--(axis cs:13400,1.97262392983867e-06)
--(axis cs:13300,1.6412481683011e-06)
--(axis cs:13200,1.59421542409959e-06)
--(axis cs:13100,1.30874731574762e-06)
--(axis cs:13000,2.09197976732868e-06)
--(axis cs:12900,2.70297615149854e-06)
--(axis cs:12800,3.60540692639174e-06)
--(axis cs:12700,3.5994387404371e-06)
--(axis cs:12600,3.40509531609909e-06)
--(axis cs:12500,3.21752741790502e-06)
--(axis cs:12400,2.76462939019449e-06)
--(axis cs:12300,2.09152528879204e-06)
--(axis cs:12200,1.95107173444089e-06)
--(axis cs:12100,1.96377015419598e-06)
--(axis cs:12000,2.0341909133078e-06)
--(axis cs:11900,2.15171569181938e-06)
--(axis cs:11800,2.05000742179284e-06)
--(axis cs:11700,1.6992992254783e-06)
--(axis cs:11600,1.57668934735529e-06)
--(axis cs:11500,1.6047538071697e-06)
--(axis cs:11400,1.70819407397769e-06)
--(axis cs:11300,1.91465308297647e-06)
--(axis cs:11200,2.050361063513e-06)
--(axis cs:11100,2.05851969608262e-06)
--(axis cs:11000,1.95170602799391e-06)
--(axis cs:10900,4.07745529816812e-06)
--(axis cs:10800,4.47497509132286e-06)
--(axis cs:10700,4.50802397197936e-06)
--(axis cs:10600,4.34127663432216e-06)
--(axis cs:10500,4.67438764152061e-06)
--(axis cs:10400,4.31094545758301e-06)
--(axis cs:10300,4.34380228516305e-06)
--(axis cs:10200,4.22946611561073e-06)
--(axis cs:10100,3.97931162881879e-06)
--(axis cs:10000,2.56323804189403e-06)
--(axis cs:9900,2.6782195578902e-06)
--(axis cs:9800,3.18944271063067e-06)
--(axis cs:9700,3.06477712403172e-06)
--(axis cs:9600,2.88245841160453e-06)
--(axis cs:9500,3.11380442041162e-06)
--(axis cs:9400,2.96116873191853e-06)
--(axis cs:9300,3.195310141332e-06)
--(axis cs:9200,3.75575795506627e-06)
--(axis cs:9100,4.11603298651462e-06)
--(axis cs:9000,4.25423439739111e-06)
--(axis cs:8900,4.31851276216306e-06)
--(axis cs:8800,3.87195141374977e-06)
--(axis cs:8700,2.93184714556664e-06)
--(axis cs:8600,2.71982573311125e-06)
--(axis cs:8500,3.04193584910979e-06)
--(axis cs:8400,2.95234647908808e-06)
--(axis cs:8300,2.61671971953236e-06)
--(axis cs:8200,2.3312325917671e-06)
--(axis cs:8100,1.8842893124167e-06)
--(axis cs:8000,4.71714903507478e-06)
--(axis cs:7900,4.85269075063334e-06)
--(axis cs:7800,4.85133793897995e-06)
--(axis cs:7700,4.87280273737201e-06)
--(axis cs:7600,4.58362294424817e-06)
--(axis cs:7500,3.56574935213063e-06)
--(axis cs:7400,3.57389703189959e-06)
--(axis cs:7300,4.14065567342771e-06)
--(axis cs:7200,4.36689998065598e-06)
--(axis cs:7100,4.75496879790164e-06)
--(axis cs:7000,5.06589034022946e-06)
--(axis cs:6900,5.75781014705978e-06)
--(axis cs:6800,5.37227505333802e-06)
--(axis cs:6700,5.00199217995322e-06)
--(axis cs:6600,4.74586491374977e-06)
--(axis cs:6500,5.5039383098701e-06)
--(axis cs:6400,5.41773075300558e-06)
--(axis cs:6300,4.70672039135151e-06)
--(axis cs:6200,4.62987256414989e-06)
--(axis cs:6100,3.76013592089438e-06)
--(axis cs:6000,3.47458932435501e-06)
--(axis cs:5900,3.74045879329973e-06)
--(axis cs:5800,4.11534884573288e-06)
--(axis cs:5700,5.32758677353281e-06)
--(axis cs:5600,7.80671010835251e-06)
--(axis cs:5500,7.47421113006718e-06)
--(axis cs:5400,7.44840099976627e-06)
--(axis cs:5300,7.13161383116382e-06)
--(axis cs:5200,7.38178674422969e-06)
--(axis cs:5100,6.61684380573406e-06)
--(axis cs:5000,6.49056499088113e-06)
--(axis cs:4900,6.37542078945126e-06)
--(axis cs:4800,7.04862624812106e-06)
--(axis cs:4700,7.60686075560795e-06)
--(axis cs:4600,5.10633767822371e-06)
--(axis cs:4500,5.27298304573519e-06)
--(axis cs:4400,5.59832509676495e-06)
--(axis cs:4300,6.2558092465692e-06)
--(axis cs:4200,8.37733640109034e-06)
--(axis cs:4100,8.66518741444429e-06)
--(axis cs:4000,1.00811280591934e-05)
--(axis cs:3900,1.08441817591591e-05)
--(axis cs:3800,1.09638078085353e-05)
--(axis cs:3700,7.84404918072293e-06)
--(axis cs:3600,6.99824365680163e-06)
--(axis cs:3500,6.76591386999192e-06)
--(axis cs:3400,7.51909318752844e-06)
--(axis cs:3300,7.4413810108097e-06)
--(axis cs:3200,8.20191042445825e-06)
--(axis cs:3100,8.814398482308e-06)
--(axis cs:3000,9.51176756997951e-06)
--(axis cs:2900,1.03466451687419e-05)
--(axis cs:2800,1.07658964057158e-05)
--(axis cs:2700,1.10564136754868e-05)
--(axis cs:2600,1.1758444274314e-05)
--(axis cs:2500,1.20280649251961e-05)
--(axis cs:2400,1.16522659980114e-05)
--(axis cs:2300,1.1812078443946e-05)
--(axis cs:2200,1.17667810902141e-05)
--(axis cs:2100,1.25679719528822e-05)
--(axis cs:2000,1.29472639291694e-05)
--(axis cs:1900,1.47786087606976e-05)
--(axis cs:1800,1.88480951843402e-05)
--(axis cs:1700,2.56473911703232e-05)
--(axis cs:1600,2.92669402588489e-05)
--(axis cs:1500,3.31754268301802e-05)
--(axis cs:1400,3.61268503002799e-05)
--(axis cs:1300,3.89621663447182e-05)
--(axis cs:1200,3.89650742304832e-05)
--(axis cs:1100,4.0758197863592e-05)
--(axis cs:1000,4.3458086296048e-05)
--(axis cs:900,4.91640433909052e-05)
--(axis cs:800,5.05134214415614e-05)
--(axis cs:700,5.43925651324475e-05)
--(axis cs:600,0.000135188613841153)
--(axis cs:500,0.000283869671890263)
--(axis cs:400,0.000497289821387315)
--(axis cs:300,0.00147499705103882)
--(axis cs:200,0.00255209079266337)
--(axis cs:100,0.00356445703881679)
--(axis cs:0,0.00449837547693887)
--cycle;

\addplot [ultra thick, red]
table {%
0 0.00793405342847109
100 0.00659654662013054
200 0.00508389482274652
300 0.00342376297339797
400 0.00182917073834687
500 0.00101173517759889
600 0.000637519755400717
700 0.000427102640969679
800 0.00036658052704297
900 0.000332209019688889
1000 0.000307628040900454
1100 0.000281147571513429
1200 0.000265089067397639
1400 0.000238726614043117
1500 0.000233736995141953
1700 0.000231615340453573
1900 0.000227314420044422
2000 0.000221258102101274
2100 0.000210850135772489
2200 0.000204190248041414
2300 0.000202144496142864
2400 0.000201189948711544
2500 0.000199273665202782
2600 0.00020576428505592
2700 0.000205204531084746
2800 0.00020130374468863
2900 0.00020063306146767
3000 0.00019834291015286
3100 0.00018788491433952
3300 0.00018049510254059
3400 0.000179234571987763
3500 0.000181931027327664
3600 0.000181396273546852
3700 0.00017959535762202
3800 0.000179362235940062
3900 0.000176450164872222
4000 0.000176762463524938
4100 0.000178749149199575
4200 0.000177824331331067
4400 0.000173895081388764
4500 0.000165694698807783
4600 0.000163775039254688
4800 0.000155528119648807
4900 0.00015576378791593
5000 0.000154546869453043
5100 0.000149956016684882
5200 0.000152601554873399
5300 0.0001536166673759
5400 0.000146753765875474
5500 0.000147121274494566
5600 0.000145179888932034
5700 0.000139716037665494
5800 0.000136467526317574
5900 0.000135597219923511
6000 0.000133604582515545
6100 0.00013084830425214
6200 0.000129231149912812
6300 0.00012983416672796
6400 0.000136511953314766
6500 0.00013915533781983
6600 0.000140681659104303
6800 0.000137996335979551
6900 0.000128596482682042
7000 0.000120703109132592
7100 0.000119993594125845
7200 0.000118506948638242
7300 0.000116378352686297
7500 0.000115315262519289
7600 0.000111335757537745
7700 0.000113365967990831
7800 0.000113493122626096
8000 0.000111313333036378
8100 0.000116250383143779
8300 0.000113271344162058
8500 0.000109320419142023
8600 0.000103790160210337
8700 0.000101606339740101
8800 0.000100322220532689
9000 0.000101782818092033
9100 0.000101495286799036
9300 0.000100200028100517
9400 9.98047544271685e-05
9500 9.86917439149693e-05
9600 9.69652537605725e-05
9900 9.59583630901761e-05
10000 9.66098887147382e-05
10100 9.94038346107118e-05
10200 9.90952248685062e-05
10300 9.96846138150431e-05
10400 9.81642515398562e-05
10500 9.9622251582332e-05
10700 9.95557711576112e-05
10800 9.78181342361495e-05
10900 9.77704621618614e-05
11000 9.52391565078869e-05
11100 9.18297955649905e-05
11200 9.20317688724026e-05
11300 9.31809190660715e-05
11400 9.50827525230125e-05
11500 9.57913071033545e-05
11700 9.51602414716035e-05
12000 9.10594098968431e-05
12500 8.87197820702568e-05
12600 8.9238936197944e-05
12800 8.91438467078842e-05
12900 8.77901256899349e-05
13000 8.78737409948371e-05
13200 8.91607778612524e-05
13300 8.88558715814725e-05
13400 8.98008511285298e-05
13500 9.12036921363324e-05
13600 8.97182617336512e-05
13700 8.78601349540986e-05
14000 8.5560699517373e-05
14100 8.57870254549198e-05
14200 8.53119272505865e-05
14400 8.55911421240307e-05
14500 8.38519044918939e-05
14700 8.43777670525014e-05
14800 8.23796872282401e-05
15000 8.08659824542701e-05
15100 8.06691168691032e-05
15200 8.00053603597917e-05
15500 8.30692442832515e-05
15600 8.20611021481454e-05
15800 8.24307135189883e-05
16000 8.1273028627038e-05
16100 8.0574223829899e-05
16200 8.08096228865907e-05
16500 7.89683108450845e-05
16600 7.9091259976849e-05
16700 7.81030976213515e-05
16900 7.74104628362693e-05
17100 7.77891837060452e-05
17200 7.76119049987756e-05
17300 7.8911536547821e-05
17400 7.91970160207711e-05
17700 7.8248413046822e-05
17800 7.60167749831453e-05
17900 7.4651870818343e-05
18100 7.52232881495729e-05
18300 7.55993605707772e-05
18400 7.61885676183738e-05
18500 7.57144880481064e-05
18600 7.45309007470496e-05
18700 7.46340010664426e-05
18800 7.51497354940511e-05
18900 7.46763762435876e-05
19100 7.61223491281271e-05
19300 7.59642935008742e-05
19500 7.54480279283598e-05
19600 7.46482619433664e-05
19700 7.50154431443661e-05
20000 7.40940595278516e-05
20100 7.45435900171287e-05
20200 7.43233395041898e-05
20300 7.4767776823137e-05
20400 7.62084819143638e-05
20500 7.63319985708222e-05
20800 7.4239338573534e-05
20900 7.31123582227156e-05
21000 7.25473364582285e-05
21600 7.15240530553274e-05
21800 7.20129974070005e-05
21900 7.27218284737319e-05
22000 7.2204515163321e-05
22100 7.2547969466541e-05
22200 7.18335068086162e-05
22300 7.22650293027982e-05
22400 7.16924623702653e-05
22500 7.16568174539134e-05
22600 7.02793913660571e-05
22800 6.92642206558958e-05
23000 6.85819395584986e-05
23100 6.90122687956318e-05
23200 7.01872413628735e-05
23300 6.9899542722851e-05
23400 7.02636534697376e-05
23600 7.15884016244672e-05
23700 7.07542349118739e-05
23900 7.05920538166538e-05
24100 6.97711802786216e-05
24200 6.99813244864345e-05
24500 6.96653150953352e-05
24700 6.85198465362191e-05
24800 6.84973565512337e-05
25000 6.7615786974784e-05
25100 6.80000957800075e-05
25200 6.77799762343056e-05
25500 6.83770558680408e-05
25600 6.77743228152394e-05
25700 6.81109086144716e-05
25800 6.78088545100763e-05
25900 6.79001241223887e-05
26000 6.74397670081817e-05
26100 6.7610882979352e-05
26200 6.71639936626889e-05
26300 6.73351460136473e-05
26400 6.71810339554213e-05
26500 6.7537504946813e-05
26600 6.74163020448759e-05
26700 6.78006690577604e-05
26800 6.7653731093742e-05
26900 6.78499709465541e-05
27100 6.69546716380864e-05
27200 6.65581392240711e-05
27400 6.65581392240711e-05
27600 6.70865338179283e-05
27700 6.7146225774195e-05
27900 6.66992564219981e-05
29000 6.72886599204503e-05
29200 6.70099761919118e-05
29400 6.71762390993536e-05
29500 6.69583459966816e-05
}; \addlegendentry{Baseline}

\addplot [ultra thick, blue]
table {%
0 0.00713266292586923
100 0.00585381686687469
200 0.00446937792003155
300 0.00292959995567799
400 0.0014729923568666
500 0.00082353682955727
600 0.000527653901372105
700 0.000327464804286137
800 0.000287563510937616
900 0.000269933487288654
1100 0.00022187405556906
1200 0.000210411322768778
1300 0.000202334675122984
1400 0.000193461324670352
1600 0.000182937350473367
1700 0.000176460918737575
1800 0.000168806567671709
1900 0.000163733959197998
2000 0.000161307994858362
2100 0.000155167377670296
2200 0.000150609761476517
2300 0.000143839264637791
2400 0.000142801553010941
2500 0.000136389033286832
2600 0.000140332078444771
2800 0.000143211844260804
2900 0.000138361123390496
3000 0.000137580442242324
3100 0.000133536392240785
3200 0.000128499304992147
3300 0.000121743527415674
3400 0.000117199655505829
3500 0.000113784022687469
3700 0.00010468480468262
3800 0.000104768165329006
3900 0.000103354395832866
4000 0.000103076519735623
4100 0.000100669960374944
4200 0.000101901678135619
4300 9.98369796434417e-05
4400 0.000101587378594559
4500 0.000100801189546473
4600 0.000101453173556365
4700 9.65851795626804e-05
4800 9.36303113121539e-05
4900 8.92090538400225e-05
5100 8.40944776427932e-05
5200 8.35357059258968e-05
5300 8.17916079540737e-05
5400 7.83899522502907e-05
5500 7.70212427596562e-05
5600 7.60818220442161e-05
5700 7.38685703254305e-05
5900 7.34010318410583e-05
6000 7.15118876541965e-05
6100 6.79179429425858e-05
6200 6.79472577758133e-05
6300 6.75207484164275e-05
6400 7.05915153957903e-05
6500 7.13030240149237e-05
6600 7.30591564206406e-05
6700 7.30759202269837e-05
6800 7.37523587304167e-05
6900 7.03525802236982e-05
7000 6.82377067278139e-05
7100 6.9061316025909e-05
7200 6.72817914164625e-05
7300 6.64671460981481e-05
7400 6.61660669720732e-05
7500 6.51553491479717e-05
7600 6.27879562671296e-05
7700 6.46648768451996e-05
7900 6.3234954723157e-05
8000 6.46249172859825e-05
8100 6.47248307359405e-05
8200 6.24350213911384e-05
8300 6.36571712675504e-05
8400 6.27443369012326e-05
8500 6.02698819420766e-05
8600 5.99148515902925e-05
8700 5.86965252296068e-05
8800 5.62677923880983e-05
8900 5.61629894946236e-05
9000 5.70373449590988e-05
9100 5.59424152015708e-05
9200 5.61162669328041e-05
9300 5.78313920414075e-05
9400 5.75635494897142e-05
9500 5.68996110814624e-05
9700 5.90866839047521e-05
9800 5.83280852879398e-05
9900 5.81168751523364e-05
10000 5.88515940762591e-05
10100 5.93128133914433e-05
10300 5.59066793357488e-05
10400 5.5451240768889e-05
10500 5.65238333365414e-05
10600 5.86967180424836e-05
10700 5.8324949350208e-05
10800 5.75684789509978e-05
10900 5.63816429348662e-05
11000 5.41459885425866e-05
11100 5.03419505548663e-05
11300 5.2260951633798e-05
11400 5.36256411578506e-05
11500 5.46011360711418e-05
11600 5.40880537300836e-05
11700 5.47399176866747e-05
11800 5.50387158000376e-05
11900 5.41352892469149e-05
12000 5.23164126207121e-05
12200 5.03150404256303e-05
12300 4.93922525492962e-05
12400 4.94614978379104e-05
12500 5.0262751756236e-05
12600 4.99896632391028e-05
12700 5.05691932630725e-05
12800 5.07604418089613e-05
12900 5.02477996633388e-05
13000 5.01809772686101e-05
13100 5.24027600476984e-05
13300 4.96385837323032e-05
13400 4.97410983371083e-05
13500 4.88508740090765e-05
13600 4.70303348265588e-05
13800 4.69724327558652e-05
13900 4.78893271065317e-05
14000 4.81093520647846e-05
14200 4.6702192776138e-05
14300 4.6875728003215e-05
14400 4.61683448520489e-05
14500 4.67048594146036e-05
14600 4.81821443827357e-05
14700 4.92927865707316e-05
14900 4.90562488266733e-05
15000 4.79381451441441e-05
15100 4.81413226225413e-05
15200 4.73553227493539e-05
15300 4.75259075756185e-05
15400 4.70261002192274e-05
15500 4.69433034595568e-05
15600 4.56275229225866e-05
15700 4.55227418569848e-05
15800 4.47544261987787e-05
15900 4.42764212493785e-05
16200 4.3533156713238e-05
16400 4.36597656516824e-05
16500 4.33954810432624e-05
16600 4.29146493843291e-05
16700 4.34193098044489e-05
17000 4.38951428805012e-05
17100 4.37237140431534e-05
17200 4.26077385782264e-05
17300 4.20713295170572e-05
17400 4.20982687501237e-05
17500 4.08218584198039e-05
17600 4.09180211136118e-05
17700 4.06854742323048e-05
17900 3.9161754102679e-05
18000 3.96513096347917e-05
18200 4.01135876018088e-05
18300 4.15428185078781e-05
18400 4.2803687392734e-05
18500 4.30402615165804e-05
18600 4.26249098381959e-05
18700 4.25858961534686e-05
18800 4.20144133386202e-05
18900 4.10349057347048e-05
19000 4.13831185142044e-05
19300 4.15166432503611e-05
19500 3.93558948417194e-05
19800 3.83021651941817e-05
19900 3.89490196539555e-05
20100 3.90845634683501e-05
20300 3.88494627259206e-05
20400 3.93964910472278e-05
20600 3.9814203773858e-05
20700 3.94081725971773e-05
20800 3.92244946851861e-05
20900 3.80382225557696e-05
21000 3.78359545720741e-05
21100 3.70987945643719e-05
21200 3.78224976884667e-05
21300 3.71685928257648e-05
21400 3.70818925148342e-05
21500 3.77999567717779e-05
21700 3.73282164218836e-05
21800 3.74825940525625e-05
21900 3.79965640604496e-05
22000 3.68943074136041e-05
22100 3.7449808587553e-05
22200 3.66390631825197e-05
22300 3.70585694327019e-05
22400 3.67401335097384e-05
22500 3.68441542377695e-05
22600 3.60963385901414e-05
22700 3.60579178959597e-05
22800 3.52325550920796e-05
23000 3.46945889759809e-05
23200 3.49556285073049e-05
23300 3.55480333382729e-05
23400 3.5411496355664e-05
23500 3.55643896909896e-05
23600 3.58897741534747e-05
23700 3.57618955604266e-05
23800 3.51045127899852e-05
23900 3.53362265741453e-05
24000 3.53531831933651e-05
24200 3.44903273798991e-05
24300 3.43762658303604e-05
24400 3.40828955813777e-05
24600 3.42208113579545e-05
24700 3.39165526384022e-05
24900 3.41634877258912e-05
25100 3.36667471856344e-05
25300 3.38954087055754e-05
25500 3.32139716192614e-05
25600 3.33744137606118e-05
25700 3.3934320526896e-05
25800 3.37239434884395e-05
26100 3.40835322276689e-05
26200 3.39424805133604e-05
26300 3.40659134963062e-05
26400 3.36005359713454e-05
26500 3.3424912544433e-05
26800 3.21380866807885e-05
26900 3.23985586874187e-05
27000 3.23399908666033e-05
27100 3.25949076795951e-05
27200 3.23804924846627e-05
27600 3.26549779856578e-05
27700 3.29856702592224e-05
27800 3.30467883031815e-05
27900 3.27835150528699e-05
28000 3.29126669385005e-05
28100 3.27461384586059e-05
28200 3.2783154892968e-05
28300 3.29677131958306e-05
28400 3.28444402839523e-05
28500 3.25536348100286e-05
28600 3.26680310536176e-05
28800 3.21993284160271e-05
28900 3.24784814438317e-05
29000 3.25794135278556e-05
29100 3.24669999827165e-05
29200 3.27094858221244e-05
29300 3.27804191329051e-05
29500 3.24254979204852e-05
}; \addlegendentry{K1}

\addplot [ultra thick,  green!50.1960784313725!black]
table {%
0 0.00447891326621175
100 0.00354398507624865
200 0.00251091783866286
300 0.00143611629027873
400 0.000459330069134012
500 0.000250420678639784
600 0.000102144644188229
700 5.03781120642088e-05
800 4.64967160951346e-05
900 4.53427128377371e-05
1000 4.19682619394735e-05
1100 3.91753019357566e-05
1200 3.7283607525751e-05
1300 3.60539597750176e-05
1500 3.0786879506195e-05
1600 2.66455299424706e-05
1700 2.26965530600864e-05
1800 1.76552875927882e-05
1900 1.40382080644486e-05
2000 1.16400196930044e-05
2100 1.03202901300392e-05
2200 1.0029842997028e-05
2300 1.05412818811601e-05
2400 1.05501167126931e-05
2500 1.03310485428665e-05
2700 9.73520582192577e-06
2800 9.20617821975611e-06
2900 8.4853718362865e-06
3000 7.68811605666997e-06
3100 7.5762723099615e-06
3200 7.14933548806584e-06
3300 6.41144333712873e-06
3400 6.29915166427963e-06
3500 6.09540029472555e-06
3600 6.30173917670618e-06
3700 6.25132179266075e-06
3800 8.25437382445671e-06
3900 9.07121466298122e-06
4000 8.81758569448721e-06
4200 7.49893388274359e-06
4300 5.57741896045627e-06
4400 4.46361082140356e-06
4500 4.33603327110177e-06
4600 4.04471848014509e-06
4700 5.36079232915654e-06
4800 5.62056129638222e-06
4900 5.73594525121734e-06
5100 5.78173603571486e-06
5200 5.60303806196316e-06
5300 5.25016412211698e-06
5400 5.3493095037993e-06
5500 5.22821301274234e-06
5600 5.37747519047116e-06
5700 4.11785231335671e-06
5800 3.98970405512955e-06
5900 3.30467537423829e-06
6000 3.07155346490617e-06
6100 2.89877152681584e-06
6200 3.29392014464247e-06
6300 3.3857470498333e-06
6400 4.00922772314516e-06
6500 4.56091402156744e-06
6600 4.56658153780154e-06
6700 4.28388057116535e-06
6800 4.12724421039457e-06
6900 4.30844193033408e-06
7000 3.87435693482985e-06
7100 3.60463582183002e-06
7300 2.88870614895131e-06
7400 2.60791034634167e-06
7500 2.50306334237393e-06
7600 4.15698286815314e-06
7700 4.31688022217713e-06
7800 4.09502490583691e-06
7900 3.450627446e-06
8000 3.25563132719253e-06
8100 1.75966499682545e-06
8200 2.02577871277754e-06
8300 2.20209904000512e-06
8400 2.46560193772893e-06
8500 2.59555577031279e-06
8700 2.51154233410489e-06
8800 2.88936280412599e-06
8900 3.13412397190405e-06
9100 3.13743612423423e-06
9200 2.75282013717515e-06
9300 2.19756066144328e-06
9400 2.17271258406981e-06
9500 2.1902762910031e-06
9600 1.94413678400451e-06
9700 2.10592065741366e-06
9800 2.26256406676839e-06
9900 1.90611444850219e-06
10000 1.76390904016444e-06
10100 2.73787236437784e-06
10200 2.65942367150274e-06
10300 2.5668894068076e-06
10400 2.63712172454689e-06
10500 3.91759431295213e-06
10600 3.2282589472743e-06
10700 3.17747640110611e-06
10800 3.19718583341455e-06
10900 3.12662427859323e-06
11000 1.84542375336605e-06
11100 1.570014887875e-06
11200 1.53512041833892e-06
11400 1.44469674978609e-06
11500 1.46278557622281e-06
11600 1.50869436765788e-06
11700 1.65161873155739e-06
11800 1.71932981629652e-06
11900 1.7172300204038e-06
12000 1.65933465723356e-06
12100 1.66244933552662e-06
12200 1.62084893418069e-06
12300 1.59129695020965e-06
12400 2.1272282992868e-06
12500 2.53299617725133e-06
12600 2.77263393400062e-06
12700 2.69889619630703e-06
12800 2.56587782132556e-06
12900 1.9360888927622e-06
13100 1.26385691601172e-06
13200 1.31161516492284e-06
13300 1.3857717249266e-06
13400 1.57666045197402e-06
13500 1.56359999436972e-06
13600 1.59792557496985e-06
13700 1.80738834387739e-06
13800 1.85061207957915e-06
13900 1.85838200650323e-06
14000 1.85608189440245e-06
14100 1.72832767475484e-06
14200 1.32857599055569e-06
14300 1.21635707728274e-06
14400 1.01252862805268e-06
14500 9.83065206128231e-07
14600 1.14930628569709e-06
14700 1.21309210499021e-06
14800 1.26332417949016e-06
14900 1.35159325509449e-06
15000 1.3788796877634e-06
15100 1.3005217169848e-06
15200 1.30857722524524e-06
15300 1.38937775773229e-06
15400 1.37384745357849e-06
15500 1.44417174396949e-06
15600 1.43940530961117e-06
15700 1.4072838894208e-06
15800 1.24433915971167e-06
15900 1.20497463740321e-06
16000 1.09743075427104e-06
16100 1.10079531623342e-06
16300 1.08708968582505e-06
16400 1.190668513118e-06
16500 1.76977141563839e-06
16600 1.75867216967163e-06
16700 1.76938669937954e-06
16800 1.77195488504367e-06
16900 1.71000135651411e-06
17000 1.11414260572928e-06
17100 1.09903453449078e-06
17200 1.13435385173943e-06
17300 1.14281203877908e-06
17400 1.12223460746463e-06
17500 1.13834130388568e-06
17600 1.20279901238973e-06
17700 1.3068757880319e-06
17800 1.30398336750659e-06
17900 1.24734708606411e-06
18000 1.22775657018792e-06
18100 1.13781777599797e-06
18200 9.50703281432652e-07
18300 9.83890231509577e-07
18400 1.08723293124058e-06
18500 1.10606413272762e-06
18600 1.13358066755609e-06
18700 1.21238235806231e-06
18800 1.20750428322935e-06
18900 1.08350297978177e-06
19000 1.08498034023796e-06
19100 1.04352011476294e-06
19200 9.53900666900154e-07
19300 1.02903061360848e-06
19400 1.04080356777558e-06
19500 1.016202872961e-06
19600 1.06144034361932e-06
19700 1.17150511869113e-06
19800 1.05842616449081e-06
19900 1.05627384527907e-06
20000 1.02929277545627e-06
20100 9.37730078476307e-07
20200 8.20702950932173e-07
20300 7.79832191710739e-07
20400 7.85733220709517e-07
20500 8.18589001028158e-07
20600 8.4176605241737e-07
20700 9.28277017919754e-07
20800 1.15472619199863e-06
20900 1.19173705570574e-06
21000 1.17565423352062e-06
21100 1.15370608000376e-06
21200 1.06534821497917e-06
21300 8.2573382087503e-07
21400 7.51277866584132e-07
21500 7.72189537201484e-07
21600 7.79487209001672e-07
21700 7.95009839293925e-07
21800 8.38926098367665e-07
21900 8.60374655076157e-07
22000 8.36168226214795e-07
22100 8.29618727493653e-07
22200 8.04954368049948e-07
22300 7.62363470130367e-07
22400 7.80434334046731e-07
22600 7.69595317251515e-07
22700 7.76942670199787e-07
22800 7.99775193627283e-07
22900 7.76633044097252e-07
23000 7.72814644278697e-07
23100 8.18813759906334e-07
23200 8.19569265786413e-07
23300 7.98829148607183e-07
23500 7.87050794315292e-07
23600 7.32529713332042e-07
23700 7.2076835522239e-07
23800 7.16438364634087e-07
23900 7.05537786416244e-07
24000 7.11066320491227e-07
24100 7.20679736332386e-07
24200 7.23428343007981e-07
24400 7.14076918484352e-07
24500 7.00708937984018e-07
24600 6.83764540099219e-07
24800 7.02275542607822e-07
24900 7.01128385571792e-07
25000 7.33528509044845e-07
25100 7.45670831747702e-07
25200 7.34564991944353e-07
25300 7.31958095911978e-07
25400 7.51252343889064e-07
25500 7.08433162799338e-07
25600 6.99627321409935e-07
25800 6.87173894675652e-07
26000 6.98758299222391e-07
26100 7.46558043829282e-07
26200 7.50418053030444e-07
26300 7.46460500522517e-07
26400 7.09618007022073e-07
26500 7.04849469457258e-07
26600 6.50891365694406e-07
26700 6.47618662696914e-07
26800 6.48920490675664e-07
26900 6.53955112284166e-07
27100 6.44688611828315e-07
27300 6.29145858965785e-07
27400 6.26041639861796e-07
27500 6.32366209174506e-07
27700 6.37141567949584e-07
27900 6.30972181170364e-07
28000 6.71815485020488e-07
28400 6.5852754005391e-07
28500 6.07388187745528e-07
28700 6.01217720941349e-07
29200 5.98749352320738e-07
29500 5.94582843405078e-07
}; \addlegendentry{K2}
