# Supplementary material for: Neural Networks with Physics-Informed Architectures and Constraints for Dynamical Systems Modeling
Source: arXiv:2109.06407 source file (2022-12-12)
Supplement: Supplementary file 22 [file traj_err_data.tex]

\path [fill=red, fill opacity=0.4, ultra thick]
(axis cs:1,0.321317324899372)
--(axis cs:1,0.154270957373277)
--(axis cs:2,0.0849194177170999)
--(axis cs:5,0.0480576647863629)
--(axis cs:10,0.0409580701297988)
--(axis cs:15,0.0377832687809504)
--(axis cs:25,0.0386983208442786)
--(axis cs:50,0.0325164114609333)
--(axis cs:50,0.069386282212959)
--(axis cs:50,0.069386282212959)
--(axis cs:25,0.106018718582589)
--(axis cs:15,0.0704285062923213)
--(axis cs:10,0.0723070156297636)
--(axis cs:5,0.301779308324021)
--(axis cs:2,0.19897611581381)
--(axis cs:1,0.321317324899372)
--cycle;

\path [fill=blue, fill opacity=0.4, ultra thick]
(axis cs:1,0.302775857204024)
--(axis cs:1,0.103822736962633)
--(axis cs:2,0.0828076115162474)
--(axis cs:5,0.0381229520179212)
--(axis cs:10,0.0304438363374599)
--(axis cs:15,0.0287823142787306)
--(axis cs:25,0.0217575984727216)
--(axis cs:50,0.00758026968939714)
--(axis cs:50,0.0199793722874369)
--(axis cs:50,0.0199793722874369)
--(axis cs:25,0.0927208561785352)
--(axis cs:15,0.0612113714019699)
--(axis cs:10,0.0660780928106958)
--(axis cs:5,0.127245395091526)
--(axis cs:2,0.253844151062908)
--(axis cs:1,0.302775857204024)
--cycle;

\path [fill=green!50.1960784313725!black, fill opacity=0.4, ultra thick]
(axis cs:1,0.109159357055561)
--(axis cs:1,0.0352173188407961)
--(axis cs:2,0.0230413231588501)
--(axis cs:5,0.00408155118403199)
--(axis cs:10,0.00418598635894365)
--(axis cs:15,0.00292412662244513)
--(axis cs:25,0.00205979541594006)
--(axis cs:50,0.00211097925347557)
--(axis cs:50,0.00372017678820147)
--(axis cs:50,0.00372017678820147)
--(axis cs:25,0.00529417726546357)
--(axis cs:15,0.00918405285446757)
--(axis cs:10,0.00746139809075942)
--(axis cs:5,0.0118184691689693)
--(axis cs:2,0.0495833337870229)
--(axis cs:1,0.109159357055561)
--cycle;

\addplot [ultra thick, red, mark=*, mark size=1.5, mark options={solid}]
table {%
1 0.237794145941734
2 0.141947731375694
5 0.174918502569199
10 0.0566325411200523
15 0.0541058890521526
25 0.0723585188388824
50 0.0509513504803181
};
\addplot [ultra thick, blue, mark=*, mark size=1.5, mark options={solid}]
table {%
1 0.203299298882484
2 0.168325915932655
5 0.0826841816306114
10 0.0482609681785107
15 0.0449968427419662
25 0.0572392269968987
50 0.013779821805656
};
\addplot [ultra thick, green!50.1960784313725!black, mark=*, mark size=1.5, mark options={solid}]
table {%
1 0.0721883475780487
2 0.0363123267889023
5 0.00795001070946455
10 0.00582369277253747
15 0.00605409080162644
25 0.00367698539048433
50 0.00291557726450264
};
