# Supplementary material for: Neural Networks with Physics-Informed Architectures and Constraints for Dynamical Systems Modeling
Source: arXiv:2109.06407 source file (2022-12-12)
Supplement: Supplementary file 24 [file train_test_loss_data.tex]

\path [fill=red, fill opacity=0.2, ultra thick]
(axis cs:0,0.0390019230544567)
--(axis cs:0,0.0390019230544567)
--(axis cs:100,0.0389935377607013)
--(axis cs:200,0.038820221300711)
--(axis cs:300,0.0374572107230414)
--(axis cs:400,0.035111146594165)
--(axis cs:500,0.0337754504536296)
--(axis cs:600,0.0327751579160007)
--(axis cs:700,0.0319456771890674)
--(axis cs:800,0.0304680000034032)
--(axis cs:900,0.0287133572675713)
--(axis cs:1000,0.0263532021837723)
--(axis cs:1100,0.0238966970479016)
--(axis cs:1200,0.0218216087100045)
--(axis cs:1300,0.0203481754139741)
--(axis cs:1400,0.0193295853171039)
--(axis cs:1500,0.0187712700380581)
--(axis cs:1600,0.0182842418278811)
--(axis cs:1700,0.0179887703582524)
--(axis cs:1800,0.0174107043169788)
--(axis cs:1900,0.0172072858140255)
--(axis cs:2000,0.0171278444714557)
--(axis cs:2100,0.0167495554083363)
--(axis cs:2200,0.0166856293560179)
--(axis cs:2300,0.0163993936321127)
--(axis cs:2400,0.0160135925717717)
--(axis cs:2500,0.0160705142018792)
--(axis cs:2600,0.015687067451869)
--(axis cs:2700,0.0155677251933654)
--(axis cs:2800,0.0153582092513127)
--(axis cs:2900,0.0152240493458081)
--(axis cs:3000,0.0150642342156459)
--(axis cs:3100,0.0148986713960833)
--(axis cs:3200,0.0147004178557138)
--(axis cs:3300,0.0143914025990864)
--(axis cs:3400,0.0141314140739747)
--(axis cs:3500,0.0138679086936188)
--(axis cs:3600,0.0136463374360309)
--(axis cs:3700,0.0135596232803747)
--(axis cs:3800,0.0133855260270621)
--(axis cs:3900,0.0130769345013418)
--(axis cs:4000,0.0130295029215585)
--(axis cs:4100,0.0126933634329218)
--(axis cs:4200,0.0124905470682182)
--(axis cs:4300,0.0124153131944128)
--(axis cs:4400,0.0124932617899268)
--(axis cs:4500,0.0121981834095788)
--(axis cs:4600,0.0120714540766274)
--(axis cs:4700,0.012112222163656)
--(axis cs:4800,0.0118186145916696)
--(axis cs:4900,0.0118592825138282)
--(axis cs:5000,0.0116095313186105)
--(axis cs:5100,0.0115649135029901)
--(axis cs:5200,0.0117047003214234)
--(axis cs:5300,0.0112487156849648)
--(axis cs:5400,0.0114230507394669)
--(axis cs:5500,0.0114000885954949)
--(axis cs:5600,0.011242422503022)
--(axis cs:5700,0.0109979109148537)
--(axis cs:5800,0.0110227020665706)
--(axis cs:5900,0.0113258599659133)
--(axis cs:6000,0.0110731459589566)
--(axis cs:6100,0.0109757591315358)
--(axis cs:6200,0.0108897253214146)
--(axis cs:6300,0.0109392678172291)
--(axis cs:6400,0.0108540003111364)
--(axis cs:6500,0.0106986108349984)
--(axis cs:6600,0.0104886898854216)
--(axis cs:6700,0.0105874528853446)
--(axis cs:6800,0.010589931894156)
--(axis cs:6900,0.0105021855651666)
--(axis cs:7000,0.0104933879271097)
--(axis cs:7100,0.0104874764774217)
--(axis cs:7200,0.0104466151104123)
--(axis cs:7300,0.0101978540003754)
--(axis cs:7400,0.0102253445844202)
--(axis cs:7500,0.0102641770055587)
--(axis cs:7600,0.0100156815841977)
--(axis cs:7700,0.0102918812925402)
--(axis cs:7800,0.0101722741298809)
--(axis cs:7900,0.0100752079581922)
--(axis cs:8000,0.0100742407043751)
--(axis cs:8100,0.00993030350670319)
--(axis cs:8200,0.0101399599634939)
--(axis cs:8300,0.00990401156249051)
--(axis cs:8400,0.00986824440778013)
--(axis cs:8500,0.0100807580725781)
--(axis cs:8600,0.00984426893009472)
--(axis cs:8700,0.00978200393536158)
--(axis cs:8800,0.0098957208040605)
--(axis cs:8900,0.00985134296544564)
--(axis cs:9000,0.00956138011118001)
--(axis cs:9100,0.00974494757994635)
--(axis cs:9200,0.00966957228431847)
--(axis cs:9300,0.00968610239147603)
--(axis cs:9400,0.00942433481852649)
--(axis cs:9500,0.00945873166574525)
--(axis cs:9600,0.00961692750765235)
--(axis cs:9700,0.00951288025889301)
--(axis cs:9800,0.00951084617814242)
--(axis cs:9900,0.00940022947421289)
--(axis cs:10000,0.00930521063777677)
--(axis cs:10100,0.00956620548676755)
--(axis cs:10200,0.00919848294011048)
--(axis cs:10300,0.00925913271811572)
--(axis cs:10400,0.00926735389766136)
--(axis cs:10500,0.00921621579480726)
--(axis cs:10600,0.00913554999404355)
--(axis cs:10700,0.00915666492010604)
--(axis cs:10800,0.00906463629858183)
--(axis cs:10900,0.00892522726758842)
--(axis cs:11000,0.00904680362973168)
--(axis cs:11100,0.00891162097254798)
--(axis cs:11200,0.00904375286613435)
--(axis cs:11300,0.00902139866044665)
--(axis cs:11400,0.0091464407591103)
--(axis cs:11500,0.00913317560390981)
--(axis cs:11600,0.00900773778476909)
--(axis cs:11700,0.00881875193035082)
--(axis cs:11800,0.00894772454291747)
--(axis cs:11900,0.00890308476985161)
--(axis cs:12000,0.0088918730606556)
--(axis cs:12100,0.00875854685392737)
--(axis cs:12200,0.0087886762856131)
--(axis cs:12300,0.00870813260688227)
--(axis cs:12400,0.00876822482892754)
--(axis cs:12500,0.00872705711636747)
--(axis cs:12600,0.00844241337050077)
--(axis cs:12700,0.00858775839734778)
--(axis cs:12800,0.00869631322190546)
--(axis cs:12900,0.00852511492234635)
--(axis cs:13000,0.00862470241674096)
--(axis cs:13100,0.00855684281157158)
--(axis cs:13200,0.00849748396239164)
--(axis cs:13300,0.00847296703056671)
--(axis cs:13400,0.00857985105092882)
--(axis cs:13500,0.00860978579817038)
--(axis cs:13600,0.0085171372593455)
--(axis cs:13700,0.00847827441763168)
--(axis cs:13800,0.00845297603993865)
--(axis cs:13900,0.00841286057663339)
--(axis cs:14000,0.00851908722302513)
--(axis cs:14100,0.00843923603366369)
--(axis cs:14200,0.00836468332273902)
--(axis cs:14300,0.00834230592489208)
--(axis cs:14400,0.00828220070166768)
--(axis cs:14500,0.00840020743556755)
--(axis cs:14600,0.00809642957247223)
--(axis cs:14700,0.00817862713847061)
--(axis cs:14800,0.00828825786729658)
--(axis cs:14900,0.00823762768116255)
--(axis cs:15000,0.00810482894566643)
--(axis cs:15100,0.00820295153444956)
--(axis cs:15200,0.00821836663425745)
--(axis cs:15300,0.00831141557665537)
--(axis cs:15400,0.00819623478996619)
--(axis cs:15500,0.00804897649605054)
--(axis cs:15600,0.00791164237865653)
--(axis cs:15700,0.00788106313789754)
--(axis cs:15800,0.00798870882063932)
--(axis cs:15900,0.00793909059815781)
--(axis cs:16000,0.00801860862503443)
--(axis cs:16100,0.00808516503598333)
--(axis cs:16200,0.00811777314866733)
--(axis cs:16300,0.00787014450993398)
--(axis cs:16400,0.00796453540891239)
--(axis cs:16500,0.00783531820941225)
--(axis cs:16600,0.00783880155870226)
--(axis cs:16700,0.0079092997486794)
--(axis cs:16800,0.00794334274554502)
--(axis cs:16900,0.00810734208059149)
--(axis cs:17000,0.00785580026397593)
--(axis cs:17100,0.00804709377977169)
--(axis cs:17200,0.00786014504959882)
--(axis cs:17300,0.00789820331957385)
--(axis cs:17400,0.00809562585048097)
--(axis cs:17500,0.00789633376190455)
--(axis cs:17600,0.00790698543359649)
--(axis cs:17700,0.00805270701066)
--(axis cs:17800,0.00784721246763646)
--(axis cs:17900,0.00779746951263744)
--(axis cs:18000,0.00785846147230269)
--(axis cs:18100,0.00790799847281275)
--(axis cs:18200,0.0077795116392026)
--(axis cs:18300,0.00789274469109758)
--(axis cs:18400,0.00791085653691805)
--(axis cs:18500,0.00780632440726103)
--(axis cs:18600,0.00782029891908889)
--(axis cs:18700,0.00782565188222422)
--(axis cs:18800,0.00774952120416009)
--(axis cs:18900,0.0078251347800603)
--(axis cs:19000,0.00768757253261497)
--(axis cs:19100,0.00771380361548724)
--(axis cs:19200,0.00759052524803289)
--(axis cs:19300,0.00774001797214972)
--(axis cs:19400,0.00783912518808262)
--(axis cs:19500,0.00787840328723618)
--(axis cs:19600,0.00760576595893871)
--(axis cs:19700,0.00783620519297671)
--(axis cs:19800,0.00777783850355871)
--(axis cs:19900,0.00765096498542813)
--(axis cs:20000,0.00771298951788669)
--(axis cs:20100,0.00758096477966604)
--(axis cs:20200,0.00793066135964605)
--(axis cs:20300,0.00776740483038818)
--(axis cs:20400,0.00763139482291003)
--(axis cs:20500,0.00765562133347785)
--(axis cs:20600,0.00767951223348876)
--(axis cs:20700,0.00759920155890349)
--(axis cs:20800,0.00752264660583358)
--(axis cs:20900,0.00747395022208779)
--(axis cs:21000,0.00758517559496483)
--(axis cs:21100,0.00752126068821471)
--(axis cs:21200,0.00755554419978906)
--(axis cs:21300,0.00761459309123421)
--(axis cs:21400,0.00764059626312338)
--(axis cs:21500,0.00772170446355137)
--(axis cs:21600,0.00741617273869792)
--(axis cs:21700,0.00757151021847276)
--(axis cs:21800,0.0077398232236092)
--(axis cs:21900,0.00741727590322288)
--(axis cs:22000,0.00759938032392324)
--(axis cs:22100,0.00762857381525359)
--(axis cs:22200,0.00755934063593784)
--(axis cs:22300,0.00760354587697724)
--(axis cs:22400,0.00756494789618983)
--(axis cs:22500,0.0074590032550326)
--(axis cs:22600,0.00766536267280333)
--(axis cs:22700,0.007575873584747)
--(axis cs:22700,0.00852821395923725)
--(axis cs:22700,0.00852821395923725)
--(axis cs:22600,0.00851400708973653)
--(axis cs:22500,0.00854710480793009)
--(axis cs:22400,0.0085299658099936)
--(axis cs:22300,0.00852379244552315)
--(axis cs:22200,0.00853086616595349)
--(axis cs:22100,0.00851981426007826)
--(axis cs:22000,0.00852445653613745)
--(axis cs:21900,0.00855391811818091)
--(axis cs:21800,0.00850243223313642)
--(axis cs:21700,0.0085289131920621)
--(axis cs:21600,0.00855409865247528)
--(axis cs:21500,0.00850522359670209)
--(axis cs:21400,0.00851791094242252)
--(axis cs:21300,0.00852203393218453)
--(axis cs:21200,0.00853147623713365)
--(axis cs:21100,0.00853700205980817)
--(axis cs:21000,0.00852672512453874)
--(axis cs:20900,0.00854467202231001)
--(axis cs:20800,0.00853677812232156)
--(axis cs:20700,0.00852448504778183)
--(axis cs:20600,0.00851178777123193)
--(axis cs:20500,0.00851553975188935)
--(axis cs:20400,0.00851936719366451)
--(axis cs:20300,0.0084982193723997)
--(axis cs:20200,0.00847460690218396)
--(axis cs:20100,0.00852739877669913)
--(axis cs:20000,0.00850657240168328)
--(axis cs:19900,0.00851627367969565)
--(axis cs:19800,0.00849663823074175)
--(axis cs:19700,0.00848794269951828)
--(axis cs:19600,0.00852343873400121)
--(axis cs:19500,0.0084818494979498)
--(axis cs:19400,0.00848751523406291)
--(axis cs:19300,0.00850240232869161)
--(axis cs:19200,0.00852587003421577)
--(axis cs:19100,0.00850644624102451)
--(axis cs:19000,0.00851052736866384)
--(axis cs:18900,0.00848957043285067)
--(axis cs:18800,0.00850094572372592)
--(axis cs:18700,0.0084894941567054)
--(axis cs:18600,0.00849028488098854)
--(axis cs:18500,0.00849236050516226)
--(axis cs:18400,0.00847730581274314)
--(axis cs:18300,0.00847982452469682)
--(axis cs:18200,0.00849638536202415)
--(axis cs:18100,0.00847770021819773)
--(axis cs:18000,0.00848470557937025)
--(axis cs:17900,0.00849368379412493)
--(axis cs:17800,0.00848633557404499)
--(axis cs:17700,0.00845989307348586)
--(axis cs:17600,0.00847784029772072)
--(axis cs:17500,0.00847932185690213)
--(axis cs:17400,0.00845603762773456)
--(axis cs:17300,0.00847906069331919)
--(axis cs:17200,0.00848446275809704)
--(axis cs:17100,0.00846046660748207)
--(axis cs:17000,0.00848509001444293)
--(axis cs:16900,0.00845518620677951)
--(axis cs:16800,0.00847291263913859)
--(axis cs:16700,0.00844037662690838)
--(axis cs:16600,0.00840402790319018)
--(axis cs:16500,0.0084073752793843)
--(axis cs:16400,0.00842647057900996)
--(axis cs:16300,0.00839681179457645)
--(axis cs:16200,0.00851360719576328)
--(axis cs:16100,0.00850046191388328)
--(axis cs:16000,0.00845512488454587)
--(axis cs:15900,0.00845222210533245)
--(axis cs:15800,0.00844608360856944)
--(axis cs:15700,0.00845295925741525)
--(axis cs:15600,0.00840490250678016)
--(axis cs:15500,0.00843070568125468)
--(axis cs:15400,0.0085227817669723)
--(axis cs:15300,0.00858073819307615)
--(axis cs:15200,0.00849682156601766)
--(axis cs:15100,0.00848399958624492)
--(axis cs:15000,0.00843696748031191)
--(axis cs:14900,0.00847256490482232)
--(axis cs:14800,0.00853539402266339)
--(axis cs:14700,0.00863410778826972)
--(axis cs:14600,0.00855669591231221)
--(axis cs:14500,0.00864330736251735)
--(axis cs:14400,0.00852071746425449)
--(axis cs:14300,0.00852016162733272)
--(axis cs:14200,0.00860455601649342)
--(axis cs:14100,0.00852340457468674)
--(axis cs:14000,0.00871133842784965)
--(axis cs:13900,0.0085958233780426)
--(axis cs:13800,0.00875096528044093)
--(axis cs:13700,0.0086427897485963)
--(axis cs:13600,0.00863826539109026)
--(axis cs:13500,0.00898183841210782)
--(axis cs:13400,0.00883680434549292)
--(axis cs:13300,0.00857401911719464)
--(axis cs:13200,0.00863820879795668)
--(axis cs:13100,0.00882062501443721)
--(axis cs:13000,0.0088118317495951)
--(axis cs:12900,0.00866310443121028)
--(axis cs:12800,0.00895445493891455)
--(axis cs:12700,0.00886710481813843)
--(axis cs:12600,0.00888762840560002)
--(axis cs:12500,0.00877532776481107)
--(axis cs:12400,0.00879215412985401)
--(axis cs:12300,0.00897497852430898)
--(axis cs:12200,0.00900164311243244)
--(axis cs:12100,0.00898484133693815)
--(axis cs:12000,0.00936606588563123)
--(axis cs:11900,0.00918494989473954)
--(axis cs:11800,0.00896314462830458)
--(axis cs:11700,0.00906422475064321)
--(axis cs:11600,0.00916905564647322)
--(axis cs:11500,0.00916659276449331)
--(axis cs:11400,0.00958263627210473)
--(axis cs:11300,0.00918483139385239)
--(axis cs:11200,0.00925321905101805)
--(axis cs:11100,0.00908139147063687)
--(axis cs:11000,0.00932396194206124)
--(axis cs:10900,0.00919033542966322)
--(axis cs:10800,0.00942002816144142)
--(axis cs:10700,0.00938779789978811)
--(axis cs:10600,0.00926109144416249)
--(axis cs:10500,0.00947963723488094)
--(axis cs:10400,0.0096596949941214)
--(axis cs:10300,0.00936210212601258)
--(axis cs:10200,0.00956413536318847)
--(axis cs:10100,0.0096797152160475)
--(axis cs:10000,0.00965273705350486)
--(axis cs:9900,0.00952052678137406)
--(axis cs:9800,0.00964103515902342)
--(axis cs:9700,0.00970604512777424)
--(axis cs:9600,0.010059750375019)
--(axis cs:9500,0.00972544793830824)
--(axis cs:9400,0.0097313134080128)
--(axis cs:9300,0.00975118150691729)
--(axis cs:9200,0.00979559727460398)
--(axis cs:9100,0.010041680383239)
--(axis cs:9000,0.0100112206111329)
--(axis cs:8900,0.0101727399684174)
--(axis cs:8800,0.00997791814374427)
--(axis cs:8700,0.010040242149249)
--(axis cs:8600,0.0100072424142189)
--(axis cs:8500,0.0102405943347582)
--(axis cs:8400,0.0101050566104977)
--(axis cs:8300,0.00998221017417903)
--(axis cs:8200,0.0103157071646717)
--(axis cs:8100,0.0100755900763959)
--(axis cs:8000,0.0104169868032162)
--(axis cs:7900,0.0102898948792909)
--(axis cs:7800,0.0103158533153004)
--(axis cs:7700,0.0103478878195302)
--(axis cs:7600,0.0102646646901783)
--(axis cs:7500,0.0104970253943706)
--(axis cs:7400,0.0106071244815639)
--(axis cs:7300,0.0106653164247217)
--(axis cs:7200,0.010934640128836)
--(axis cs:7100,0.0108335849003023)
--(axis cs:7000,0.0108945467576437)
--(axis cs:6900,0.0106327888698052)
--(axis cs:6800,0.0106896750740085)
--(axis cs:6700,0.0108020867786457)
--(axis cs:6600,0.0108178099534075)
--(axis cs:6500,0.0110615262958183)
--(axis cs:6400,0.0114355471372206)
--(axis cs:6300,0.0111486700245837)
--(axis cs:6200,0.0112242504369392)
--(axis cs:6100,0.0112935432266942)
--(axis cs:6000,0.0115619774230554)
--(axis cs:5900,0.0115284868160557)
--(axis cs:5800,0.0110447690303424)
--(axis cs:5700,0.0112602360615776)
--(axis cs:5600,0.0113096219382806)
--(axis cs:5500,0.0116192593652554)
--(axis cs:5400,0.0114529710232221)
--(axis cs:5300,0.011527771288003)
--(axis cs:5200,0.0117419812773989)
--(axis cs:5100,0.0118656506273559)
--(axis cs:5000,0.0121325459326649)
--(axis cs:4900,0.0120196196830559)
--(axis cs:4800,0.0121390377585972)
--(axis cs:4700,0.0123337368927611)
--(axis cs:4600,0.0121886291368212)
--(axis cs:4500,0.0126026871579814)
--(axis cs:4400,0.012760267560036)
--(axis cs:4300,0.0128665420212161)
--(axis cs:4200,0.0129199405587715)
--(axis cs:4100,0.0132699591370048)
--(axis cs:4000,0.0131105716345141)
--(axis cs:3900,0.0134690464438878)
--(axis cs:3800,0.0137955740732167)
--(axis cs:3700,0.0138610794204389)
--(axis cs:3600,0.0140495425250227)
--(axis cs:3500,0.0140949758616416)
--(axis cs:3400,0.0141659655389479)
--(axis cs:3300,0.014597876422733)
--(axis cs:3200,0.0150502037114561)
--(axis cs:3100,0.0149925711875094)
--(axis cs:3000,0.015092295603326)
--(axis cs:2900,0.0153364453651936)
--(axis cs:2800,0.0155164714764075)
--(axis cs:2700,0.0157650557241201)
--(axis cs:2600,0.0159194800825968)
--(axis cs:2500,0.0161309423250361)
--(axis cs:2400,0.0163668753298556)
--(axis cs:2300,0.01667861625145)
--(axis cs:2200,0.0168888834932335)
--(axis cs:2100,0.016997188787284)
--(axis cs:2000,0.0172256042274623)
--(axis cs:1900,0.0174184033746138)
--(axis cs:1800,0.0176467609184135)
--(axis cs:1700,0.0182706809019169)
--(axis cs:1600,0.0183582226707977)
--(axis cs:1500,0.0189357607351048)
--(axis cs:1400,0.0195207395321838)
--(axis cs:1300,0.0208439116204103)
--(axis cs:1200,0.0221191241664553)
--(axis cs:1100,0.0242660252913312)
--(axis cs:1000,0.0269350464942761)
--(axis cs:900,0.0288973531943631)
--(axis cs:800,0.0307619814786258)
--(axis cs:700,0.0324469863493886)
--(axis cs:600,0.0331448051060724)
--(axis cs:500,0.0342312066103315)
--(axis cs:400,0.0353095805395859)
--(axis cs:300,0.0375690133338382)
--(axis cs:200,0.0388255995752516)
--(axis cs:100,0.0389938276639317)
--(axis cs:0,0.0390019230544567)
--cycle;

\path [fill=blue, fill opacity=0.2, ultra thick]
(axis cs:0,0.038980360346801)
--(axis cs:0,0.0389803568345637)
--(axis cs:100,0.0389721848099988)
--(axis cs:200,0.0387978504297354)
--(axis cs:300,0.037416131816138)
--(axis cs:400,0.0351344817768292)
--(axis cs:500,0.0336935621386484)
--(axis cs:600,0.0327247050193857)
--(axis cs:700,0.0319627263859943)
--(axis cs:800,0.0303625192061382)
--(axis cs:900,0.0283576864043883)
--(axis cs:1000,0.0260043408975868)
--(axis cs:1100,0.0234878884424759)
--(axis cs:1200,0.0214170939421079)
--(axis cs:1300,0.0202215421845153)
--(axis cs:1400,0.0192905561711082)
--(axis cs:1500,0.018568268183964)
--(axis cs:1600,0.0180824703411802)
--(axis cs:1700,0.0176455662925474)
--(axis cs:1800,0.0171719887525245)
--(axis cs:1900,0.0168443696723664)
--(axis cs:2000,0.0163694674161094)
--(axis cs:2100,0.0158459593809483)
--(axis cs:2200,0.0154668718878377)
--(axis cs:2300,0.0149198261708462)
--(axis cs:2400,0.0141955985261853)
--(axis cs:2500,0.0142092102276979)
--(axis cs:2600,0.0137411311458298)
--(axis cs:2700,0.0136212100073159)
--(axis cs:2800,0.0132749232272979)
--(axis cs:2900,0.0131564389878724)
--(axis cs:3000,0.0129516400876213)
--(axis cs:3100,0.0128067363169031)
--(axis cs:3200,0.0127304952225964)
--(axis cs:3300,0.0124568400099384)
--(axis cs:3400,0.0125115983962562)
--(axis cs:3500,0.0121923084621607)
--(axis cs:3600,0.0122234976383133)
--(axis cs:3700,0.0121354270499735)
--(axis cs:3800,0.011882547837733)
--(axis cs:3900,0.0119184152480948)
--(axis cs:4000,0.0118032223081315)
--(axis cs:4100,0.0119024465824155)
--(axis cs:4200,0.0116873125650591)
--(axis cs:4300,0.0117222575913396)
--(axis cs:4400,0.0116457164775315)
--(axis cs:4500,0.0114728227144562)
--(axis cs:4600,0.0113898960957961)
--(axis cs:4700,0.0114035357242036)
--(axis cs:4800,0.0113699003676702)
--(axis cs:4900,0.0112372807627182)
--(axis cs:5000,0.0111406086964914)
--(axis cs:5100,0.0110891127488941)
--(axis cs:5200,0.0110954118913194)
--(axis cs:5300,0.0108640509765671)
--(axis cs:5400,0.0108781974035263)
--(axis cs:5500,0.0111339849469059)
--(axis cs:5600,0.0109519955586202)
--(axis cs:5700,0.0106666206095436)
--(axis cs:5800,0.0107454282936472)
--(axis cs:5900,0.0108044403928586)
--(axis cs:6000,0.0107194096838028)
--(axis cs:6100,0.010597745589222)
--(axis cs:6200,0.0107401374215122)
--(axis cs:6300,0.0105291358947433)
--(axis cs:6400,0.0103793072275857)
--(axis cs:6500,0.0102338978412076)
--(axis cs:6600,0.0101838031956194)
--(axis cs:6700,0.0104625614751282)
--(axis cs:6800,0.0101029542470737)
--(axis cs:6900,0.00989806233169144)
--(axis cs:7000,0.0100067357010927)
--(axis cs:7100,0.0102067653008396)
--(axis cs:7200,0.0100081847327594)
--(axis cs:7300,0.00988462787603704)
--(axis cs:7400,0.00977607490814138)
--(axis cs:7500,0.00956886383740498)
--(axis cs:7600,0.00965966469205192)
--(axis cs:7700,0.00950330992030682)
--(axis cs:7800,0.00955123298993774)
--(axis cs:7900,0.0094522805693688)
--(axis cs:8000,0.00931912498732138)
--(axis cs:8100,0.00950747856645895)
--(axis cs:8200,0.00931660340577969)
--(axis cs:8300,0.00911405457891658)
--(axis cs:8400,0.0092207814061763)
--(axis cs:8500,0.00913149880302797)
--(axis cs:8600,0.0091987051461474)
--(axis cs:8700,0.00906780558604704)
--(axis cs:8800,0.00896956344587149)
--(axis cs:8900,0.00899653767674365)
--(axis cs:9000,0.00893033980424356)
--(axis cs:9100,0.0089215929134014)
--(axis cs:9200,0.00888550623348204)
--(axis cs:9300,0.00886176494480199)
--(axis cs:9400,0.00849689186354955)
--(axis cs:9500,0.00868439716808915)
--(axis cs:9600,0.00867833022524581)
--(axis cs:9700,0.0083988752378818)
--(axis cs:9800,0.00856478470075495)
--(axis cs:9900,0.00849520308787294)
--(axis cs:10000,0.00838825828897466)
--(axis cs:10100,0.00866240942720303)
--(axis cs:10200,0.00819942787740677)
--(axis cs:10300,0.00848647863103921)
--(axis cs:10400,0.00827440098847979)
--(axis cs:10500,0.00828305876315057)
--(axis cs:10600,0.00809241686160554)
--(axis cs:10700,0.00797315661509834)
--(axis cs:10800,0.00800735487681699)
--(axis cs:10900,0.00777791655004944)
--(axis cs:11000,0.00791165344409051)
--(axis cs:11100,0.00773609681103695)
--(axis cs:11200,0.00784543908309972)
--(axis cs:11300,0.00761609665838511)
--(axis cs:11400,0.00794606767211969)
--(axis cs:11500,0.00760464704590356)
--(axis cs:11600,0.00760642208449722)
--(axis cs:11700,0.00777880064906505)
--(axis cs:11800,0.007705969625634)
--(axis cs:11900,0.00770212091396891)
--(axis cs:12000,0.00762178288261719)
--(axis cs:12100,0.00743533161715177)
--(axis cs:12200,0.00725828843871519)
--(axis cs:12300,0.00730049838585498)
--(axis cs:12400,0.00726049048835554)
--(axis cs:12500,0.00744890649412878)
--(axis cs:12600,0.00723177190805919)
--(axis cs:12700,0.00743024244721573)
--(axis cs:12800,0.00716151818236276)
--(axis cs:12900,0.00717142691343633)
--(axis cs:13000,0.00706647175747577)
--(axis cs:13100,0.00729899610664002)
--(axis cs:13200,0.00693629834888316)
--(axis cs:13300,0.00694568735613641)
--(axis cs:13400,0.00696144878839016)
--(axis cs:13500,0.00708887565391173)
--(axis cs:13600,0.00709457720270843)
--(axis cs:13700,0.00691325231660435)
--(axis cs:13800,0.00688392193197541)
--(axis cs:13900,0.00679142768582729)
--(axis cs:14000,0.00675322766270128)
--(axis cs:14100,0.0068470827387971)
--(axis cs:14200,0.00680981983088893)
--(axis cs:14300,0.00656805376546546)
--(axis cs:14400,0.00668084678094104)
--(axis cs:14500,0.00660636573296926)
--(axis cs:14600,0.00669499299108831)
--(axis cs:14700,0.00656764966842501)
--(axis cs:14800,0.00660066955185303)
--(axis cs:14900,0.0065216203205995)
--(axis cs:15000,0.0067054257270076)
--(axis cs:15100,0.00644700803819003)
--(axis cs:15200,0.00657660024364443)
--(axis cs:15300,0.00647662395437266)
--(axis cs:15400,0.00653311396626778)
--(axis cs:15500,0.00627659959432214)
--(axis cs:15600,0.00630108807038502)
--(axis cs:15700,0.00623155433442663)
--(axis cs:15800,0.00632928979543296)
--(axis cs:15900,0.00623340804685052)
--(axis cs:16000,0.00621633208266651)
--(axis cs:16100,0.00634656439186504)
--(axis cs:16200,0.00620301784558253)
--(axis cs:16300,0.00612101827533021)
--(axis cs:16400,0.00608617525561459)
--(axis cs:16500,0.00628151758046672)
--(axis cs:16600,0.0064018964828007)
--(axis cs:16700,0.00602537345592028)
--(axis cs:16800,0.00607406861764413)
--(axis cs:16900,0.00603267125946271)
--(axis cs:17000,0.00599511593603545)
--(axis cs:17100,0.00603225232076827)
--(axis cs:17200,0.00604644357890509)
--(axis cs:17300,0.006129523967479)
--(axis cs:17400,0.00605193265427383)
--(axis cs:17500,0.0061461732439221)
--(axis cs:17600,0.00594677277434289)
--(axis cs:17700,0.00579436420948821)
--(axis cs:17800,0.00595430883462606)
--(axis cs:17900,0.00589069862388415)
--(axis cs:18000,0.00584553950173259)
--(axis cs:18100,0.00586802476801412)
--(axis cs:18200,0.00581697877415387)
--(axis cs:18300,0.00583165936548952)
--(axis cs:18400,0.00573803728088986)
--(axis cs:18500,0.0057443358420666)
--(axis cs:18600,0.00582729756128459)
--(axis cs:18700,0.00581481694696823)
--(axis cs:18800,0.00570845378929767)
--(axis cs:18900,0.00570043654715355)
--(axis cs:19000,0.00585628529869073)
--(axis cs:19100,0.00563092633216951)
--(axis cs:19200,0.00583227470401506)
--(axis cs:19300,0.00576280173593403)
--(axis cs:19400,0.00562517856011497)
--(axis cs:19500,0.00563887668270049)
--(axis cs:19600,0.00562185692928885)
--(axis cs:19700,0.00558684199721526)
--(axis cs:19800,0.00576467033891056)
--(axis cs:19900,0.0057120508071795)
--(axis cs:20000,0.00564121735563552)
--(axis cs:20100,0.00551094827399823)
--(axis cs:20200,0.00559778378070519)
--(axis cs:20300,0.00548548837794752)
--(axis cs:20400,0.00563609031572937)
--(axis cs:20500,0.00564888849976819)
--(axis cs:20600,0.00563948451894676)
--(axis cs:20700,0.00536918796828598)
--(axis cs:20800,0.00547037206451498)
--(axis cs:20900,0.00536696785608402)
--(axis cs:21000,0.00549672290580982)
--(axis cs:21100,0.00545821540817292)
--(axis cs:21200,0.00538335488955533)
--(axis cs:21300,0.00557010000013288)
--(axis cs:21400,0.00558686984527378)
--(axis cs:21500,0.00546788175377224)
--(axis cs:21600,0.0054015255020328)
--(axis cs:21700,0.00533397649438218)
--(axis cs:21800,0.00541972499123919)
--(axis cs:21900,0.00542409663302114)
--(axis cs:22000,0.00538981594098939)
--(axis cs:22100,0.00541585406440399)
--(axis cs:22200,0.00535599354803356)
--(axis cs:22300,0.00542055997996261)
--(axis cs:22400,0.00540709929058687)
--(axis cs:22500,0.00535037656099055)
--(axis cs:22600,0.005420318017853)
--(axis cs:22700,0.00527054074815825)
--(axis cs:22800,0.00537088338243734)
--(axis cs:22900,0.00538343561876557)
--(axis cs:23000,0.00536328469756404)
--(axis cs:23100,0.00540891740492364)
--(axis cs:23200,0.00541321184283982)
--(axis cs:23300,0.00536481179112321)
--(axis cs:23400,0.00533050647498585)
--(axis cs:23500,0.00541125038294635)
--(axis cs:23600,0.00540632652328542)
--(axis cs:23700,0.00536690474105718)
--(axis cs:23800,0.00538605910576488)
--(axis cs:23800,0.00551867522759135)
--(axis cs:23800,0.00551867522759135)
--(axis cs:23700,0.00551488304582395)
--(axis cs:23600,0.00579368270103006)
--(axis cs:23500,0.00553422682952243)
--(axis cs:23400,0.00551362918196701)
--(axis cs:23300,0.00551465110417082)
--(axis cs:23200,0.00550527502053489)
--(axis cs:23100,0.00549176877964159)
--(axis cs:23000,0.00550916161345283)
--(axis cs:22900,0.00566255396168687)
--(axis cs:22800,0.00564474197767405)
--(axis cs:22700,0.00542863392917399)
--(axis cs:22600,0.00554399084751536)
--(axis cs:22500,0.00560977394908216)
--(axis cs:22400,0.00547726391365393)
--(axis cs:22300,0.00560324953249365)
--(axis cs:22200,0.00564785151283153)
--(axis cs:22100,0.00575206644060312)
--(axis cs:22000,0.00555151812778578)
--(axis cs:21900,0.00564477461176703)
--(axis cs:21800,0.00575257831780406)
--(axis cs:21700,0.00557527226993406)
--(axis cs:21600,0.00568719626255158)
--(axis cs:21500,0.005678911077748)
--(axis cs:21400,0.00566650571477146)
--(axis cs:21300,0.00593596137997532)
--(axis cs:21200,0.00567478565652812)
--(axis cs:21100,0.00572245117759038)
--(axis cs:21000,0.00595984395695216)
--(axis cs:20900,0.0056058067314876)
--(axis cs:20800,0.00578586948553322)
--(axis cs:20700,0.00580655440458446)
--(axis cs:20600,0.00579496250134552)
--(axis cs:20500,0.00573675814893681)
--(axis cs:20400,0.00585715979104242)
--(axis cs:20300,0.00574874446745821)
--(axis cs:20200,0.00590125853159899)
--(axis cs:20100,0.00576871510747897)
--(axis cs:20000,0.00589547863880122)
--(axis cs:19900,0.00600961205939304)
--(axis cs:19800,0.0058800410686118)
--(axis cs:19700,0.00588680159627487)
--(axis cs:19600,0.00591503619509285)
--(axis cs:19500,0.00598863195510529)
--(axis cs:19400,0.0059891726627975)
--(axis cs:19300,0.00597439745382824)
--(axis cs:19200,0.00591664580123047)
--(axis cs:19100,0.00606764159719772)
--(axis cs:19000,0.00601759044595009)
--(axis cs:18900,0.00592792269860372)
--(axis cs:18800,0.0059550333917698)
--(axis cs:18700,0.0058542153287085)
--(axis cs:18600,0.00593775003610384)
--(axis cs:18500,0.00610777520444632)
--(axis cs:18400,0.00607427152231086)
--(axis cs:18300,0.00612353605151729)
--(axis cs:18200,0.00592862560184431)
--(axis cs:18100,0.00619468470009231)
--(axis cs:18000,0.00612346680817405)
--(axis cs:17900,0.00605720360604084)
--(axis cs:17800,0.00606712348565084)
--(axis cs:17700,0.00614390783457441)
--(axis cs:17600,0.00610594919047336)
--(axis cs:17500,0.00632934123009234)
--(axis cs:17400,0.00645696166257826)
--(axis cs:17300,0.0062854057999707)
--(axis cs:17200,0.00625053542623299)
--(axis cs:17100,0.0062157928232135)
--(axis cs:17000,0.00638786139564262)
--(axis cs:16900,0.00629929598259938)
--(axis cs:16800,0.00641318641918677)
--(axis cs:16700,0.00639522092586909)
--(axis cs:16600,0.00654432580511247)
--(axis cs:16500,0.00663062264738754)
--(axis cs:16400,0.0064469424509624)
--(axis cs:16300,0.00635090346663223)
--(axis cs:16200,0.00645934601393187)
--(axis cs:16100,0.00644531384148825)
--(axis cs:16000,0.00653298408814515)
--(axis cs:15900,0.00640805258791749)
--(axis cs:15800,0.00661823851717067)
--(axis cs:15700,0.00688658047709394)
--(axis cs:15600,0.00655010082025095)
--(axis cs:15500,0.00666010488731931)
--(axis cs:15400,0.00670149049422992)
--(axis cs:15300,0.00684649495582078)
--(axis cs:15200,0.00667010954767812)
--(axis cs:15100,0.00681016423093575)
--(axis cs:15000,0.00684804650879124)
--(axis cs:14900,0.00677172762173292)
--(axis cs:14800,0.00696906357609859)
--(axis cs:14700,0.00682615817738604)
--(axis cs:14600,0.00693172838608575)
--(axis cs:14500,0.00699019258953987)
--(axis cs:14400,0.00708341231405223)
--(axis cs:14300,0.0070538306326969)
--(axis cs:14200,0.00693903798268793)
--(axis cs:14100,0.00727181530026572)
--(axis cs:14000,0.00705841246827556)
--(axis cs:13900,0.00710914009162757)
--(axis cs:13800,0.00733804743906525)
--(axis cs:13700,0.00718670945098967)
--(axis cs:13600,0.00719263566085606)
--(axis cs:13500,0.0071657989719817)
--(axis cs:13400,0.00718919927900473)
--(axis cs:13300,0.00731712050980114)
--(axis cs:13200,0.00735545936884546)
--(axis cs:13100,0.00744886380349048)
--(axis cs:13000,0.00753517826946155)
--(axis cs:12900,0.00735966238995783)
--(axis cs:12800,0.00756918335109389)
--(axis cs:12700,0.00768315567507504)
--(axis cs:12600,0.00746226531827999)
--(axis cs:12500,0.00763615365530245)
--(axis cs:12400,0.0079444703024177)
--(axis cs:12300,0.0077030881125446)
--(axis cs:12200,0.00777596433898047)
--(axis cs:12100,0.00765860620950155)
--(axis cs:12000,0.00796956936408453)
--(axis cs:11900,0.00781449455876506)
--(axis cs:11800,0.00787988347170548)
--(axis cs:11700,0.00795816077776922)
--(axis cs:11600,0.0080005788649849)
--(axis cs:11500,0.0079115421915321)
--(axis cs:11400,0.00825299770022814)
--(axis cs:11300,0.00823121407590676)
--(axis cs:11200,0.00833820762314363)
--(axis cs:11100,0.00827164820657105)
--(axis cs:11000,0.00825672174501516)
--(axis cs:10900,0.00824148396957988)
--(axis cs:10800,0.00833370800671903)
--(axis cs:10700,0.0084237626502911)
--(axis cs:10600,0.0083907658468168)
--(axis cs:10500,0.0085466883226194)
--(axis cs:10400,0.00849632197691963)
--(axis cs:10300,0.00860916663771893)
--(axis cs:10200,0.00862148157801182)
--(axis cs:10100,0.00888745676235627)
--(axis cs:10000,0.00919481327565998)
--(axis cs:9900,0.0087295042423937)
--(axis cs:9800,0.00875703722230229)
--(axis cs:9700,0.00901998801392351)
--(axis cs:9600,0.00891482507934506)
--(axis cs:9500,0.00893482088831146)
--(axis cs:9400,0.00884268976012388)
--(axis cs:9300,0.00897325234888965)
--(axis cs:9200,0.00936557879953735)
--(axis cs:9100,0.00923410233623557)
--(axis cs:9000,0.00915430546705771)
--(axis cs:8900,0.0091454720981002)
--(axis cs:8800,0.00950734185534178)
--(axis cs:8700,0.00966434108437392)
--(axis cs:8600,0.00948043188508988)
--(axis cs:8500,0.00961469159093649)
--(axis cs:8400,0.00977868029930968)
--(axis cs:8300,0.00949431497516598)
--(axis cs:8200,0.00961785943457872)
--(axis cs:8100,0.00980114870618669)
--(axis cs:8000,0.00975633760730696)
--(axis cs:7900,0.00951577445537428)
--(axis cs:7800,0.00983036526907416)
--(axis cs:7700,0.00994602342955687)
--(axis cs:7600,0.00988701732300946)
--(axis cs:7500,0.00983184267731117)
--(axis cs:7400,0.0100666906963149)
--(axis cs:7300,0.0102170075303776)
--(axis cs:7200,0.0103337592167016)
--(axis cs:7100,0.0103674827845798)
--(axis cs:7000,0.0103921027444515)
--(axis cs:6900,0.0103644137251228)
--(axis cs:6800,0.0102929443235433)
--(axis cs:6700,0.0105352856448389)
--(axis cs:6600,0.0103832941950721)
--(axis cs:6500,0.0107622884201681)
--(axis cs:6400,0.0110378927168708)
--(axis cs:6300,0.0106655859877987)
--(axis cs:6200,0.0108357064938311)
--(axis cs:6100,0.0108784759920781)
--(axis cs:6000,0.0109503121679435)
--(axis cs:5900,0.0110906329613856)
--(axis cs:5800,0.0108595424247763)
--(axis cs:5700,0.0107211973494471)
--(axis cs:5600,0.011028309954126)
--(axis cs:5500,0.0113493881139166)
--(axis cs:5400,0.0112124350649357)
--(axis cs:5300,0.011178669291603)
--(axis cs:5200,0.0113400986397484)
--(axis cs:5100,0.0115137154706389)
--(axis cs:5000,0.0115810494538636)
--(axis cs:4900,0.0113814544463892)
--(axis cs:4800,0.0114849251141022)
--(axis cs:4700,0.011684244577566)
--(axis cs:4600,0.0116603630820874)
--(axis cs:4500,0.0119545562926846)
--(axis cs:4400,0.011891256224018)
--(axis cs:4300,0.0117566129991883)
--(axis cs:4200,0.0119003905188932)
--(axis cs:4100,0.0119863555734368)
--(axis cs:4000,0.0119033032560622)
--(axis cs:3900,0.0121107632967842)
--(axis cs:3800,0.0121817639199507)
--(axis cs:3700,0.0123087674606057)
--(axis cs:3600,0.012243868798804)
--(axis cs:3500,0.0123426167354009)
--(axis cs:3400,0.0126116966675176)
--(axis cs:3300,0.0125983983462545)
--(axis cs:3200,0.0128530395893375)
--(axis cs:3100,0.0130794919911785)
--(axis cs:3000,0.0130228987105123)
--(axis cs:2900,0.0133204614158259)
--(axis cs:2800,0.0133883360653444)
--(axis cs:2700,0.0141489087805688)
--(axis cs:2600,0.013888425609395)
--(axis cs:2500,0.0143933128806255)
--(axis cs:2400,0.0145572872326915)
--(axis cs:2300,0.0152544323046561)
--(axis cs:2200,0.0157980180974853)
--(axis cs:2100,0.0162056672119262)
--(axis cs:2000,0.016494140834906)
--(axis cs:1900,0.0170010140015399)
--(axis cs:1800,0.0172474075187838)
--(axis cs:1700,0.0179972885768183)
--(axis cs:1600,0.0182401916447734)
--(axis cs:1500,0.0188074774900103)
--(axis cs:1400,0.0193273043547383)
--(axis cs:1300,0.020423161869284)
--(axis cs:1200,0.0219590376620072)
--(axis cs:1100,0.0239195747504638)
--(axis cs:1000,0.0265207162493598)
--(axis cs:900,0.028694050457079)
--(axis cs:800,0.0307005965893152)
--(axis cs:700,0.0322308948918148)
--(axis cs:600,0.0330829280825545)
--(axis cs:500,0.0342243212575003)
--(axis cs:400,0.0353059844284499)
--(axis cs:300,0.0374776705882657)
--(axis cs:200,0.0388021791778785)
--(axis cs:100,0.0389724788537064)
--(axis cs:0,0.038980360346801)
--cycle;

\path [fill=green!50.1960784313725!black, fill opacity=0.2, ultra thick]
(axis cs:0,0.0574927553534508)
--(axis cs:0,0.0574927553534508)
--(axis cs:100,0.0574398323094995)
--(axis cs:200,0.0563991881086609)
--(axis cs:300,0.0523909474641775)
--(axis cs:400,0.0436406503344025)
--(axis cs:500,0.0385023750332377)
--(axis cs:600,0.037651315161948)
--(axis cs:700,0.0373019520434192)
--(axis cs:800,0.0364657131109171)
--(axis cs:900,0.0347989297400964)
--(axis cs:1000,0.0342157445924293)
--(axis cs:1100,0.0337431832079807)
--(axis cs:1200,0.0325821984786356)
--(axis cs:1300,0.0302271483511611)
--(axis cs:1400,0.0274892540903305)
--(axis cs:1500,0.0236997992574177)
--(axis cs:1600,0.0190136311119597)
--(axis cs:1700,0.0158657616125858)
--(axis cs:1800,0.0130195795652949)
--(axis cs:1900,0.0108368017797645)
--(axis cs:2000,0.00967926016292388)
--(axis cs:2100,0.00895624320031587)
--(axis cs:2200,0.00830202486666007)
--(axis cs:2300,0.00802377392365909)
--(axis cs:2400,0.00756239412250593)
--(axis cs:2500,0.00725581998975785)
--(axis cs:2600,0.00705759761986934)
--(axis cs:2700,0.00672410837629789)
--(axis cs:2800,0.00660251940527448)
--(axis cs:2900,0.00643624548207266)
--(axis cs:3000,0.0063785414956291)
--(axis cs:3100,0.00618853762073734)
--(axis cs:3200,0.00603176230732301)
--(axis cs:3300,0.00607485187707195)
--(axis cs:3400,0.00589666125938017)
--(axis cs:3500,0.0057840881000999)
--(axis cs:3600,0.00575743244126428)
--(axis cs:3700,0.00548745148047913)
--(axis cs:3800,0.00550193740326262)
--(axis cs:3900,0.00540350220548376)
--(axis cs:4000,0.00536310874848743)
--(axis cs:4100,0.00537538443499439)
--(axis cs:4200,0.00526290261699403)
--(axis cs:4300,0.00513957142066924)
--(axis cs:4400,0.00498894239818718)
--(axis cs:4500,0.0049644915066338)
--(axis cs:4600,0.00486604764061657)
--(axis cs:4700,0.00483501374457394)
--(axis cs:4800,0.00464911614254584)
--(axis cs:4900,0.00475488219397346)
--(axis cs:5000,0.0046803856785804)
--(axis cs:5100,0.00459886784477667)
--(axis cs:5200,0.00451916193782644)
--(axis cs:5300,0.00438402450545458)
--(axis cs:5400,0.00434502094534958)
--(axis cs:5500,0.00420185405675307)
--(axis cs:5600,0.00419464309442004)
--(axis cs:5700,0.00415376400983838)
--(axis cs:5800,0.00419456178156951)
--(axis cs:5900,0.0040516090345773)
--(axis cs:6000,0.00397977203318683)
--(axis cs:6100,0.00390457263832518)
--(axis cs:6200,0.00393980429653285)
--(axis cs:6300,0.00388658414080813)
--(axis cs:6400,0.00378568302883886)
--(axis cs:6500,0.0038974358418345)
--(axis cs:6600,0.00374189224500883)
--(axis cs:6700,0.00368783240425656)
--(axis cs:6800,0.00360360615701652)
--(axis cs:6900,0.00351975973118442)
--(axis cs:7000,0.00356356159235256)
--(axis cs:7100,0.00355335472379002)
--(axis cs:7200,0.00356858310341571)
--(axis cs:7300,0.00352944144576628)
--(axis cs:7400,0.00339610554475564)
--(axis cs:7500,0.00343882356805005)
--(axis cs:7600,0.0033903580711612)
--(axis cs:7700,0.00337631645582562)
--(axis cs:7800,0.00336384556796734)
--(axis cs:7900,0.00338933067496195)
--(axis cs:8000,0.00328717716787304)
--(axis cs:8100,0.00330344313968388)
--(axis cs:8200,0.00319484943963583)
--(axis cs:8300,0.00329678070589538)
--(axis cs:8400,0.00316306813276715)
--(axis cs:8500,0.0031883282392319)
--(axis cs:8600,0.00314854921959609)
--(axis cs:8700,0.00313843947499677)
--(axis cs:8800,0.00314055295118974)
--(axis cs:8900,0.00309746360519006)
--(axis cs:9000,0.00308585928031348)
--(axis cs:9100,0.0030630458173316)
--(axis cs:9200,0.00310510912508572)
--(axis cs:9300,0.0030208764110315)
--(axis cs:9400,0.00305738914492321)
--(axis cs:9500,0.00303580912832017)
--(axis cs:9600,0.00303640560959866)
--(axis cs:9700,0.00302146828939068)
--(axis cs:9800,0.00302254309751515)
--(axis cs:9900,0.00298186013404566)
--(axis cs:10000,0.00297436451393183)
--(axis cs:10100,0.00298347594339993)
--(axis cs:10200,0.0029145140971962)
--(axis cs:10300,0.00296134084544412)
--(axis cs:10400,0.00287271819317)
--(axis cs:10500,0.00291190251002215)
--(axis cs:10600,0.00286245950750932)
--(axis cs:10700,0.00289253700825415)
--(axis cs:10800,0.00283302903483228)
--(axis cs:10900,0.00284892455584192)
--(axis cs:11000,0.00289913787428177)
--(axis cs:11100,0.00282868989433339)
--(axis cs:11200,0.00285093792260446)
--(axis cs:11300,0.00282676906755292)
--(axis cs:11400,0.00282031945035925)
--(axis cs:11500,0.00279546957378494)
--(axis cs:11600,0.00278755206559797)
--(axis cs:11700,0.00279952027369041)
--(axis cs:11800,0.00278749613198058)
--(axis cs:11900,0.00277580899163854)
--(axis cs:12000,0.00272635423474712)
--(axis cs:12100,0.00275848021636245)
--(axis cs:12200,0.00276132622682162)
--(axis cs:12300,0.00270913885691506)
--(axis cs:12400,0.00268529107986946)
--(axis cs:12500,0.0026606823870683)
--(axis cs:12600,0.00268922332422041)
--(axis cs:12700,0.00270070295349551)
--(axis cs:12800,0.00263753361679908)
--(axis cs:12900,0.00269554873018744)
--(axis cs:13000,0.00264939232614243)
--(axis cs:13100,0.00267358035453497)
--(axis cs:13200,0.00260228182833258)
--(axis cs:13300,0.0026012575501849)
--(axis cs:13400,0.00259584605655915)
--(axis cs:13500,0.00258682430238121)
--(axis cs:13600,0.00257792812973971)
--(axis cs:13700,0.00266199596468644)
--(axis cs:13800,0.00259685989299156)
--(axis cs:13900,0.00261539077296135)
--(axis cs:14000,0.00255323239020712)
--(axis cs:14100,0.00254425387263483)
--(axis cs:14200,0.00251745482382591)
--(axis cs:14300,0.00252255024781303)
--(axis cs:14400,0.00250737768907652)
--(axis cs:14500,0.0024866776061413)
--(axis cs:14600,0.00251389887196295)
--(axis cs:14700,0.00253186219724647)
--(axis cs:14800,0.00247536179743562)
--(axis cs:14900,0.00246446270102361)
--(axis cs:15000,0.00245139955477073)
--(axis cs:15100,0.0024640071841481)
--(axis cs:15200,0.00247728550736303)
--(axis cs:15300,0.00246617142568105)
--(axis cs:15400,0.00245606735780731)
--(axis cs:15500,0.0024044939213219)
--(axis cs:15600,0.00242717445755324)
--(axis cs:15700,0.0024650787121936)
--(axis cs:15800,0.00242970733507119)
--(axis cs:15900,0.00239470289017186)
--(axis cs:16000,0.00239440214628934)
--(axis cs:16100,0.00245976207314404)
--(axis cs:16200,0.00246074993386205)
--(axis cs:16300,0.00242224203622883)
--(axis cs:16400,0.00246222251992883)
--(axis cs:16500,0.00239864531535138)
--(axis cs:16600,0.00235370263261714)
--(axis cs:16700,0.00235248345394131)
--(axis cs:16800,0.00244819159369603)
--(axis cs:16900,0.00234651148568928)
--(axis cs:17000,0.00238102360967895)
--(axis cs:17100,0.00248087553342339)
--(axis cs:17200,0.0023208446960262)
--(axis cs:17300,0.00237260049709953)
--(axis cs:17400,0.00237273561909024)
--(axis cs:17500,0.00229228056251799)
--(axis cs:17600,0.00230433497218091)
--(axis cs:17700,0.00229306913334434)
--(axis cs:17800,0.0022924052957772)
--(axis cs:17900,0.00230430628257357)
--(axis cs:18000,0.00227996609640185)
--(axis cs:18100,0.00236565145292991)
--(axis cs:18200,0.00228075652415216)
--(axis cs:18300,0.00230192295749275)
--(axis cs:18400,0.00224867240426361)
--(axis cs:18500,0.00225365130372409)
--(axis cs:18600,0.00230889891806977)
--(axis cs:18700,0.00231714625709217)
--(axis cs:18800,0.00223408808565062)
--(axis cs:18900,0.00228259123640209)
--(axis cs:19000,0.00229423495742668)
--(axis cs:19100,0.00223361311534969)
--(axis cs:19200,0.00227049994633992)
--(axis cs:19300,0.00224840837270605)
--(axis cs:19400,0.00221888900264166)
--(axis cs:19500,0.00223300107225086)
--(axis cs:19600,0.00219846103298763)
--(axis cs:19700,0.0022162170204979)
--(axis cs:19800,0.00224015208724876)
--(axis cs:19900,0.00220916164368035)
--(axis cs:20000,0.0022426420262222)
--(axis cs:20100,0.00220846788330132)
--(axis cs:20200,0.0022573019006563)
--(axis cs:20300,0.00227880008622362)
--(axis cs:20400,0.00225922659707393)
--(axis cs:20500,0.00223127316565127)
--(axis cs:20600,0.0021849147996661)
--(axis cs:20700,0.00218527252869171)
--(axis cs:20800,0.00215941015303199)
--(axis cs:20900,0.00223217222135763)
--(axis cs:21000,0.0021795323114389)
--(axis cs:21100,0.00218254749033367)
--(axis cs:21200,0.00222667095117489)
--(axis cs:21300,0.00218396005447646)
--(axis cs:21400,0.00219648367558879)
--(axis cs:21500,0.00215373729538639)
--(axis cs:21600,0.00215062662044993)
--(axis cs:21700,0.00216776895711523)
--(axis cs:21800,0.00216631967830252)
--(axis cs:21900,0.00218755615577619)
--(axis cs:22000,0.00217865970123537)
--(axis cs:22100,0.00219655721337103)
--(axis cs:22200,0.00212227347903391)
--(axis cs:22300,0.00214030589963905)
--(axis cs:22400,0.00221684915068995)
--(axis cs:22500,0.00220701884489582)
--(axis cs:22600,0.00216535496963465)
--(axis cs:22700,0.00218442436081818)
--(axis cs:22800,0.00216903765641537)
--(axis cs:22900,0.00215598303987088)
--(axis cs:23000,0.00216182080568759)
--(axis cs:23100,0.00213334526995943)
--(axis cs:23200,0.00219626565264362)
--(axis cs:23300,0.00215878533676516)
--(axis cs:23300,0.00256254095107068)
--(axis cs:23300,0.00256254095107068)
--(axis cs:23200,0.002560023105525)
--(axis cs:23100,0.00256475554029022)
--(axis cs:23000,0.00256230084685596)
--(axis cs:22900,0.00256276752016443)
--(axis cs:22800,0.00256175319708499)
--(axis cs:22700,0.0025607048246001)
--(axis cs:22600,0.00256202848500606)
--(axis cs:22500,0.00255951259894842)
--(axis cs:22400,0.00255914856624354)
--(axis cs:22300,0.00256411610736537)
--(axis cs:22200,0.00256581902838806)
--(axis cs:22100,0.00256000783716139)
--(axis cs:22000,0.00256107743691676)
--(axis cs:21900,0.00256051321501016)
--(axis cs:21800,0.00256195551770338)
--(axis cs:21700,0.00256184703295725)
--(axis cs:21600,0.00256321323086986)
--(axis cs:21500,0.00256295240301172)
--(axis cs:21400,0.00256001168097096)
--(axis cs:21300,0.00256073389285862)
--(axis cs:21200,0.00255889579477191)
--(axis cs:21100,0.00256082335806374)
--(axis cs:21000,0.00256101942352515)
--(axis cs:20900,0.00255880814749498)
--(axis cs:20800,0.00256249107127324)
--(axis cs:20700,0.00256065216142572)
--(axis cs:20600,0.00256067430388362)
--(axis cs:20500,0.00255881965278774)
--(axis cs:20400,0.00255906371973628)
--(axis cs:20300,0.00256017506018923)
--(axis cs:20200,0.00255900190510225)
--(axis cs:20100,0.00255945247294253)
--(axis cs:20000,0.00255876139444466)
--(axis cs:19900,0.00255942445298392)
--(axis cs:19800,0.00256044310064376)
--(axis cs:19700,0.00255200927521171)
--(axis cs:19600,0.0025488839240561)
--(axis cs:19500,0.00255515738920067)
--(axis cs:19400,0.00256195904226043)
--(axis cs:19300,0.0025655256827614)
--(axis cs:19200,0.00257206839778622)
--(axis cs:19100,0.00255656957571777)
--(axis cs:19000,0.00256454150390636)
--(axis cs:18900,0.00259202469361872)
--(axis cs:18800,0.00255150225380141)
--(axis cs:18700,0.00257245667101978)
--(axis cs:18600,0.00256465933994714)
--(axis cs:18500,0.00256520386022763)
--(axis cs:18400,0.00256861549901545)
--(axis cs:18300,0.00256580568686835)
--(axis cs:18200,0.0025786121031179)
--(axis cs:18100,0.00257859791379061)
--(axis cs:18000,0.00257235955911811)
--(axis cs:17900,0.00257781719394165)
--(axis cs:17800,0.00256164501393052)
--(axis cs:17700,0.00257931534778769)
--(axis cs:17600,0.00258573532464307)
--(axis cs:17500,0.0025758469983459)
--(axis cs:17400,0.00259683361446635)
--(axis cs:17300,0.00257510423159324)
--(axis cs:17200,0.00257298503959064)
--(axis cs:17100,0.00261293818518364)
--(axis cs:17000,0.00257961035987635)
--(axis cs:16900,0.00257306062677165)
--(axis cs:16800,0.00259811365295515)
--(axis cs:16700,0.00258072337623243)
--(axis cs:16600,0.00260260674056293)
--(axis cs:16500,0.00261734134576491)
--(axis cs:16400,0.00261054206672845)
--(axis cs:16300,0.00258630739324743)
--(axis cs:16200,0.00259277973722084)
--(axis cs:16100,0.00259986217286714)
--(axis cs:16000,0.00259550406788827)
--(axis cs:15900,0.00260115835576827)
--(axis cs:15800,0.00260872109568474)
--(axis cs:15700,0.00263904614429828)
--(axis cs:15600,0.00258457732459584)
--(axis cs:15500,0.00261595470624937)
--(axis cs:15400,0.00263572896088268)
--(axis cs:15300,0.00262049252952066)
--(axis cs:15200,0.00259569825054015)
--(axis cs:15100,0.00260659580281351)
--(axis cs:15000,0.00260180570561533)
--(axis cs:14900,0.00262375982250671)
--(axis cs:14800,0.00262634550087299)
--(axis cs:14700,0.00264517357530563)
--(axis cs:14600,0.00269674988451131)
--(axis cs:14500,0.00262846355464485)
--(axis cs:14400,0.00264643803860441)
--(axis cs:14300,0.00265920515710635)
--(axis cs:14200,0.00263852110656683)
--(axis cs:14100,0.00267023736556186)
--(axis cs:14000,0.00268490838778807)
--(axis cs:13900,0.00266824666500809)
--(axis cs:13800,0.00271787719971202)
--(axis cs:13700,0.00274313700453404)
--(axis cs:13600,0.00270379528511848)
--(axis cs:13500,0.00268067704066045)
--(axis cs:13400,0.00271290744382296)
--(axis cs:13300,0.00269017474729322)
--(axis cs:13200,0.00276328079689678)
--(axis cs:13100,0.0027444832525319)
--(axis cs:13000,0.00271902278491254)
--(axis cs:12900,0.00273635619298337)
--(axis cs:12800,0.00278724575735334)
--(axis cs:12700,0.00275354377735861)
--(axis cs:12600,0.00279054816443619)
--(axis cs:12500,0.00276770819036719)
--(axis cs:12400,0.00280604712472301)
--(axis cs:12300,0.00282804044178384)
--(axis cs:12200,0.00286510730213813)
--(axis cs:12100,0.00279503587727907)
--(axis cs:12000,0.00284282685981986)
--(axis cs:11900,0.00280394649466105)
--(axis cs:11800,0.00289069828781072)
--(axis cs:11700,0.00282247286445401)
--(axis cs:11600,0.00289203949327569)
--(axis cs:11500,0.00284984403684828)
--(axis cs:11400,0.00283912930865019)
--(axis cs:11300,0.00285811721537786)
--(axis cs:11200,0.00294929685214403)
--(axis cs:11100,0.00290955636028954)
--(axis cs:11000,0.00292867631108924)
--(axis cs:10900,0.00287641046348826)
--(axis cs:10800,0.00289895593812151)
--(axis cs:10700,0.00296897242786644)
--(axis cs:10600,0.00293089481127834)
--(axis cs:10500,0.0029776031035731)
--(axis cs:10400,0.00296675428819004)
--(axis cs:10300,0.00302367391604352)
--(axis cs:10200,0.00295501682025955)
--(axis cs:10100,0.00304813257605486)
--(axis cs:10000,0.00306774156314317)
--(axis cs:9900,0.00302715512063068)
--(axis cs:9800,0.00309464791295007)
--(axis cs:9700,0.00305936699217014)
--(axis cs:9600,0.00313932818268647)
--(axis cs:9500,0.00312450972315078)
--(axis cs:9400,0.00310468323173531)
--(axis cs:9300,0.00305465545412817)
--(axis cs:9200,0.00314790767708615)
--(axis cs:9100,0.00308113538700727)
--(axis cs:9000,0.00322625459583061)
--(axis cs:8900,0.00321906179076956)
--(axis cs:8800,0.00321944999740237)
--(axis cs:8700,0.00321506454944924)
--(axis cs:8600,0.00323056617565185)
--(axis cs:8500,0.0033205829444929)
--(axis cs:8400,0.003326864869973)
--(axis cs:8300,0.00330754742478693)
--(axis cs:8200,0.00344677288266524)
--(axis cs:8100,0.00337299434876275)
--(axis cs:8000,0.00335969921073273)
--(axis cs:7900,0.00347060328249559)
--(axis cs:7800,0.00345837417139029)
--(axis cs:7700,0.00340963183932061)
--(axis cs:7600,0.00343471182571562)
--(axis cs:7500,0.00349075639896196)
--(axis cs:7400,0.00357024117485704)
--(axis cs:7300,0.00357692791551512)
--(axis cs:7200,0.0036060900763697)
--(axis cs:7100,0.00362693200281388)
--(axis cs:7000,0.00362533008917951)
--(axis cs:6900,0.0036996866261552)
--(axis cs:6800,0.00380391629287425)
--(axis cs:6700,0.00374776103935569)
--(axis cs:6600,0.00381985241140496)
--(axis cs:6500,0.00392106699782019)
--(axis cs:6400,0.00390168276261109)
--(axis cs:6300,0.00409497077469951)
--(axis cs:6200,0.00395674849714877)
--(axis cs:6100,0.00402094583963127)
--(axis cs:6000,0.0041363704806645)
--(axis cs:5900,0.00407264529889892)
--(axis cs:5800,0.00424698856514276)
--(axis cs:5700,0.00428949531379831)
--(axis cs:5600,0.0044416061348919)
--(axis cs:5500,0.00436941928005482)
--(axis cs:5400,0.00449551264894084)
--(axis cs:5300,0.00449712468719654)
--(axis cs:5200,0.00461846293688459)
--(axis cs:5100,0.0047546081108487)
--(axis cs:5000,0.00482224376045566)
--(axis cs:4900,0.00482200811319471)
--(axis cs:4800,0.00497885534519483)
--(axis cs:4700,0.00498675106978302)
--(axis cs:4600,0.00502386328828844)
--(axis cs:4500,0.00502994299658374)
--(axis cs:4400,0.00521293862059051)
--(axis cs:4300,0.0051954542673432)
--(axis cs:4200,0.00535342253542299)
--(axis cs:4100,0.00549806584175793)
--(axis cs:4000,0.00553104234557171)
--(axis cs:3900,0.00562463143768644)
--(axis cs:3800,0.00579799714537366)
--(axis cs:3700,0.00577194042339813)
--(axis cs:3600,0.00586719158008705)
--(axis cs:3500,0.00594751197834379)
--(axis cs:3400,0.00599099122966608)
--(axis cs:3300,0.00616958252928804)
--(axis cs:3200,0.00636461675620377)
--(axis cs:3100,0.00630860682007254)
--(axis cs:3000,0.00646943588432874)
--(axis cs:2900,0.00665419831533688)
--(axis cs:2800,0.00681588777414074)
--(axis cs:2700,0.00712447049151507)
--(axis cs:2600,0.00714183684927421)
--(axis cs:2500,0.00750111441709885)
--(axis cs:2400,0.00762264381575113)
--(axis cs:2300,0.00812546941623711)
--(axis cs:2200,0.00856174902069605)
--(axis cs:2100,0.00903626260338839)
--(axis cs:2000,0.00994691333828951)
--(axis cs:1900,0.0114469944412533)
--(axis cs:1800,0.0140522540452398)
--(axis cs:1700,0.0168517730387731)
--(axis cs:1600,0.0201794241700767)
--(axis cs:1500,0.0241990260005989)
--(axis cs:1400,0.0279663486151482)
--(axis cs:1300,0.0311468553373333)
--(axis cs:1200,0.0331320614637371)
--(axis cs:1100,0.0339162867342711)
--(axis cs:1000,0.0343155724230596)
--(axis cs:900,0.0358465267726726)
--(axis cs:800,0.0369442589805988)
--(axis cs:700,0.0375177195675719)
--(axis cs:600,0.0377604019350165)
--(axis cs:500,0.0388990345132966)
--(axis cs:400,0.0439598217383578)
--(axis cs:300,0.0528053199022318)
--(axis cs:200,0.0564248942659119)
--(axis cs:100,0.0574415192806571)
--(axis cs:0,0.0574927553534508)
--cycle;

\addplot [ultra thick, red]
table {%
0 0.0390019230544567
100 0.0389936827123165
200 0.0388229079544544
300 0.0375131145119667
400 0.0352103672921658
500 0.0340033285319805
600 0.0329599864780903
700 0.0321963354945183
800 0.0306149907410145
900 0.0288053564727306
1000 0.0266441255807877
1100 0.0240813568234444
1200 0.0219703651964664
1300 0.0205960422754288
1400 0.0194251611828804
1600 0.0183212328702211
1700 0.0181297268718481
1800 0.017528735101223
1900 0.0173128470778465
2000 0.0171767212450504
2100 0.016873374581337
2200 0.0167872570455074
2300 0.0165390074253082
2400 0.0161902327090502
2500 0.0161007288843393
2600 0.0158032737672329
2700 0.0156663898378611
2800 0.0154373422265053
2900 0.0152802485972643
3000 0.0150782661512494
3100 0.0149456197395921
3200 0.0148753104731441
3400 0.0141486888751388
3500 0.0139814401045442
3800 0.0135905491188169
3900 0.0132729904726148
4000 0.0130700385197997
4100 0.0129816606640816
4200 0.0127052450552583
4300 0.0126409288495779
4400 0.0126267662271857
4500 0.0124004362151027
4600 0.0121300416067243
4700 0.0122229782864451
4800 0.0119788274168968
4900 0.0119394520297647
5000 0.0118710398674011
5100 0.0117152826860547
5200 0.0117233404889703
5300 0.0113882422447205
5400 0.0114380121231079
5500 0.0115096746012568
5600 0.0112760234624147
5700 0.0111290719360113
5800 0.0110337361693382
5900 0.0114271733909845
6000 0.0113175623118877
6100 0.0111346514895558
6200 0.0110569866374135
6300 0.0110439686104655
6400 0.0111447731032968
6500 0.0108800670132041
6600 0.0106532508507371
6700 0.010694770142436
6900 0.0105674890801311
7000 0.0106939664110541
7100 0.0106605319306254
7200 0.010690625756979
7300 0.0104315839707851
7400 0.0104162357747555
7500 0.010380600579083
7600 0.0101401722058654
7700 0.0103198848664761
7900 0.0101825511083007
8000 0.0102456137537956
8100 0.0100029455497861
8200 0.0102278329432011
8300 0.00994311273097992
8400 0.00998665206134319
8500 0.0101606762036681
8600 0.00992575846612453
8700 0.00991112273186445
8800 0.00993682071566582
8900 0.0100120408460498
9000 0.00978629849851131
9100 0.00989331398159266
9200 0.00973258260637522
9300 0.0097186416387558
9400 0.00957782100886106
9500 0.0095920916646719
9600 0.00983833987265825
9700 0.0096094636246562
9800 0.00957593880593777
9900 0.00946037843823433
10000 0.00947897415608168
10100 0.00962296221405268
10200 0.00938130635768175
10300 0.00931061618030071
10400 0.00946352630853653
10500 0.00934792682528496
10600 0.00919832289218903
10700 0.00927223265171051
10800 0.00924233440309763
10900 0.00905777886509895
11000 0.00918538402765989
11100 0.00899650622159243
11200 0.00914848688989878
11300 0.00910311751067638
11400 0.0093645378947258
11500 0.00914988294243813
11600 0.00908839702606201
11700 0.00894148834049702
11800 0.00895543489605188
12000 0.00912897009402514
12100 0.00887169595807791
12200 0.00889515783637762
12400 0.00878018885850906
12500 0.00875119026750326
12600 0.00866502150893211
12700 0.00872743222862482
12800 0.00882538314908743
12900 0.00859410688281059
13000 0.00871826708316803
13100 0.0086887339130044
13200 0.00856784451752901
13300 0.0085234921425581
13400 0.00870832707732916
13500 0.00879580993205309
13600 0.00857770442962646
13700 0.00856053363531828
13800 0.00860197097063065
13900 0.00850434321910143
14000 0.00861521251499653
14100 0.00848131999373436
14200 0.0084846168756485
14300 0.00843123439699411
14400 0.00840146094560623
14500 0.00852175615727901
14600 0.00832656212151051
14700 0.00840636435896158
14800 0.00841182563453913
14900 0.00835509784519672
15000 0.00827089883387089
15100 0.00834347866475582
15200 0.00835759285837412
15300 0.00844607688486576
15400 0.00835950672626495
15500 0.00823984108865261
15600 0.00815827213227749
15700 0.00816701073199511
15800 0.0082173990085721
15900 0.00819565635174513
16200 0.00831568986177444
16300 0.00813348032534122
16400 0.00819550361484289
16500 0.00812134891748428
16600 0.00812141504138708
16700 0.00817483849823475
16800 0.00820812862366438
16900 0.00828126259148121
17000 0.00817044544965029
17100 0.00825378019362688
17200 0.00817230250686407
17300 0.0081886313855648
17400 0.00827583111822605
17500 0.00818782765418291
17600 0.00819241348654032
17700 0.00825630035251379
17800 0.00816677324473858
17900 0.00814557634294033
18100 0.00819284934550524
18200 0.00813794694840908
18300 0.00818628538399935
18400 0.00819408241659403
18500 0.00814934261143208
18700 0.00815757364034653
18800 0.00812523253262043
18900 0.00815735477954149
19000 0.00809905119240284
19100 0.00811012554913759
19200 0.00805819593369961
19300 0.00812121015042067
19400 0.00816332176327705
19500 0.00818012654781342
19600 0.00806459970772266
19700 0.00816207565367222
19800 0.00813724100589752
19900 0.00808362010866404
20000 0.00810977816581726
20100 0.00805418007075787
20200 0.00820263382047415
20400 0.00807537883520126
20600 0.00809565093368292
20800 0.00802971329540014
20900 0.00800931174308062
21000 0.00805594958364964
21100 0.00802913121879101
21400 0.00807925406843424
21500 0.00811346527189016
21600 0.0079851346090436
21800 0.00812112540006638
21900 0.00798559933900833
22000 0.00806191749870777
22100 0.00807419512420893
22200 0.00804510340094566
22300 0.0080636702477932
22400 0.00804745778441429
22500 0.0080030532553792
22600 0.00808968394994736
22700 0.00805204547941685
};\addlegendentry{Baseline}

\addplot [ultra thick, blue]
table {%
0 0.0389803573489189
100 0.038972333073616
200 0.0388000160455704
300 0.0374469012022018
400 0.0352202355861664
500 0.033958937972784
600 0.0329038128256798
700 0.0320968106389046
800 0.030531557276845
900 0.0285258647054434
1000 0.026262529194355
1100 0.0237037353217602
1200 0.0216880682855844
1300 0.0203223526477814
1400 0.0193089321255684
1500 0.0186878722161055
1600 0.0181613303720951
1700 0.0178214274346828
1800 0.0172096956521273
1900 0.0169226881116629
2000 0.0164318047463894
2200 0.0156324468553066
2300 0.015087129548192
2400 0.0143764419481158
2500 0.0143012637272477
2600 0.0138147780671716
2700 0.0138850584626198
2800 0.0133316274732351
2900 0.0132384495809674
3000 0.0129872700199485
3100 0.0129431122913957
3200 0.0127917695790529
3300 0.0125276194885373
3400 0.012561647221446
3500 0.0122674638405442
3600 0.0122336819767952
3700 0.012222096323967
3800 0.0120321568101645
3900 0.0120145892724395
4000 0.0118532618507743
4100 0.0119444020092487
4200 0.0117938509210944
4300 0.0117394346743822
4400 0.0117684882134199
4500 0.0117136873304844
4600 0.0115251308307052
4700 0.0115438904613256
4900 0.0113093676045537
5000 0.0113608287647367
5100 0.0113014141097665
5200 0.0112177571281791
5300 0.0110213588923216
5400 0.0110453171655536
5500 0.0112416855990887
5600 0.0109901521354914
5700 0.0106939077377319
5800 0.0108024850487709
5900 0.0109475366771221
6100 0.0107381111010909
6200 0.0107879210263491
6300 0.0105973612517118
6400 0.0107086002826691
6600 0.0102835493162274
6700 0.0104989232495427
6800 0.0101979495957494
6900 0.0101312389597297
7000 0.0101994192227721
7100 0.0102871228009462
7300 0.0100508155301213
7400 0.00992138404399157
7500 0.00970035325735807
7600 0.00977334380149841
7800 0.00969079881906509
7900 0.00948402844369411
8000 0.00953772943466902
8100 0.00965431425720453
8200 0.00946723110973835
8300 0.00930418260395527
8400 0.00949972867965698
8500 0.00937309581786394
8600 0.00933957006782293
8700 0.00936607457697392
8800 0.00923845358192921
8900 0.00907100550830364
9000 0.00904232263565063
9200 0.00912554282695055
9300 0.00891750771552324
9400 0.00866978894919157
9500 0.00880960747599602
9600 0.00879657827317715
9700 0.00870943162590265
9900 0.00861235242336988
10000 0.00879153795540333
10100 0.00877493154257536
10200 0.00841045472770929
10300 0.00854782108217478
10400 0.00838536117225885
10500 0.00841487478464842
10600 0.00824159197509289
10700 0.0081984605640173
10800 0.00817053113132715
10900 0.00800969917327166
11000 0.00808418821543455
11100 0.00800387468189001
11200 0.0080918250605464
11300 0.00792365428060293
11400 0.00809953175485134
11500 0.00775809353217483
11600 0.00780349923297763
11700 0.00786848179996014
11800 0.00779292499646544
11900 0.00775830633938313
12000 0.00779567658901215
12100 0.00754696922376752
12200 0.0075171273201704
12300 0.00750179123133421
12400 0.00760247884318233
12500 0.00754252914339304
12600 0.0073470170609653
12700 0.00755669921636581
12800 0.00736535107716918
12900 0.0072655463591218
13000 0.00730082346126437
13100 0.0073739280924201
13200 0.00714587885886431
13300 0.0071314019151032
13400 0.00707532232627273
13500 0.00712733576074243
13600 0.00714360782876611
13700 0.00704998057335615
13800 0.00711098359897733
13900 0.00695028528571129
14000 0.00690582022070885
14100 0.00705944979563355
14200 0.00687442906200886
14300 0.00681094126775861
14400 0.0068821283057332
14500 0.00679827760905027
14600 0.00681336084380746
14700 0.00669690407812595
14800 0.00678486656397581
14900 0.00664667459204793
15000 0.00677673658356071
15100 0.00662858597934246
15200 0.00662335567176342
15300 0.0066615603864193
15400 0.00661730067804456
15500 0.00646835193037987
15600 0.00642559444531798
15700 0.00655906740576029
15800 0.00647376570850611
15900 0.00632072938606143
16000 0.0063746590167284
16100 0.00639594020321965
16200 0.00633118255063891
16300 0.00623595947399735
16400 0.00626655714586377
16500 0.00645607011392713
16600 0.00647311192005873
16700 0.00621029548346996
16800 0.0062436256557703
16900 0.00616598315536976
17000 0.00619148788973689
17100 0.0061240210197866
17200 0.00614849105477333
17300 0.00620746333152056
17400 0.00625444576144218
17500 0.00623775692656636
17600 0.00602635974064469
17700 0.00596913741901517
17800 0.00601071491837502
17900 0.00597394956275821
18000 0.00598450284451246
18100 0.00603135395795107
18200 0.00587280141189694
18300 0.00597759801894426
18400 0.00590615486726165
18500 0.00592605443671346
18700 0.00583451567217708
18800 0.00583174219354987
18900 0.00581417977809906
19000 0.00593693694099784
19100 0.00584928411990404
19200 0.00587445870041847
19300 0.00586859881877899
19400 0.00580717483535409
19500 0.00581375509500504
19600 0.00576844578608871
19700 0.00573682086542249
19800 0.00582235679030418
19900 0.00586082972586155
20000 0.00576834753155708
20100 0.00563983293250203
20200 0.00574952038004994
20300 0.00561711611226201
20400 0.00574662396684289
20500 0.0056928233243525
20600 0.00571722397580743
20700 0.00558786978945136
20800 0.00562812015414238
20900 0.00548638682812452
21000 0.0057282829657197
21100 0.00559033360332251
21200 0.0055290712043643
21300 0.00575303146615624
21400 0.00562668638303876
21500 0.00557339703664184
21600 0.00554435979574919
21700 0.00545462500303984
21800 0.00558615196496248
21900 0.00553443701937795
22000 0.00547066610306501
22100 0.00558395963162184
22200 0.00550192315131426
22300 0.00551190553233027
22400 0.00544218253344297
22500 0.00548007432371378
22600 0.00548215350136161
22700 0.00534958811476827
22800 0.00550781330093741
22900 0.00552299479022622
23000 0.00543622206896544
23200 0.00545924436300993
23400 0.00542206782847643
23500 0.00547273876145482
23600 0.00560000585392118
23700 0.00544089497998357
23800 0.00545236794278026
};\addlegendentry{K1}

\addplot [ultra thick, green!50.2156862745098!black]
table {%
0 0.0574927590787411
100 0.0574406757950783
200 0.056412048637867
300 0.0525981411337852
400 0.0438002310693264
500 0.0387007035315037
600 0.0377058610320091
700 0.0374098345637321
800 0.0367049835622311
900 0.0353227257728577
1000 0.0342656560242176
1100 0.0338297300040722
1200 0.0328571349382401
1300 0.0306870006024837
1400 0.0277278013527393
1500 0.0239494126290083
1600 0.0195965263992548
1700 0.0163587685674429
1800 0.0135359186679125
1900 0.0111418971791863
2000 0.0098130851984024
2100 0.00899625476449728
2200 0.00843188725411892
2300 0.00807462073862553
2400 0.0075925188139081
2500 0.00737846782431006
2600 0.00709971832111478
2700 0.00692428881302476
2800 0.00670920219272375
2900 0.00654522236436605
3000 0.00642398931086063
3100 0.00624857377260923
3200 0.0061981906183064
3300 0.0061222156509757
3400 0.00594382779672742
3500 0.00586579972878098
3600 0.00581231294199824
3700 0.00562969595193863
3800 0.00564996665343642
3900 0.00551406666636467
4000 0.00544707523658872
4100 0.00543672358617187
4200 0.00530816148966551
4300 0.00516751362010837
4400 0.00510093942284584
4500 0.0049972184933722
4600 0.00494495546445251
4700 0.00491088163107634
4800 0.00481398683041334
4900 0.00478844624012709
5000 0.00475131534039974
5100 0.00467673875391483
5200 0.00456881290301681
5300 0.0044405753724277
5400 0.00442026648670435
5500 0.00428563542664051
5600 0.00431812461465597
5700 0.00422163028270006
5800 0.00422077486291528
5900 0.00406212639063597
6000 0.00405807187780738
6100 0.00396275892853737
6200 0.00394827499985695
6300 0.00399077776819468
6400 0.00384368281811476
6500 0.00390925258398056
6600 0.00378087139688432
6700 0.00371779594570398
6800 0.0037037602160126
6900 0.00360972317866981
7000 0.00359444529749453
7200 0.00358733674511313
7300 0.00355318398214877
7400 0.00348317273892462
7500 0.00346478982828557
7600 0.00341253401711583
7700 0.00339297391474247
7900 0.00342996744439006
8000 0.00332343811169267
8100 0.00333821843378246
8300 0.00330216367729008
8400 0.00324496650137007
8500 0.00325445551425219
8600 0.00318955816328526
8700 0.00317675271071494
8800 0.00318000162951648
8900 0.0031582631636411
9000 0.00315605662763119
9100 0.00307208974845707
9200 0.00312650762498379
9300 0.00303776515647769
9400 0.00308103626593947
9500 0.0030801584944129
9600 0.00308786705136299
9700 0.00304041802883148
9800 0.00305859535001218
9900 0.0030045066960156
10000 0.00302105280570686
10100 0.00301580503582954
10200 0.00293476553633809
10300 0.00299250660464168
10400 0.00291973678395152
10500 0.00294475210830569
10600 0.00289667816832662
10700 0.00293075502850115
10800 0.00286599318496883
10900 0.00286266743205488
11000 0.00291390670463443
11100 0.00286912266165018
11200 0.0029001166112721
11300 0.00284244283102453
11400 0.00282972399145365
11500 0.00282265688292682
11600 0.00283979577943683
11700 0.00281099718995392
11800 0.00283909752033651
11900 0.0027898782864213
12100 0.00277675758115947
12200 0.00281321723014116
12300 0.00276858964934945
12400 0.00274566933512688
12500 0.00271419598720968
12600 0.00273988582193851
12800 0.00271238922141492
12900 0.00271595316007733
13000 0.00268420740030706
13100 0.00270903180353343
13200 0.00268278131261468
13300 0.00264571630395949
13400 0.00265437690541148
13500 0.00263375067152083
13600 0.00264086248353124
13700 0.00270256726071239
13800 0.00265736877918243
13900 0.00264181941747665
14000 0.00261907000094652
14100 0.00260724616236985
14200 0.00257798796519637
14300 0.00259087770245969
14400 0.00257690832950175
14500 0.00255757058039308
14600 0.00260532461106777
14700 0.00258851773105562
14800 0.00255085388198495
14900 0.00254411180503666
15000 0.00252660224214196
15100 0.0025353014934808
15200 0.00253649172373116
15400 0.00254589854739606
15500 0.00251022446900606
15600 0.00250587635673583
15700 0.0025520627386868
15800 0.00251921452581882
15900 0.00249793077819049
16000 0.00249495264142752
16100 0.00252981251105666
16200 0.00252676452510059
16300 0.00250427424907684
16400 0.00253638182766736
16600 0.00247815414331853
16700 0.00246660364791751
16800 0.0025231521576643
16900 0.00245978566817939
17000 0.00248031690716743
17100 0.00254690647125244
17200 0.00244691525585949
17300 0.00247385213151574
17400 0.00248478446155787
17500 0.00243406416848302
17600 0.00244503538124263
17800 0.00242702569812536
17900 0.00244106142781675
18000 0.00242616236209869
18100 0.00247212522663176
18200 0.00242968392558396
18300 0.00243386370129883
18400 0.00240864348597825
18500 0.00240942765958607
18600 0.00243677967227995
18700 0.00244480185210705
18800 0.00239279516972601
18900 0.00243730819784105
19000 0.00242938776500523
19100 0.00239509111270308
19200 0.00242128456011415
19400 0.00239042402245104
19500 0.00239407899789512
19600 0.00237367255613208
19700 0.00238411361351609
19800 0.00240029697306454
19900 0.00238429312594235
20000 0.00240070163272321
20100 0.00238396064378321
20200 0.00240815151482821
20300 0.00241948803886771
20500 0.0023950464092195
20600 0.00237279431894422
20700 0.00237296242266893
20800 0.00236095068976283
20900 0.00239548971876502
21000 0.00237027532421052
21100 0.00237168488092721
21200 0.00239278329536319
21300 0.00237234774976969
21400 0.00237824814394116
21500 0.00235834438353777
21600 0.00235691945999861
21700 0.00236480846069753
21800 0.00236413744278252
21900 0.0023740348406136
22000 0.00236986787058413
22100 0.00237828213721514
22200 0.00234404671937227
22300 0.00235221046023071
22400 0.00238799885846674
22500 0.0023832656443119
22600 0.00236369227059186
22700 0.002372563816607
22900 0.00235937512479722
23000 0.00236206059344113
23100 0.00234905024990439
23200 0.00237814383581281
23300 0.00236066314391792
}; \addlegendentry{K2}
