# Supplementary material for: Neural Networks with Physics-Informed Architectures and Constraints for Dynamical Systems Modeling
Source: arXiv:2109.06407 source file (2022-12-12)
Supplement: Supplementary file 25 [file traj_err_data.tex]

\path [fill=red, fill opacity=0.4, ultra thick]
(axis cs:1,0.425842757042726)
--(axis cs:1,0.369011197968586)
--(axis cs:5,0.340659076055574)
--(axis cs:15,0.215481461951959)
--(axis cs:25,0.161485036747361)
--(axis cs:50,0.121269717837292)
--(axis cs:100,0.122246150710438)
--(axis cs:100,0.199646389379003)
--(axis cs:100,0.199646389379003)
--(axis cs:50,0.204837884818649)
--(axis cs:25,0.260791318943091)
--(axis cs:15,0.310860167617414)
--(axis cs:5,0.379305355618416)
--(axis cs:1,0.425842757042726)
--cycle;

\path [fill=blue, fill opacity=0.4, ultra thick]
(axis cs:1,0.425728743098355)
--(axis cs:1,0.368476143608182)
--(axis cs:5,0.340969836179182)
--(axis cs:15,0.198690673072993)
--(axis cs:25,0.164320584402678)
--(axis cs:50,0.115447289735228)
--(axis cs:100,0.122139999108882)
--(axis cs:100,0.158075039864172)
--(axis cs:100,0.158075039864172)
--(axis cs:50,0.158764253051484)
--(axis cs:25,0.259565857354428)
--(axis cs:15,0.300096100030564)
--(axis cs:5,0.38032091498312)
--(axis cs:1,0.425728743098355)
--cycle;

\path [fill=green!50.1960784313725!black, fill opacity=0.4, ultra thick]
(axis cs:1,0.403154509634611)
--(axis cs:1,0.360432041582331)
--(axis cs:5,0.0947917792092252)
--(axis cs:15,0.0874259090992881)
--(axis cs:25,0.0684932792479964)
--(axis cs:50,0.0639969877720852)
--(axis cs:100,0.0616857911404033)
--(axis cs:100,0.0796748887686242)
--(axis cs:100,0.0796748887686242)
--(axis cs:50,0.0856512706605412)
--(axis cs:25,0.0920321341262693)
--(axis cs:15,0.121028934402069)
--(axis cs:5,0.146313848306424)
--(axis cs:1,0.403154509634611)
--cycle;

\addplot [ultra thick, red, mark=*, mark size=1.5, mark options={solid}]
table {%
1 0.3974269926548
5 0.359982252120972
15 0.263170778751373
25 0.211138218641281
50 0.163053810596466
100 0.160946264863014
};
\addplot [ultra thick, blue, mark=*, mark size=1.5, mark options={solid}]
table {%
1 0.397102475166321
5 0.36064538359642
15 0.249393373727798
25 0.211943238973618
50 0.137105777859688
100 0.140107527375221
};
\addplot [ultra thick, green!50.1960784313725!black, mark=*, mark size=1.5, mark options={solid}]
table {%
1 0.381793349981308
5 0.120552815496922
15 0.104227423667908
25 0.0802627131342888
50 0.0748241320252419
100 0.0706803351640701
};
